# Supplementary material for: Certifiably Optimal Outlier-Robust Geometric Perception: Semidefinite Relaxations and Scalable Global Optimization
Source: arXiv:2109.03349 source file (2022-05-29)
Supplement: Supplementary file 2 [file supp-fig-3dmatch.tex]

%!TEX root = ../main.tex
\renewcommand{\myhspace}{\hspace{-3mm}}
\renewcommand{\mpwtwo}{9.0cm}
\begin{figure*}[t]
	\begin{center}
	\begin{minipage}{\textwidth}
	\begin{tabular}{cc}%
		\myhspace
		\begin{minipage}{\mpwtwo}%
		\centering%
		\includegraphics[width=0.9\columnwidth]{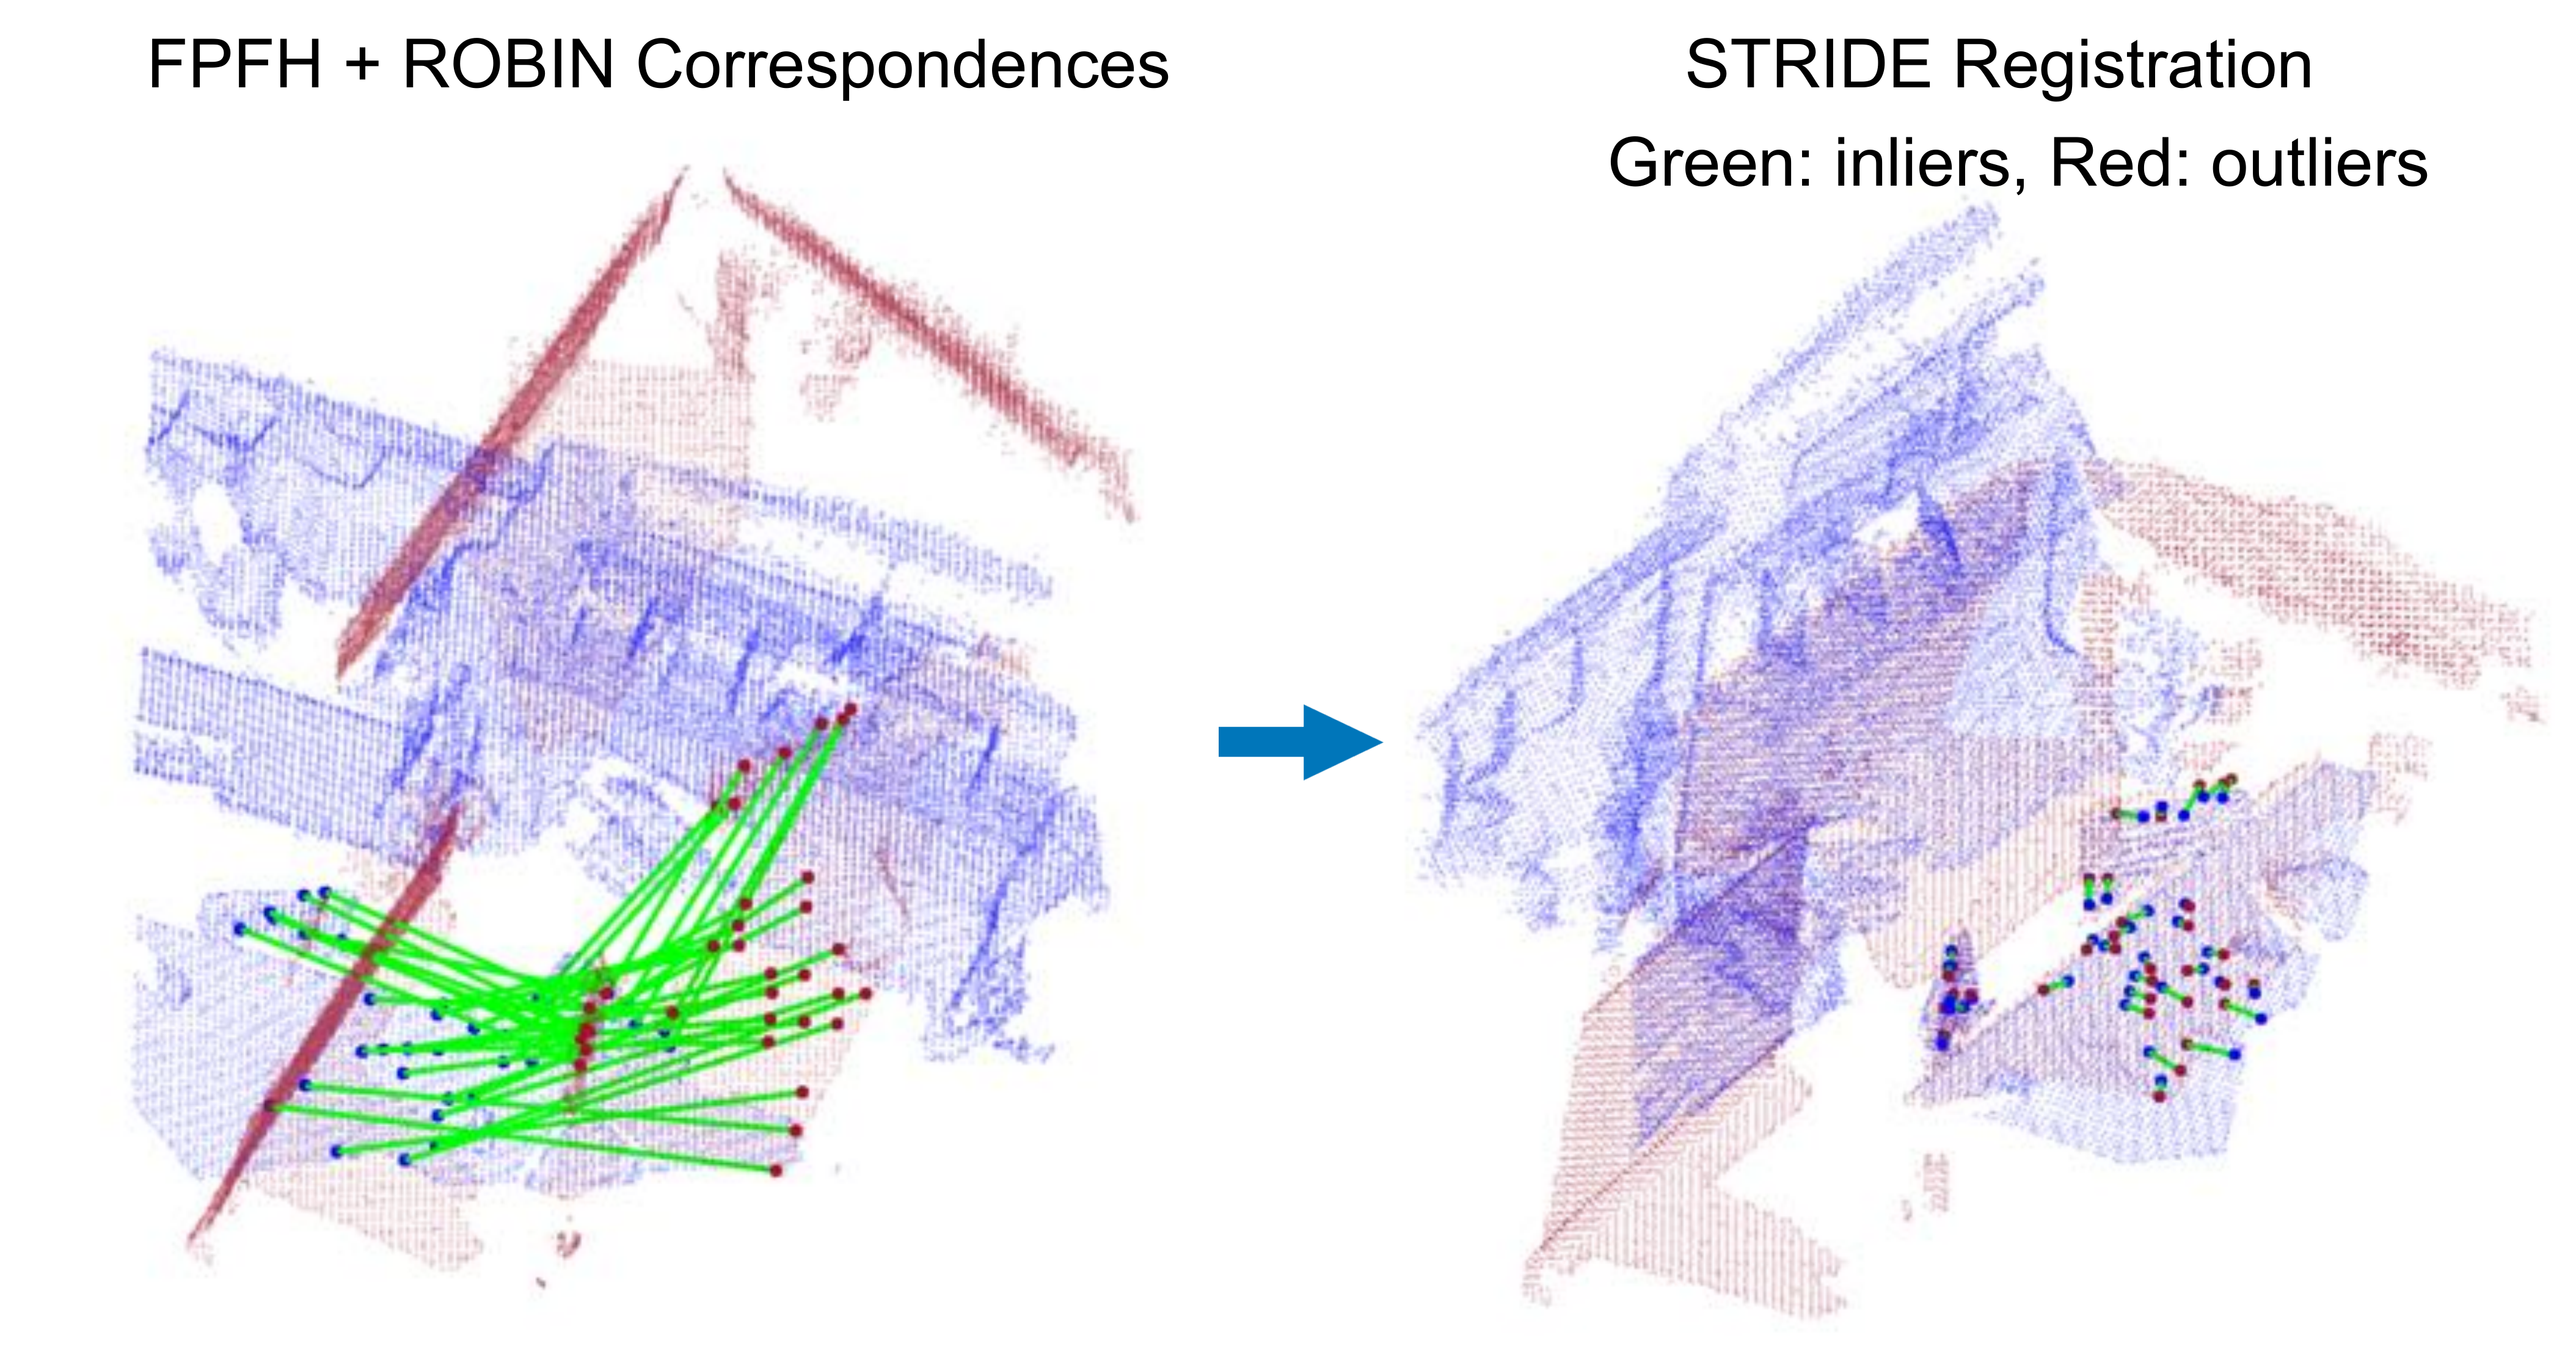}
		\\
		{\subcapsize (a) $\MR$ error: $2.8^{\circ}$, $\vt$ error: $1.2\ee{-1}$,  $\subopt = 6.5\ee{-8}$, time: $129$ [s]}
		\end{minipage}

		& 
		\myhspace
		\begin{minipage}{\mpwtwo}%
		\centering%
		\includegraphics[width=0.9\columnwidth]{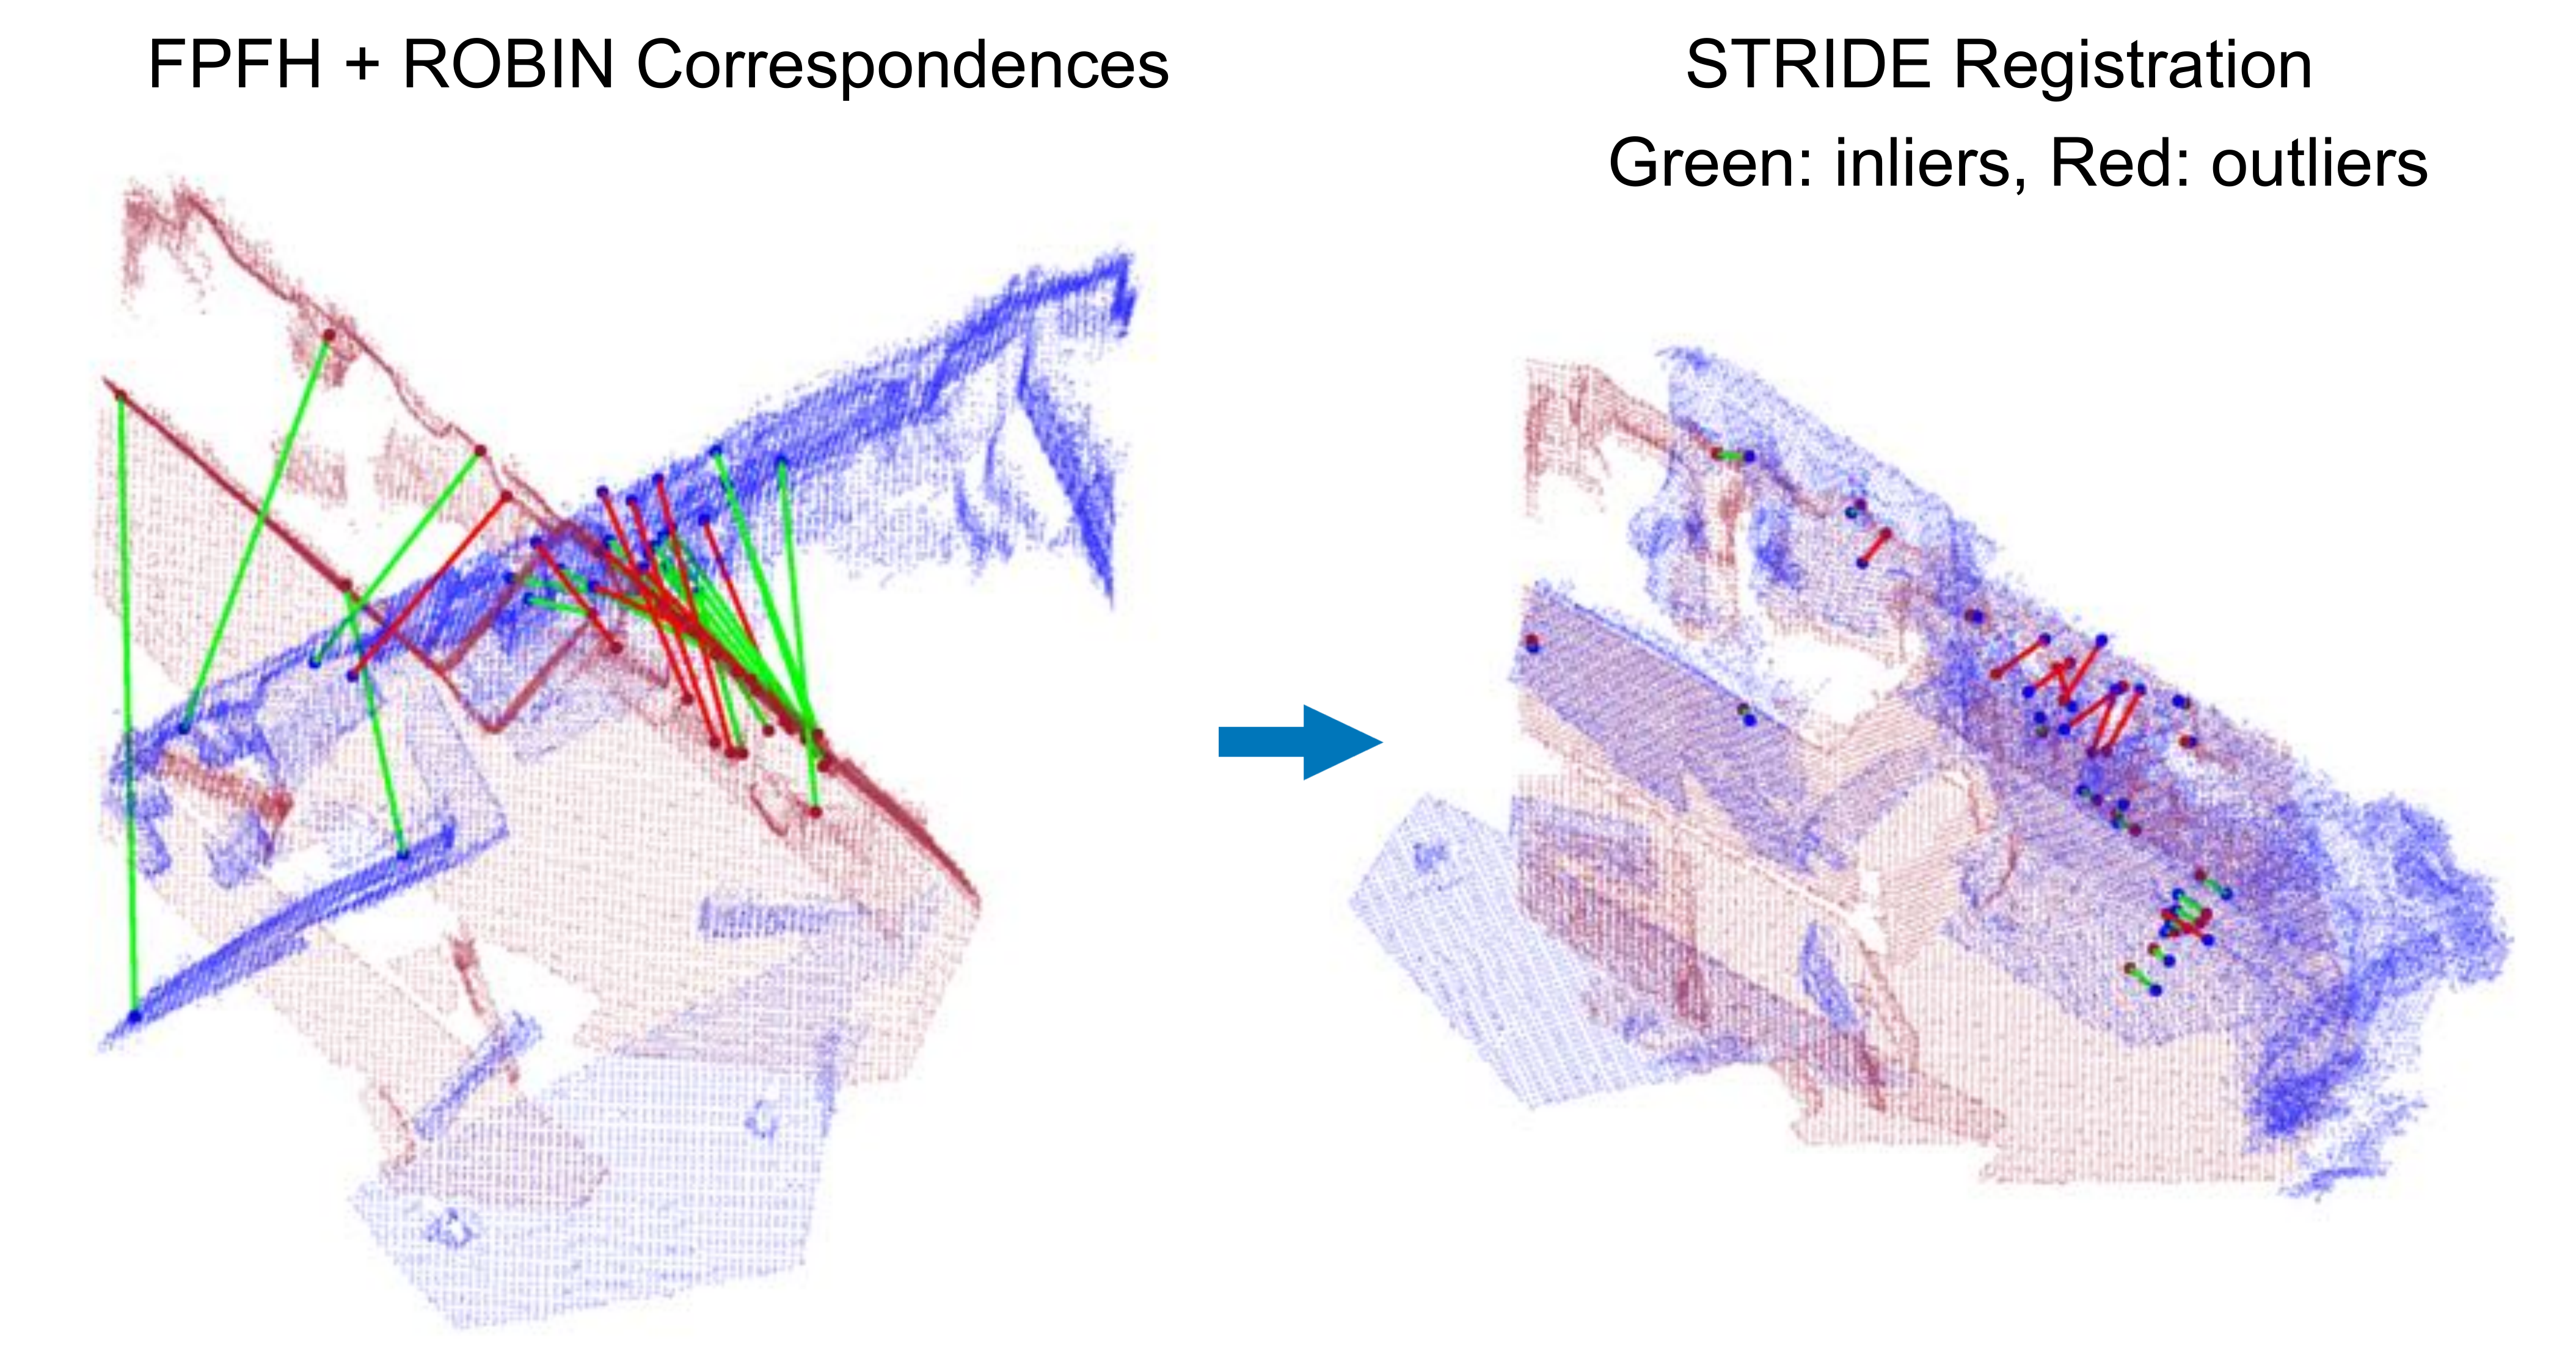}
		\\
		{\subcapsize (b) $\MR$ error: $3.0^{\circ}$, $\vt$ error: $1.9\ee{-1}$,  $\subopt = 1.2\ee{-8}$, time: $228$ [s]}
		\end{minipage}

		\\

		\myhspace
		\begin{minipage}{\mpwtwo}%
		\centering%
		\includegraphics[width=0.9\columnwidth]{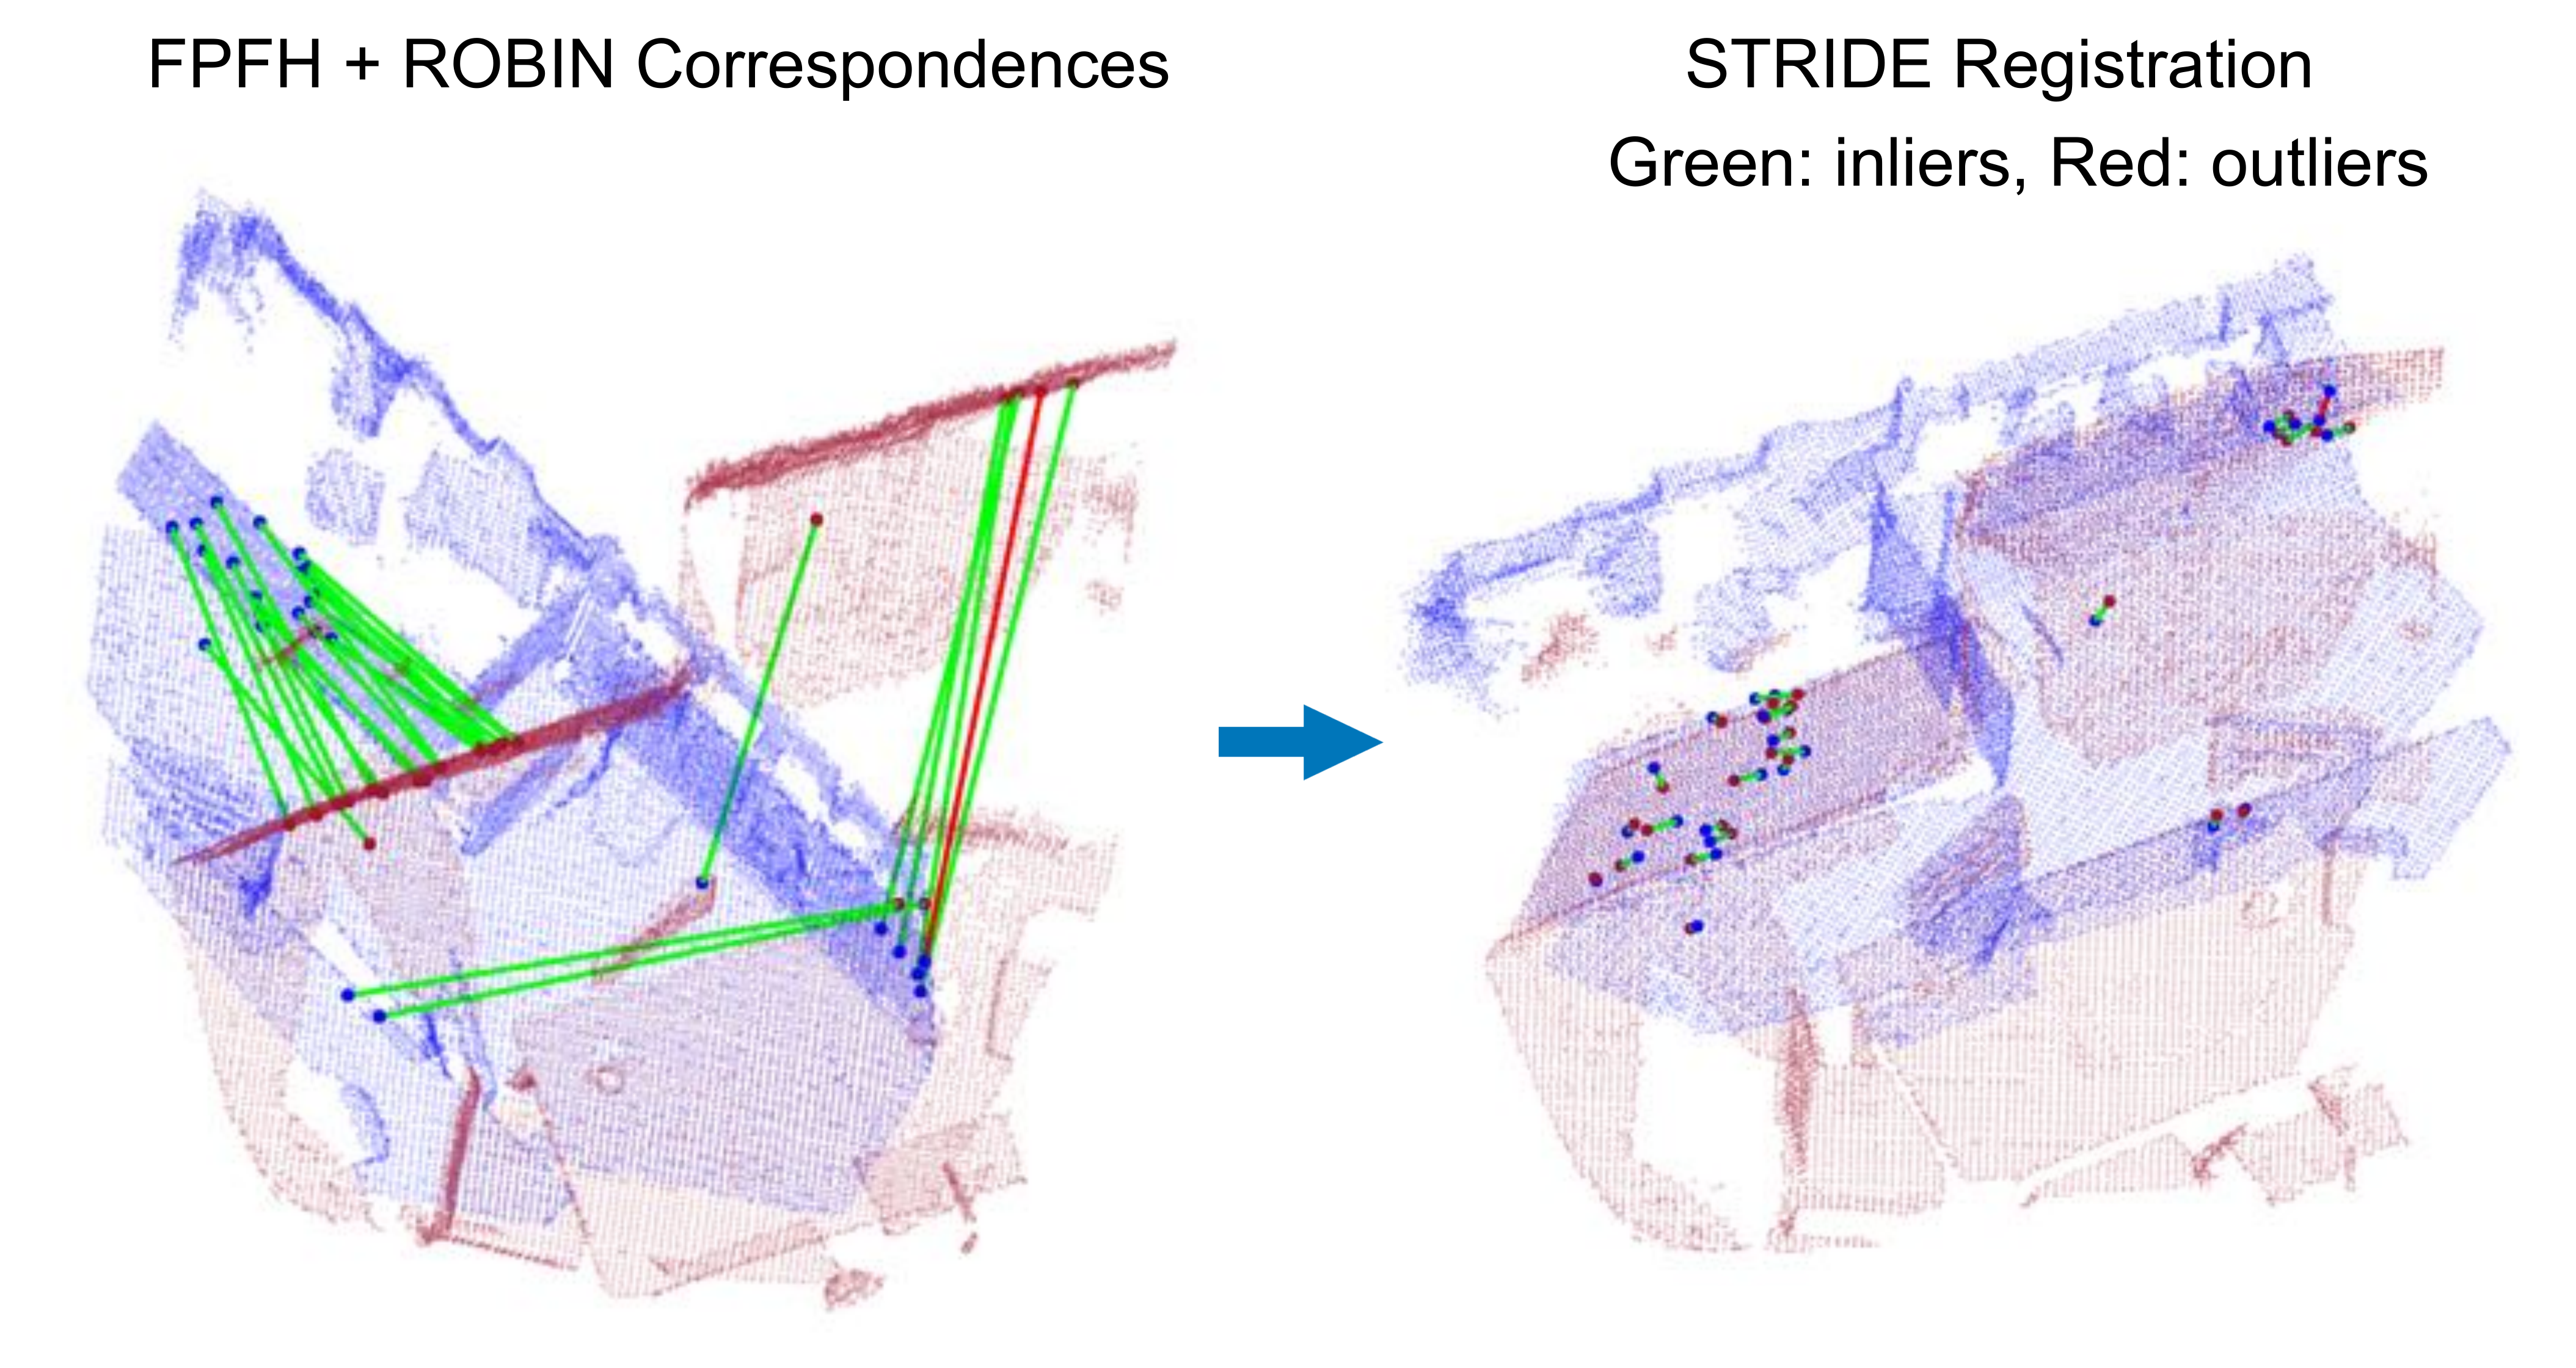}
		\\
		{\subcapsize (c) $\MR$ error: $4.3^{\circ}$, $\vt$ error: $1.7\ee{-1}$,  $\subopt = 2.1\ee{-8}$, time: $117$ [s]}
		\end{minipage}

		& 
		\myhspace
		\begin{minipage}{\mpwtwo}%
		\centering%
		\includegraphics[width=0.9\columnwidth]{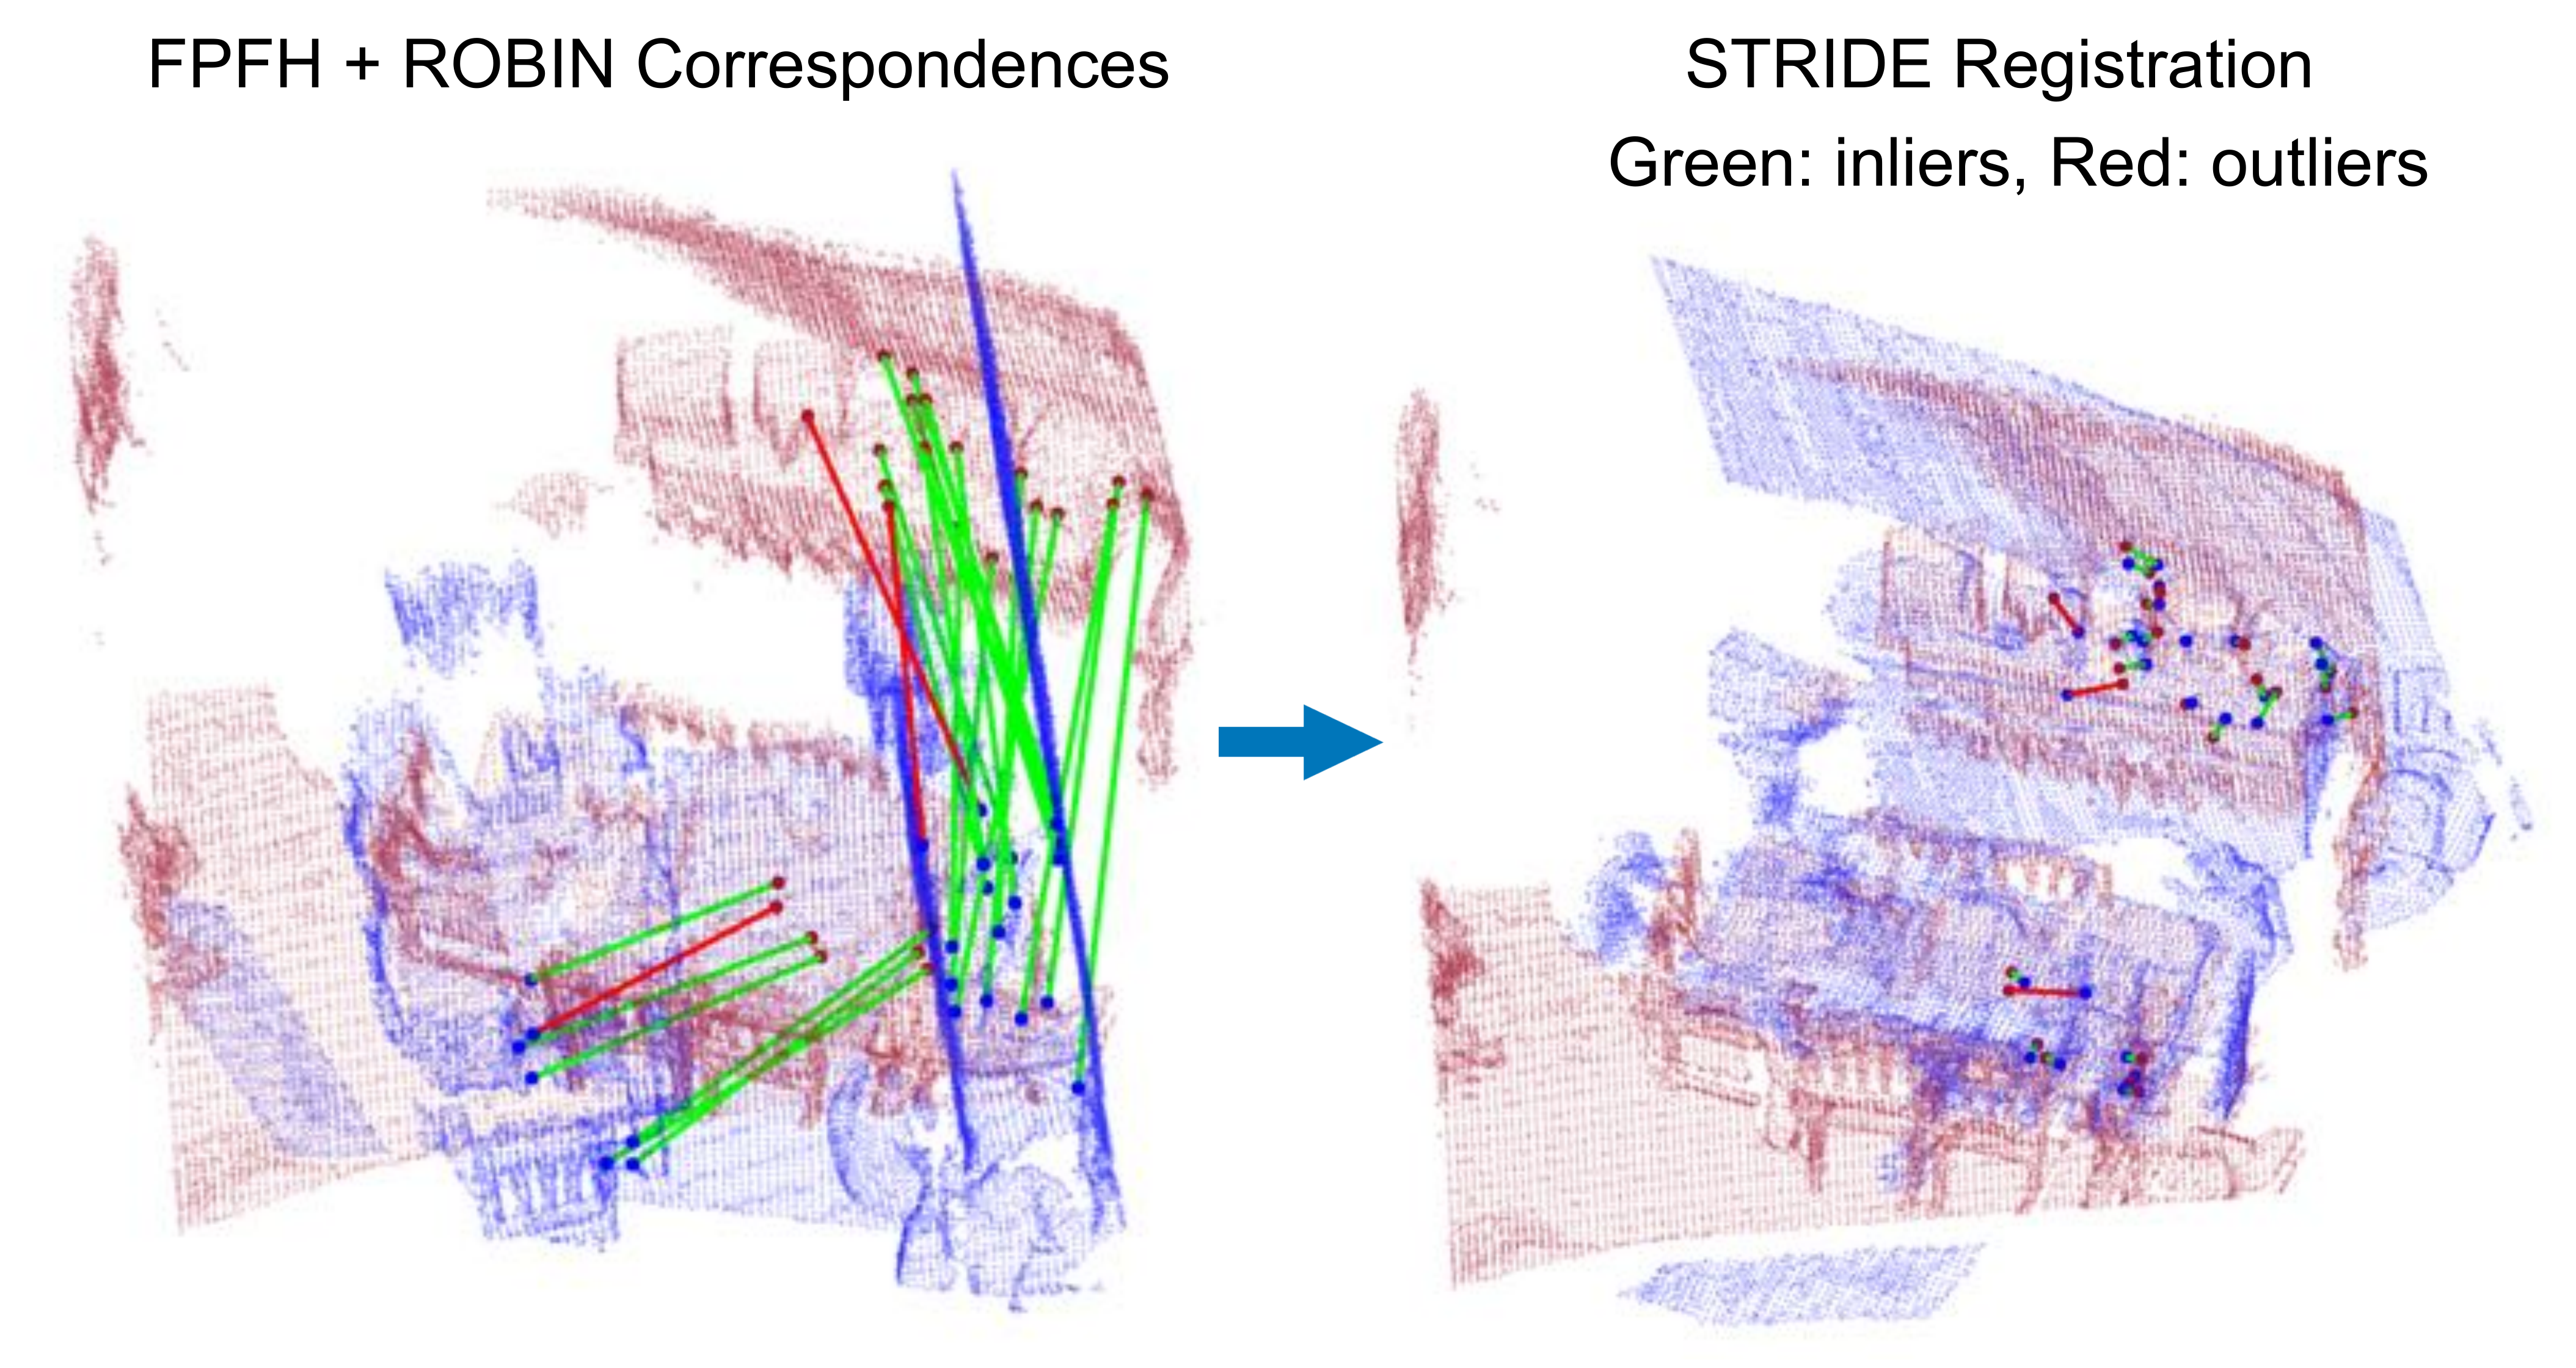}
		\\
		{\subcapsize (d) $\MR$ error: $2.3^{\circ}$, $\vt$ error: $1.5\ee{-1}$,  $\subopt = 2.2\ee{-8}$, time: $134$ [s]}
		\end{minipage}

		\\

		\myhspace
		\begin{minipage}{\mpwtwo}%
		\centering%
		\includegraphics[width=0.9\columnwidth]{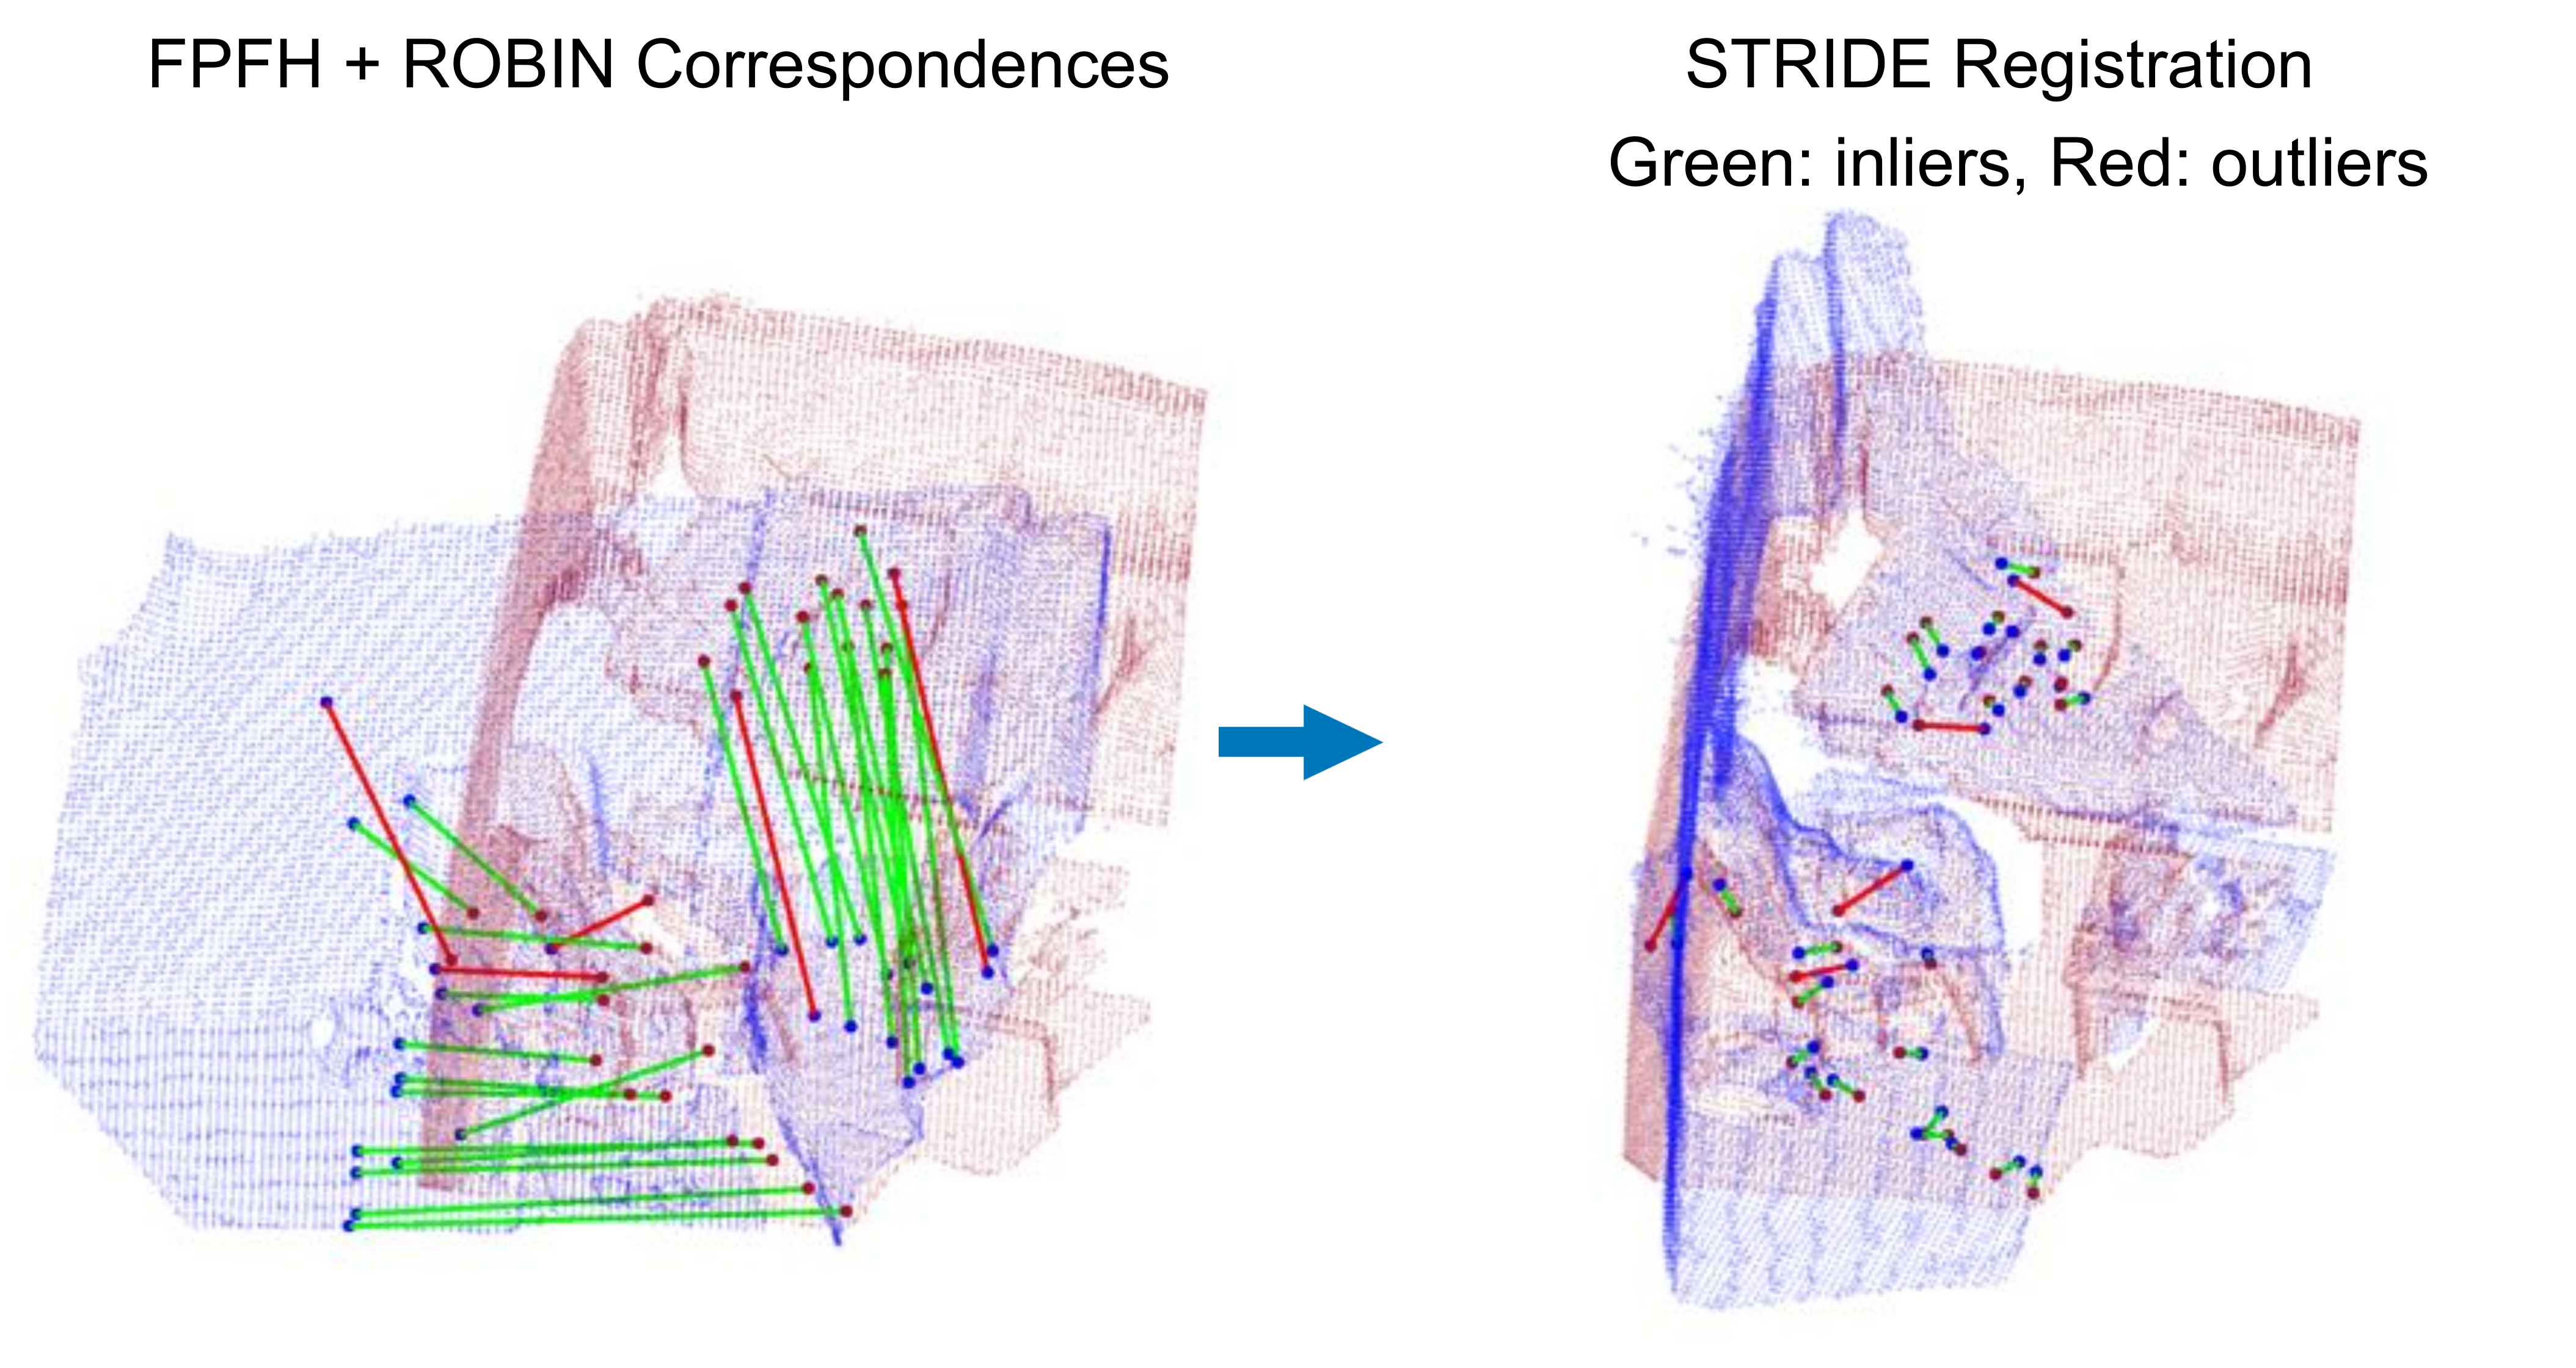}
		\\
		{\subcapsize (e) $\MR$ error: $4.5^{\circ}$, $\vt$ error: $2.3\ee{-1}$,  $\subopt = 1.3\ee{-8}$, time: $176$ [s]}
		\end{minipage}

		& 
		\myhspace
		\begin{minipage}{\mpwtwo}%
		\centering%
		\includegraphics[width=0.9\columnwidth]{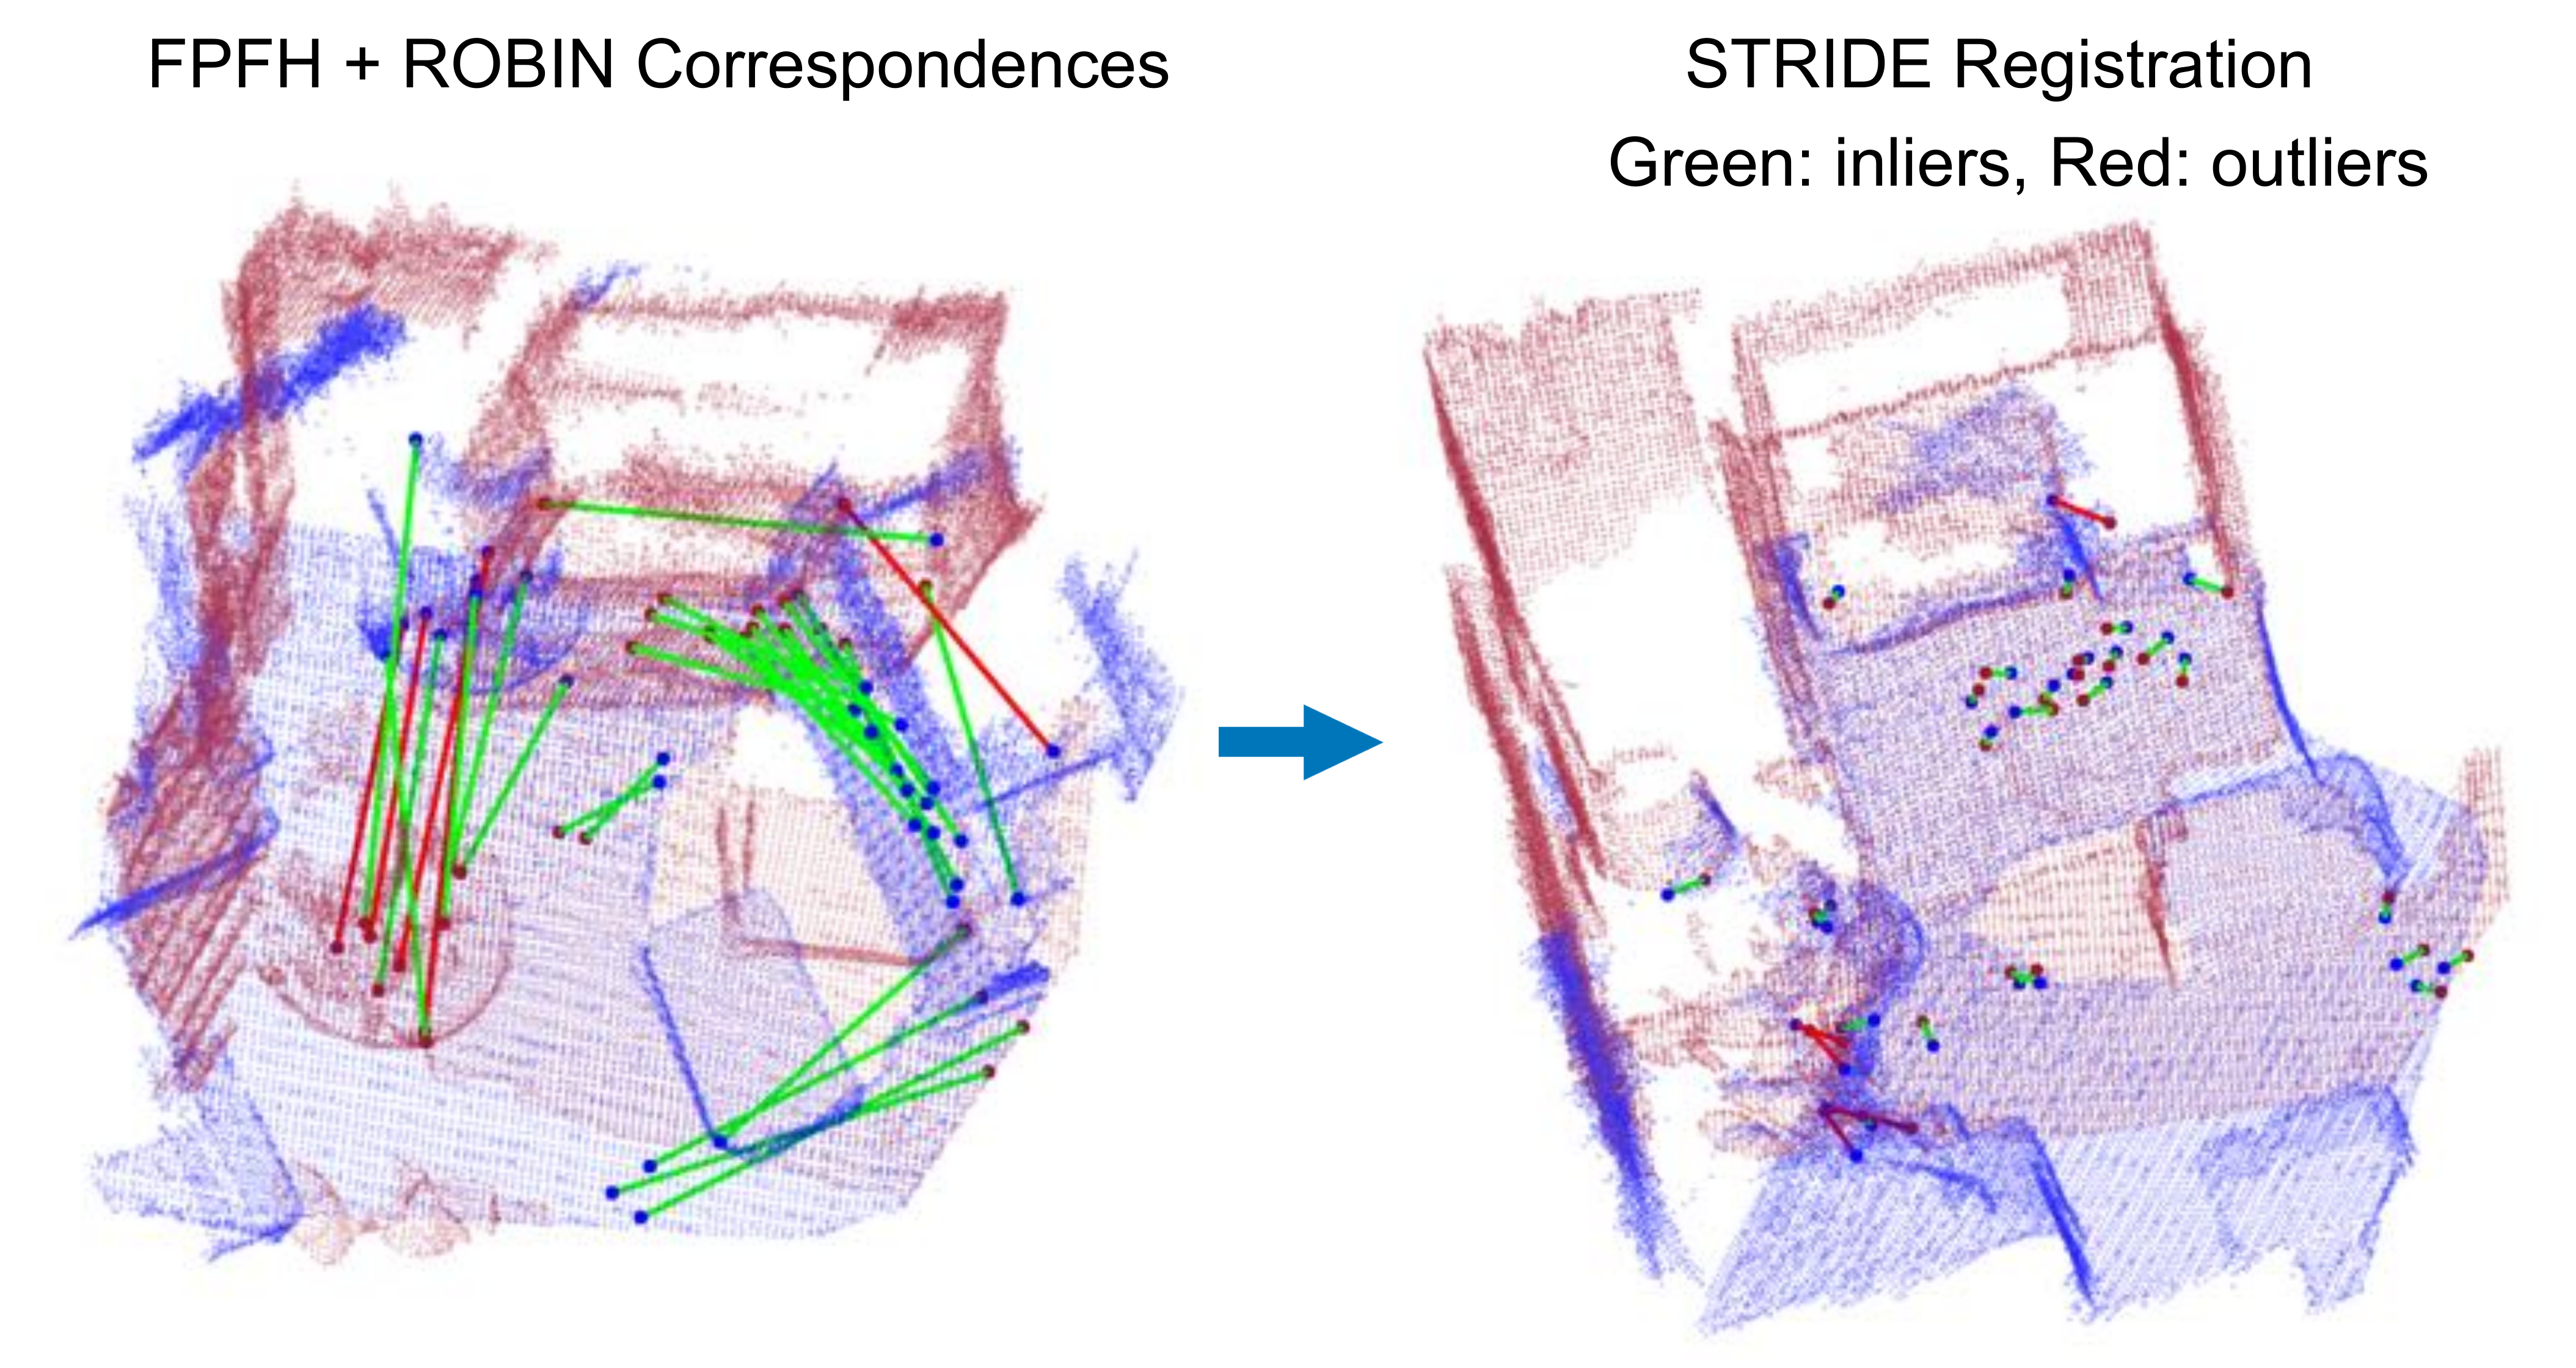}
		\\
		{\subcapsize (f) $\MR$ error: $3.1^{\circ}$, $\vt$ error: $1.6\ee{-1}$,  $\subopt = 2.4\ee{-8}$, time: $187$ [s]}
		\end{minipage}

		\\

		\myhspace
		\begin{minipage}{\mpwtwo}%
		\centering%
		\includegraphics[width=0.9\columnwidth]{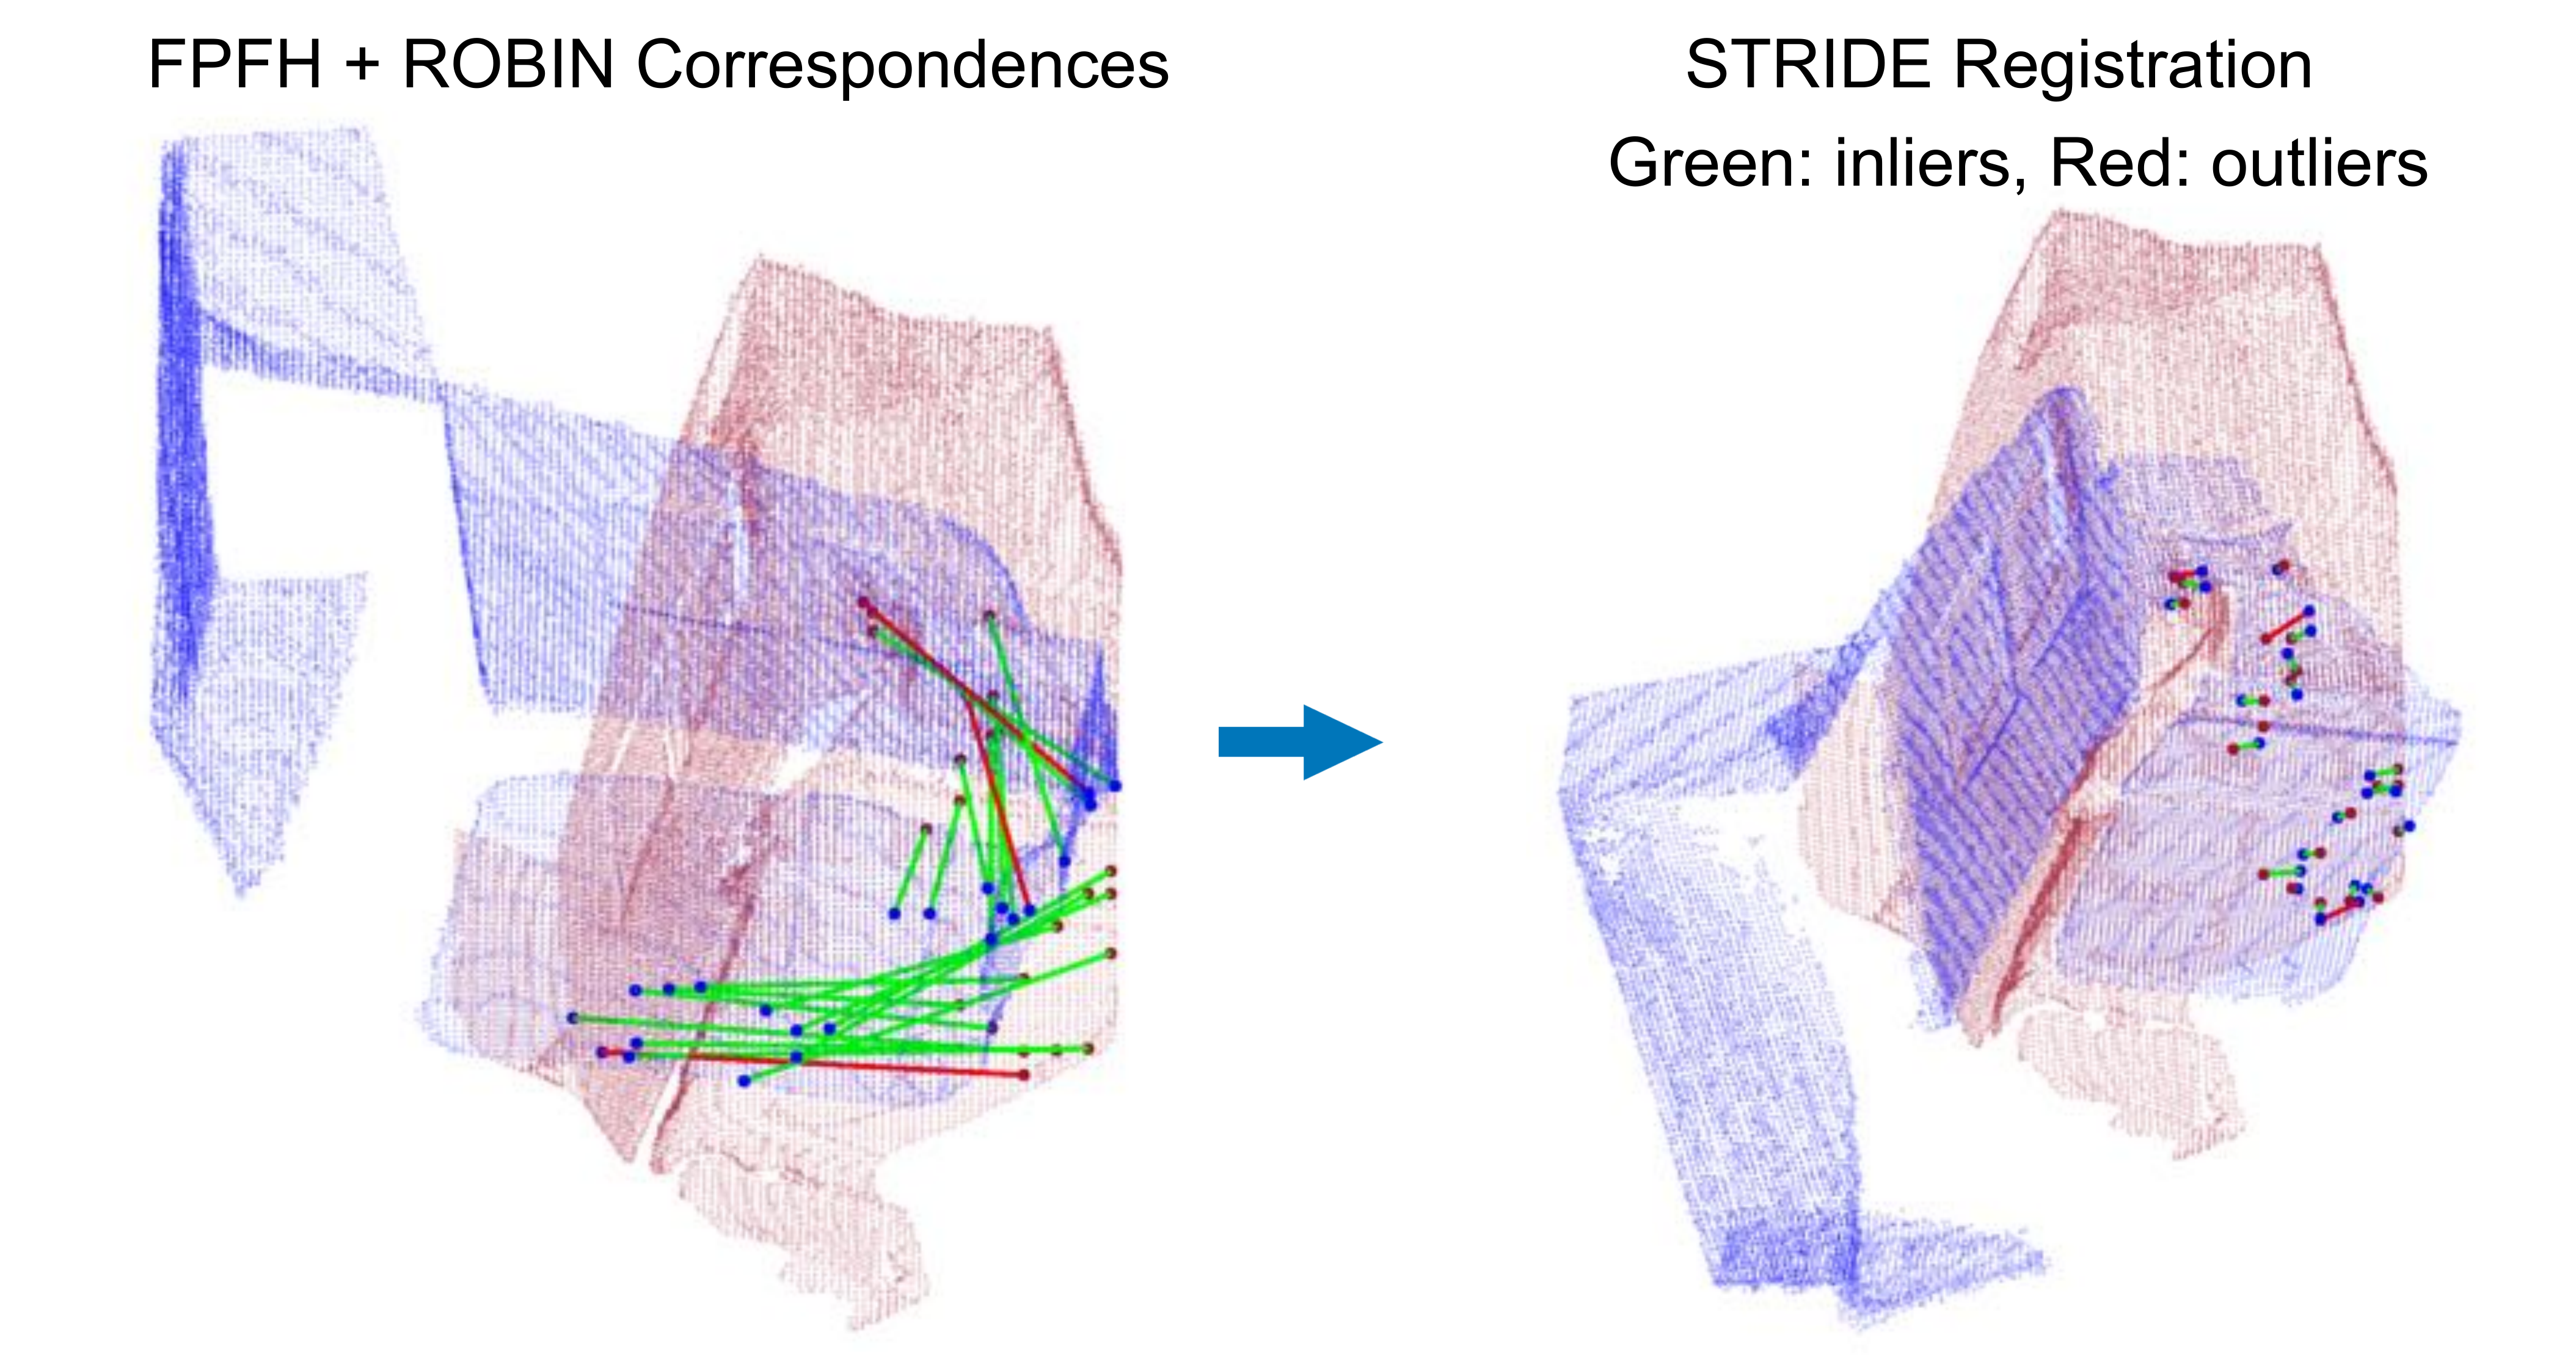}
		\\
		{\subcapsize (g) $\MR$ error: $2.4^{\circ}$, $\vt$ error: $8.9\ee{-2}$,  $\subopt = 2.4\ee{-8}$, time: $117$ [s]}
		\end{minipage}

		& 
		\myhspace
		\begin{minipage}{\mpwtwo}%
		\centering%
		\includegraphics[width=0.9\columnwidth]{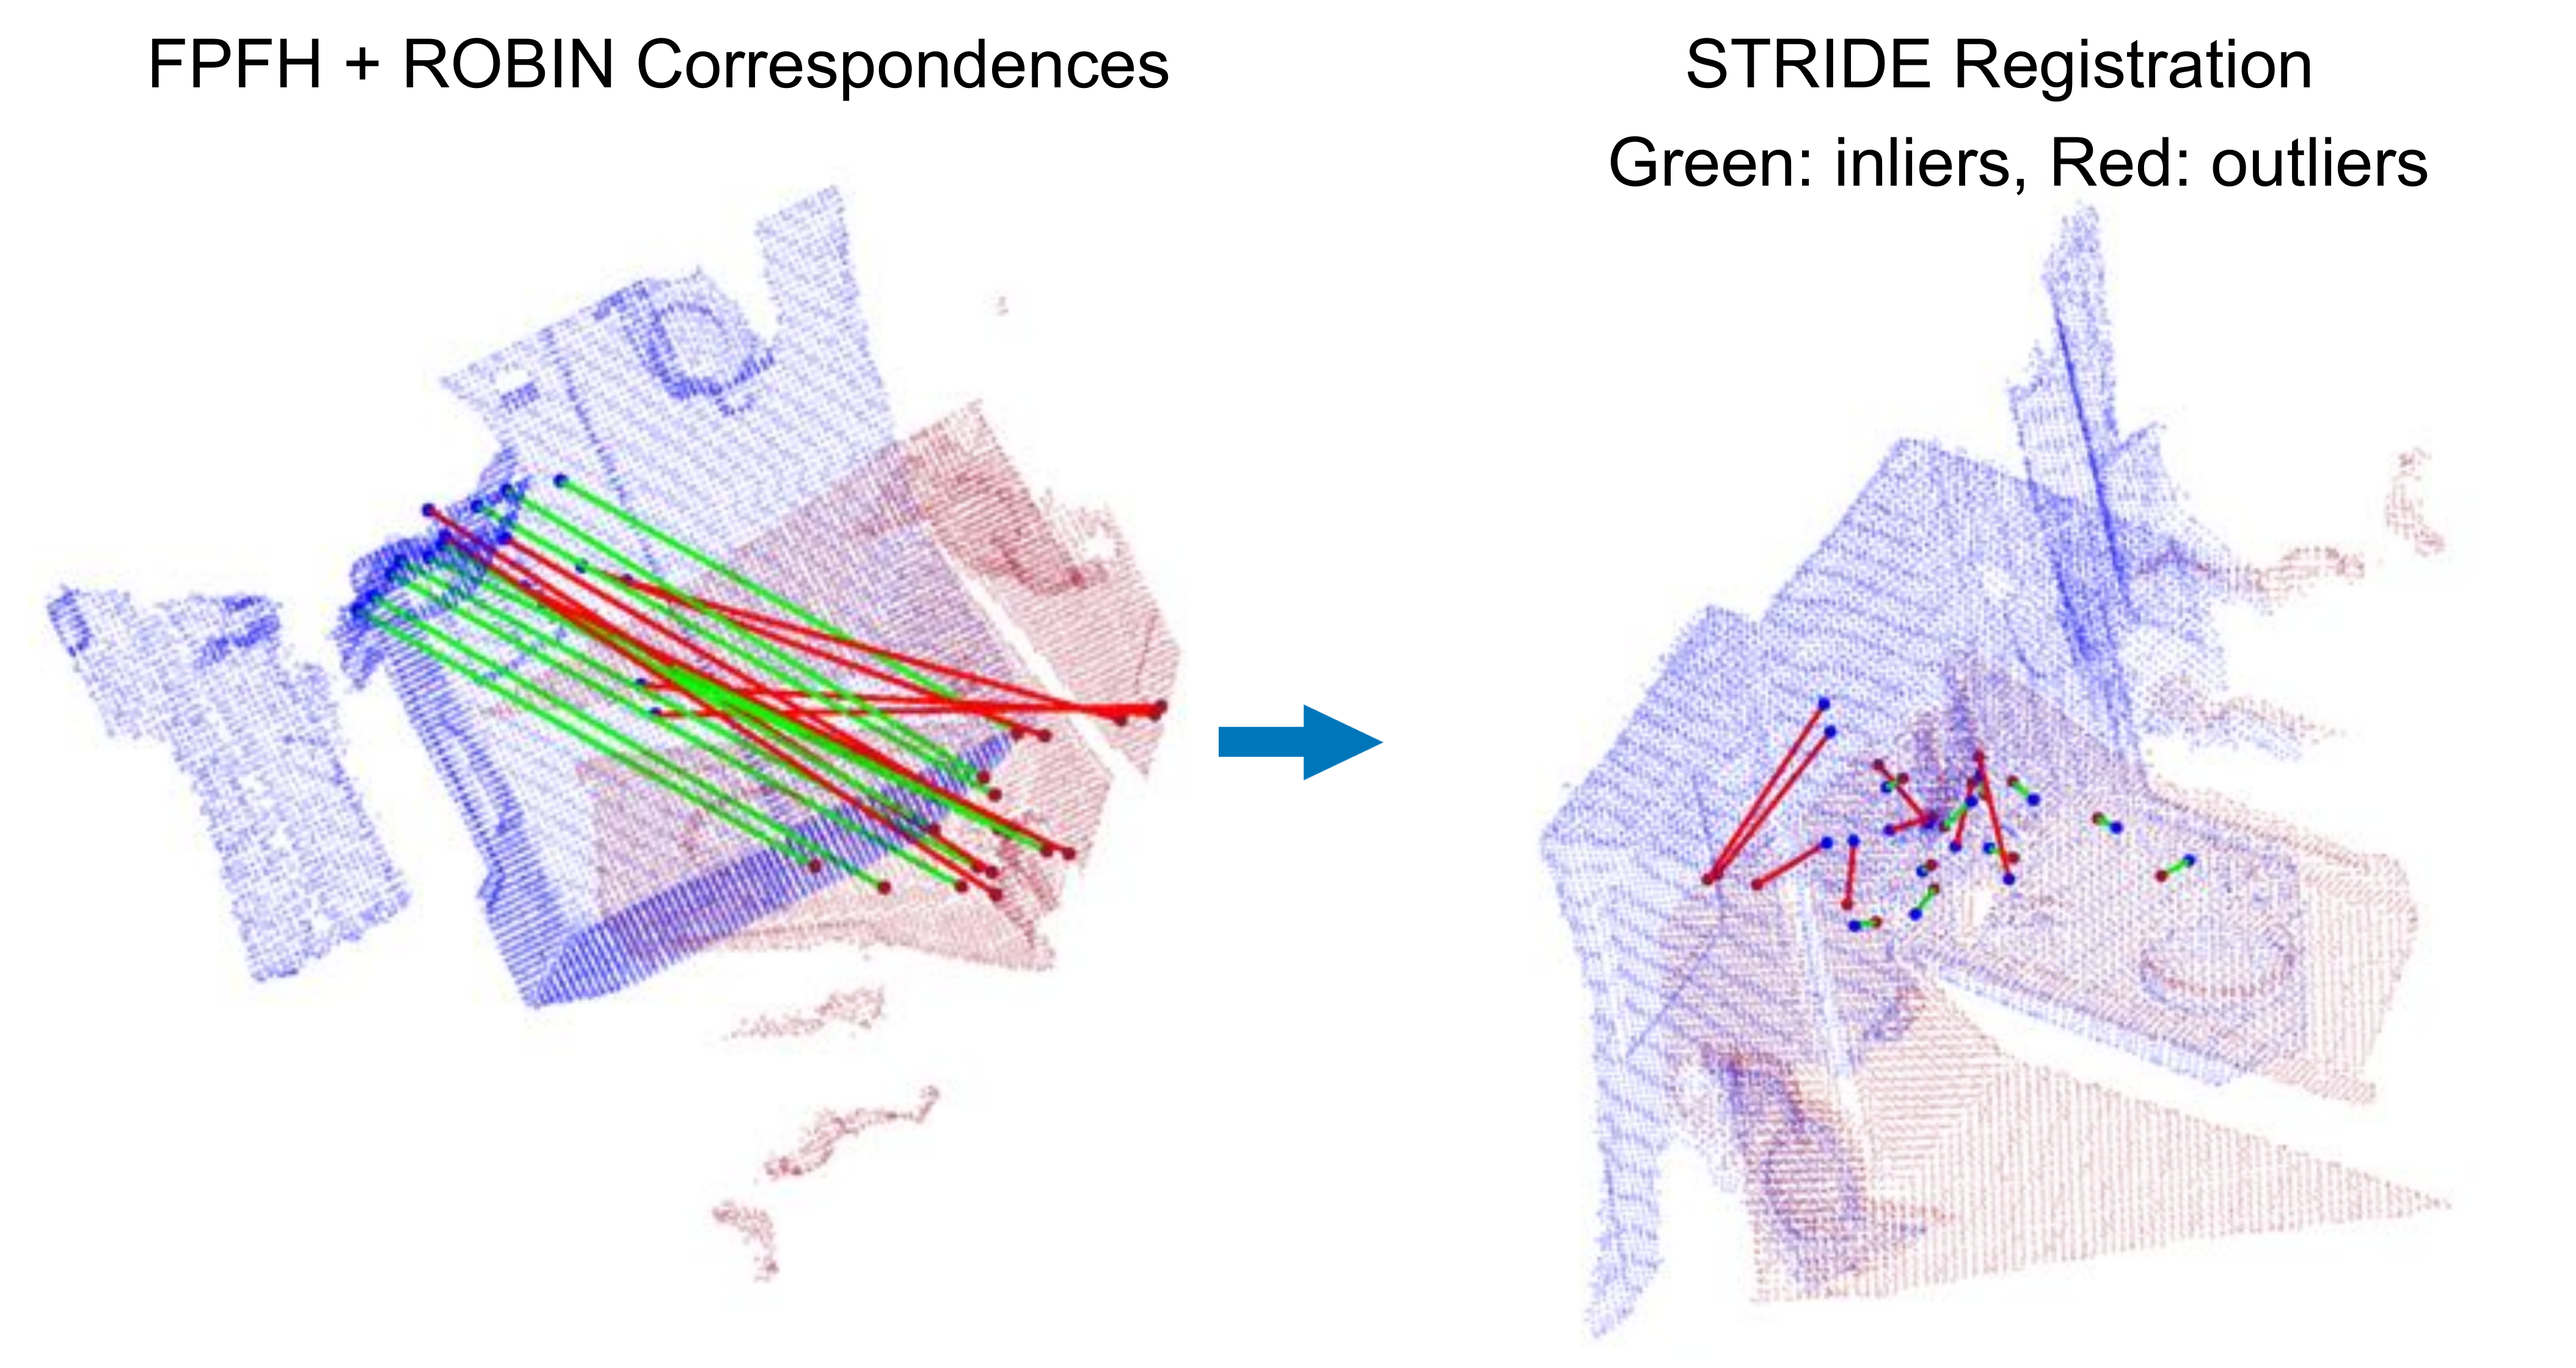}
		\\
		{\subcapsize (h) $\MR$ error: $3.2^{\circ}$, $\vt$ error: $1.5\ee{-1}$,  $\subopt = 4.5\ee{-8}$, time: $81$ [s]}
		\end{minipage}
		\\

		\myhspace
		\begin{minipage}{\mpwtwo}%
		\centering%
		\includegraphics[width=0.9\columnwidth]{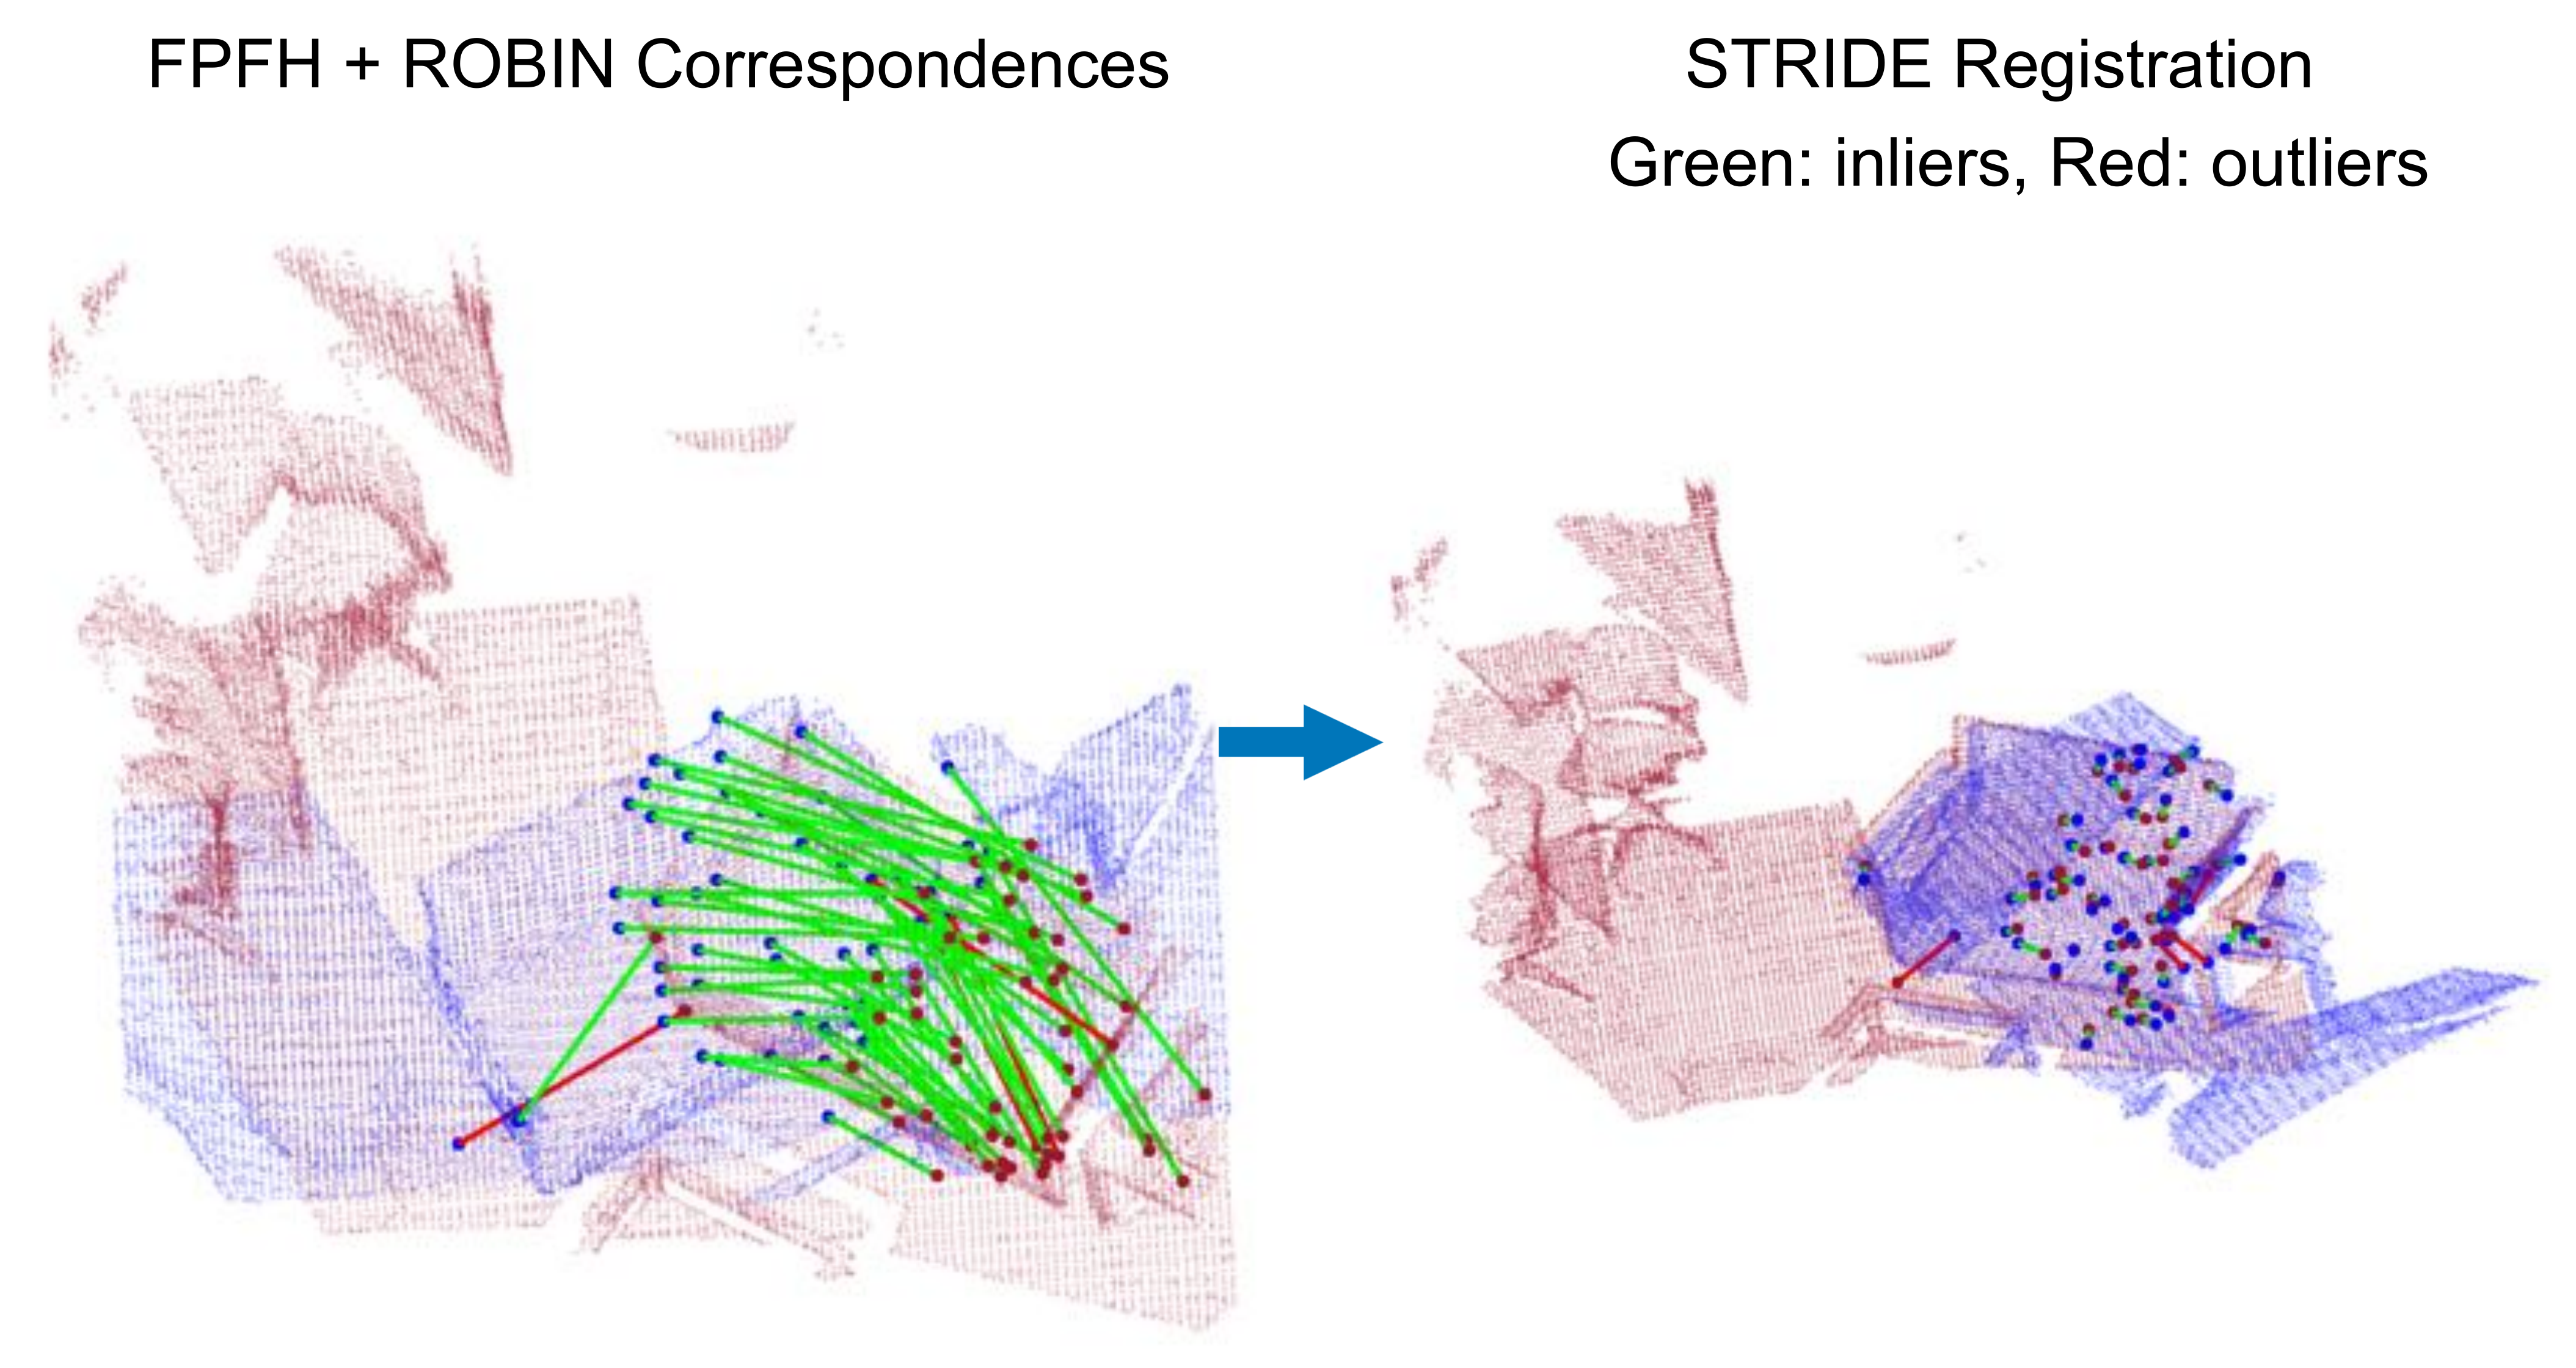}
		\\
		{\subcapsize (i) $\MR$ error: $3.5^{\circ}$, $\vt$ error: $1.3\ee{-1}$,  $\subopt = 1.7\ee{-6}$, time: $874$ [s]}
		\end{minipage}

		& 
		\myhspace
		\begin{minipage}{\mpwtwo}%
		\centering%
		\includegraphics[width=0.9\columnwidth]{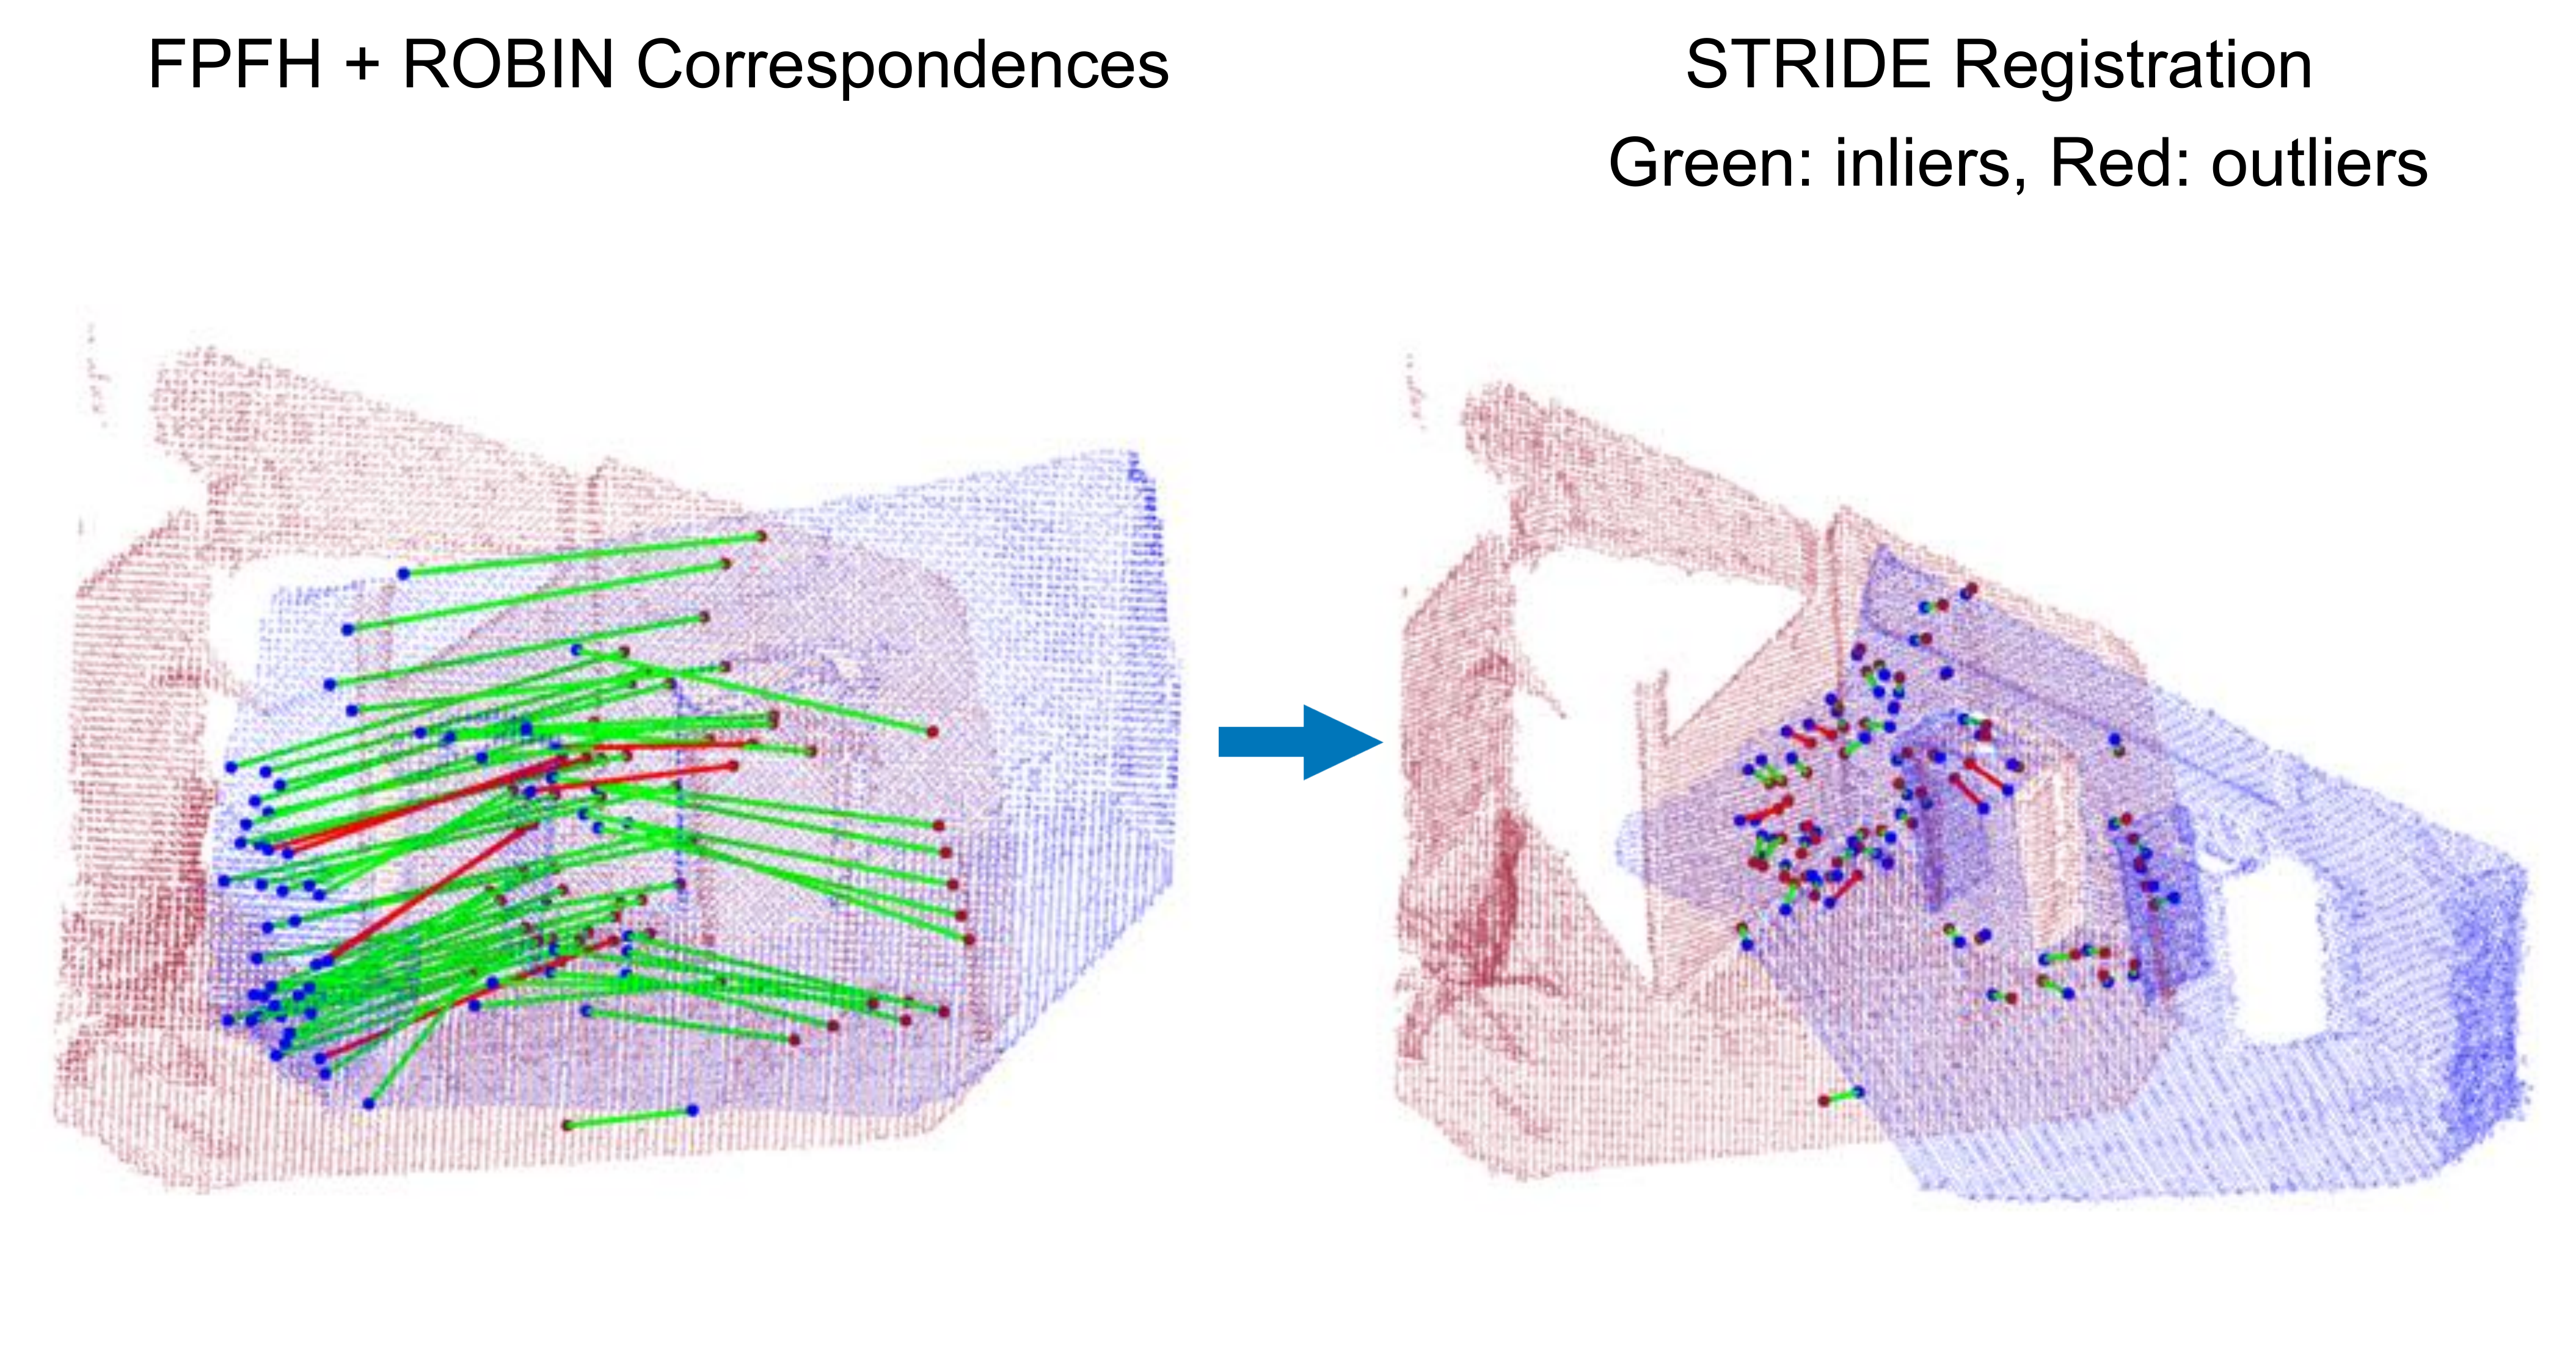}
		\\
		{\subcapsize (j) $\MR$ error: $3.4^{\circ}$, $\vt$ error: $1.9\ee{-1}$,  $\subopt = 3.8\ee{-10}$, time: $1560$ [s]}
		\end{minipage}
	\end{tabular}
	\end{minipage} 
	\caption{Extra scan matching results on {\threedmatch} \cite{Zeng17cvpr-3dmatch}.
	\label{fig:supp-3dmatch}} 
	\vspace{-7mm} 
	\end{center}
\end{figure*}
