# Supplementary material for: Certifiably Optimal Outlier-Robust Geometric Perception: Semidefinite Relaxations and Scalable Global Optimization
Source: arXiv:2109.03349 source file (2022-05-29)
Supplement: Supplementary file 3 [file supp-fig-apollo.tex]

%!TEX root = ../main.tex
% \vspace{-10mm}
\renewcommand{\mpwfour}{5cm}
\renewcommand{\myhspace}{\hspace{-4mm}}
\begin{figure*}[t]
	\begin{center}
	\begin{minipage}{\textwidth}
	\begin{tabular}{cccc}%
		%%%%%%%%%%%%%%%%%%%%%%%%%%%%%%%%%%%%%%%%%%%%%%%%%%%%%%%%%%%%%%%%%%%%%%%%%%%%%%%%%%%%%%%%%%%%%%%%%%%%%%%%%
		   \myhspace \hspace{-4mm}
			\begin{minipage}{\mpwfour}%
			\centering%
			\includegraphics[width=0.95\columnwidth]{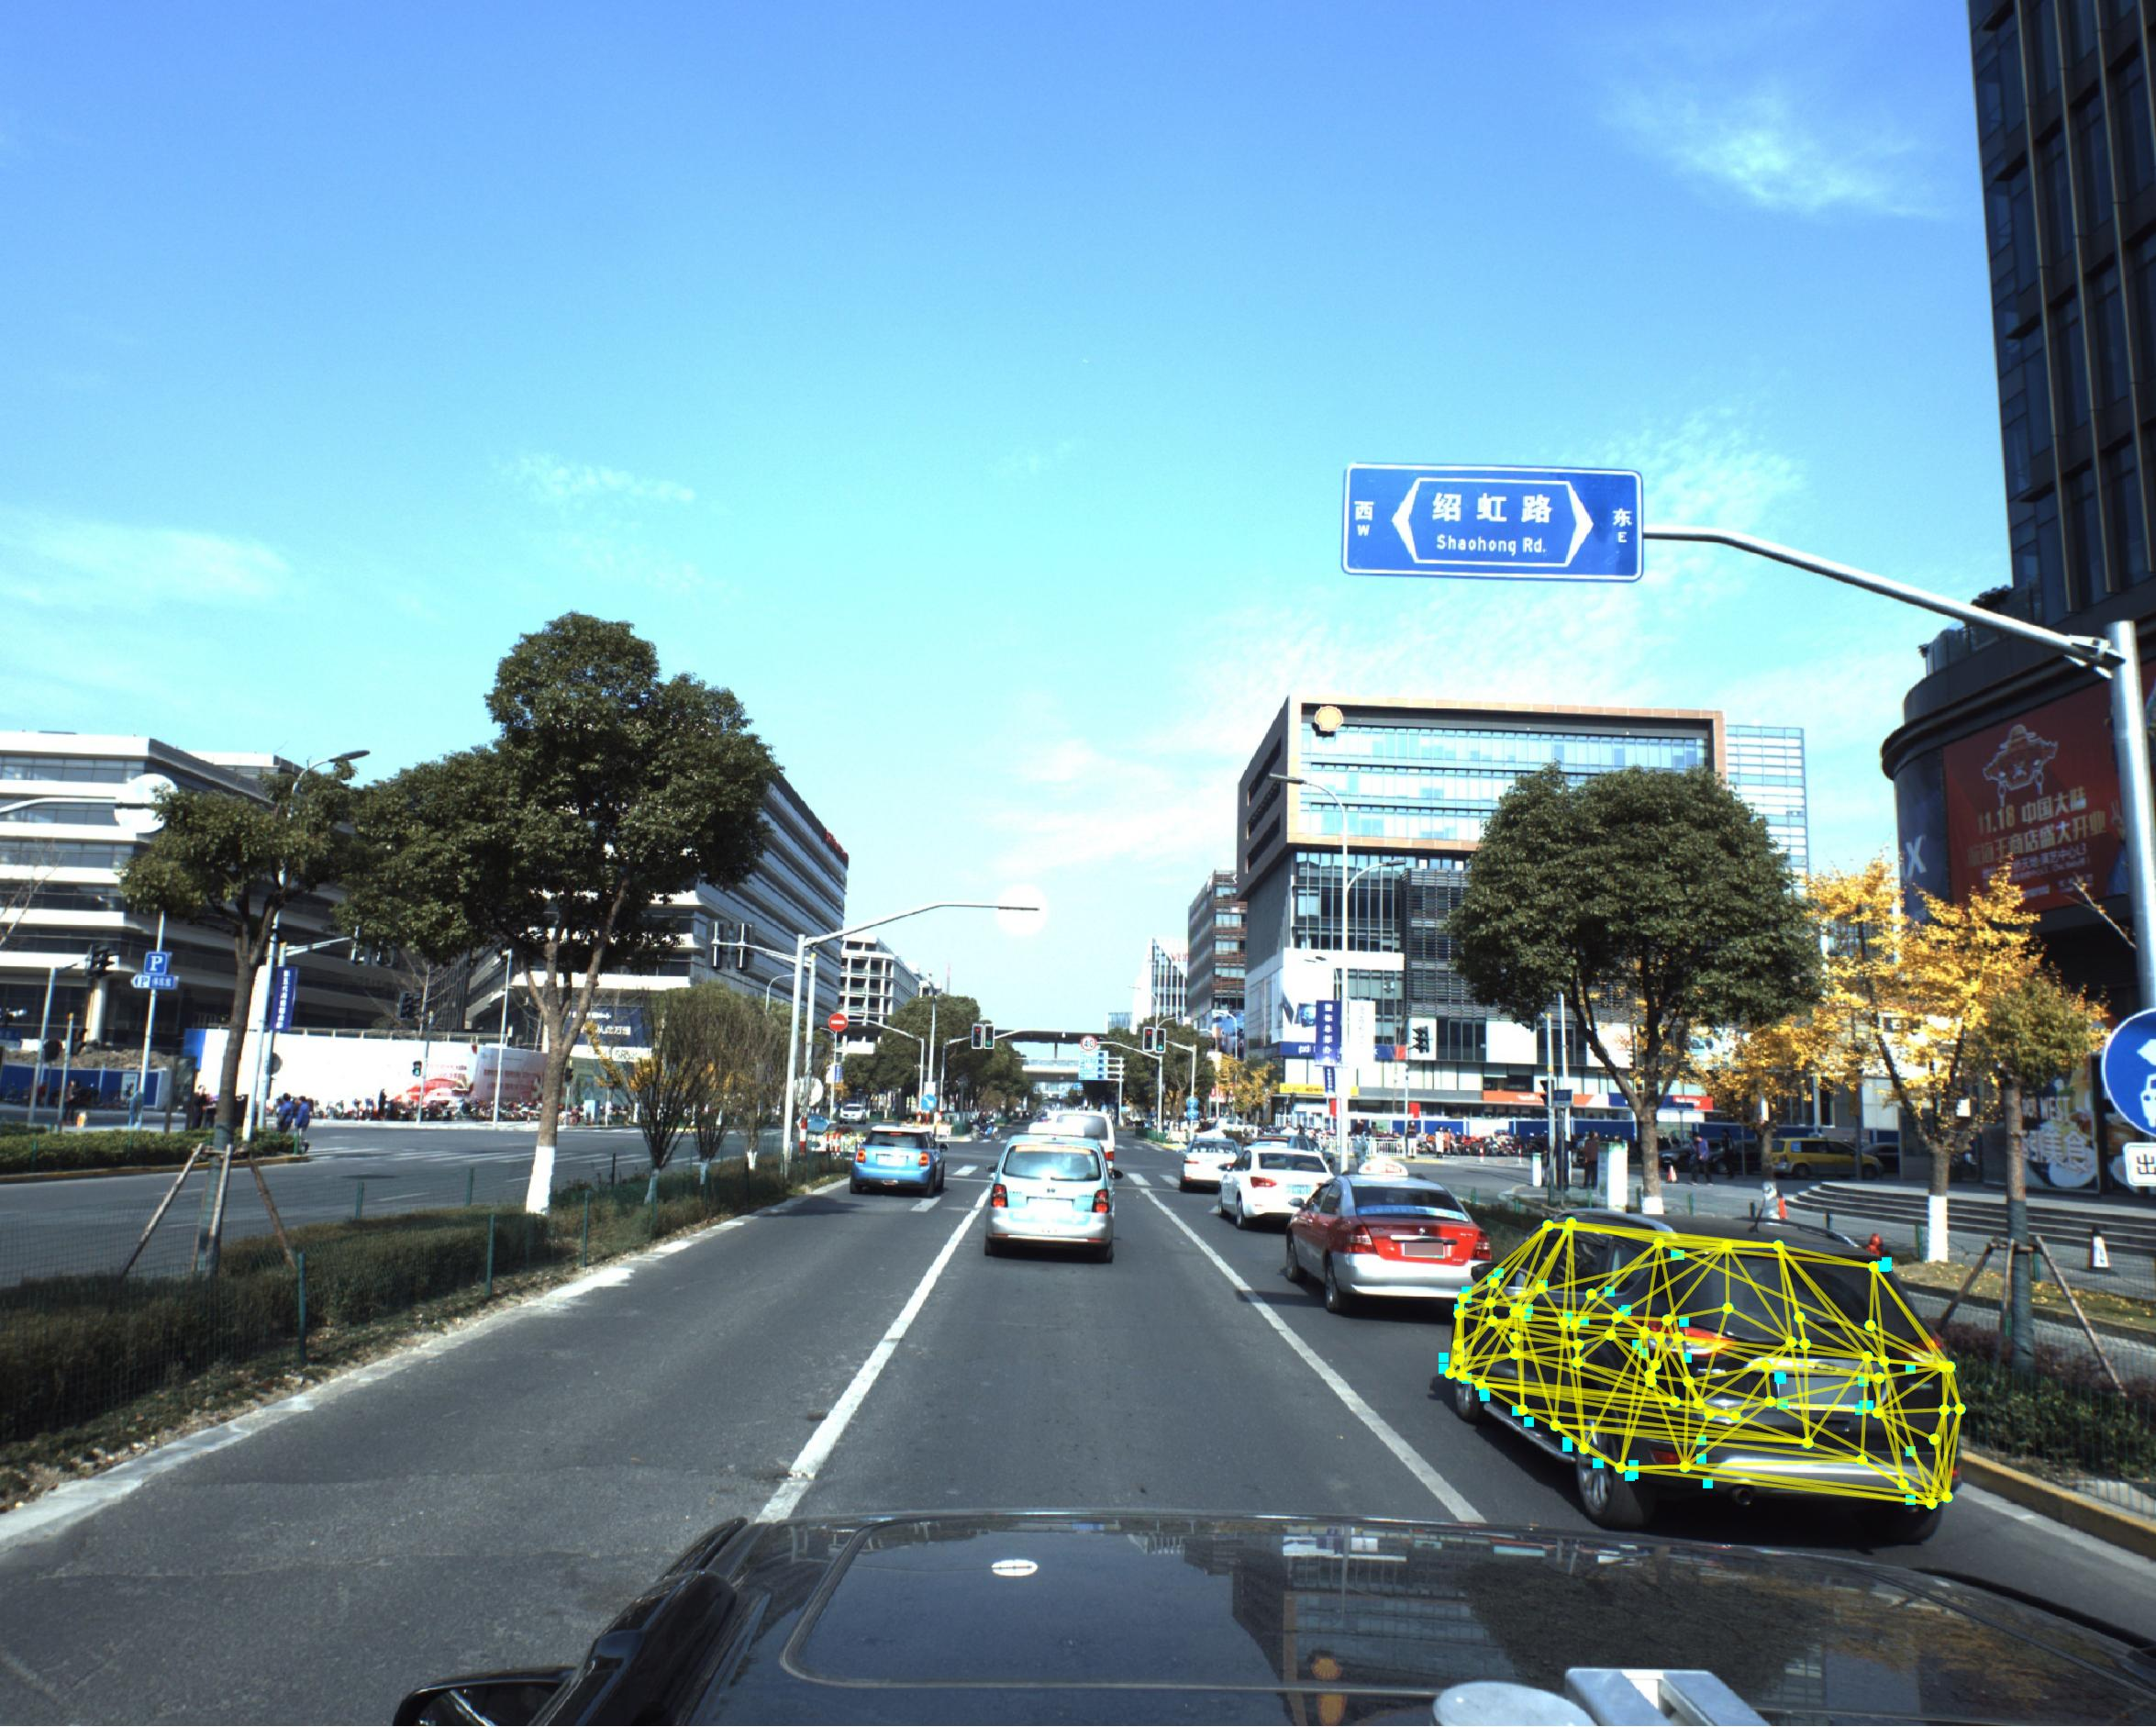} \\
			$\MR$ error: $1.75^{\circ}$, $\vt$ error: $0.09$ \\
			$\subopt=1.5\ee{-7}$, time: $4899$ [s] \\
			$n_1 = 1080, m=320,275$\\
			$N=59$, \# outliers: $26$
			\end{minipage}
		&  \myhspace \hspace{-3mm}
			\begin{minipage}{\mpwfour}%
			\centering%
			\includegraphics[width=0.95\columnwidth]{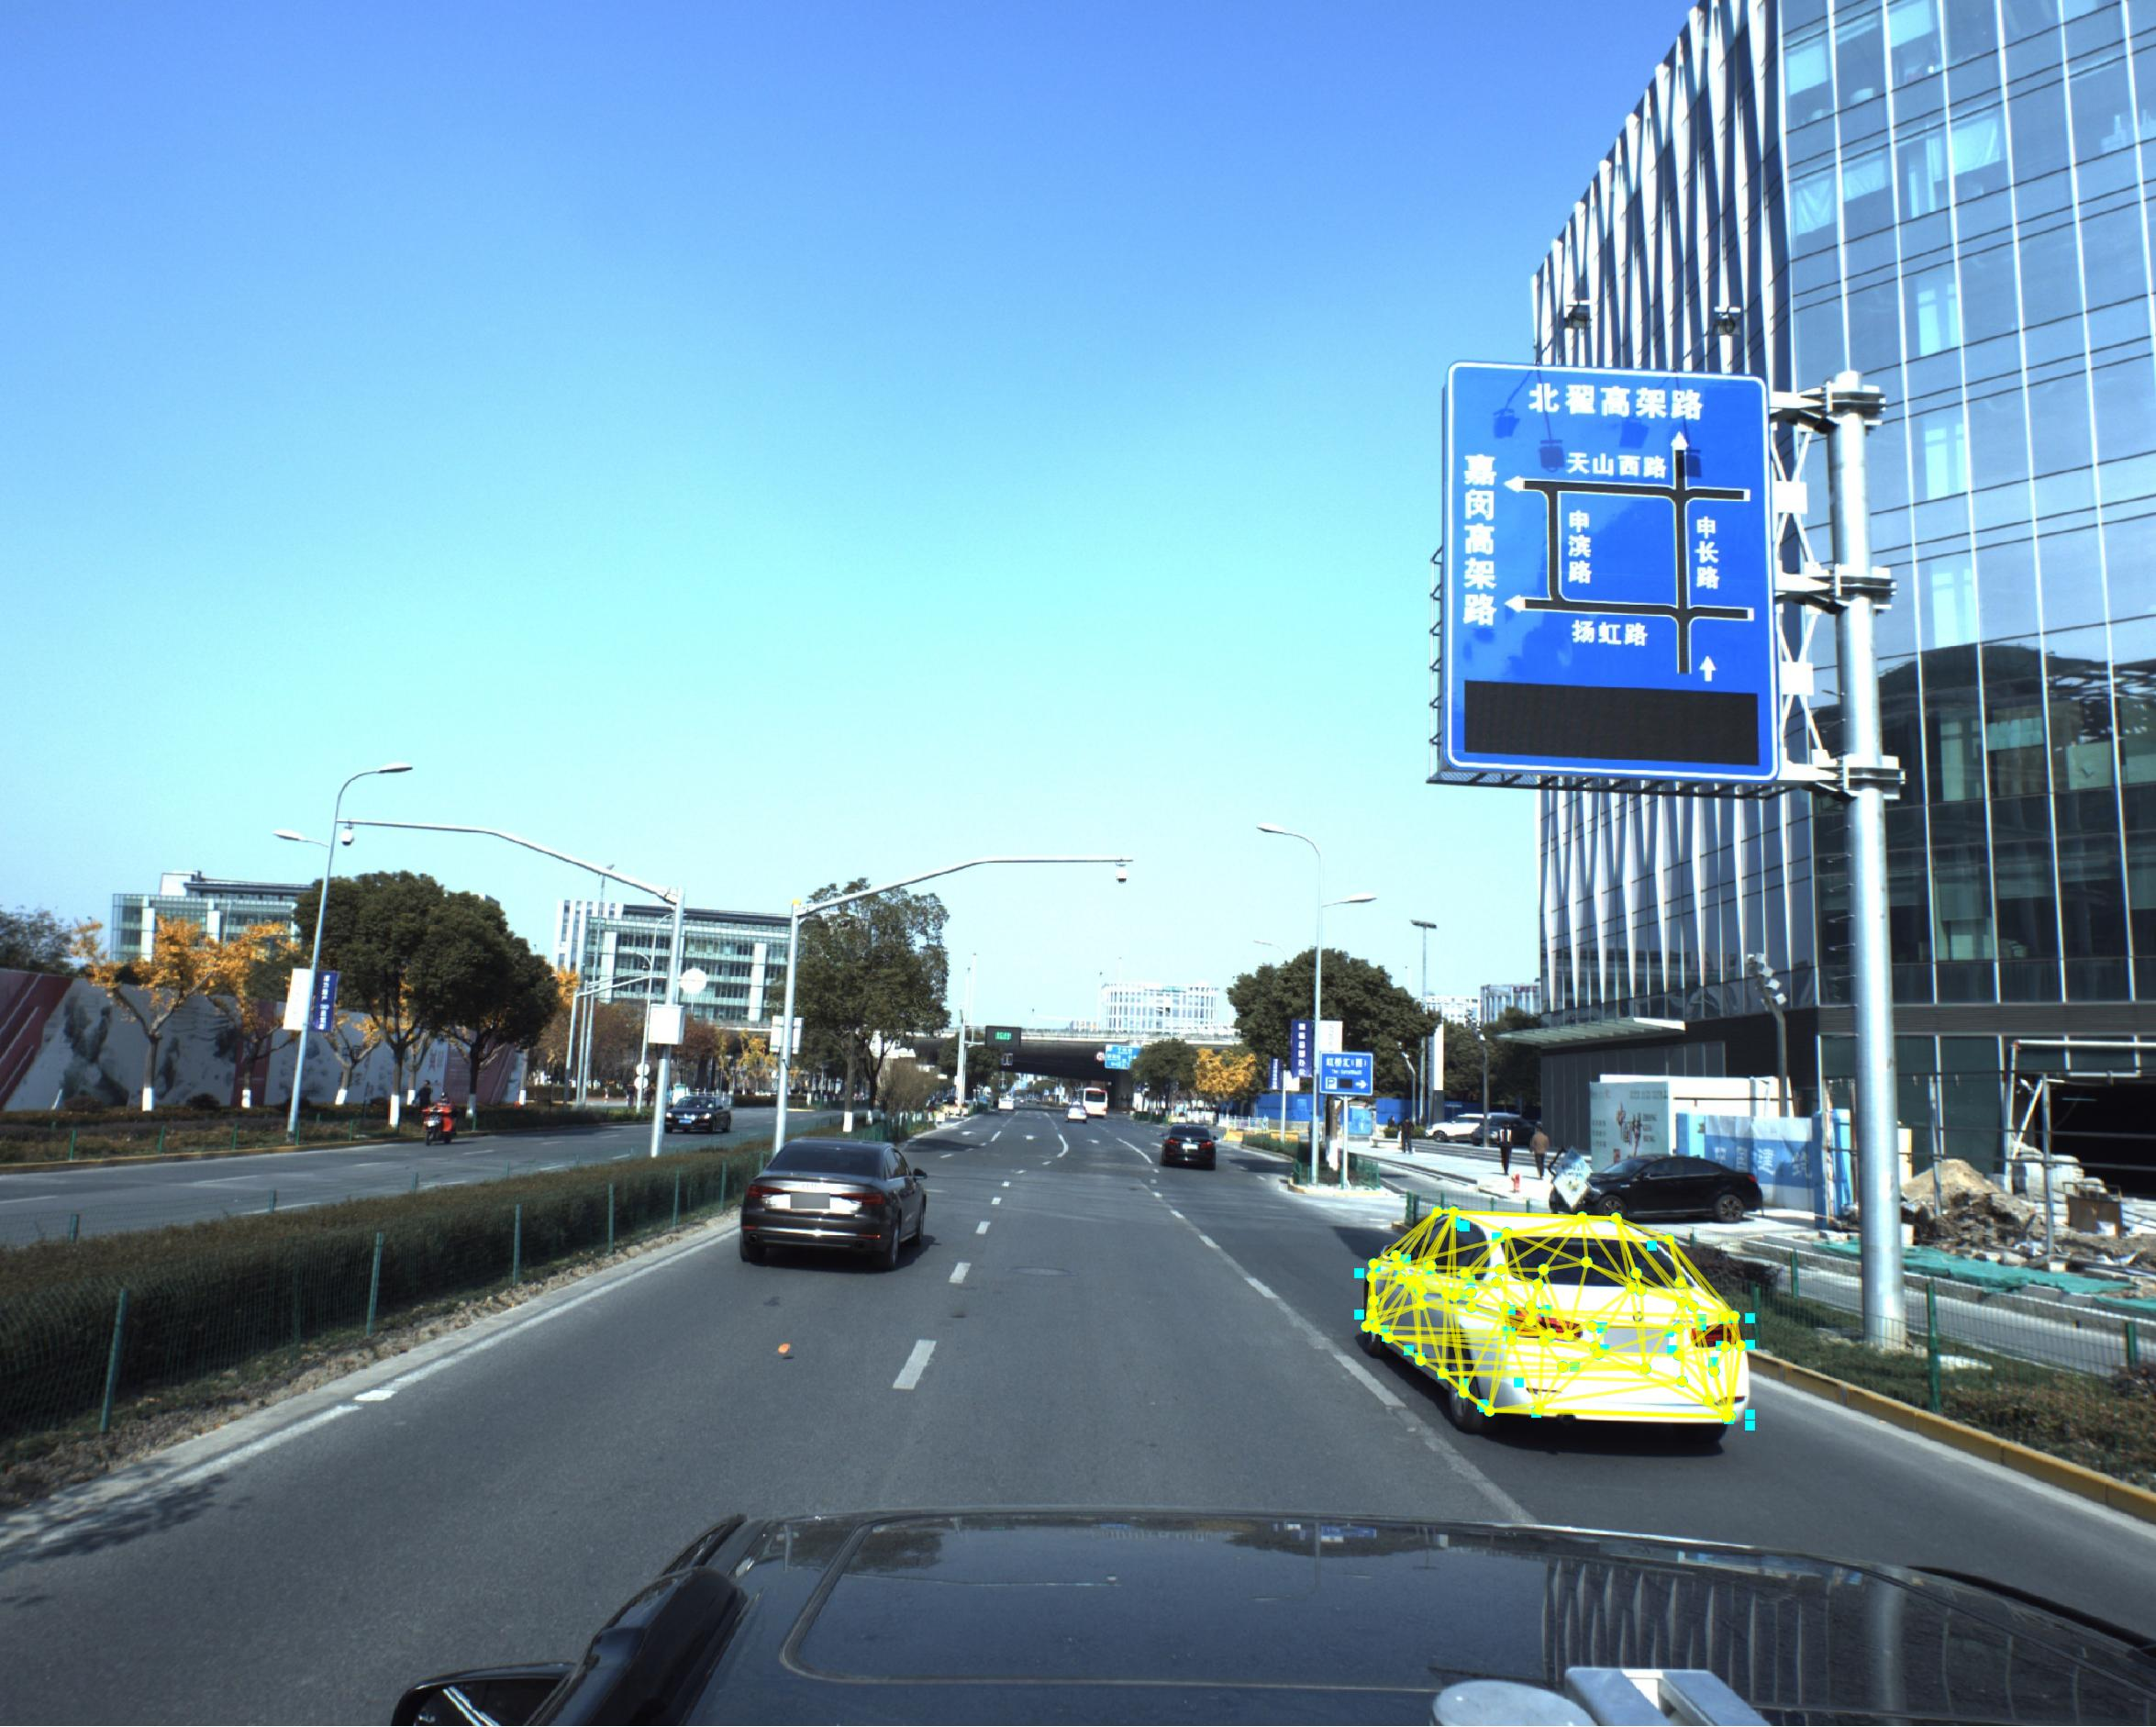}\\
			$\MR$ error: $0.51^{\circ}$, $\vt$ error: $0.01$ \\
			$\subopt=1.35\ee{-9}$, time: $4174$ [s]\\
			$n_1 = 1152, m=364,037$\\
			$N=63$, \# outliers: $27$
			\end{minipage}
		&  \myhspace \hspace{-3mm}
			\begin{minipage}{\mpwfour}%
			\centering%
			\includegraphics[width=0.95\columnwidth]{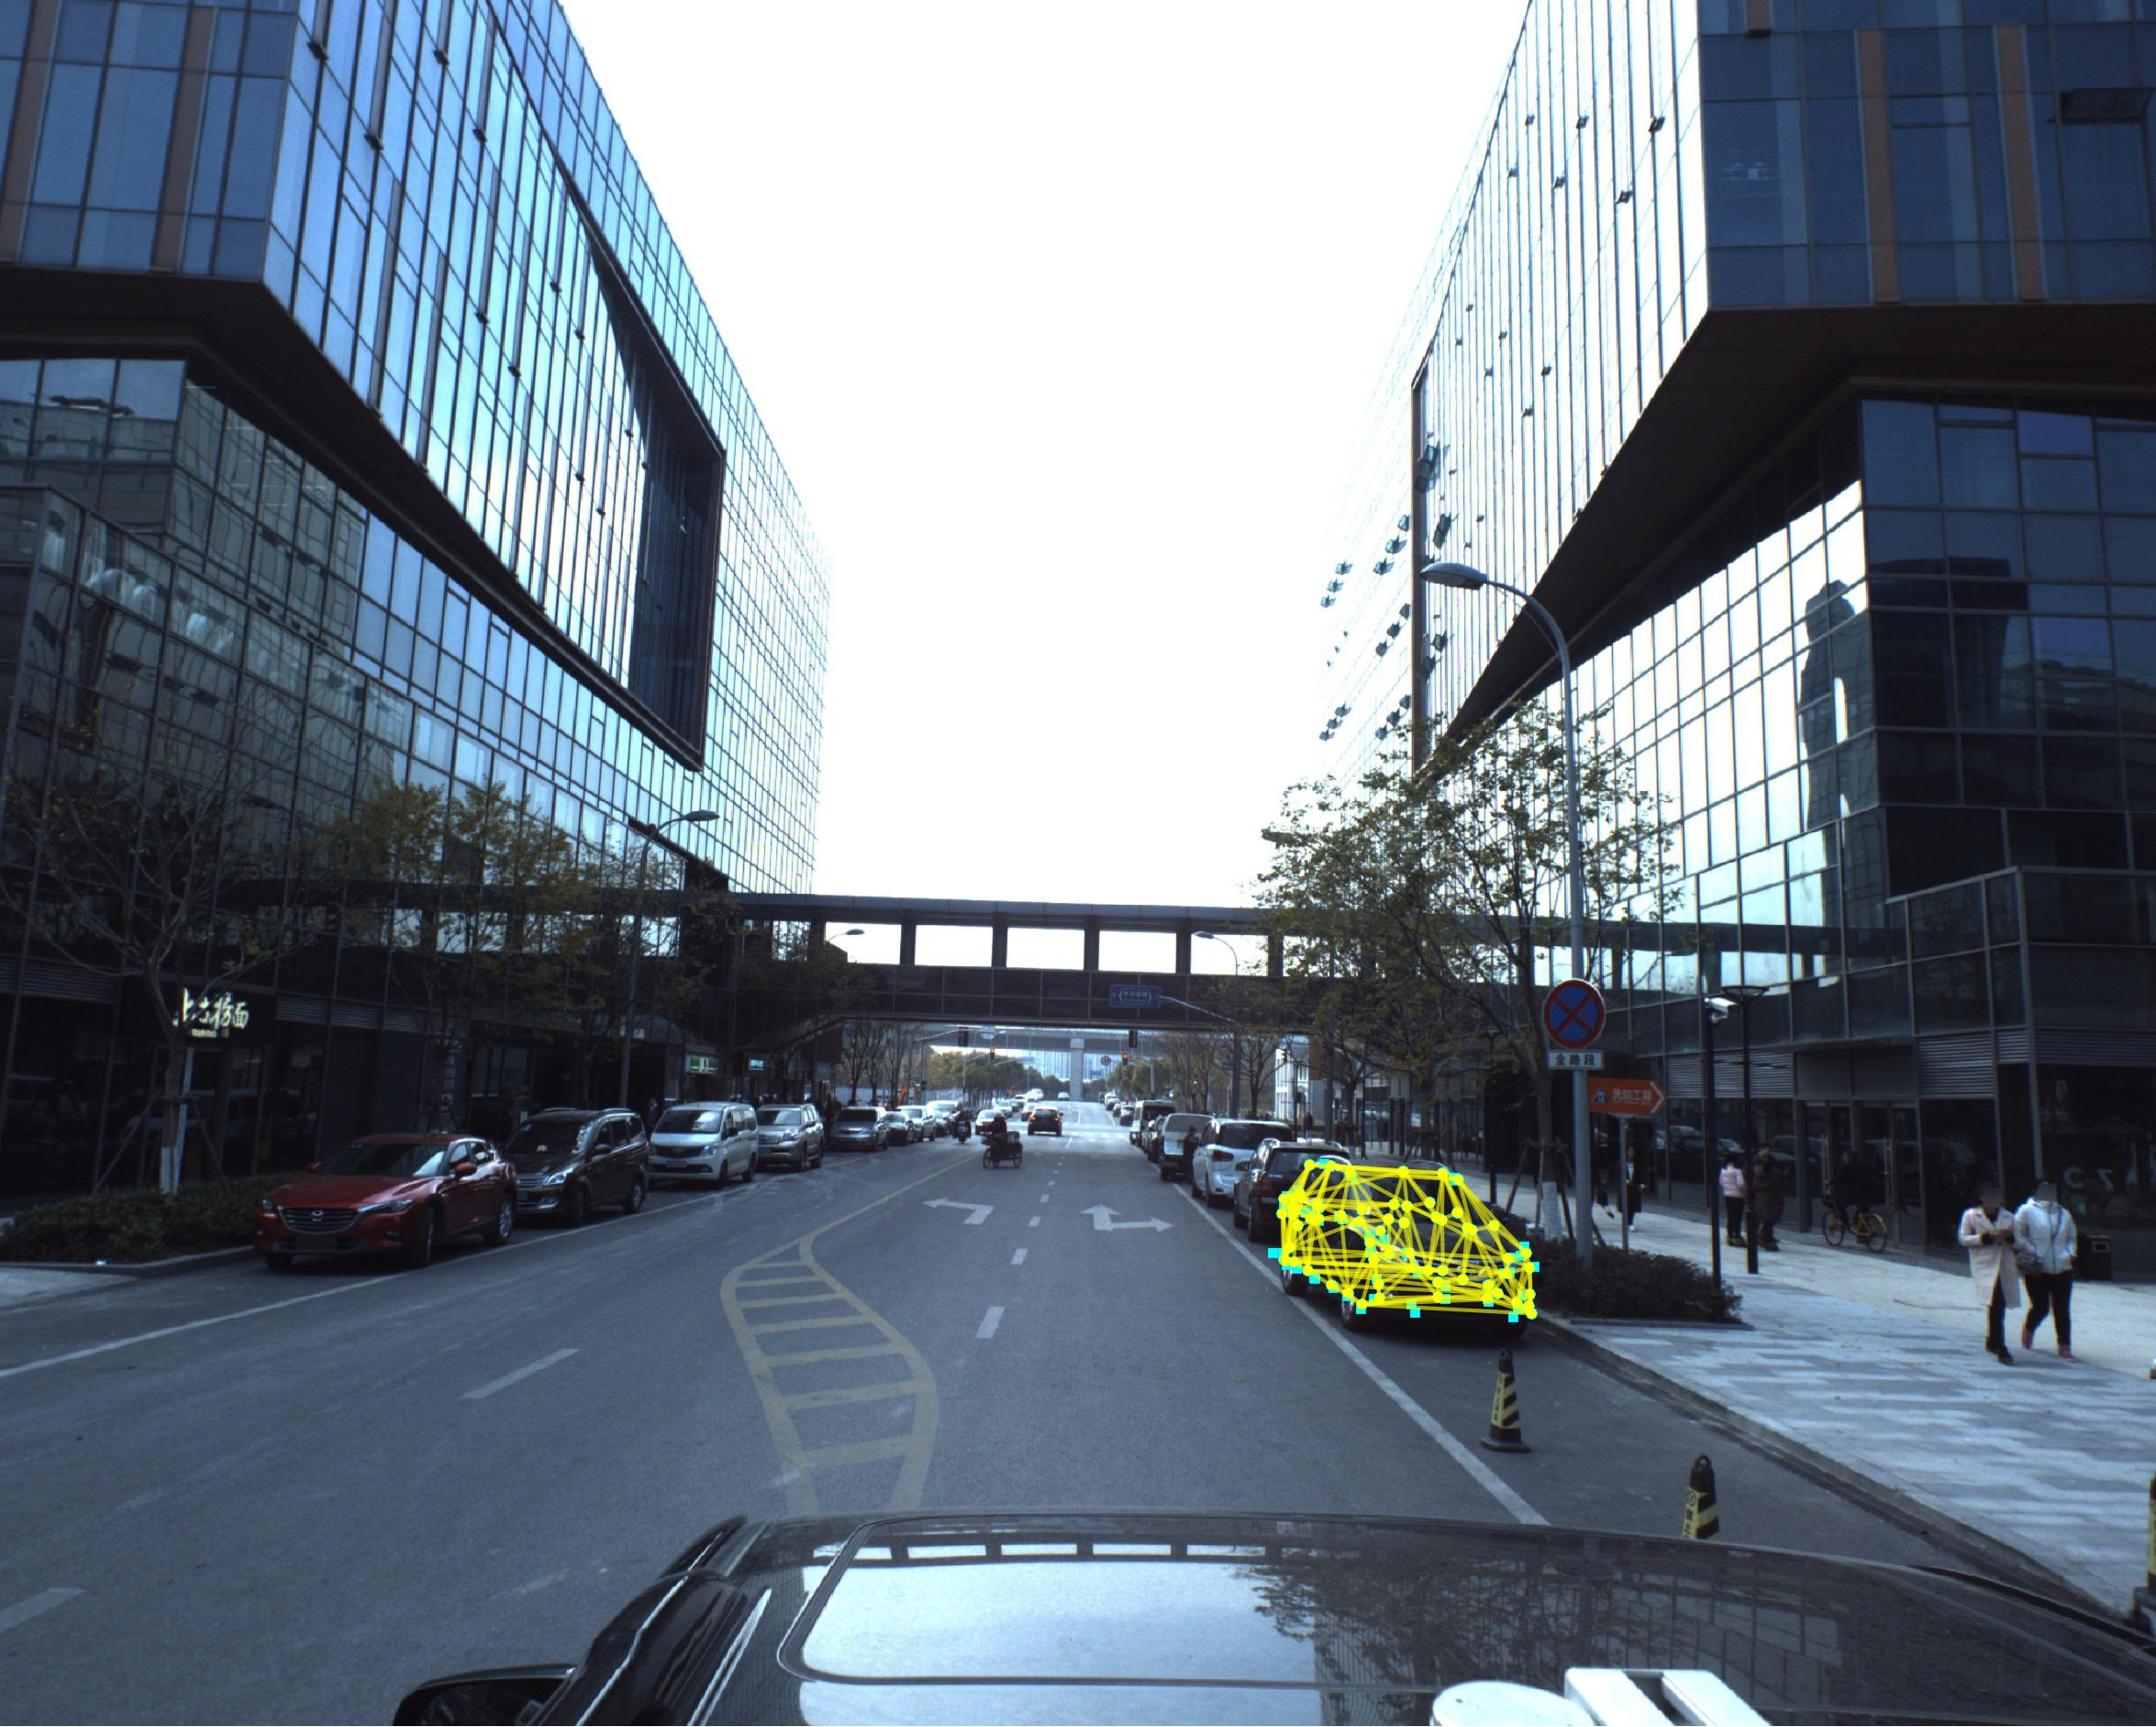}\\
			$\MR$ error: $1.07^{\circ}$, $\vt$ error: $0.02$ \\
			$\subopt=1.4\ee{-10}$, time: $4507$ [s]\\
			$n_1 = 1188, m=386,968$\\
			$N=65$, \# outliers: $30$
			\end{minipage}
		&  \myhspace \hspace{-3mm}
			\begin{minipage}{\mpwfour}%
			\centering%
			\includegraphics[width=0.95\columnwidth]{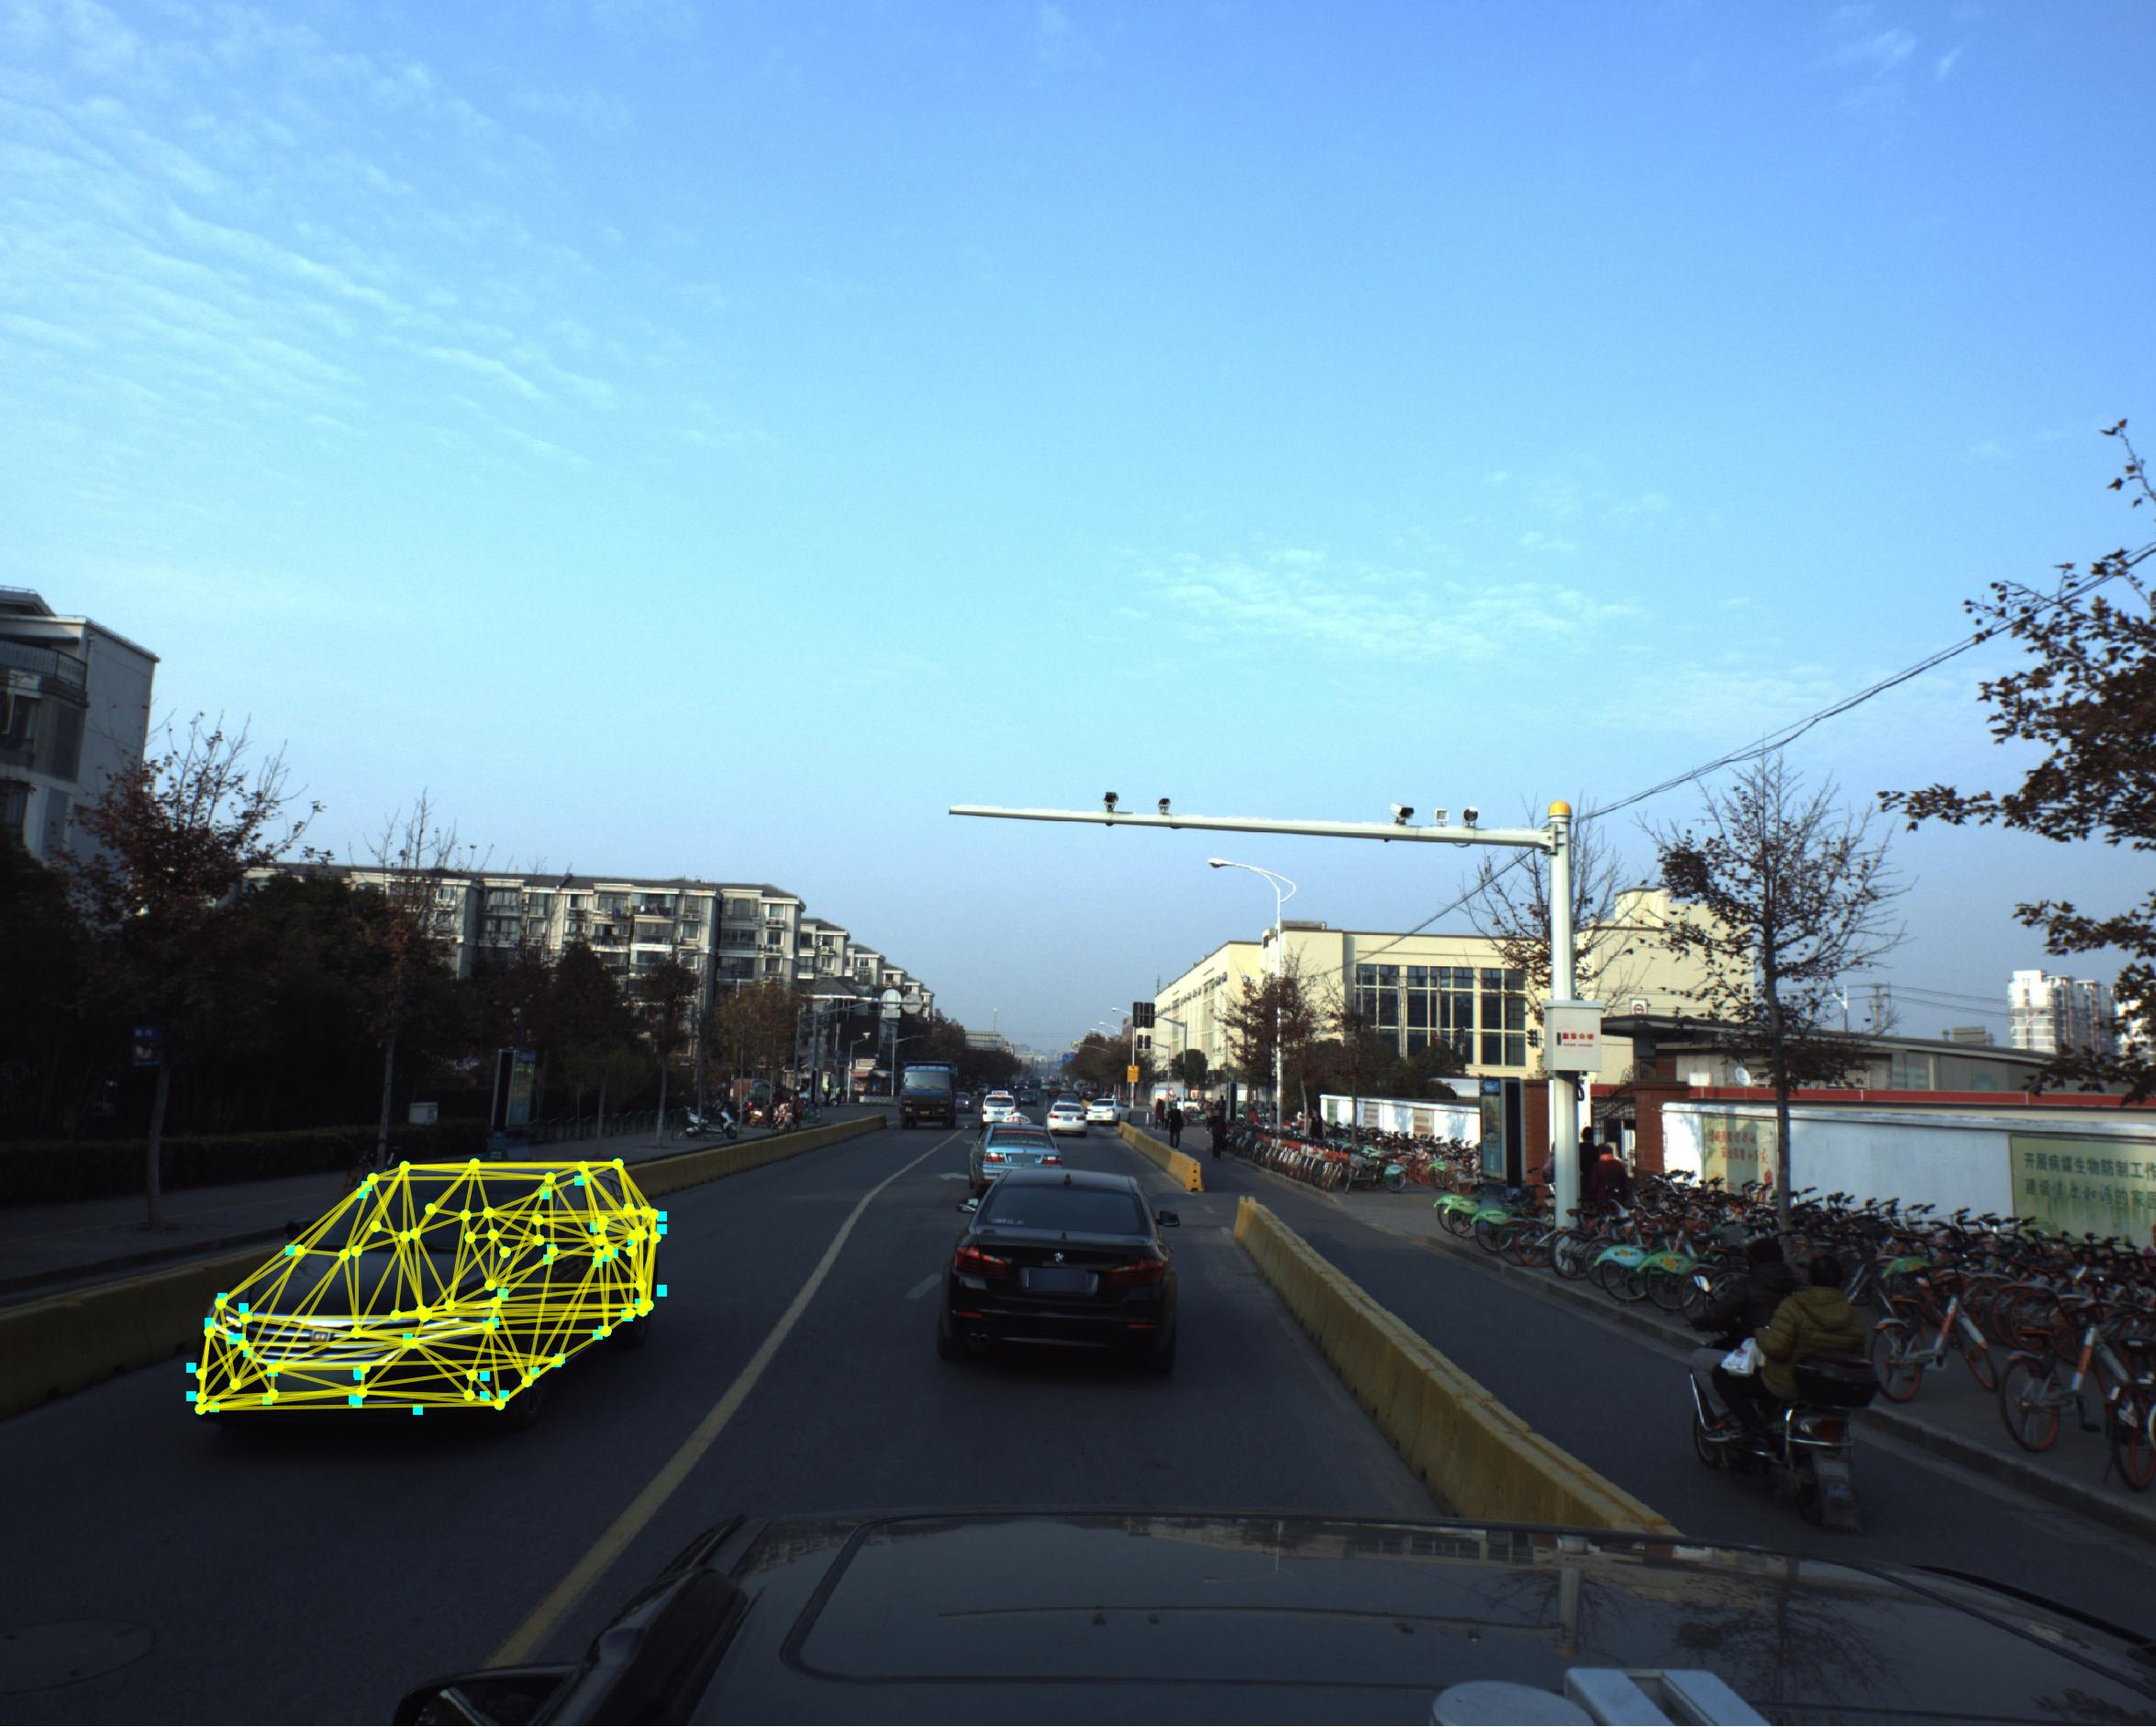}\\
			$\MR$ error: $1.74^{\circ}$, $\vt$ error: $0.03$ \\
			$\subopt=1.6\ee{-9}$, time: $4446$ [s]\\
			$n_1 = 1206, m=398,696$\\
			$N=66$, \# outliers: $30$
			\end{minipage}
			\vspace{1mm}
		\\

		%%%%%%%%%%%%%%%%%%%%%%%%%%%%%%%%%%%%%%%%%%%%%%%%%%%%%%%%%%%%%%%%%%%%%%%%%%%%%%%%%%%%%%%%%%%%%%%%%%%%%%%%%
		   \myhspace \hspace{-4mm}
			\begin{minipage}{\mpwfour}%
			\centering%
			\includegraphics[width=0.95\columnwidth]{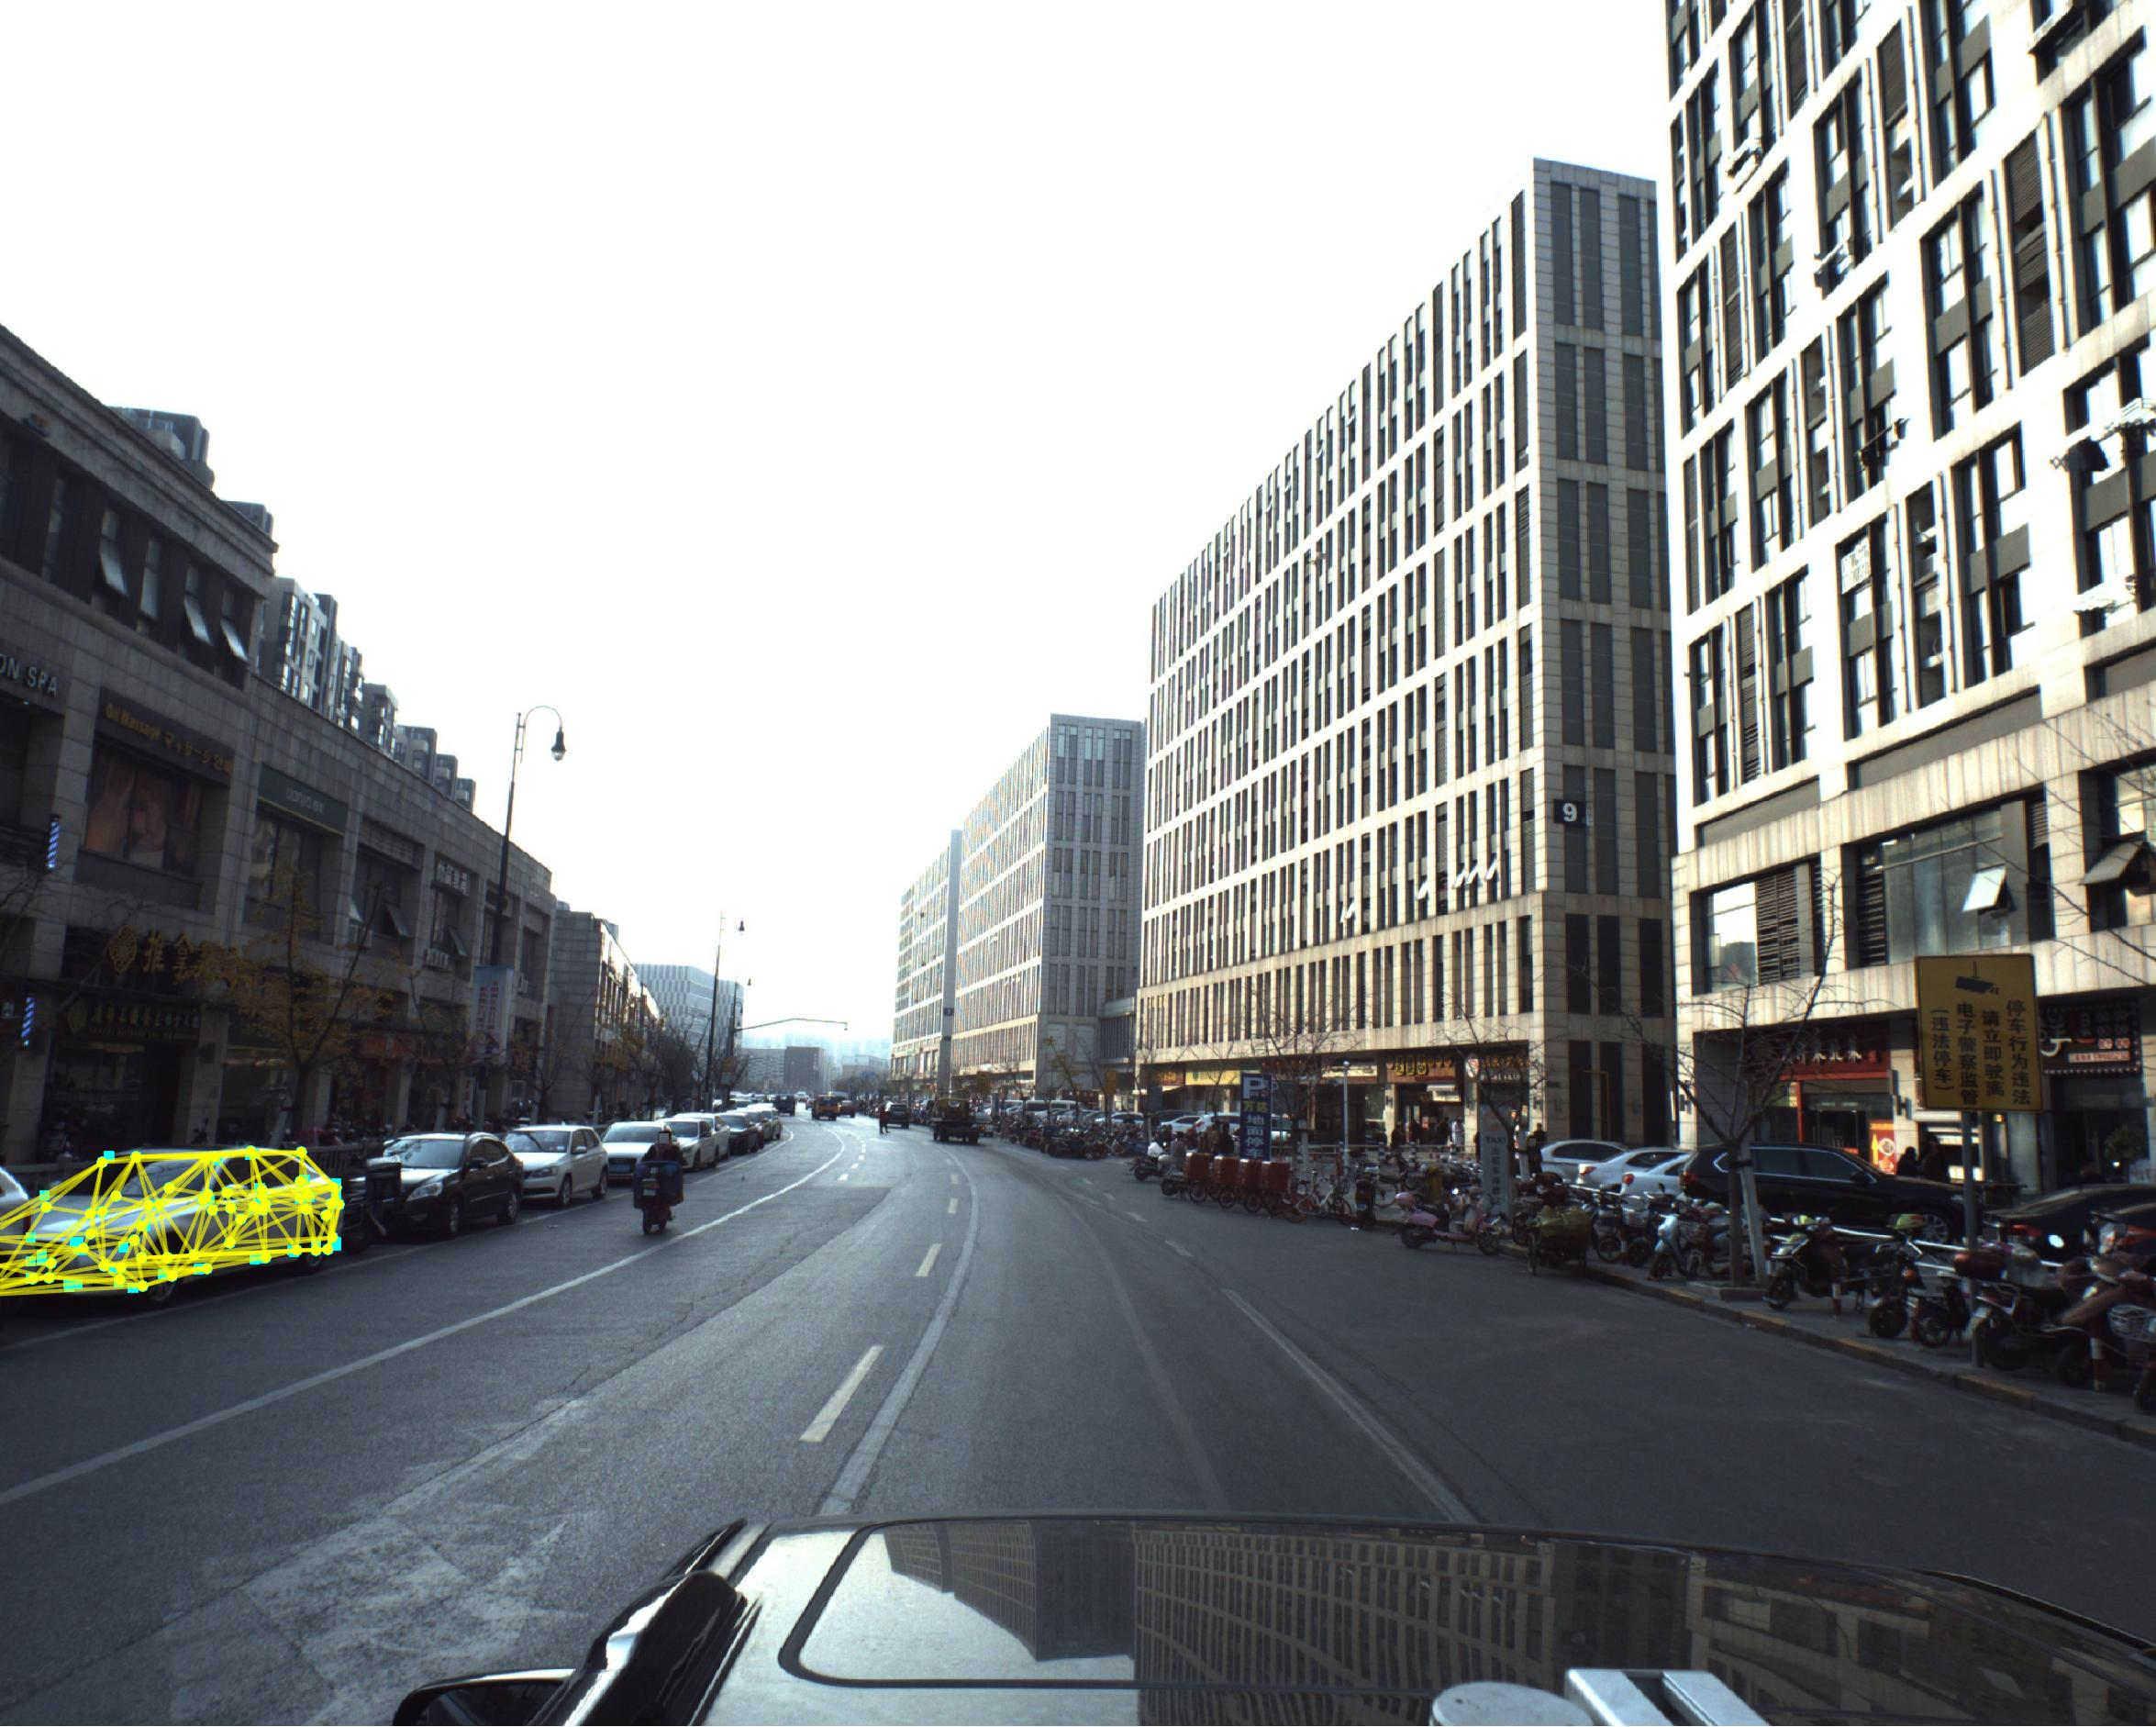} \\
			$\MR$ error: $2.02^{\circ}$, $\vt$ error: $0.04$ \\
			$\subopt=5.6\ee{-10}$, time: $4096$ [s] \\
			$n_1 = 1116, m=341,806$\\
			$N=61$, \# outliers: $29$
			\end{minipage}
		&  \myhspace \hspace{-3mm}
			\begin{minipage}{\mpwfour}%
			\centering%
			\includegraphics[width=0.95\columnwidth]{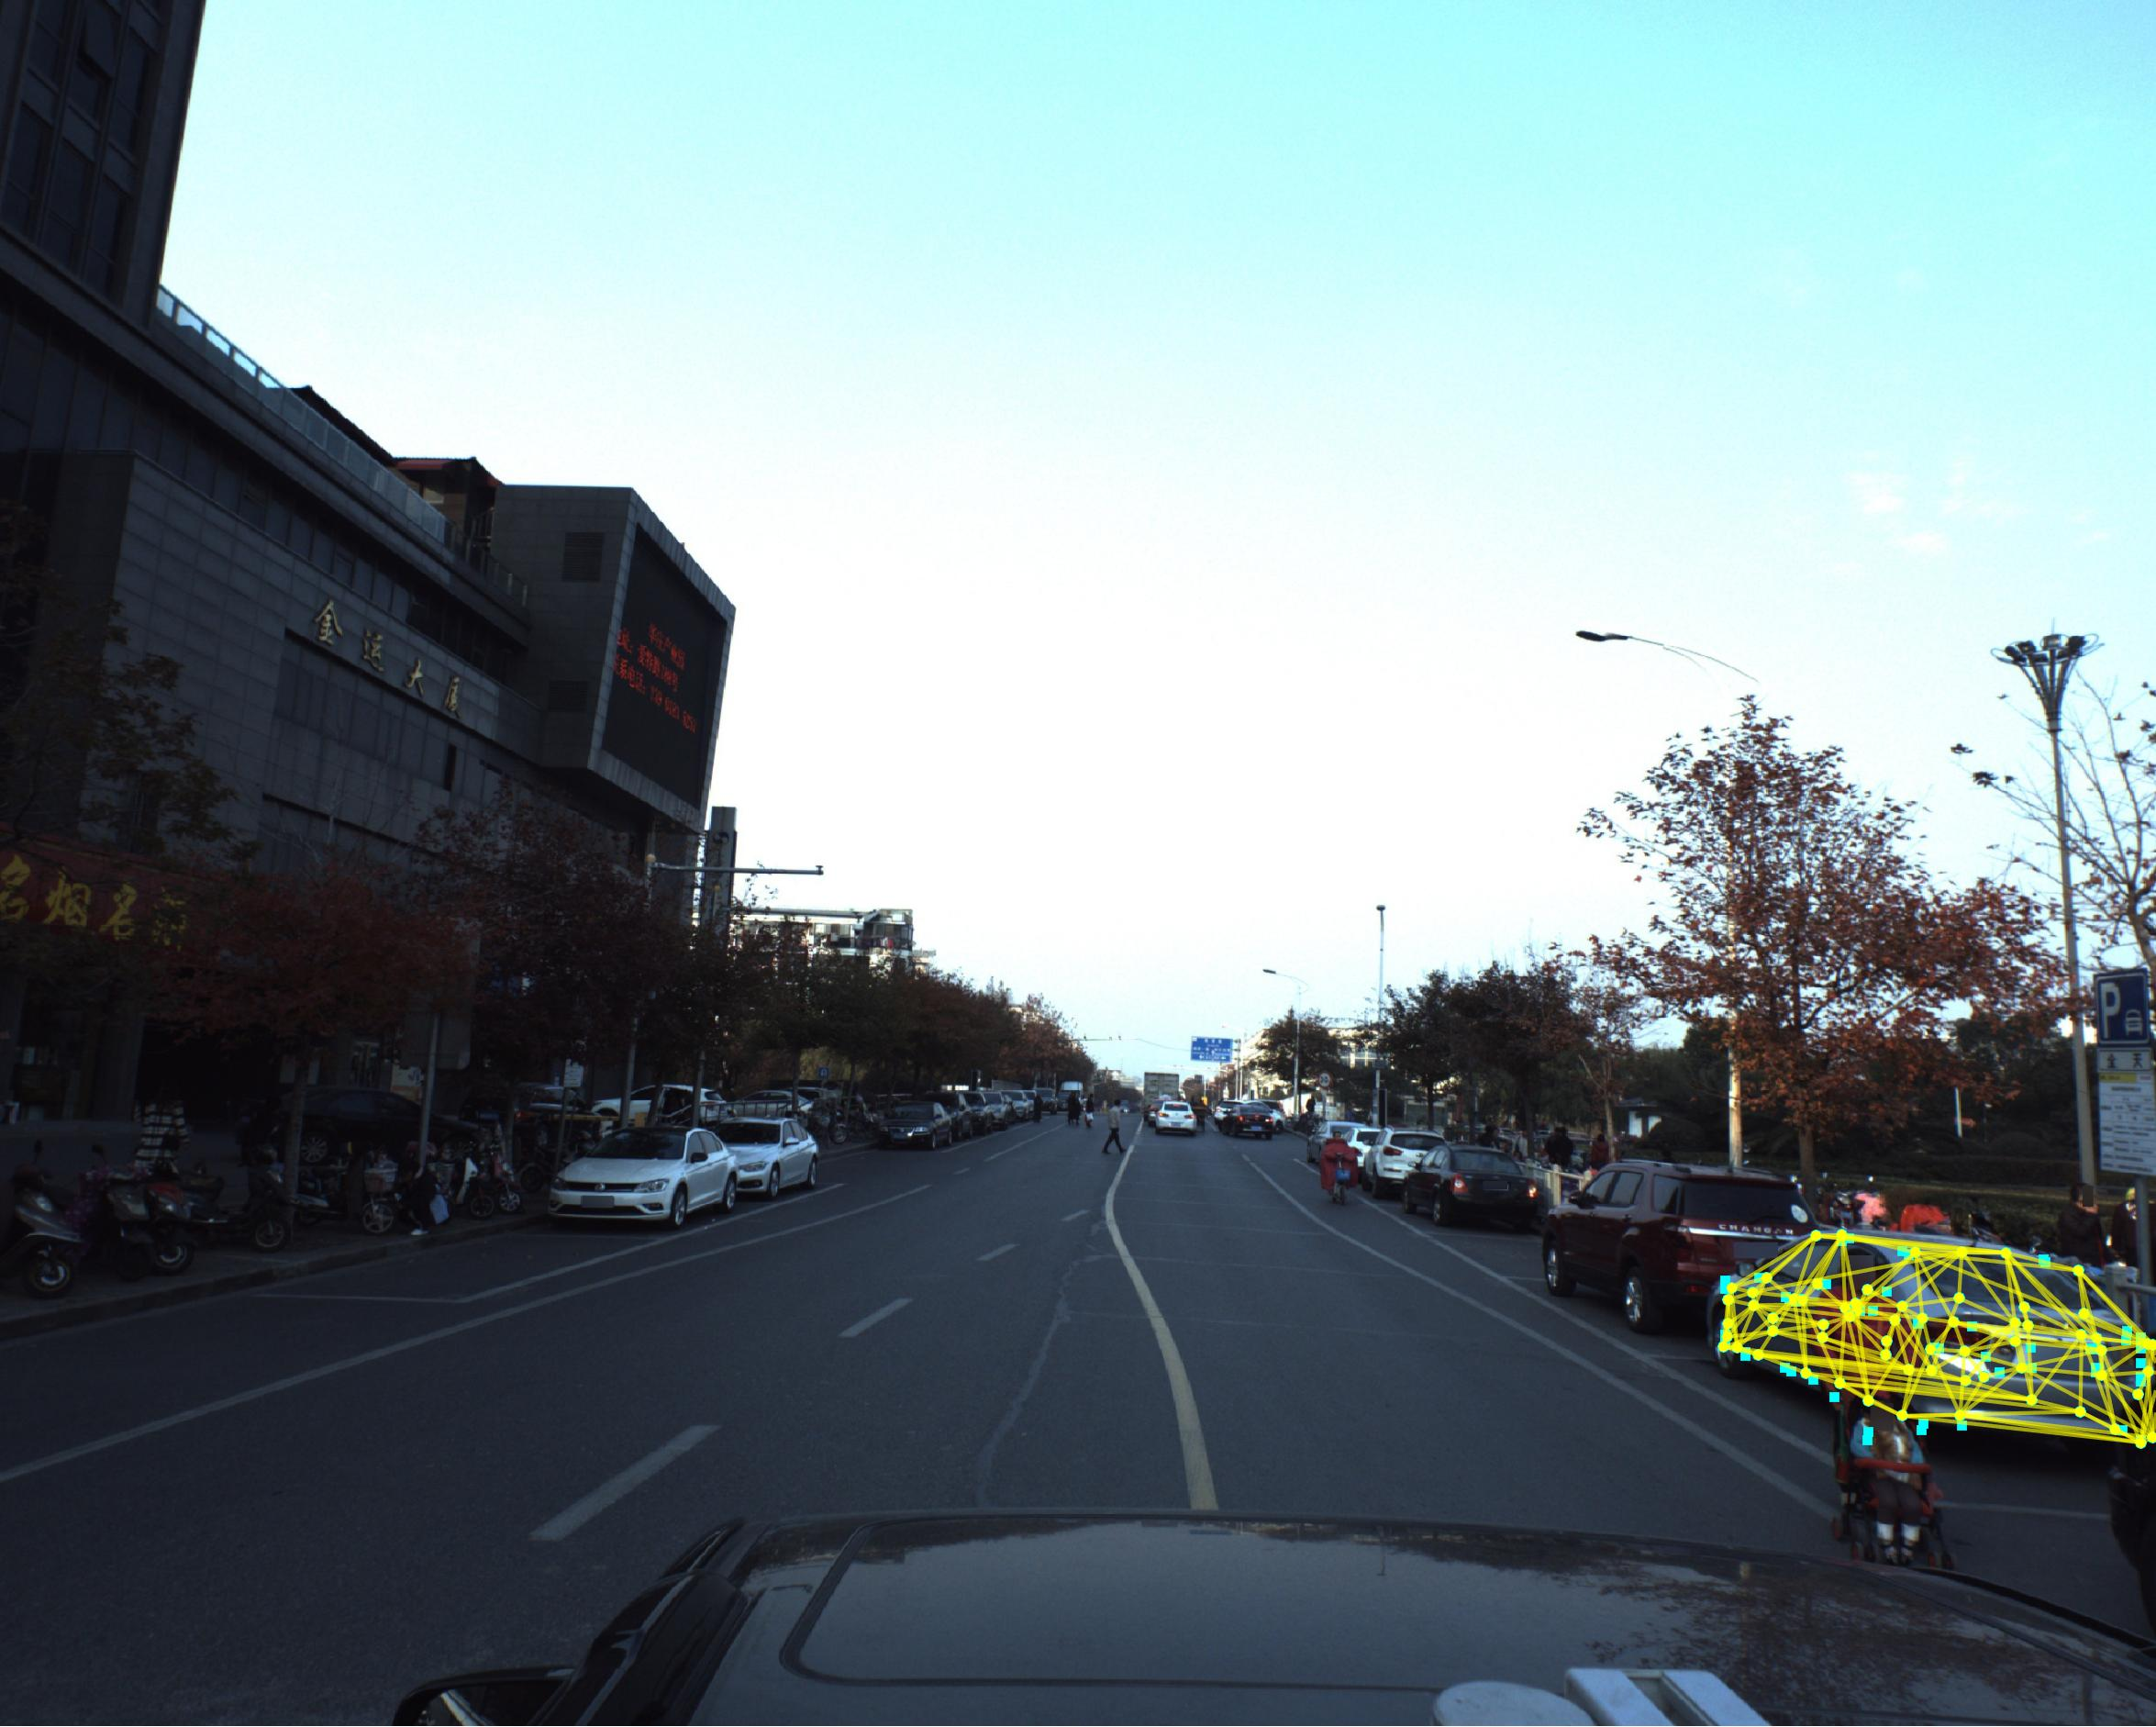}\\
			$\MR$ error: $2.48^{\circ}$, $\vt$ error: $0.05$ \\
			$\subopt=1.9\ee{-5}$, time: $7255$ [s]\\
			$n_1 = 1116, m=341,806$\\
			$N=61$, \# outliers: $25$
			\end{minipage}
		&  \myhspace \hspace{-3mm}
			\begin{minipage}{\mpwfour}%
			\centering%
			\includegraphics[width=0.95\columnwidth]{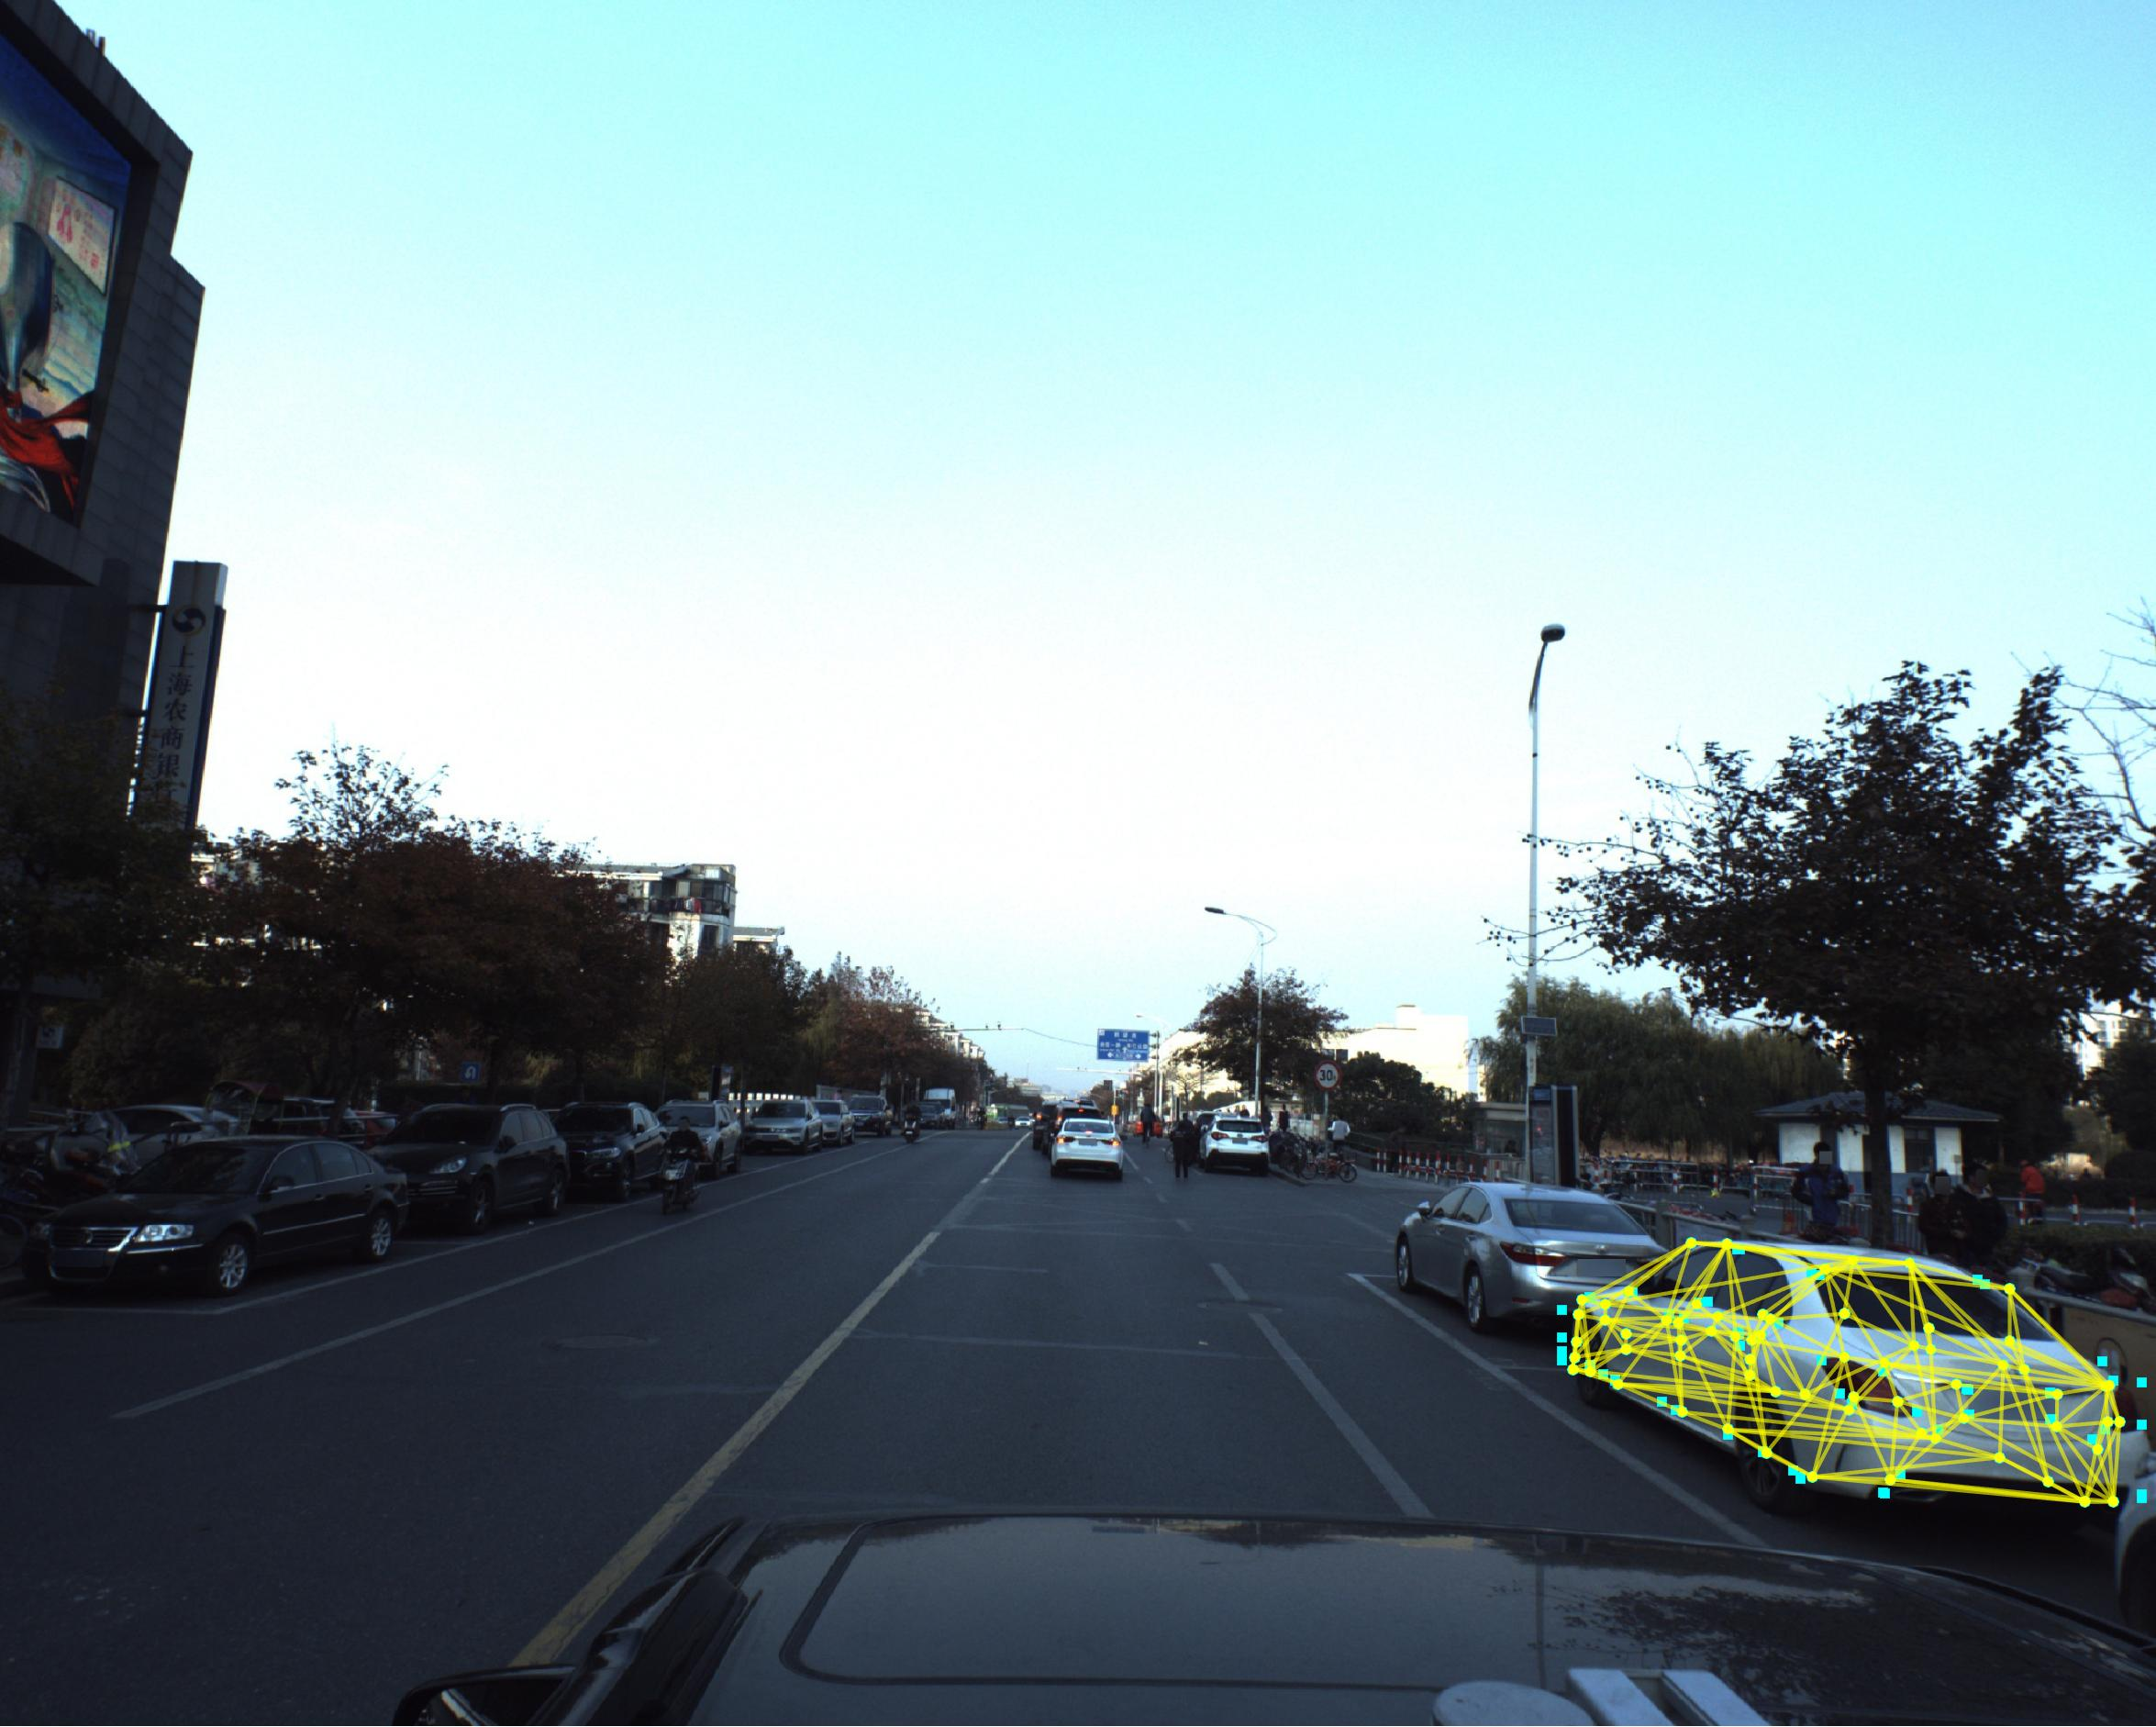}\\
			$\MR$ error: $1.89^{\circ}$, $\vt$ error: $0.05$ \\
			$\subopt=2.0\ee{-7}$, time: $5277$ [s]\\
			$n_1 = 1170, m=375,415$\\
			$N=64$, \# outliers: $26$
			\end{minipage}
		&  \myhspace \hspace{-3mm}
			\begin{minipage}{\mpwfour}%
			\centering%
			\includegraphics[width=0.95\columnwidth]{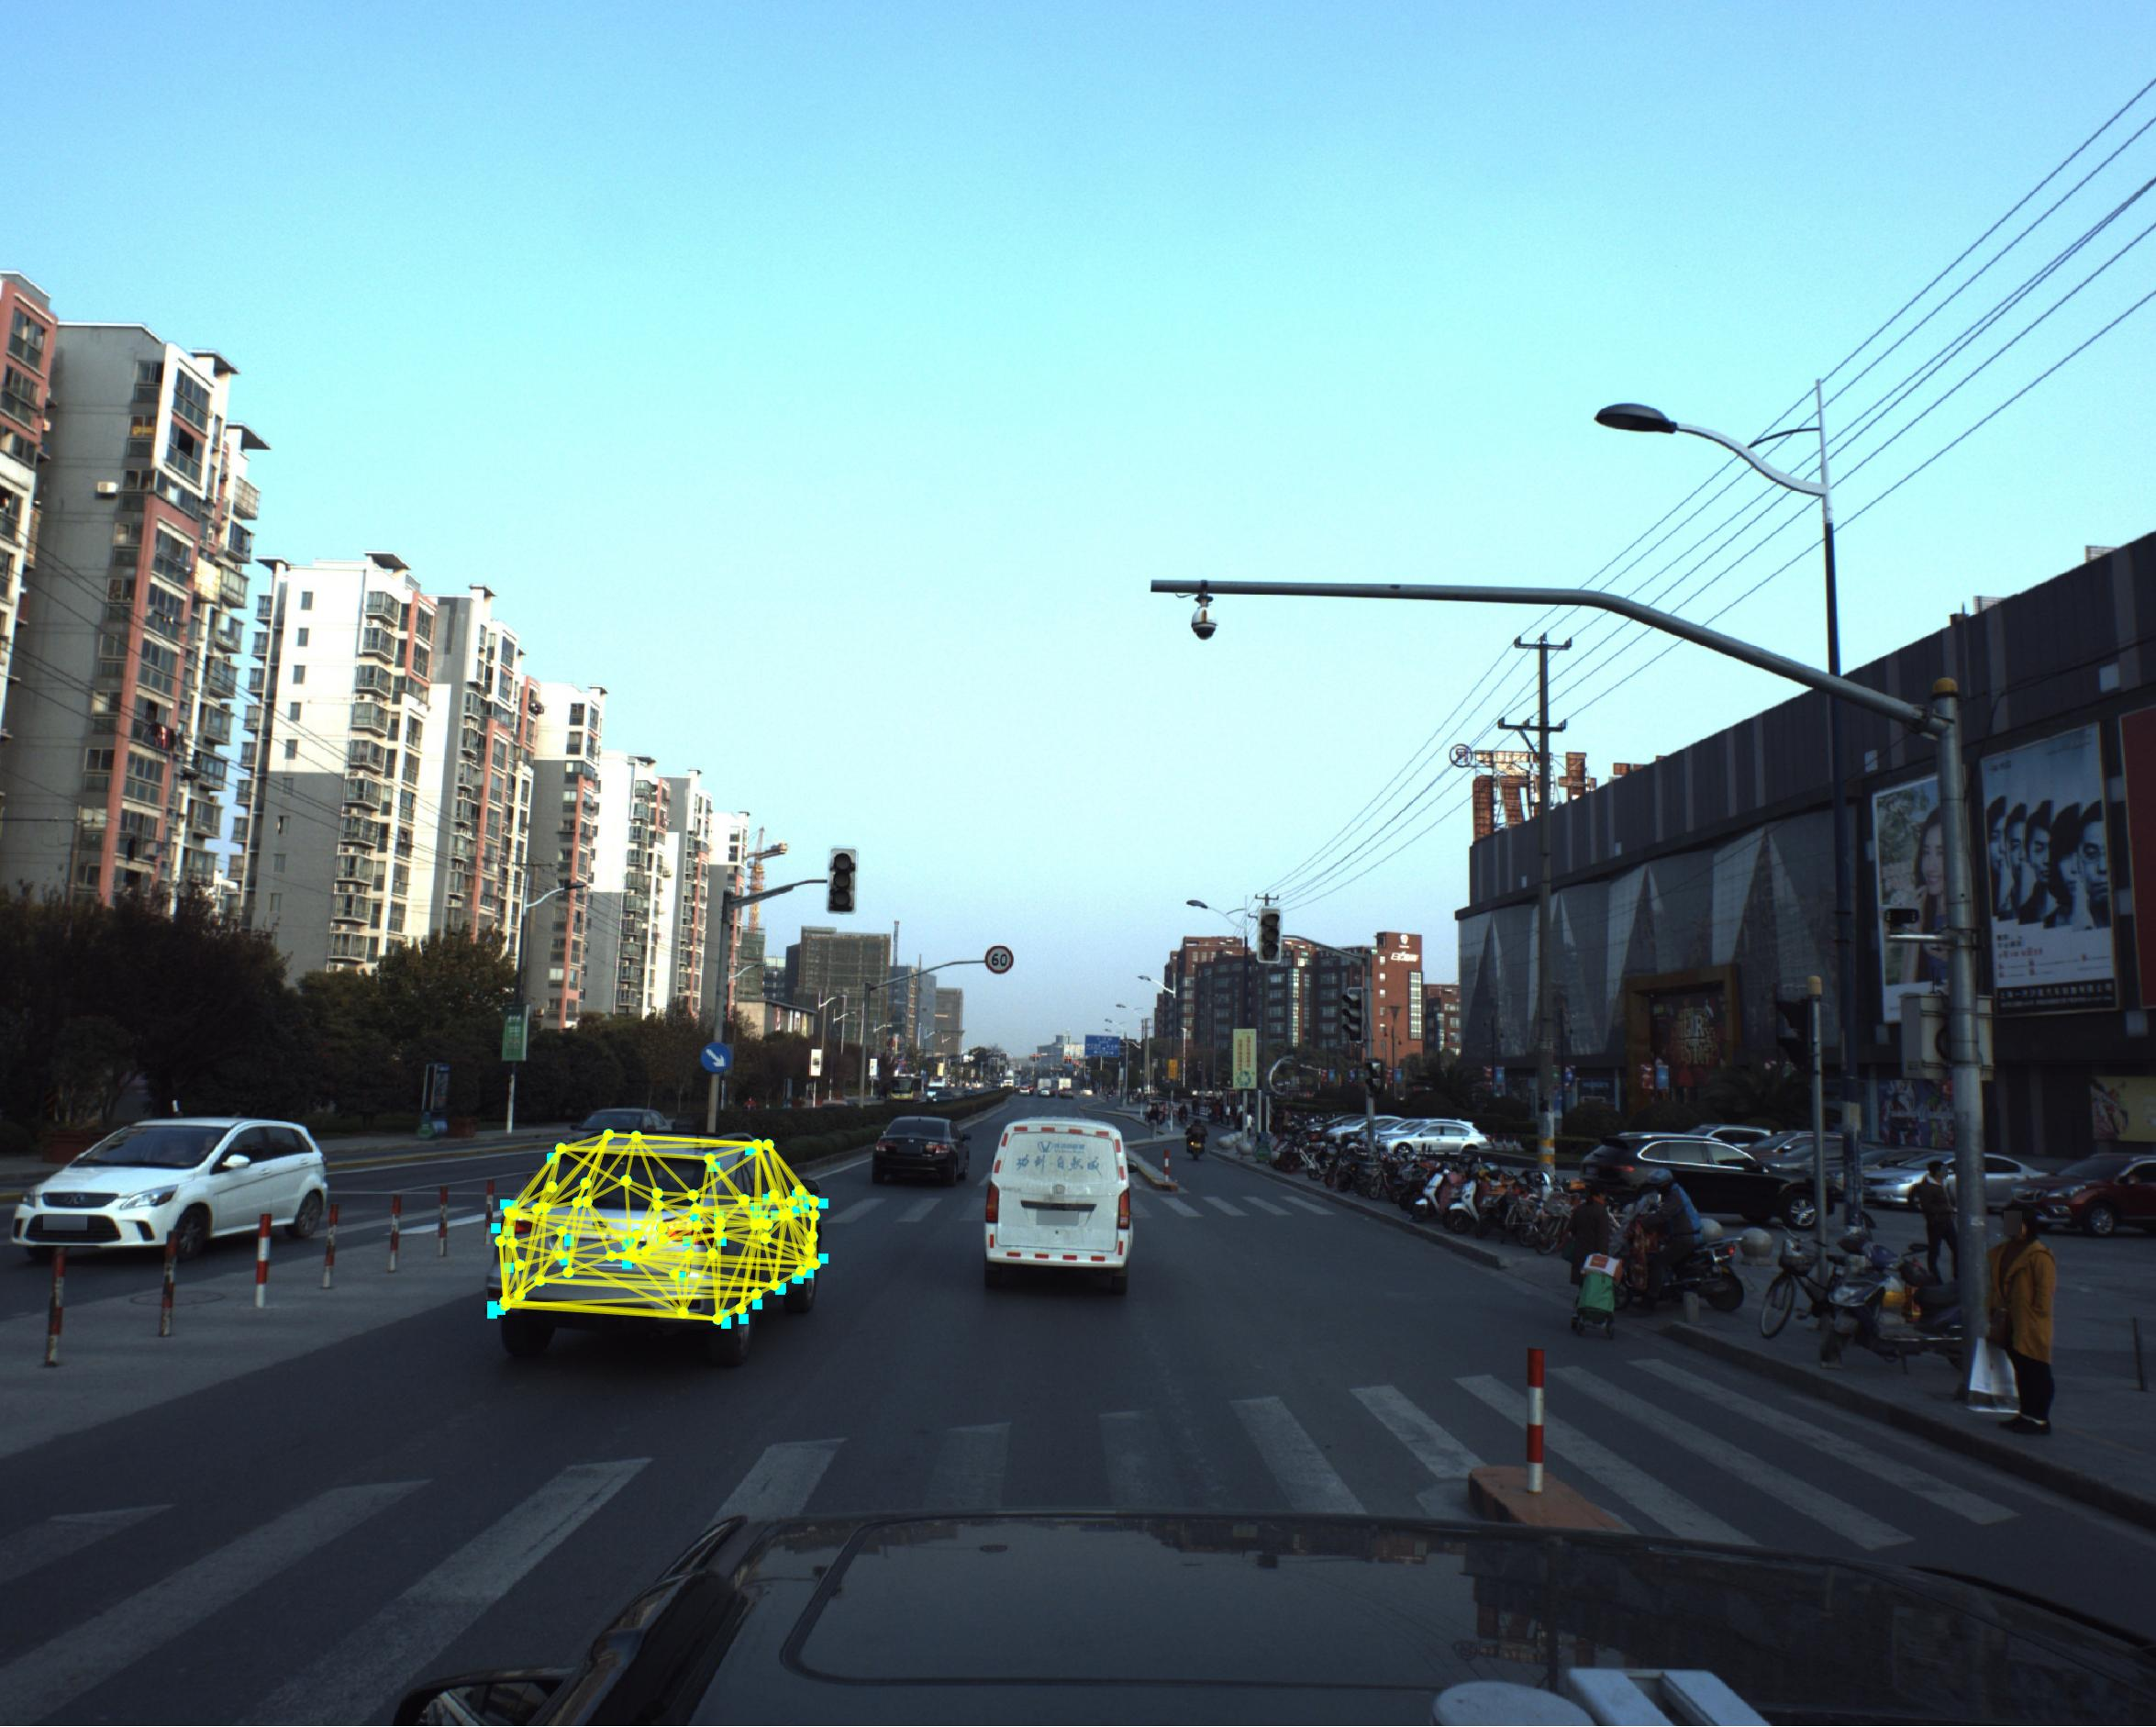}\\
			$\MR$ error: $1.83^{\circ}$, $\vt$ error: $0.04$ \\
			$\subopt=3.5\ee{-9}$, time: $3445$ [s]\\
			$n_1 = 1062, m=309,772$\\
			$N=58$, \# outliers: $23$
			\end{minipage}
			\vspace{1mm}
		\\

		\myhspace \hspace{-4mm}
			\begin{minipage}{\mpwfour}%
			\centering%
			\includegraphics[width=0.95\columnwidth]{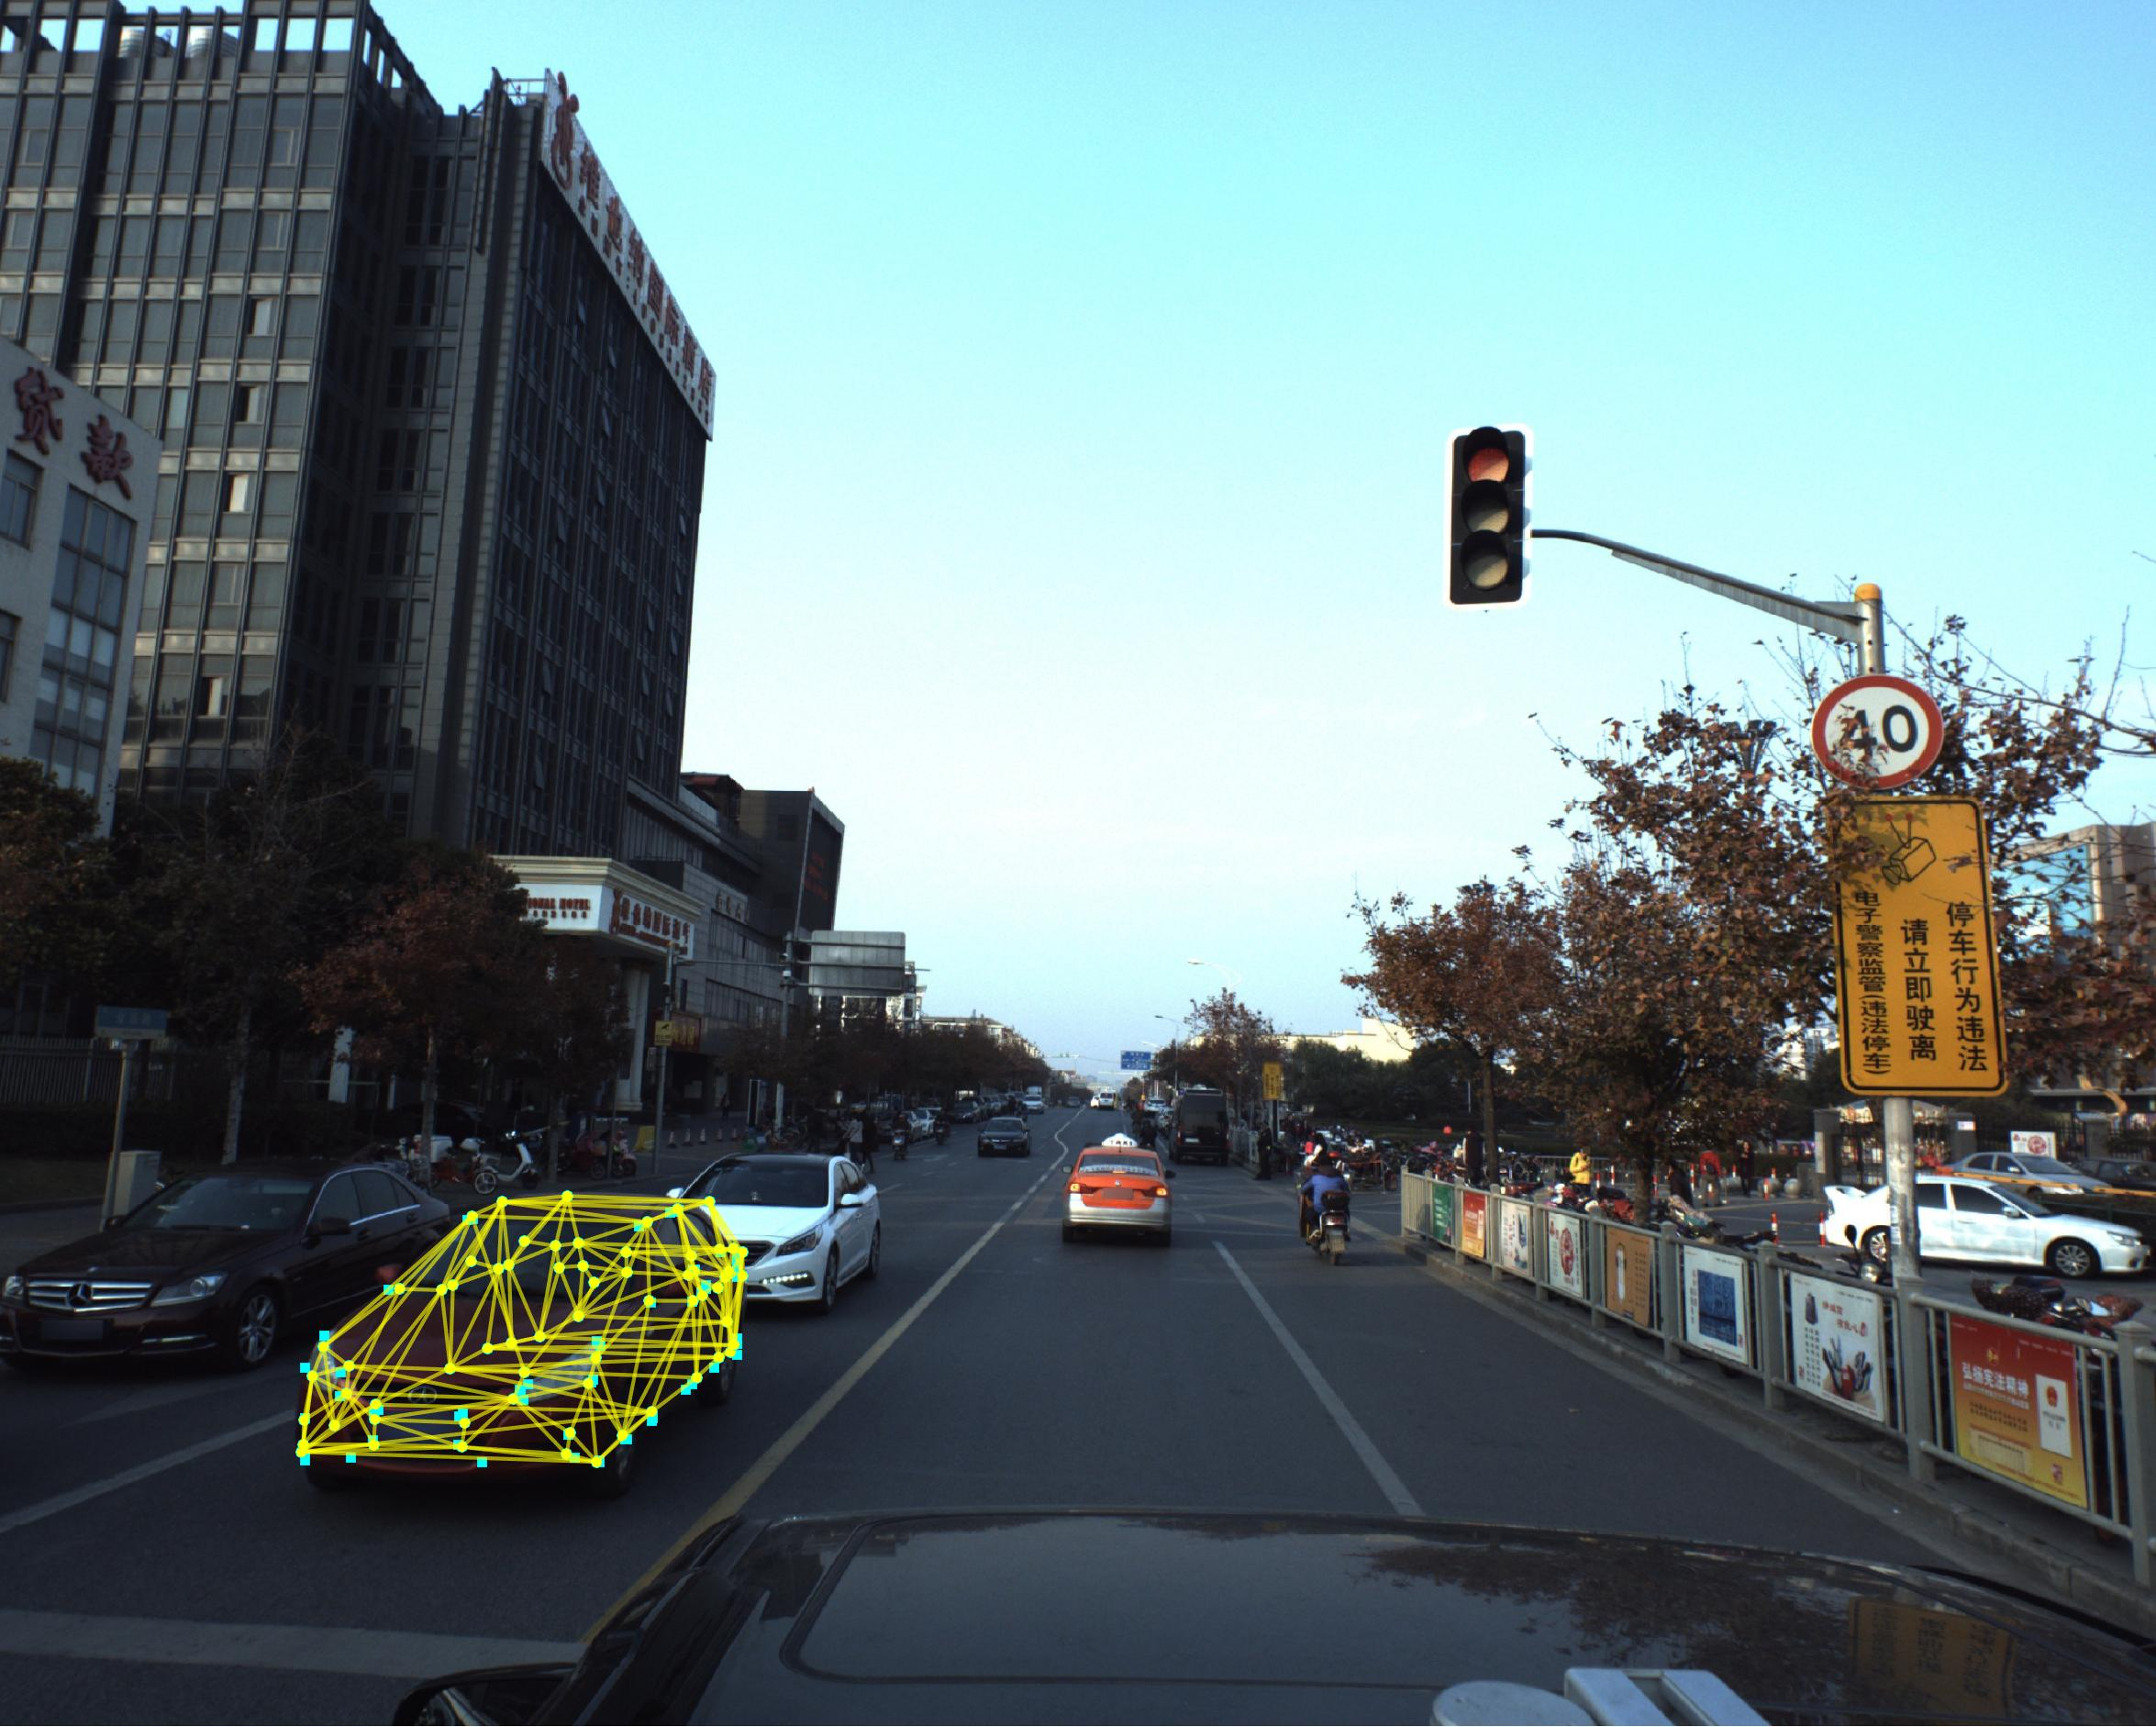}\\
			$\MR$ error: $1.51^{\circ}$, $\vt$ error: $0.03$ \\
			$\subopt=6.6\ee{-10}$, time: $4144$ [s]\\
			$n_1 = 1170, m=375,415$\\
			$N=64$, \# outliers: $29$
			\end{minipage}
		&  \myhspace \hspace{-3mm}
			\begin{minipage}{\mpwfour}%
			\centering%
			\includegraphics[width=0.95\columnwidth]{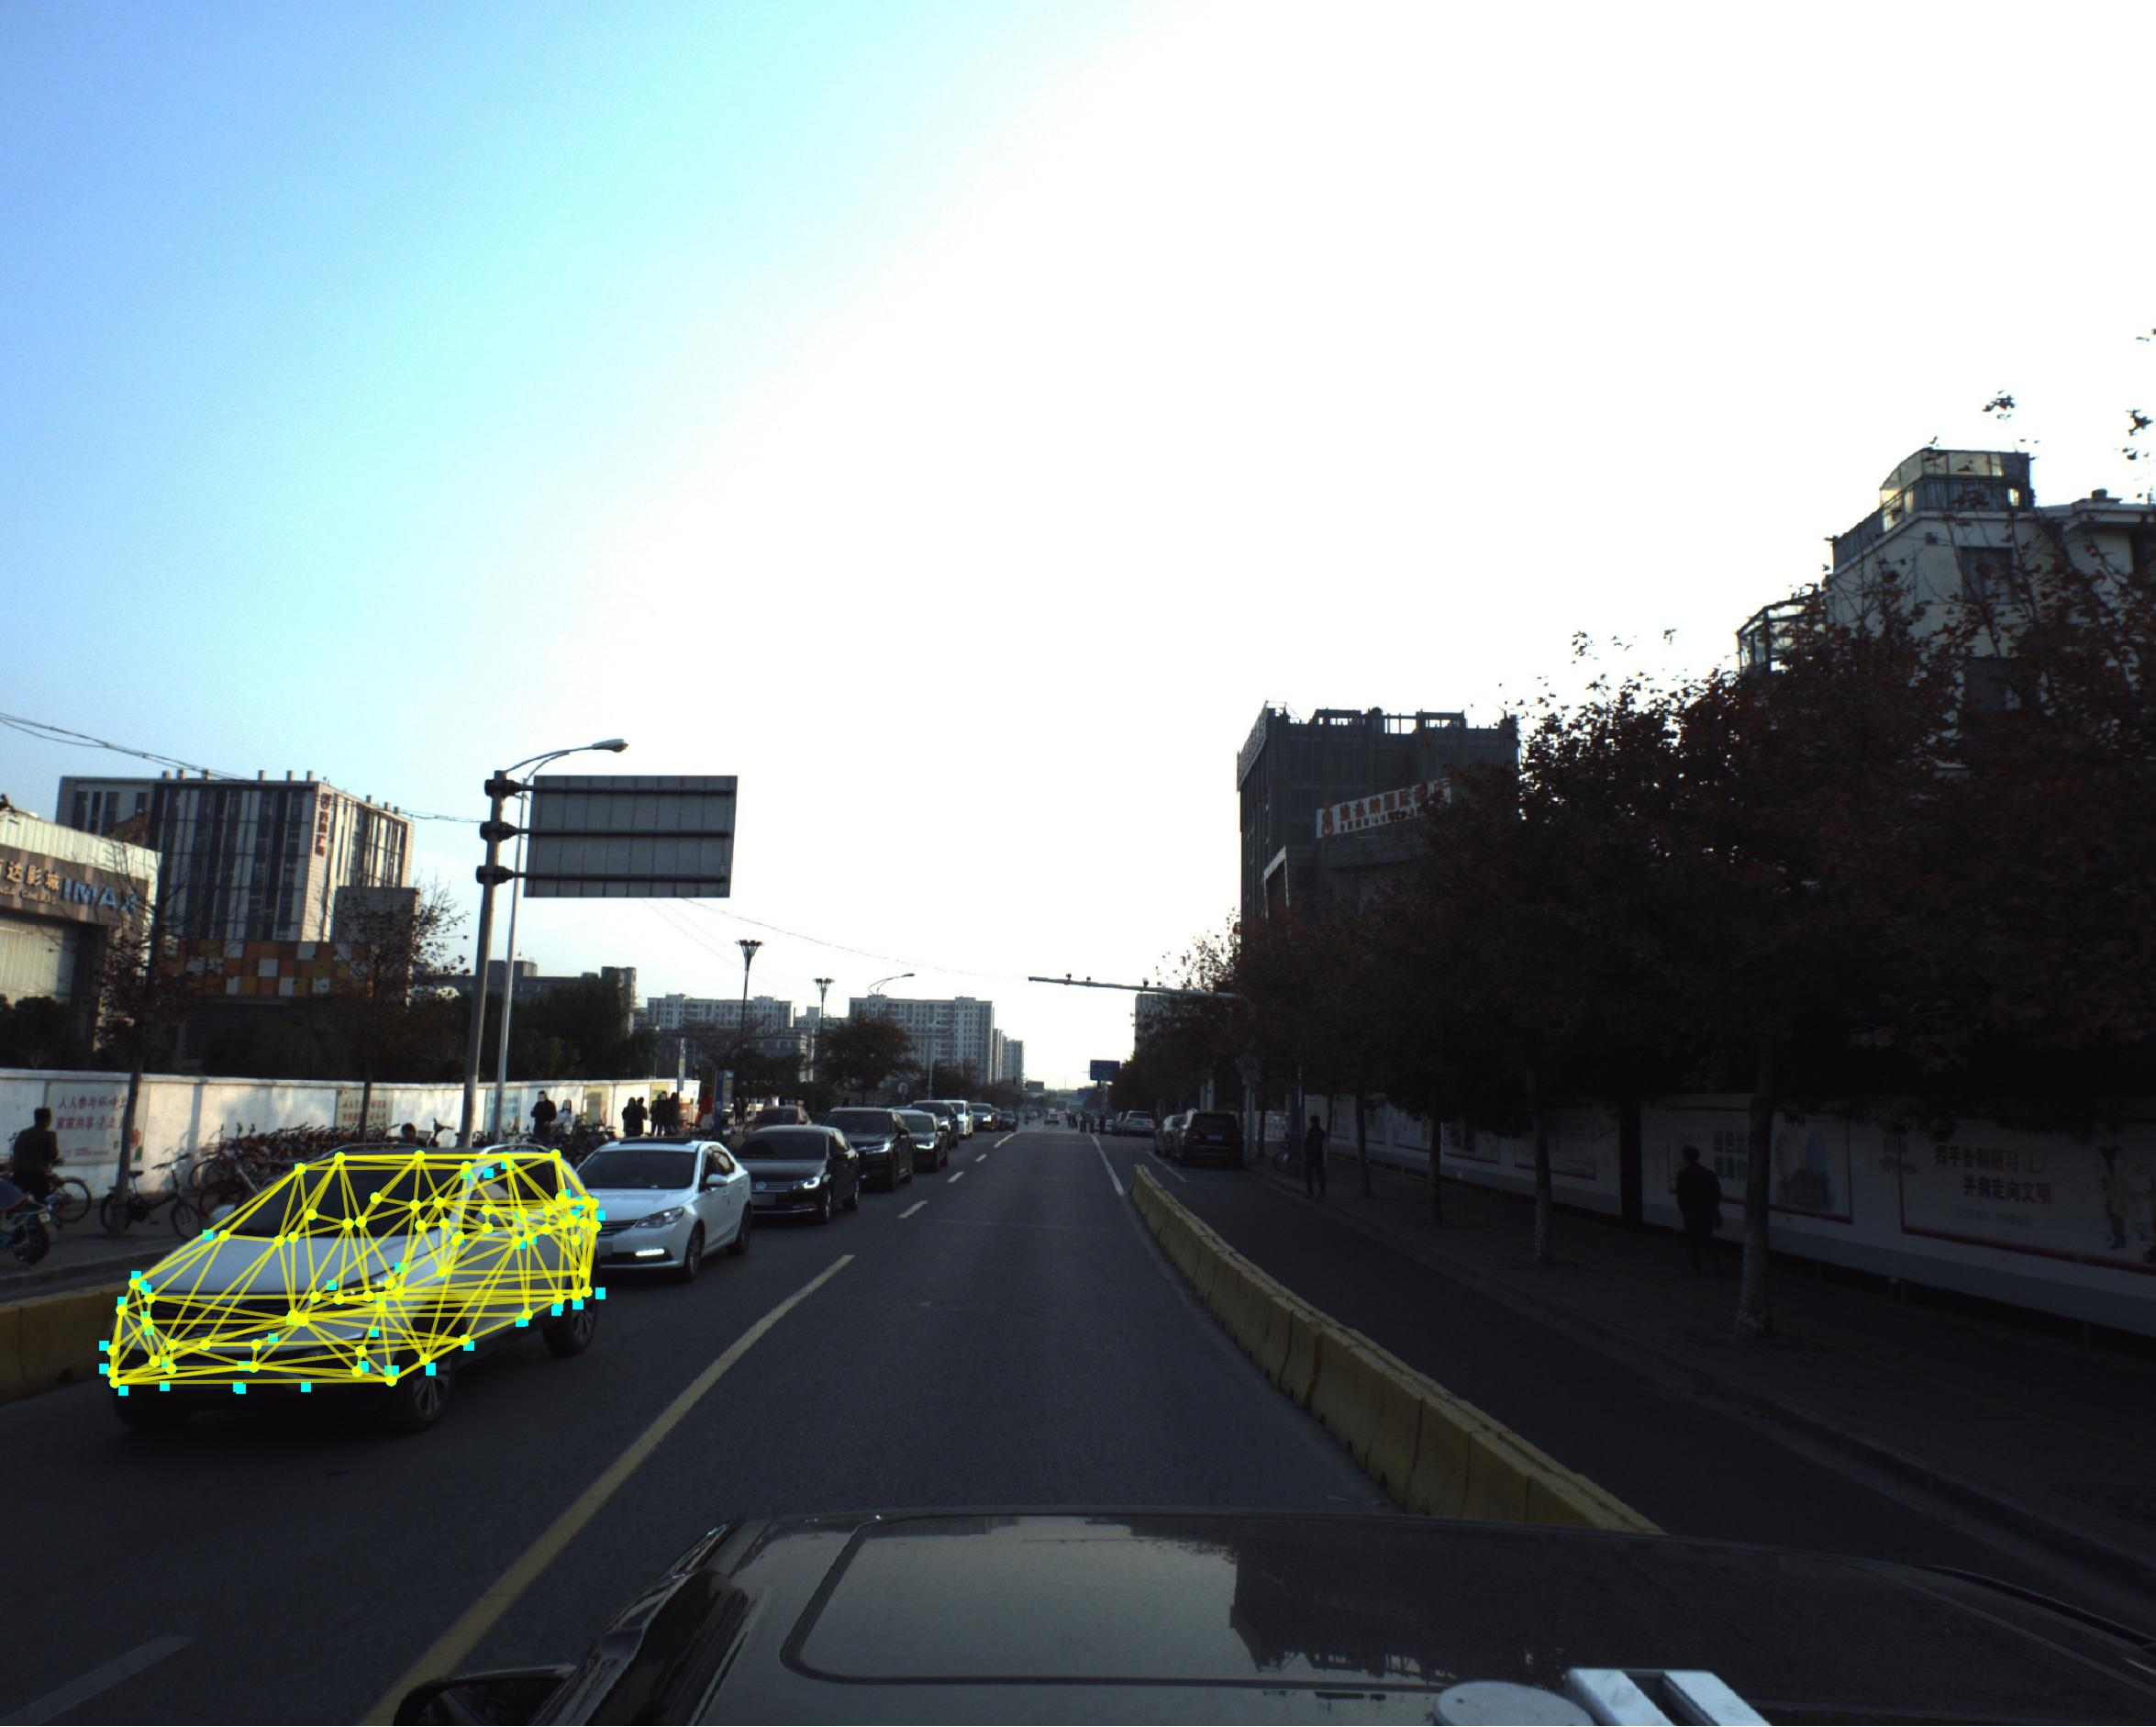}\\
			$\MR$ error: $2.03^{\circ}$, $\vt$ error: $0.09$ \\
			$\subopt=5.1\ee{-10}$, time: $4424$ [s]\\
			$n_1 = 1206, m=398,696$\\
			$N=66$, \# outliers: $30$
			\end{minipage}
		&  \myhspace \hspace{-3mm}
			\begin{minipage}{\mpwfour}%
			\centering%
			\includegraphics[width=0.95\columnwidth]{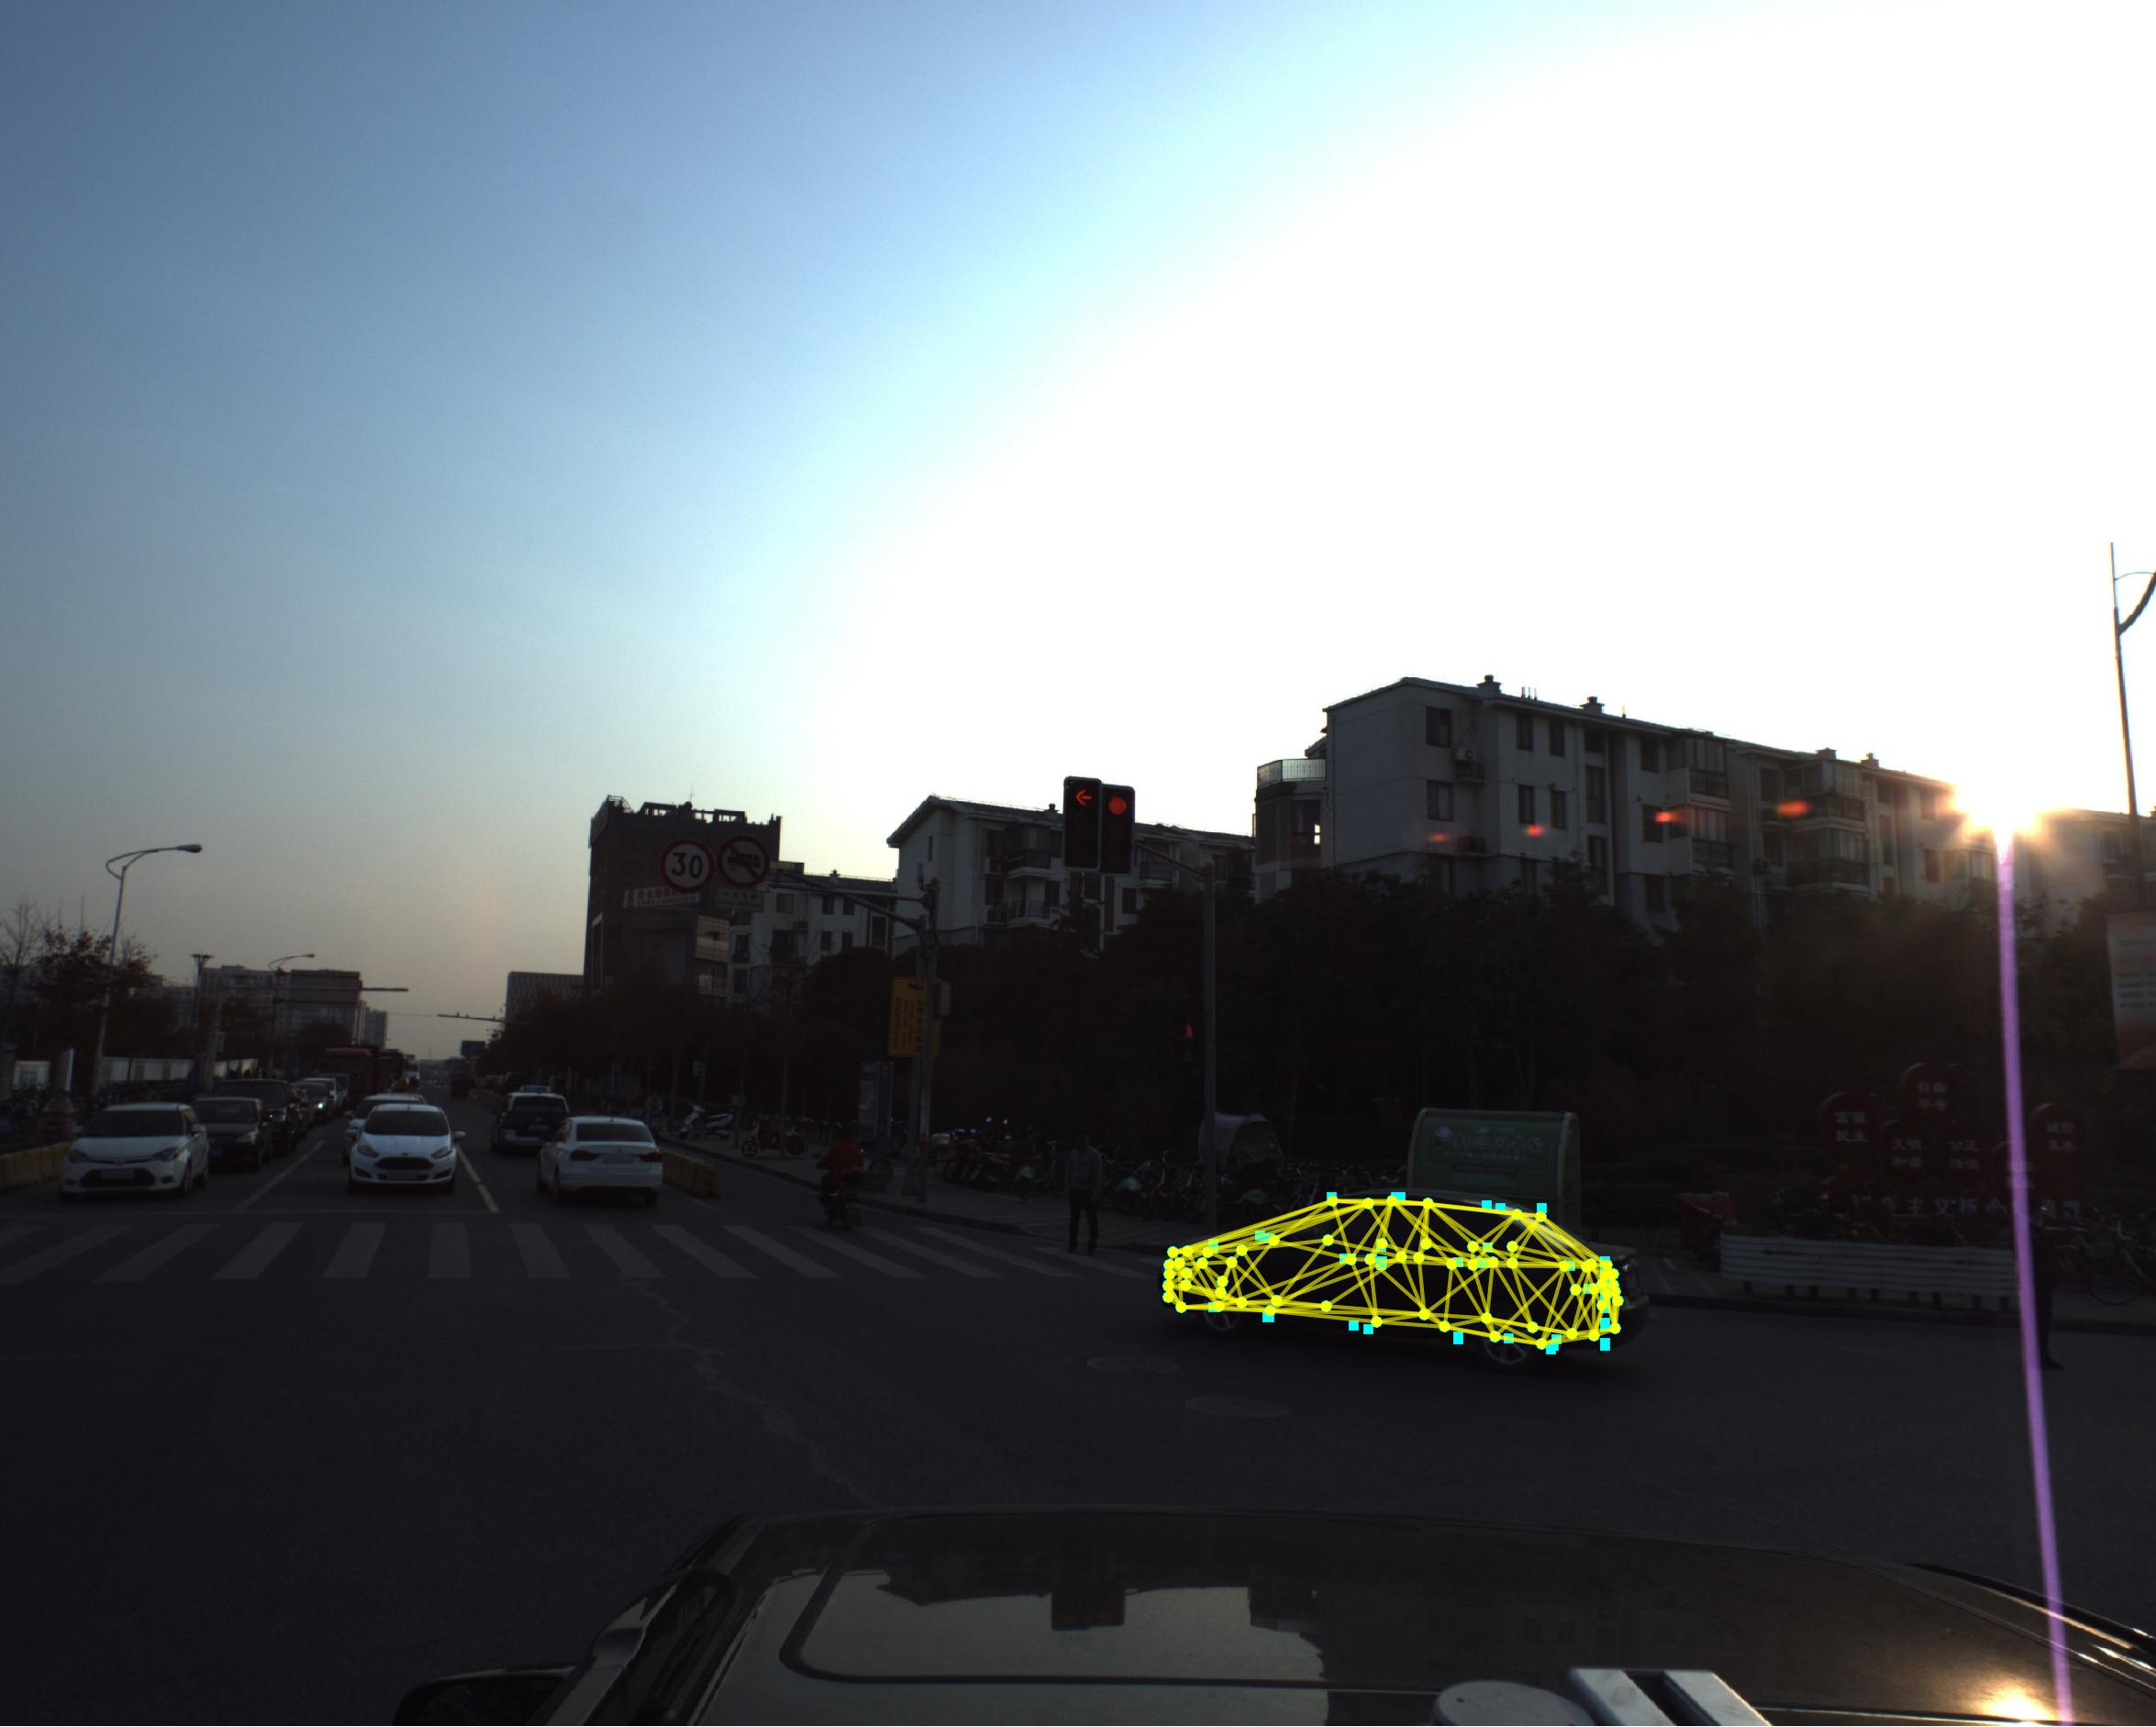}\\
			$\MR$ error: $2.36^{\circ}$, $\vt$ error: $0.08$ \\
			$\subopt=1.1\ee{-3}$, time: $6604$ [s]\\
			$n_1 = 1098, m=330,953$\\
			$N=60$, \# outliers: $23$
			\end{minipage}
		&  \myhspace \hspace{-3mm}
			\begin{minipage}{\mpwfour}%
			\centering%
			\includegraphics[width=0.95\columnwidth]{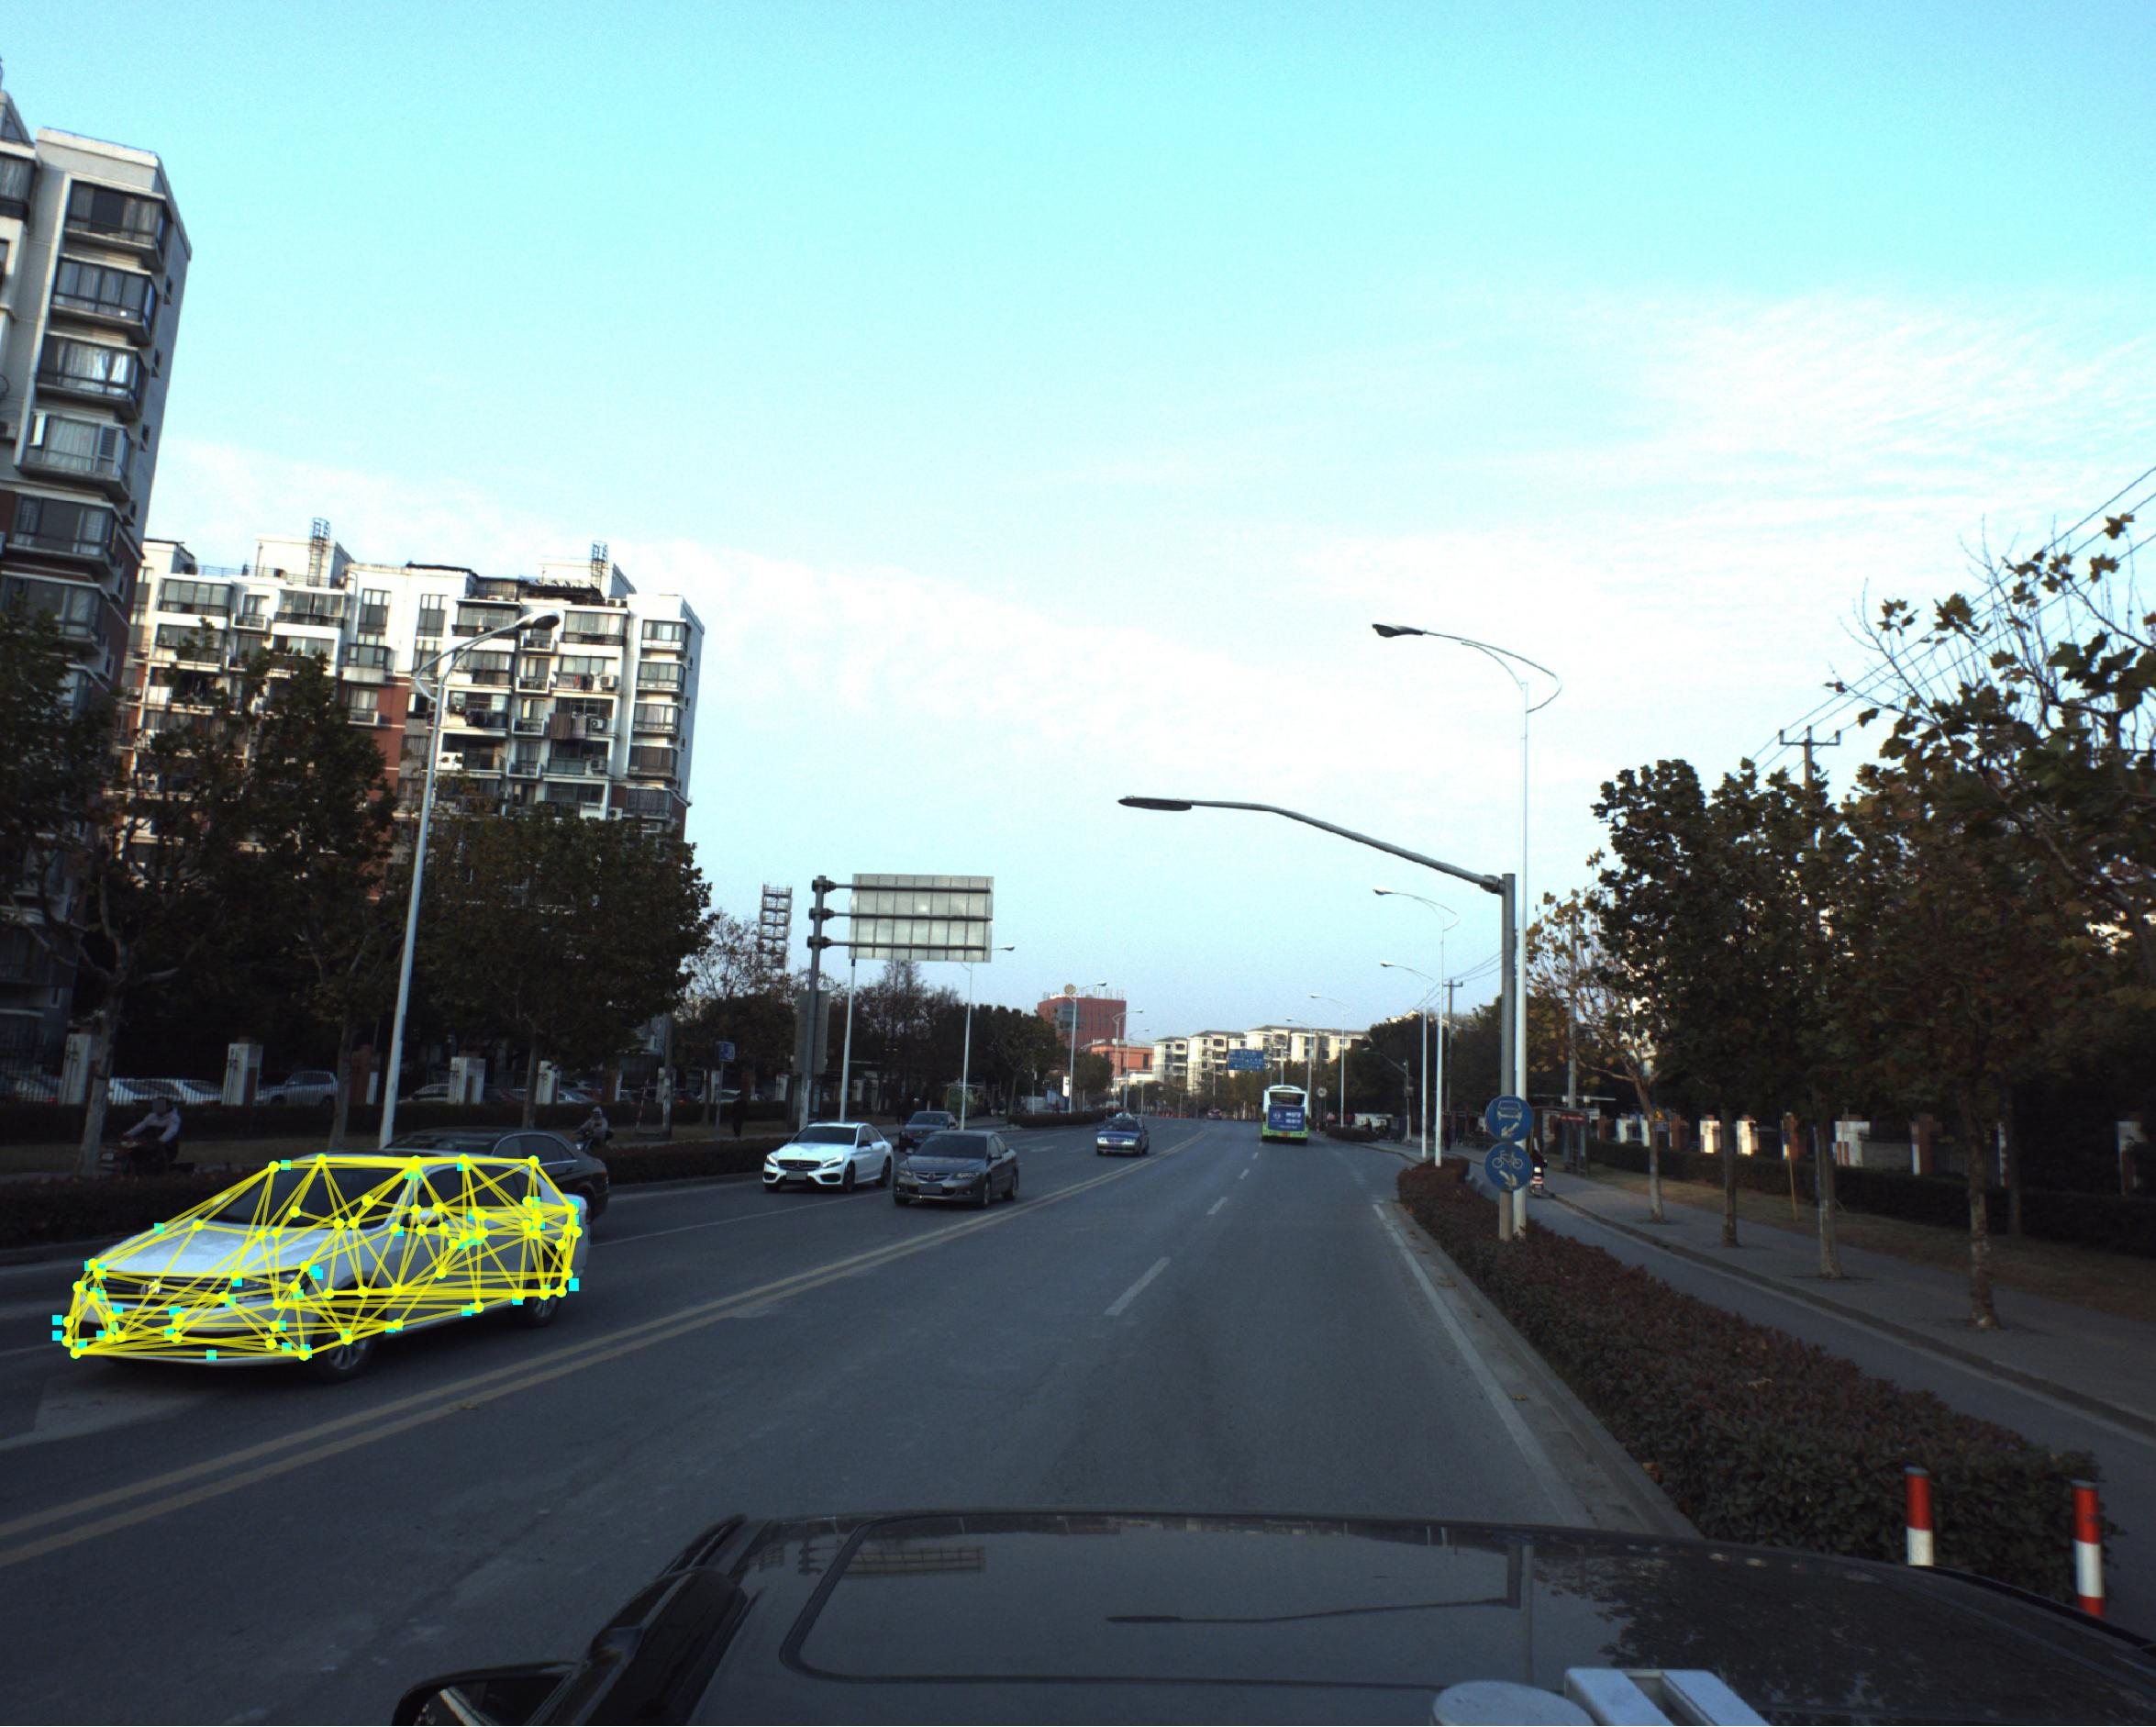}\\
			$\MR$ error: $2.80^{\circ}$, $\vt$ error: $0.09$ \\
			$\subopt=1.5\ee{-9}$, time: $4367$ [s]\\
			$n_1 = 1188, m=386,968$\\
			$N=65$, \# outliers: $28$
			\end{minipage}
			\vspace{1mm}
		\\

		\myhspace \hspace{-4mm}
			\begin{minipage}{\mpwfour}%
			\centering%
			\includegraphics[width=0.95\columnwidth]{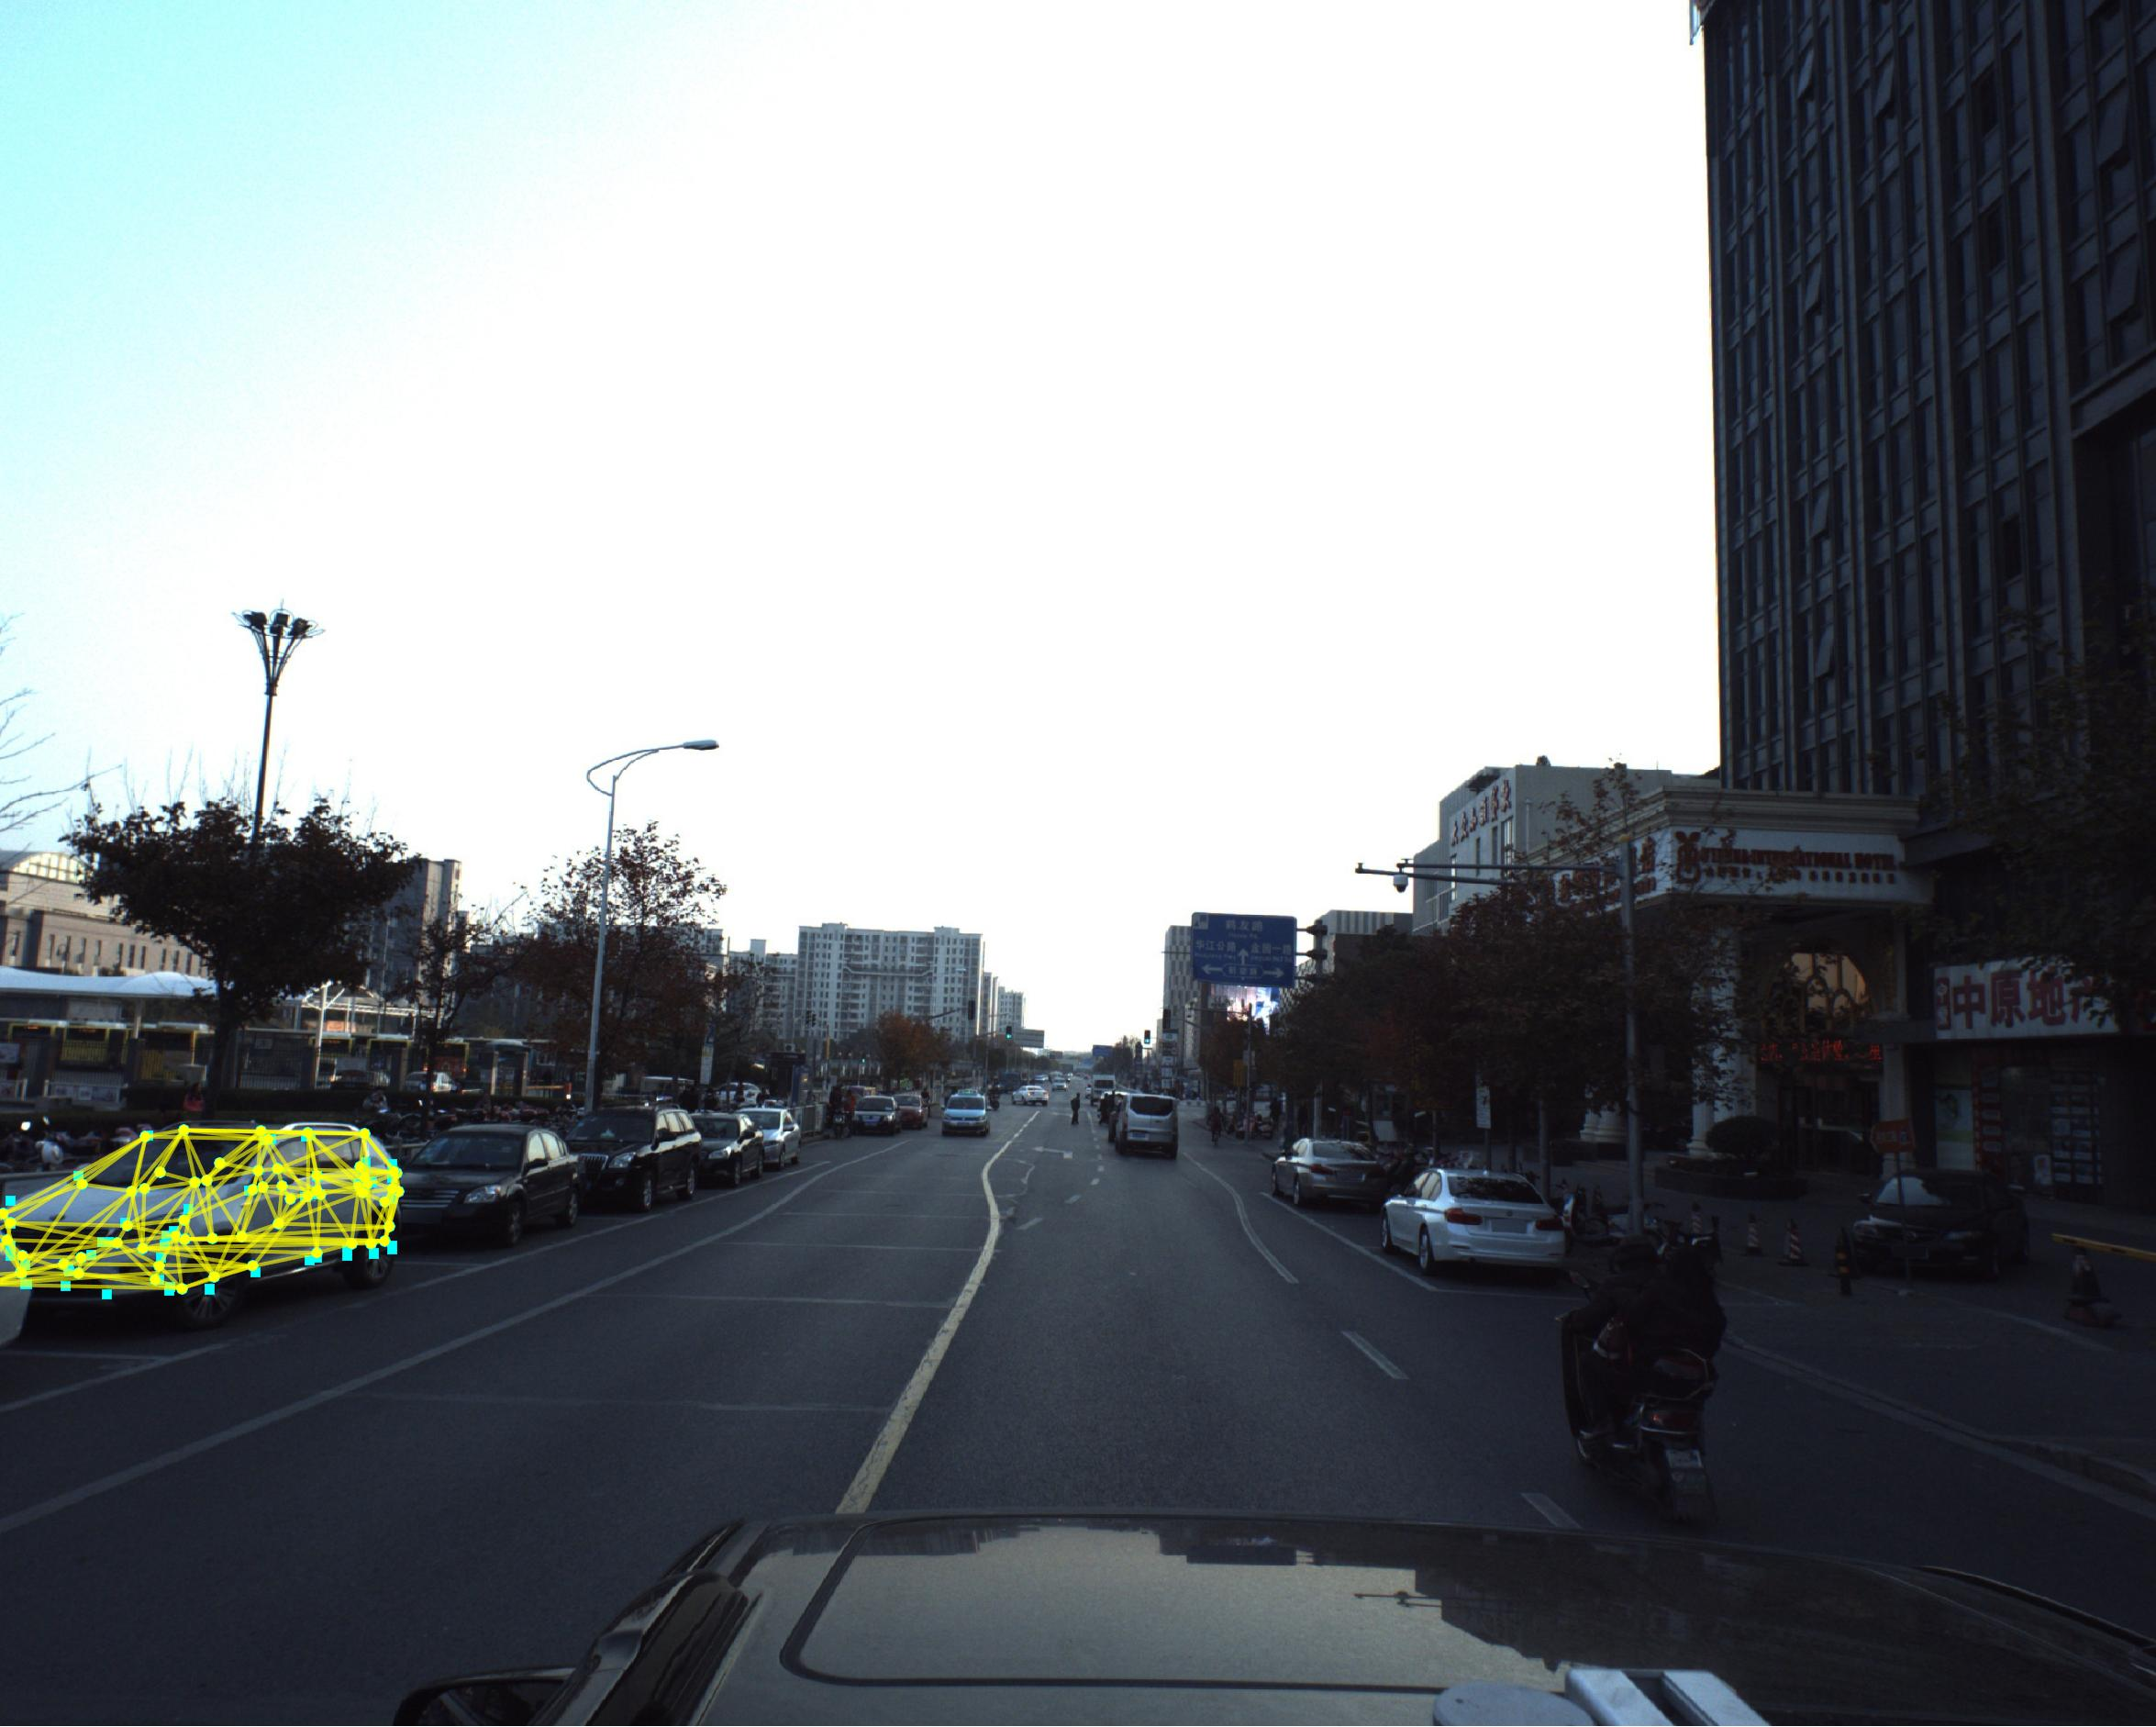}\\
			$\MR$ error: $2.12^{\circ}$, $\vt$ error: $0.10$ \\
			$\subopt=3.2\ee{-10}$, time: $4482$ [s]\\
			$n_1 = 1152, m=364,037$\\
			$N=63$, \# outliers: $28$
			\end{minipage}
		&  \myhspace \hspace{-3mm}
			\begin{minipage}{\mpwfour}%
			\centering%
			\includegraphics[width=0.95\columnwidth]{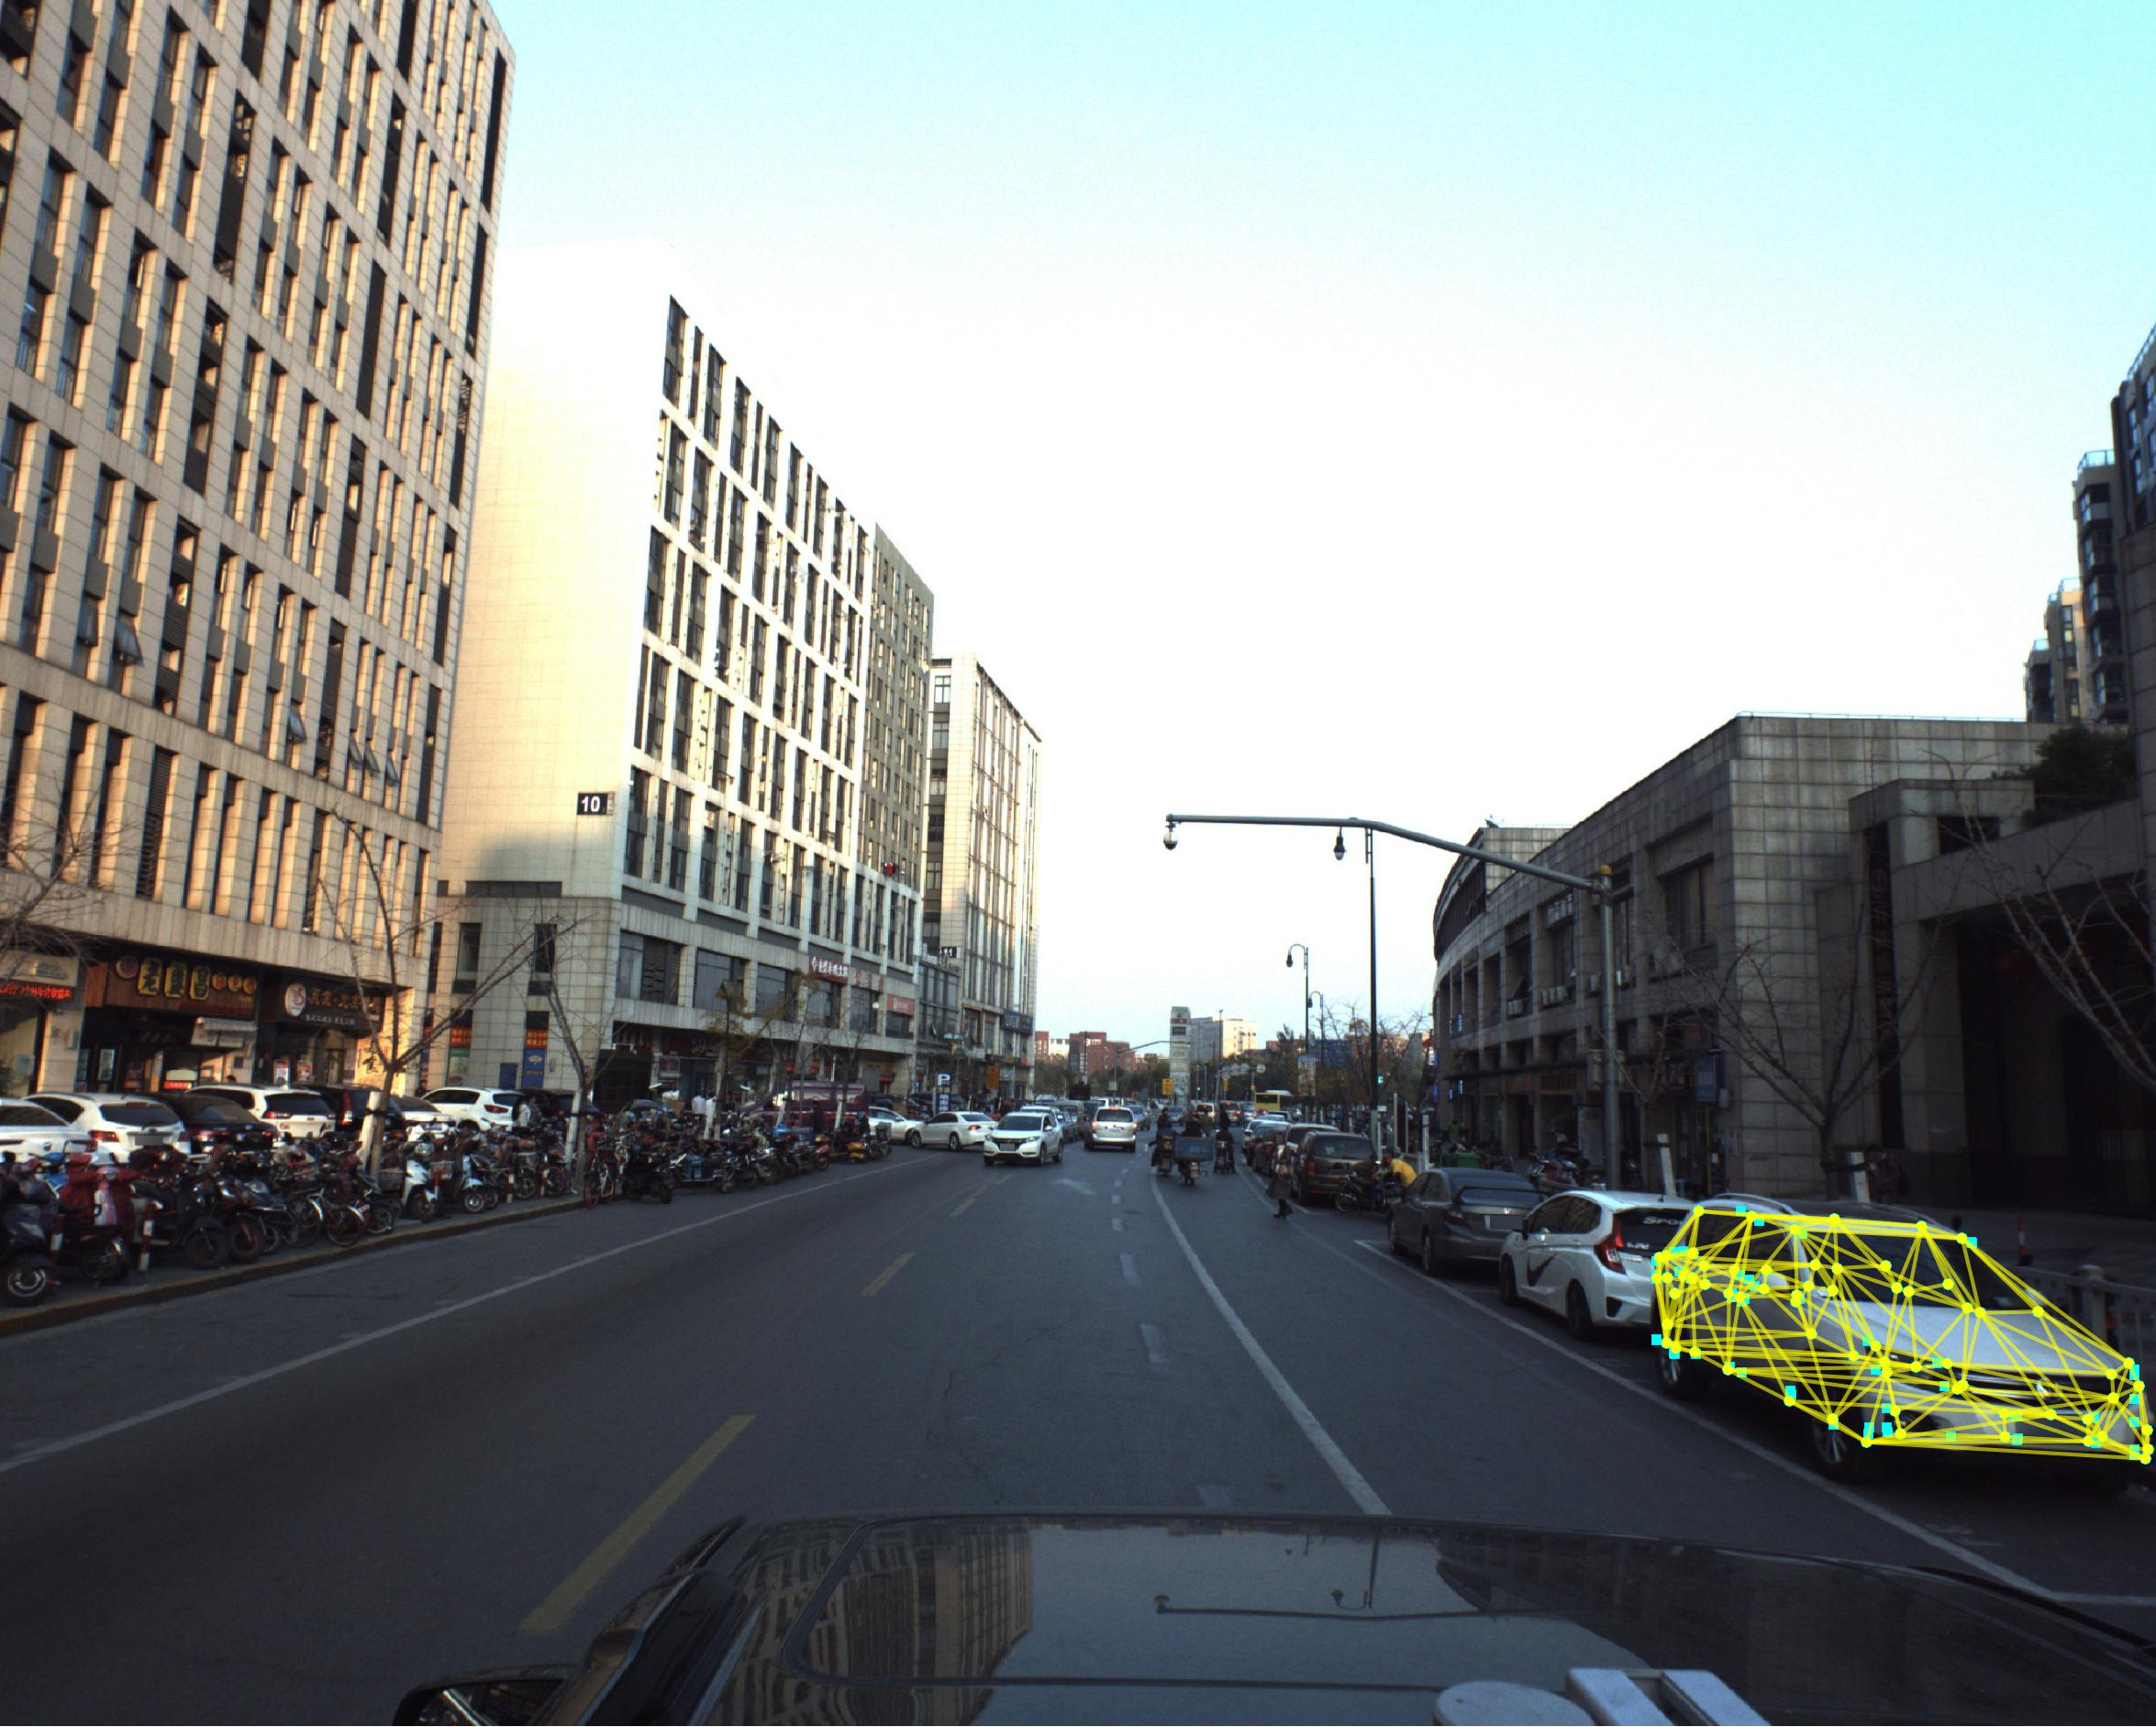}\\
			$\MR$ error: $2.62^{\circ}$, $\vt$ error: $0.04$ \\
			$\subopt=1.2\ee{-10}$, time: $4524$ [s]\\
			$n_1 = 1152, m=364,037$\\
			$N=63$, \# outliers: $29$
			\end{minipage}
		&  \myhspace \hspace{-3mm}
			\begin{minipage}{\mpwfour}%
			\centering%
			\includegraphics[width=0.95\columnwidth]{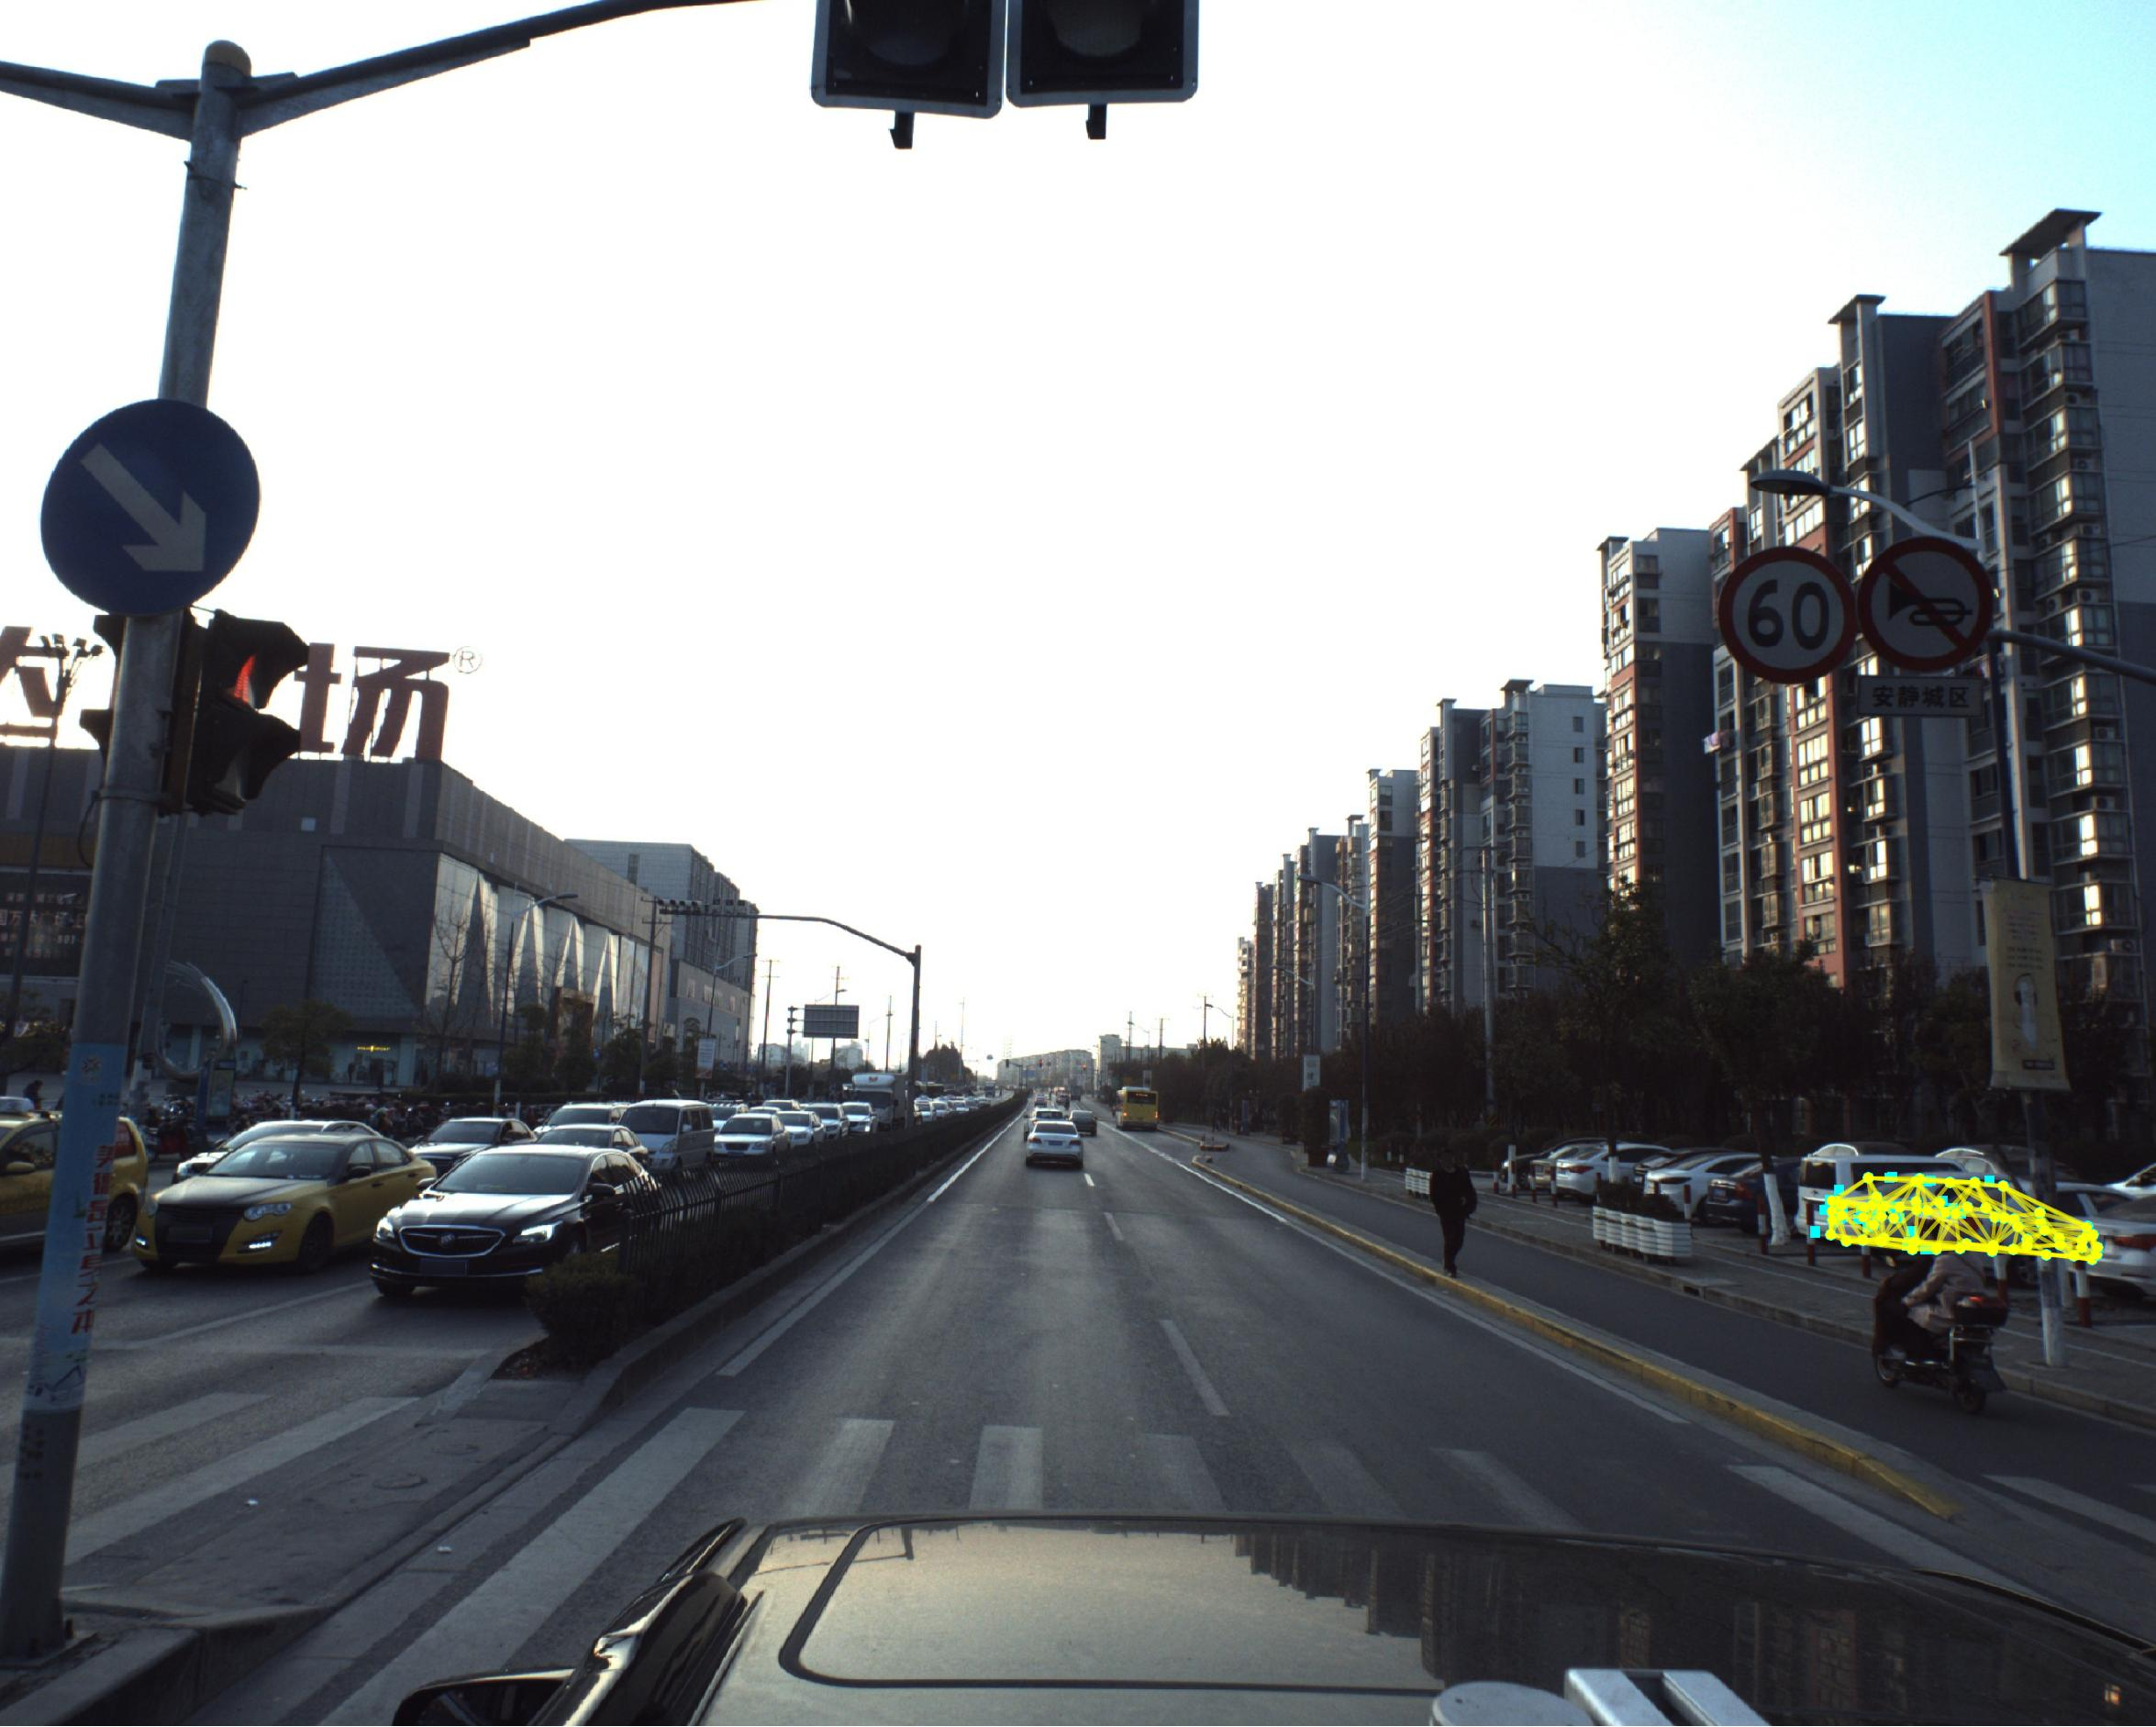}\\
			$\MR$ error: $2.62^{\circ}$, $\vt$ error: $0.07$ \\
			$\subopt=1.8\ee{-7}$, time: $2344$ [s]\\
			$n_1 = 684, m=129,634$\\
			$N=37$, \# outliers: $16$
			\end{minipage}
		&  \myhspace \hspace{-3mm}
			\begin{minipage}{\mpwfour}%
			\centering%
			\includegraphics[width=0.95\columnwidth]{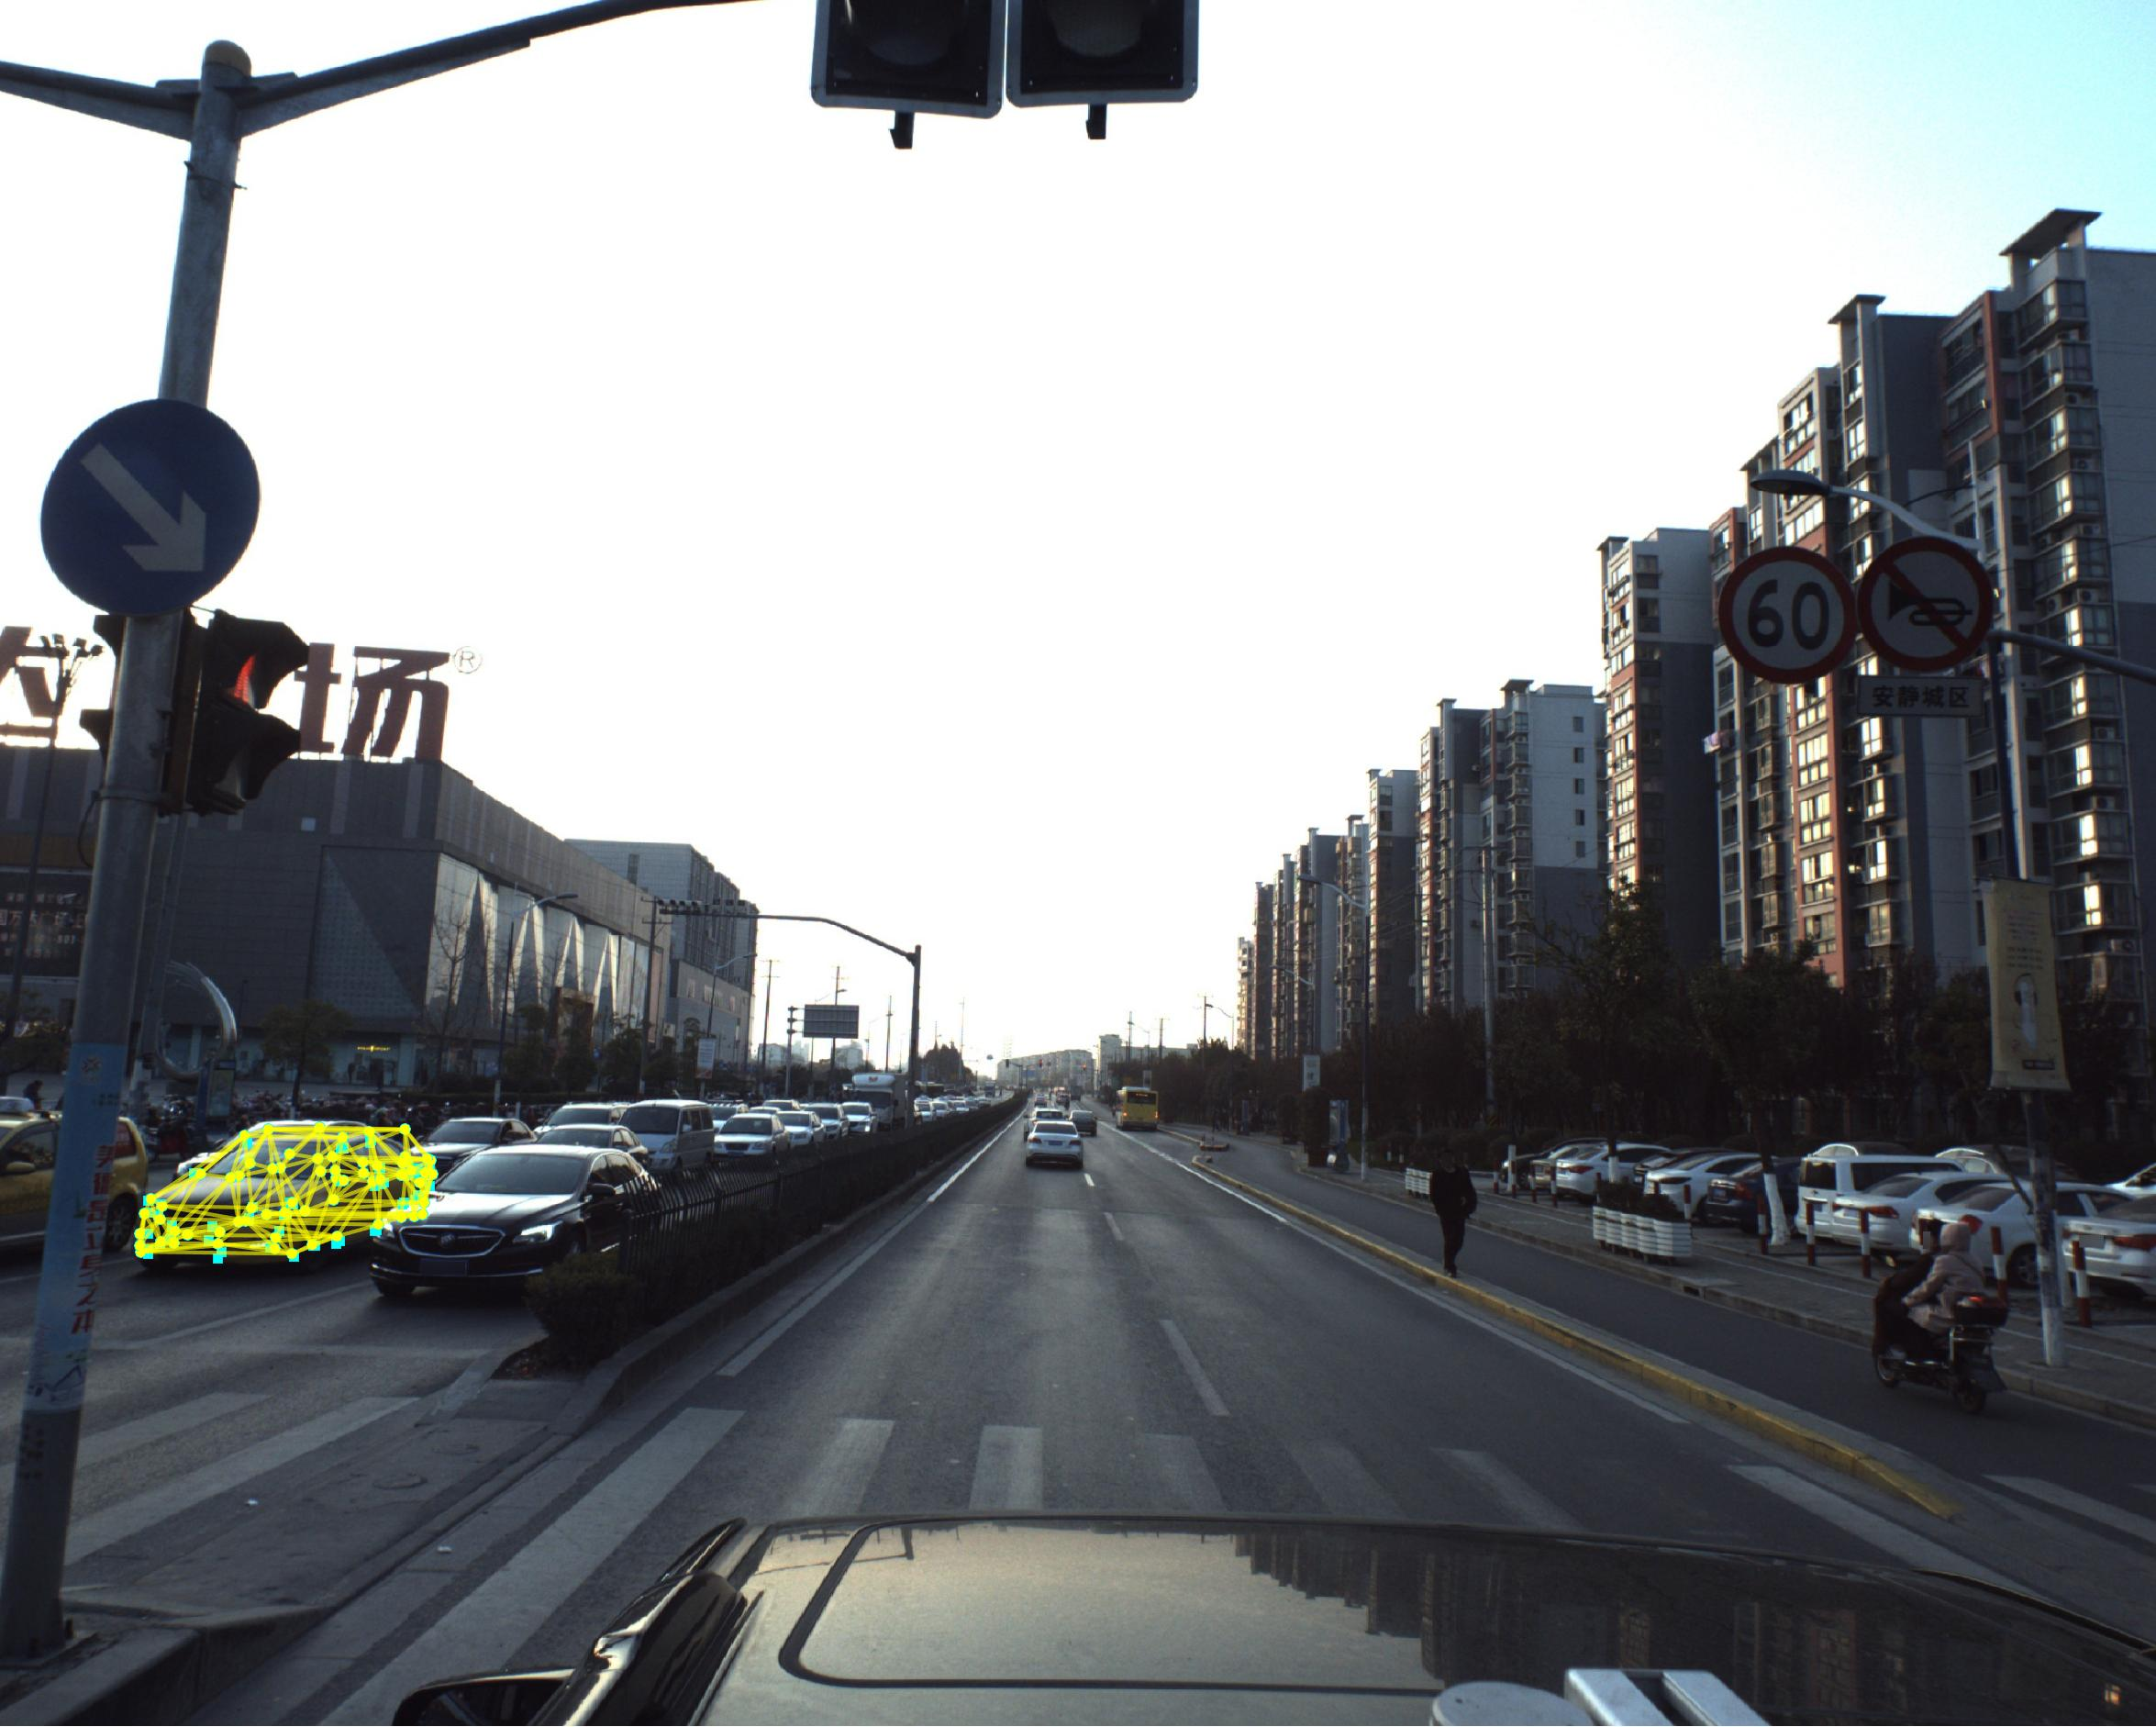}\\
			$\MR$ error: $2.19^{\circ}$, $\vt$ error: $0.09$ \\
			$\subopt=3.1\ee{-10}$, time: $5090$ [s]\\
			$n_1 = 1170, m=375,415$\\
			$N=64$, \# outliers: $28$
			\end{minipage}
	\end{tabular}
	\end{minipage} 
	\caption{Extra vehicle pose and shape estimation on {\apollo} \cite{Wang19pami-apolloscape}.
	\label{fig:supp-apollo}} 
	\vspace{-4mm} 
	\end{center}
\end{figure*}
