# Supplementary material for: Certifiably Optimal Outlier-Robust Geometric Perception: Semidefinite Relaxations and Scalable Global Optimization
Source: arXiv:2109.03349 source file (2022-05-29)
Supplement: Supplementary file 4 [file supp-fig-speed.tex]

%!TEX root = ../main.tex
% \vspace{-10mm}
\renewcommand{\mpwfour}{4.2cm}
\begin{figure*}[t]
	\begin{center}
	\begin{minipage}{\textwidth}
	\begin{tabular}{cccc}%
	% \hline
	$2$ outliers & $3$ outliers & $4$ outliers & $5$ outliers \\
	% \hline
	% \hline
		%%%%%%%%%%%%%%%%%%%%%%%%%%%%%%%%%%%%%%%%%%%%%%%%%%%%%%%%%%%%%%%%%%%%%%%%%%%%%%%%%%%%%%%%%%%%%%%%%%%%%%%%%
			\begin{minipage}{\mpwfour}%
			\centering%
			\includegraphics[width=\columnwidth]{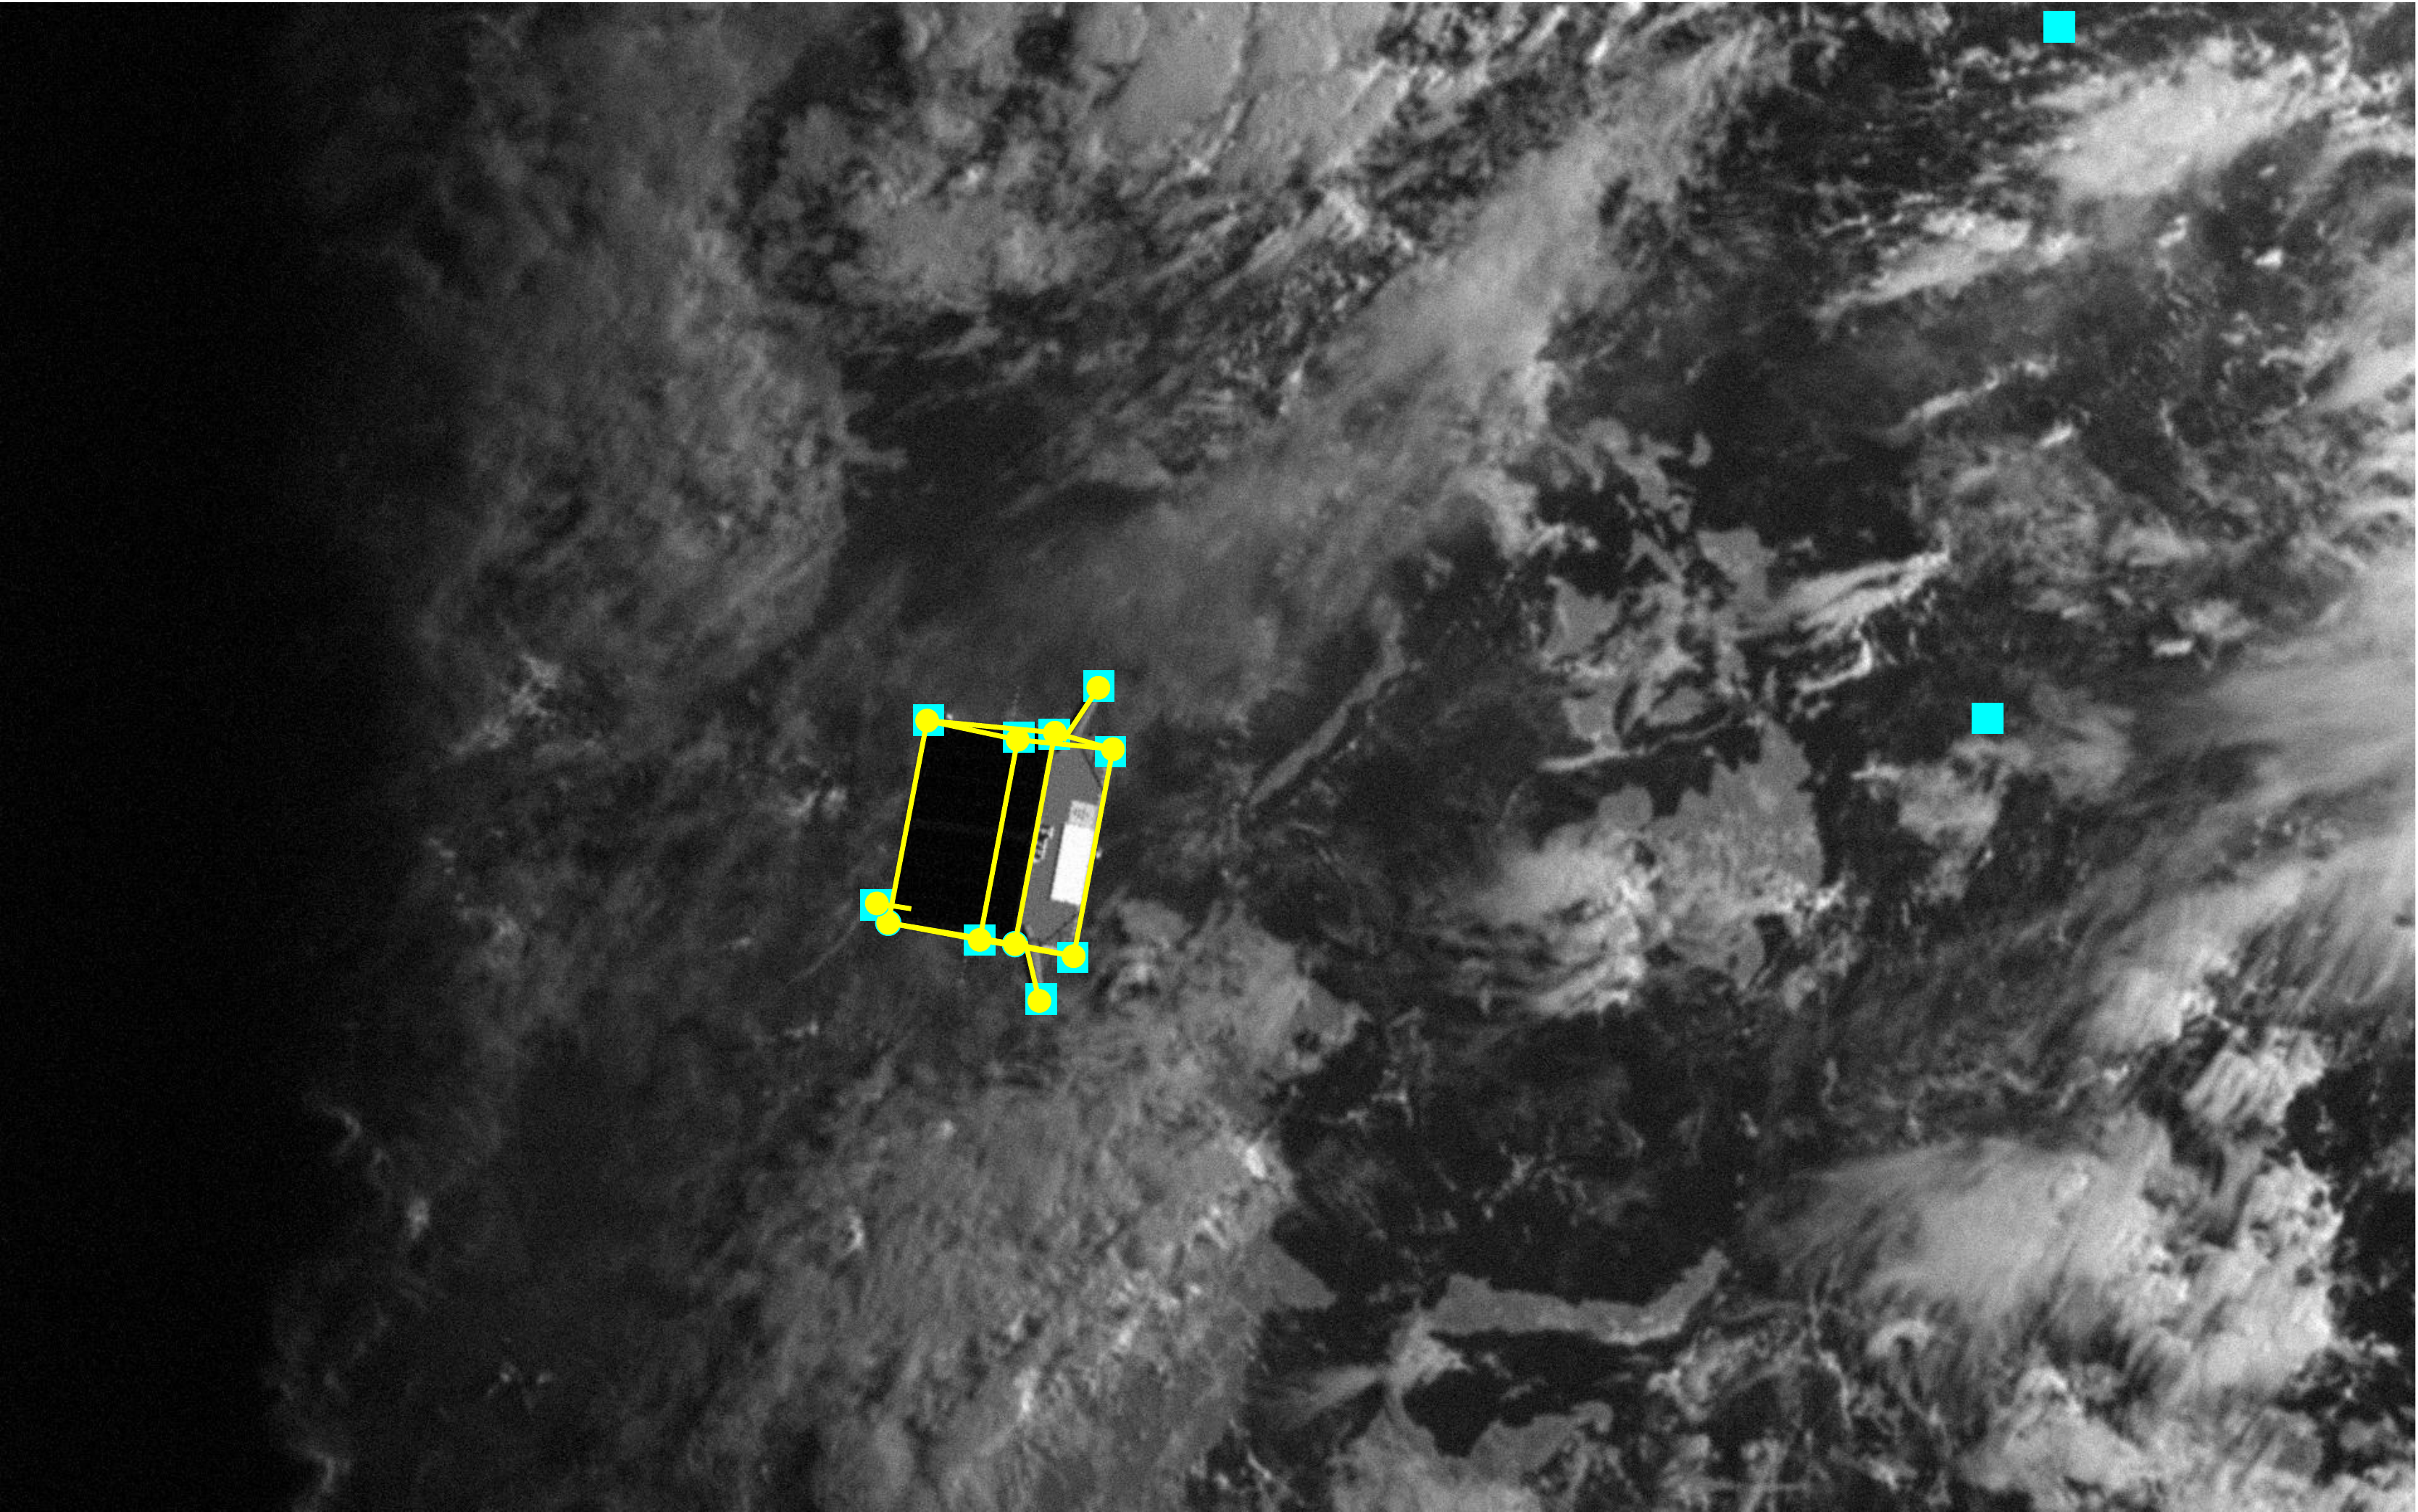}\\
			 $\MR$ error: $0.48^{\circ}$, $\vt$ error: $0.05$ \\ 
			 $\subopt=2.9\ee{-8}$, time: $51$ [s]
			\end{minipage}
		&  
			\begin{minipage}{\mpwfour}%
			\centering%
			\includegraphics[width=\columnwidth]{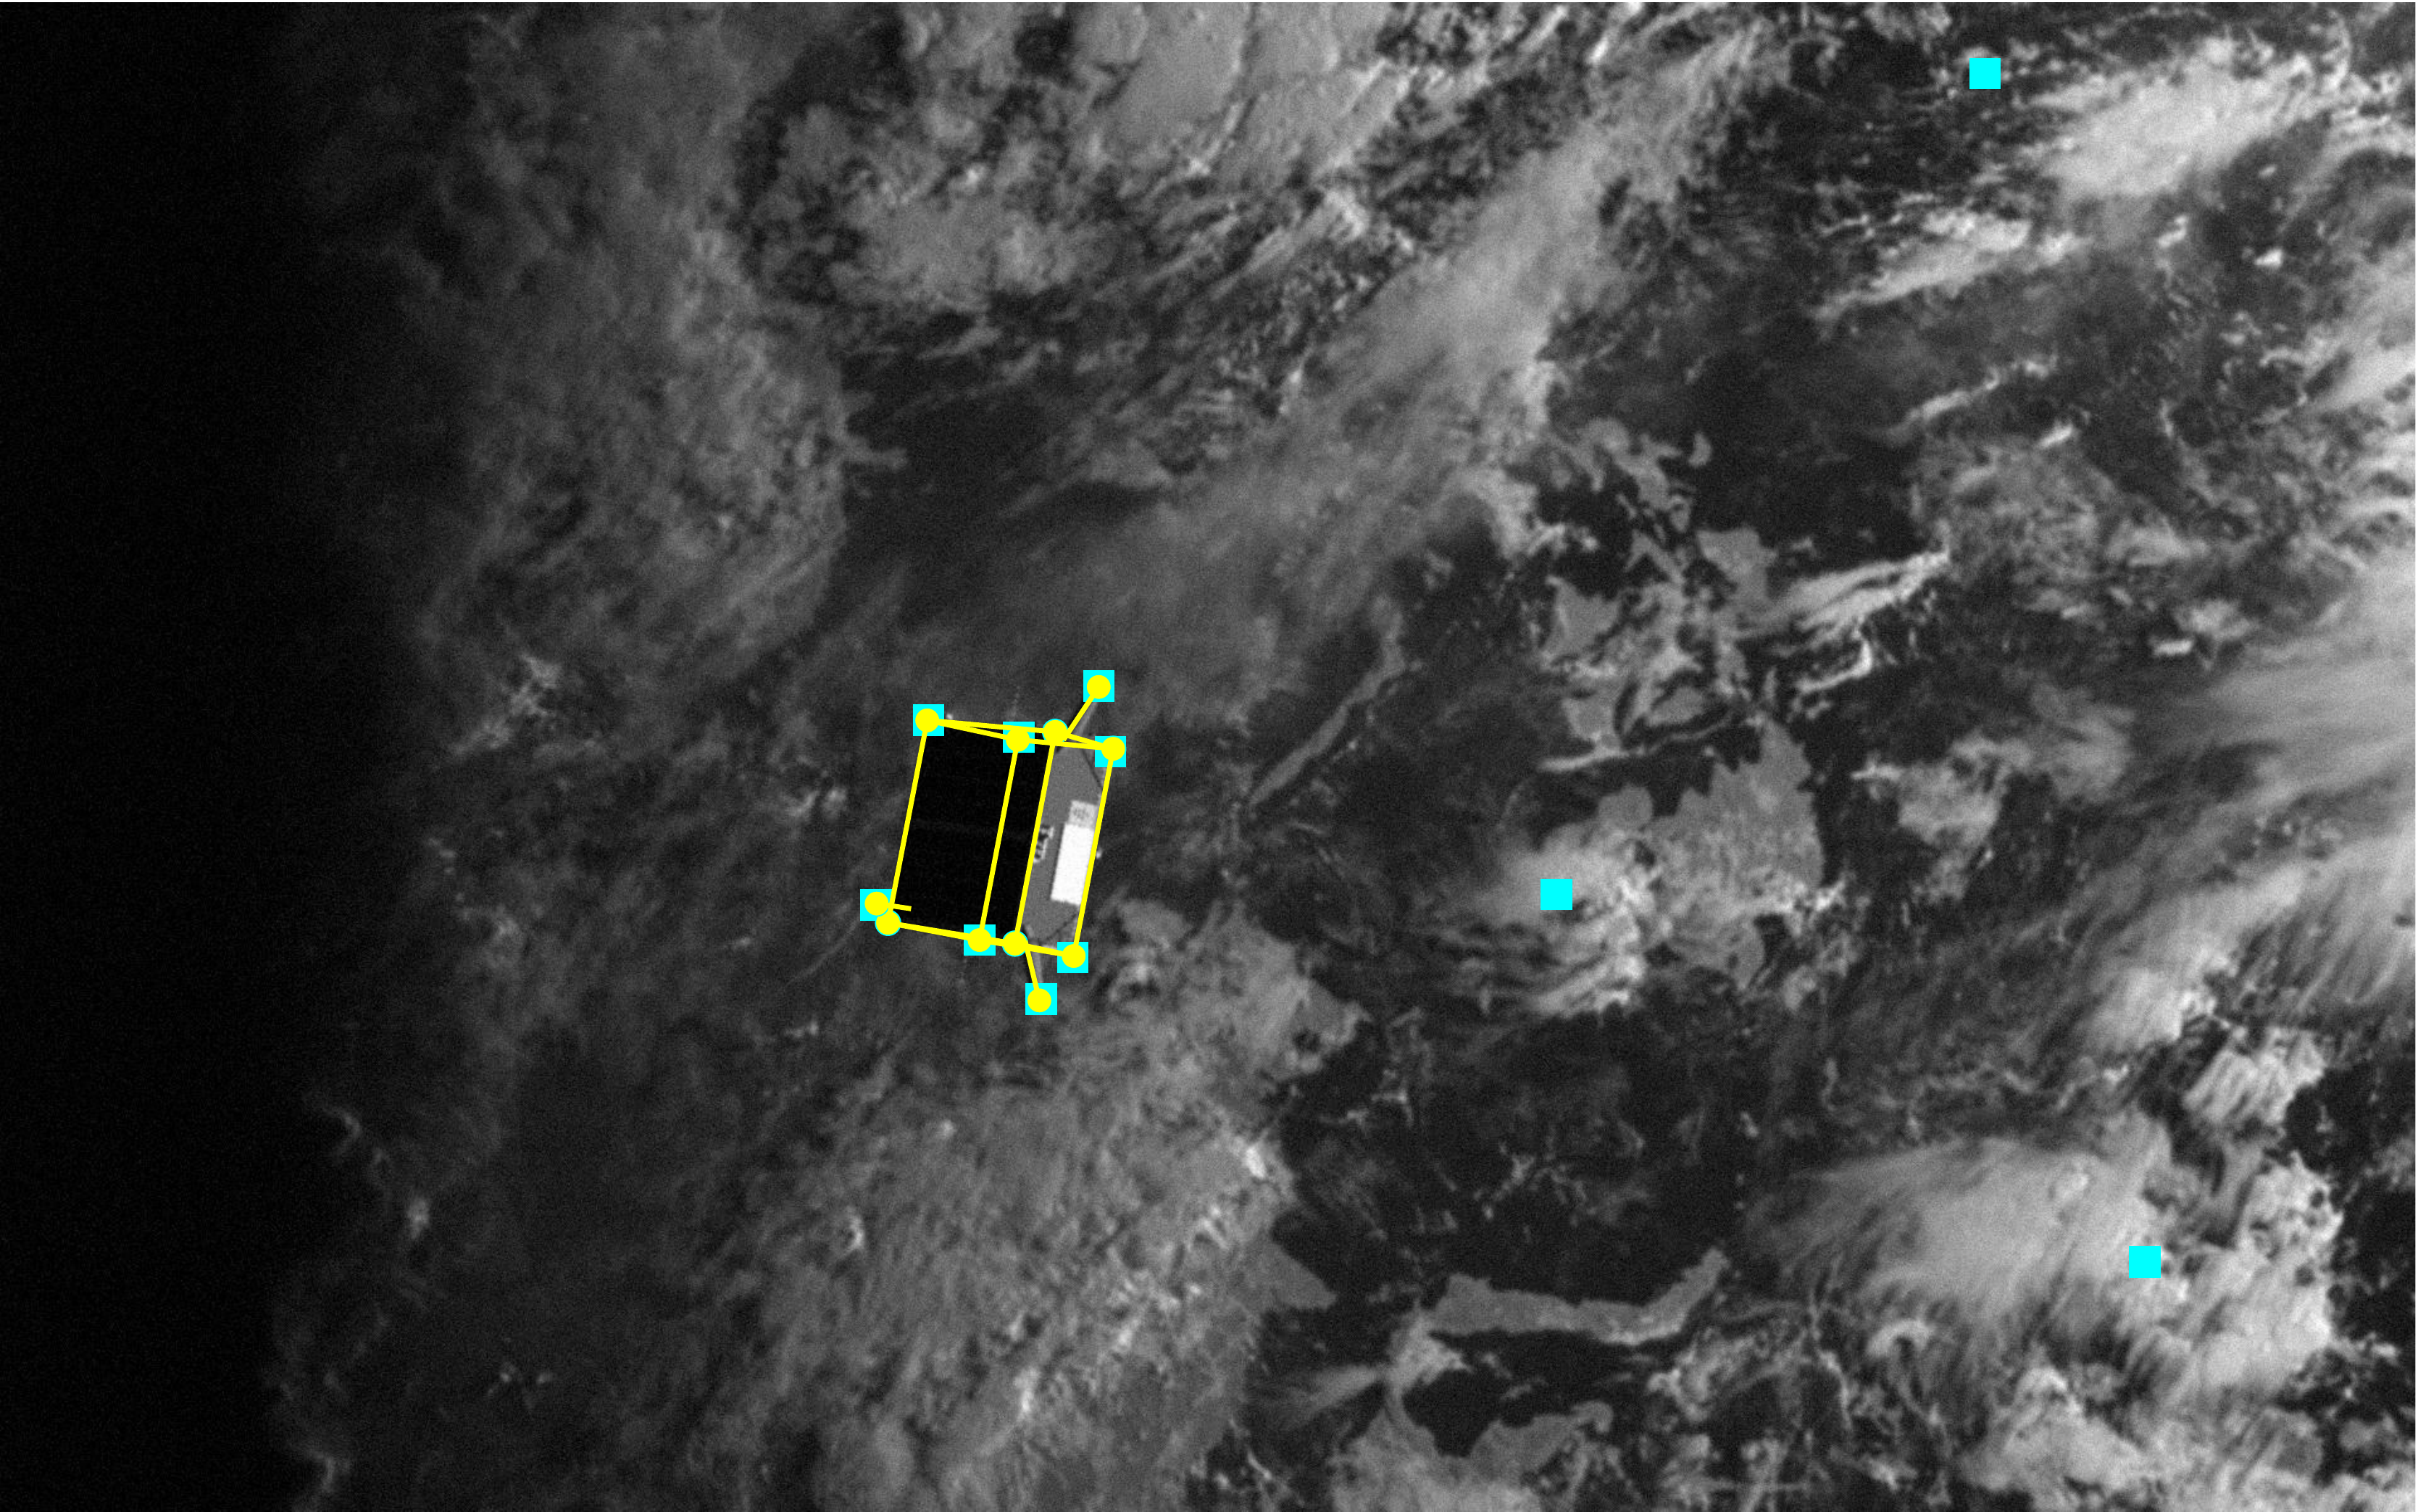}\\
			 $\MR$ error: $0.37^{\circ}$, $\vt$ error: $0.07$ \\ 
			 $\subopt=1.3\ee{-7}$, time: $47$ [s]
			\end{minipage}
		&  
			\begin{minipage}{\mpwfour}%
			\centering%
			\includegraphics[width=\columnwidth]{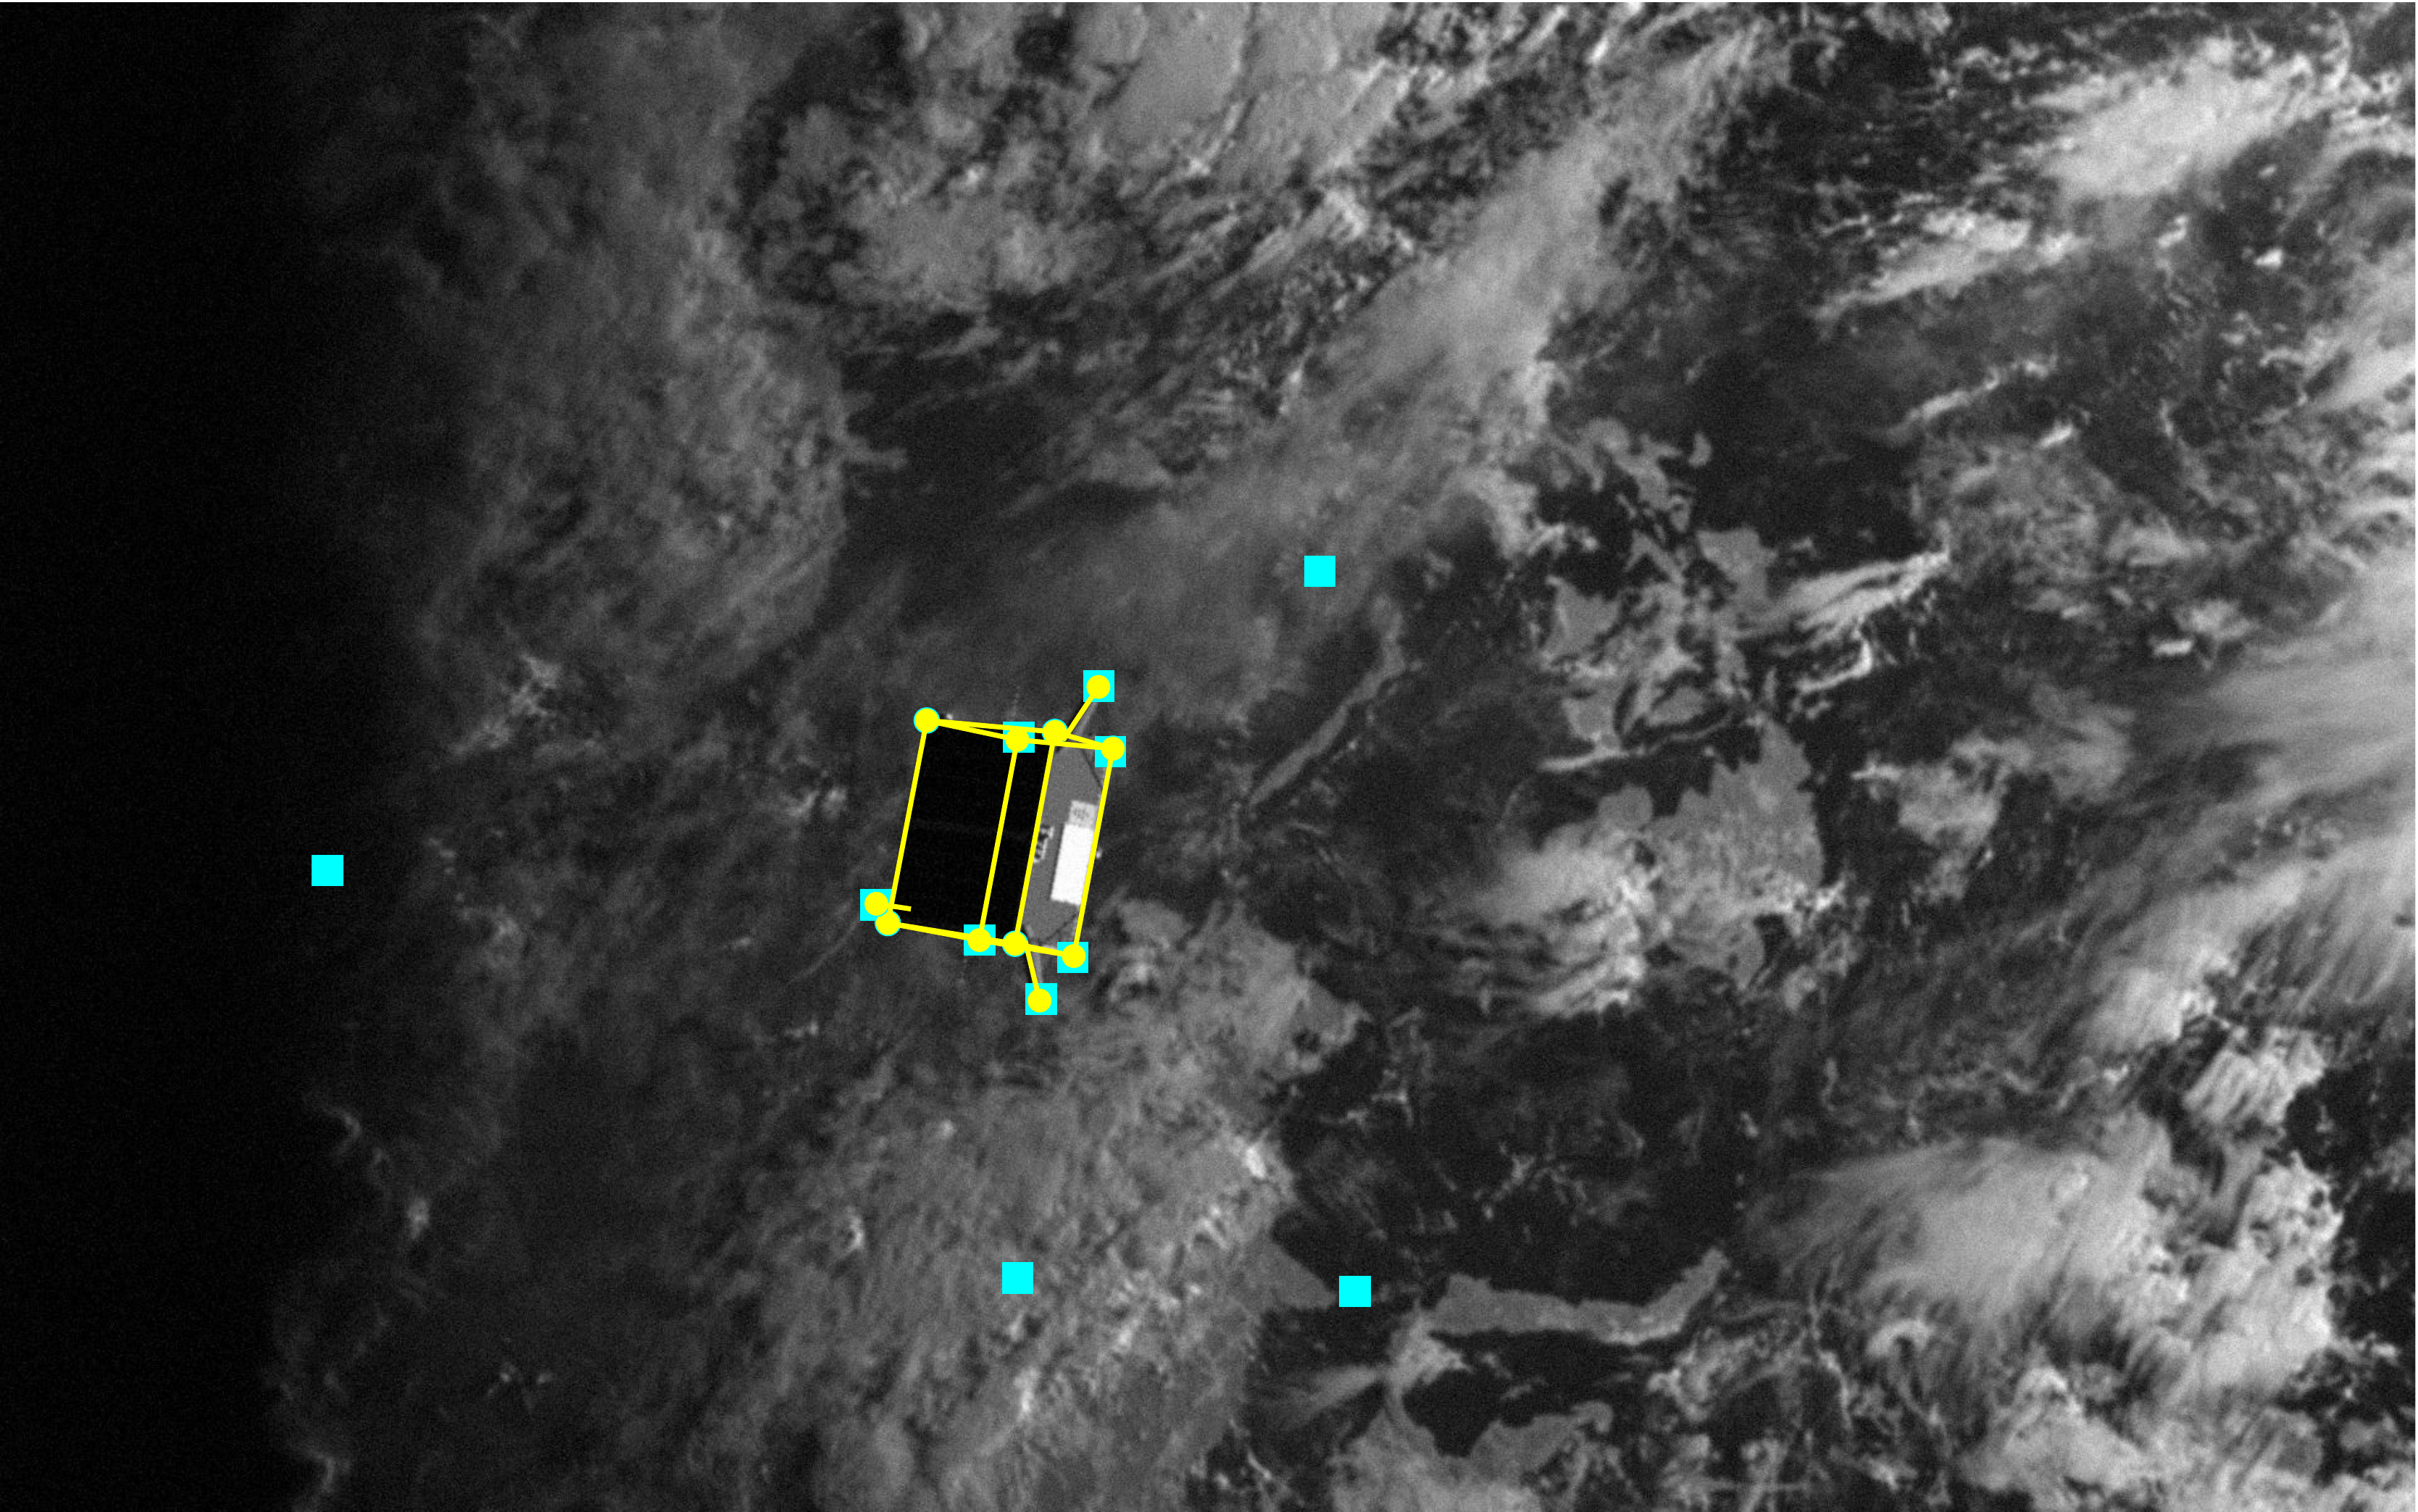}\\
			 $\MR$ error: $0.37^{\circ}$, $\vt$ error: $0.07$ \\ 
			 $\subopt=1.8\ee{-8}$, time: $109$ [s]
			\end{minipage}
		&  
			\begin{minipage}{\mpwfour}%
			\centering%
			\includegraphics[width=\columnwidth]{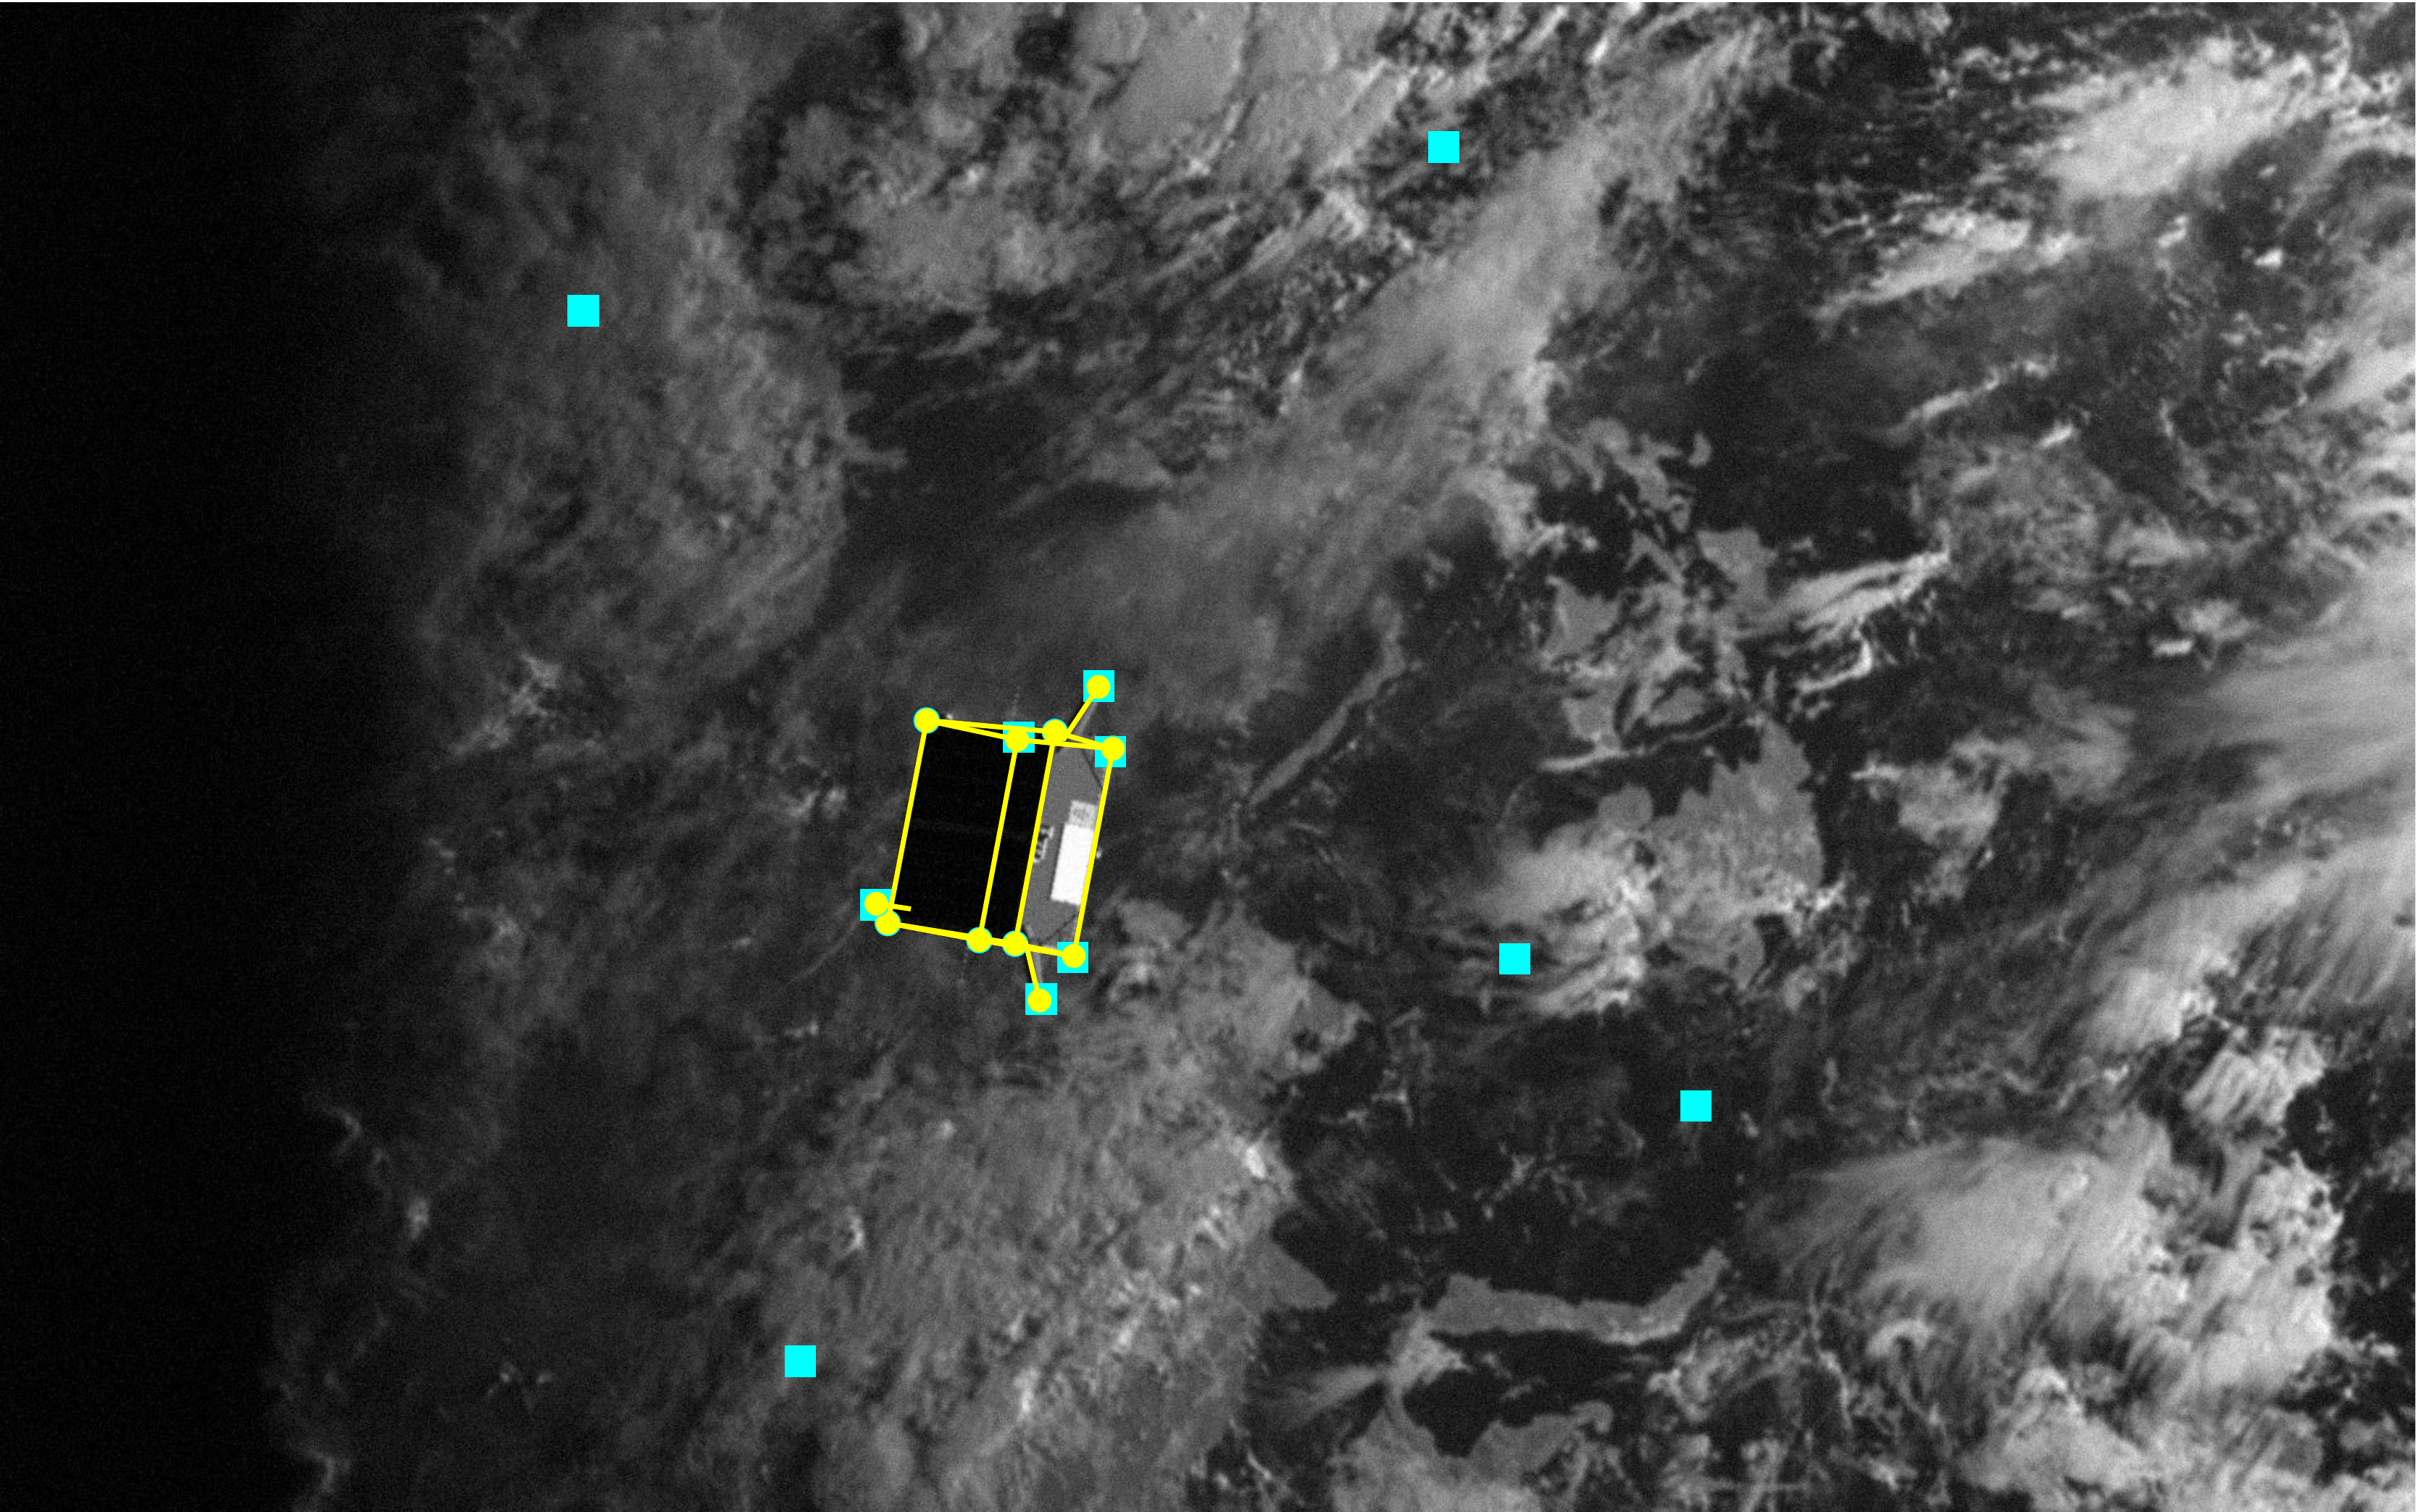}\\
			 $\MR$ error: $0.34^{\circ}$, $\vt$ error: $0.07$ \\ 
			 $\subopt=1.4\ee{-9}$, time: $107$ [s]
			\end{minipage} \vspace{1mm}
		\\

		%%%%%%%%%%%%%%%%%%%%%%%%%%%%%%%%%%%%%%%%%%%%%%%%%%%%%%%%%%%%%%%%%%%%%%%%%%%%%%%%%%%%%%%%%%%%%%%%%%%%%%%%%
			\begin{minipage}{\mpwfour}%
			\centering%
			\includegraphics[width=\columnwidth]{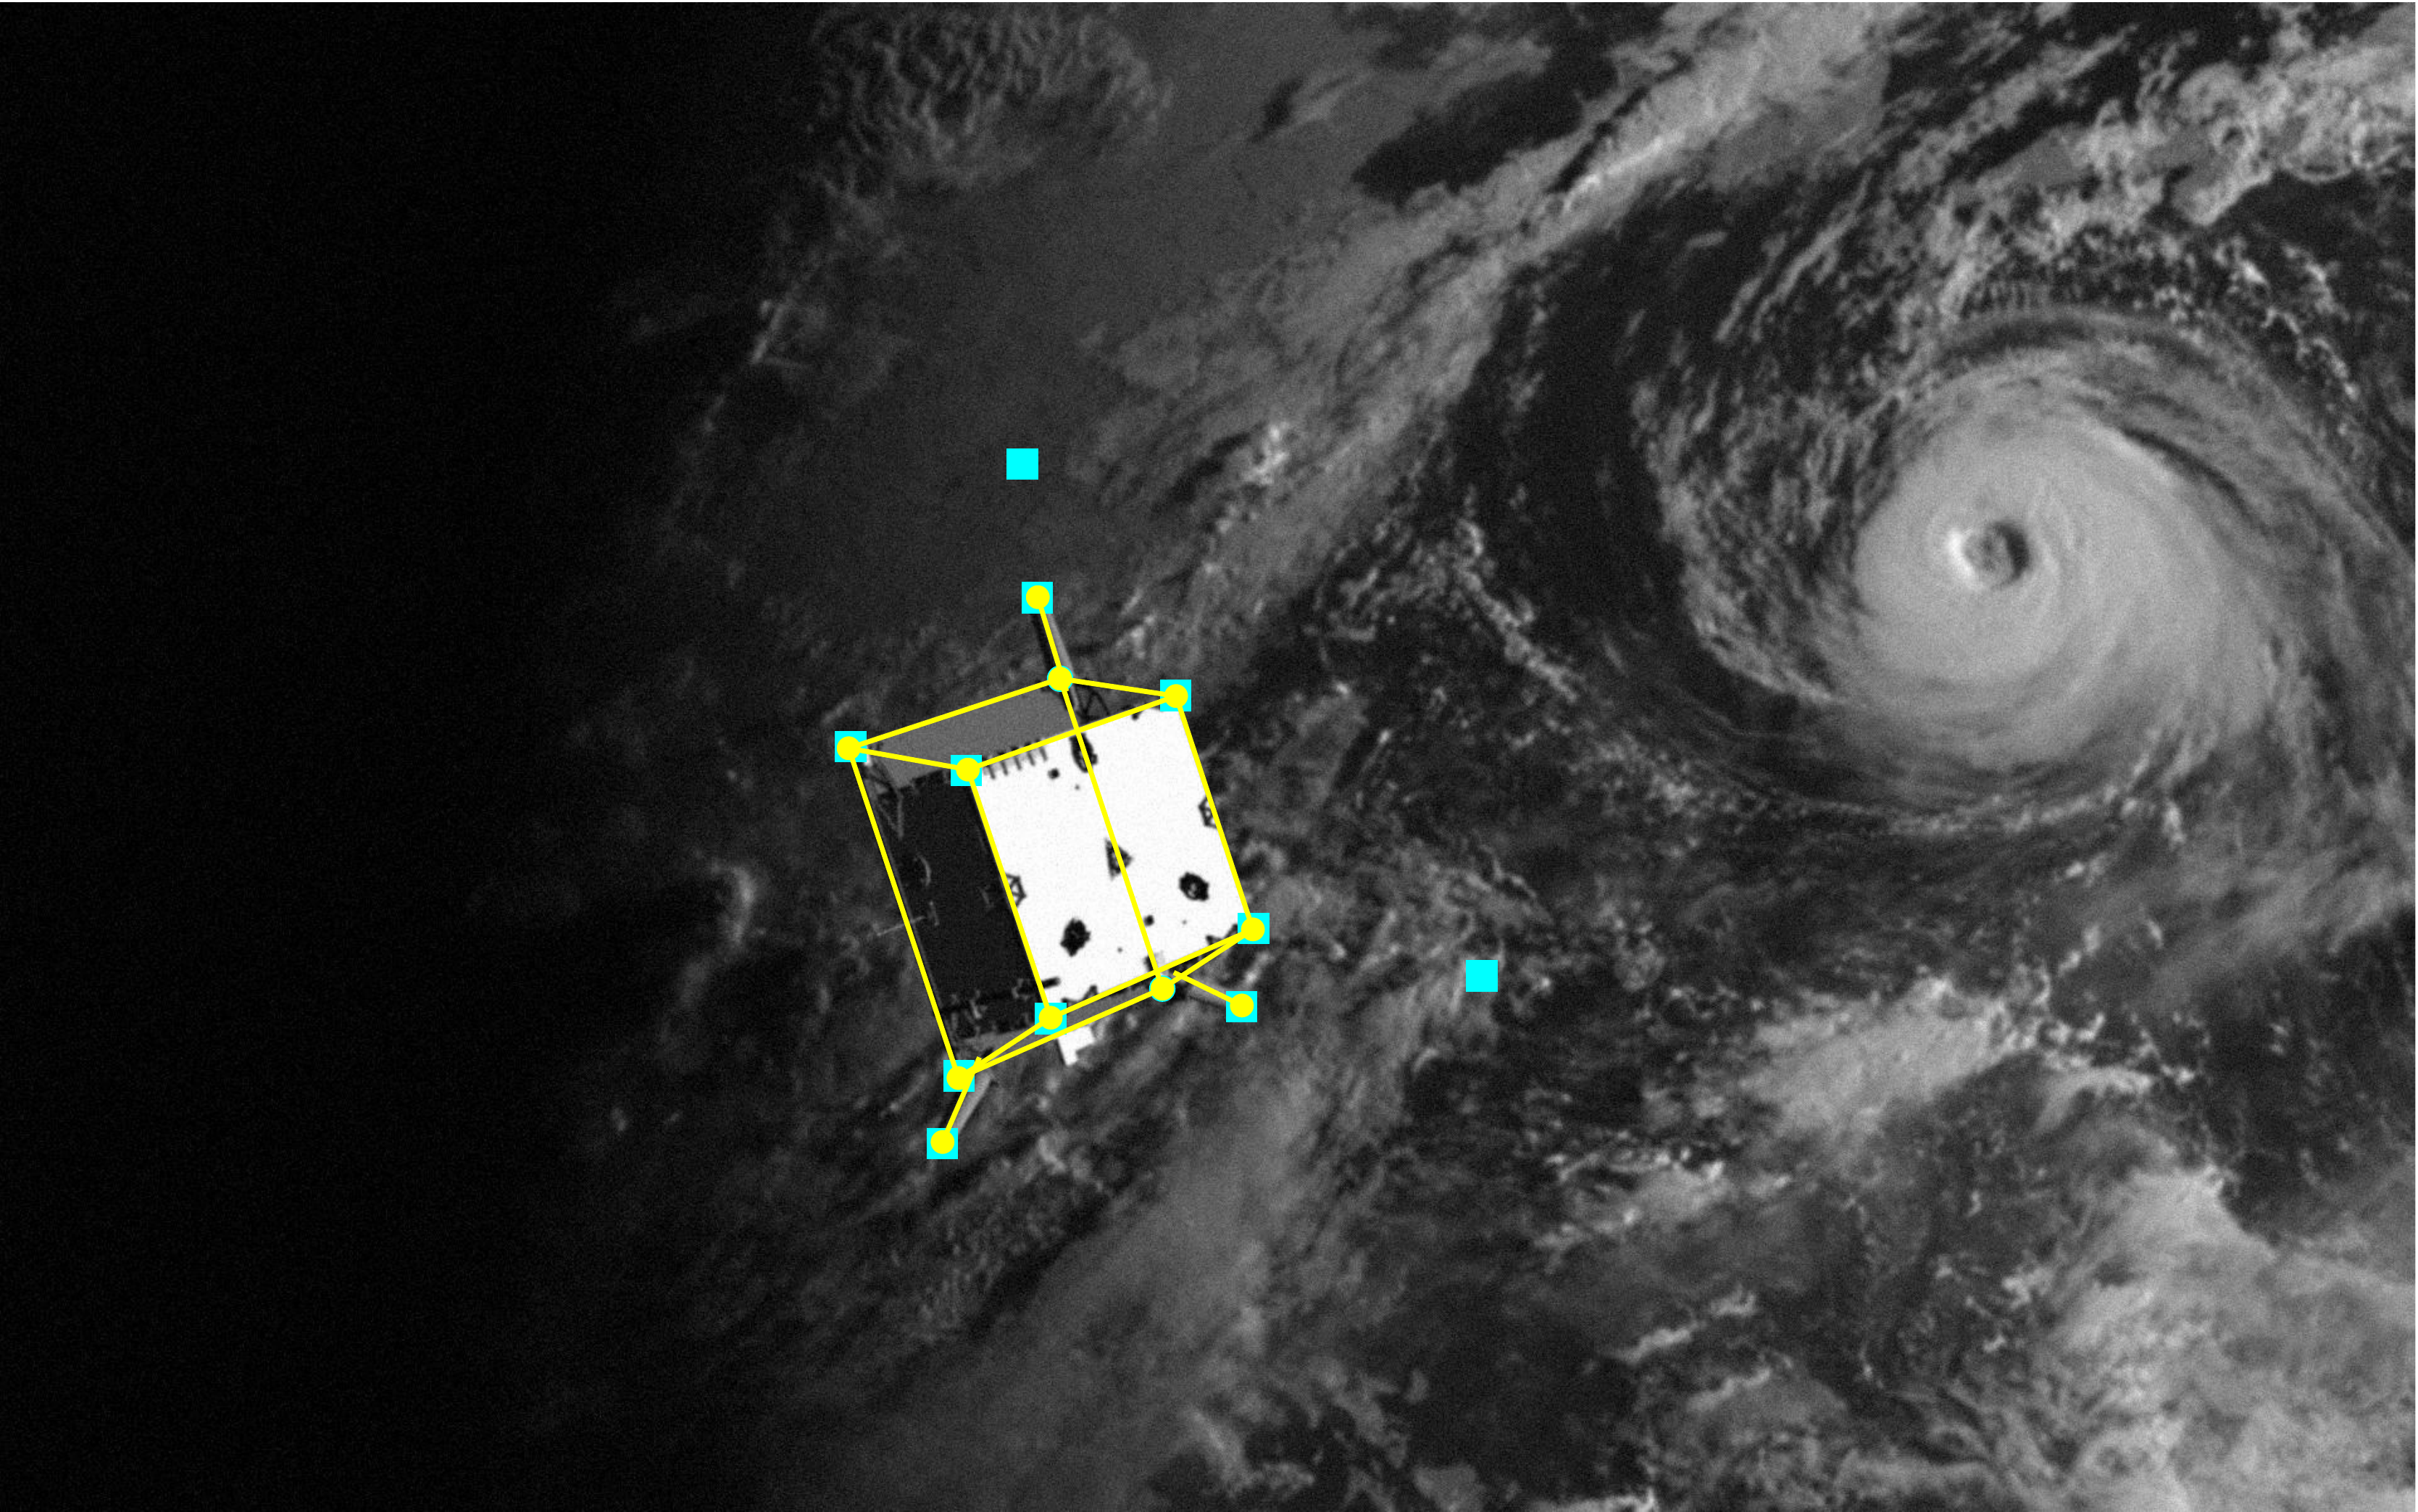}\\
			 $\MR$ error: $0.21^{\circ}$, $\vt$ error: $0.007$ \\ 
			 $\subopt=5.1\ee{-8}$, time: $46$ [s]
			\end{minipage}
		&  
			\begin{minipage}{\mpwfour}%
			\centering%
			\includegraphics[width=\columnwidth]{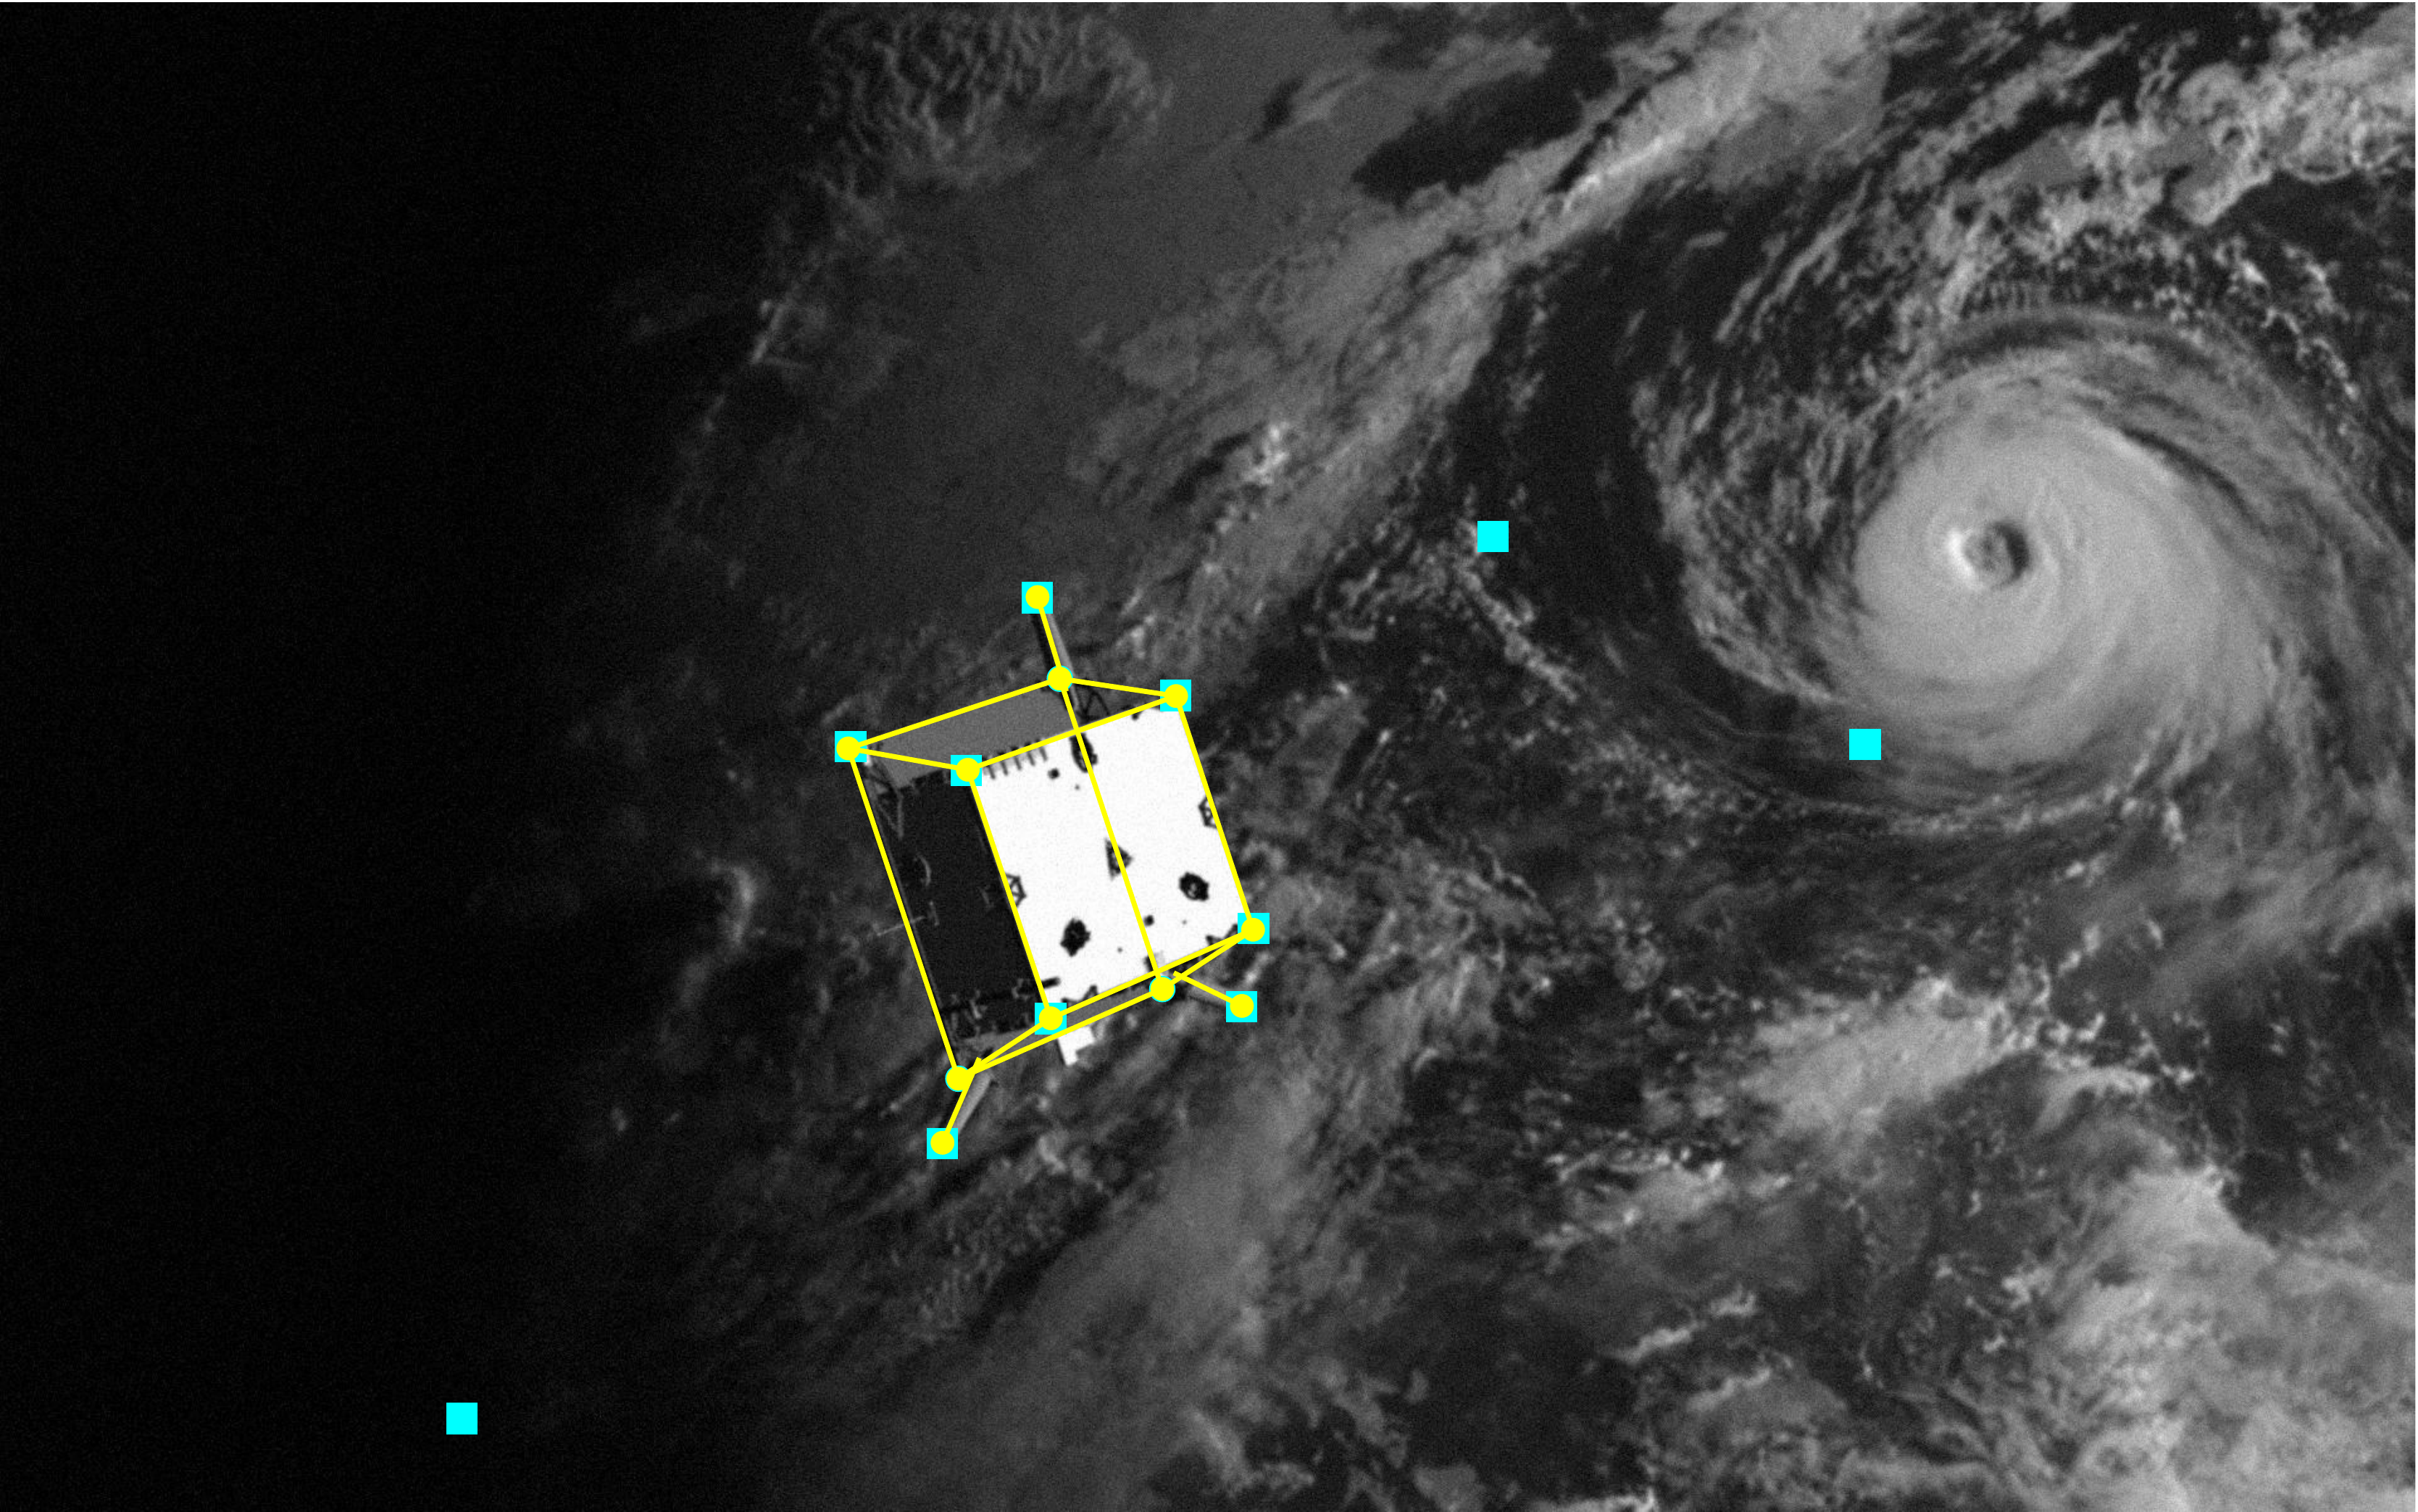}\\
			 $\MR$ error: $0.23^{\circ}$, $\vt$ error: $0.02$ \\ 
			 $\subopt=5.0\ee{-8}$, time: $49$ [s]
			\end{minipage}
		&  
			\begin{minipage}{\mpwfour}%
			\centering%
			\includegraphics[width=\columnwidth]{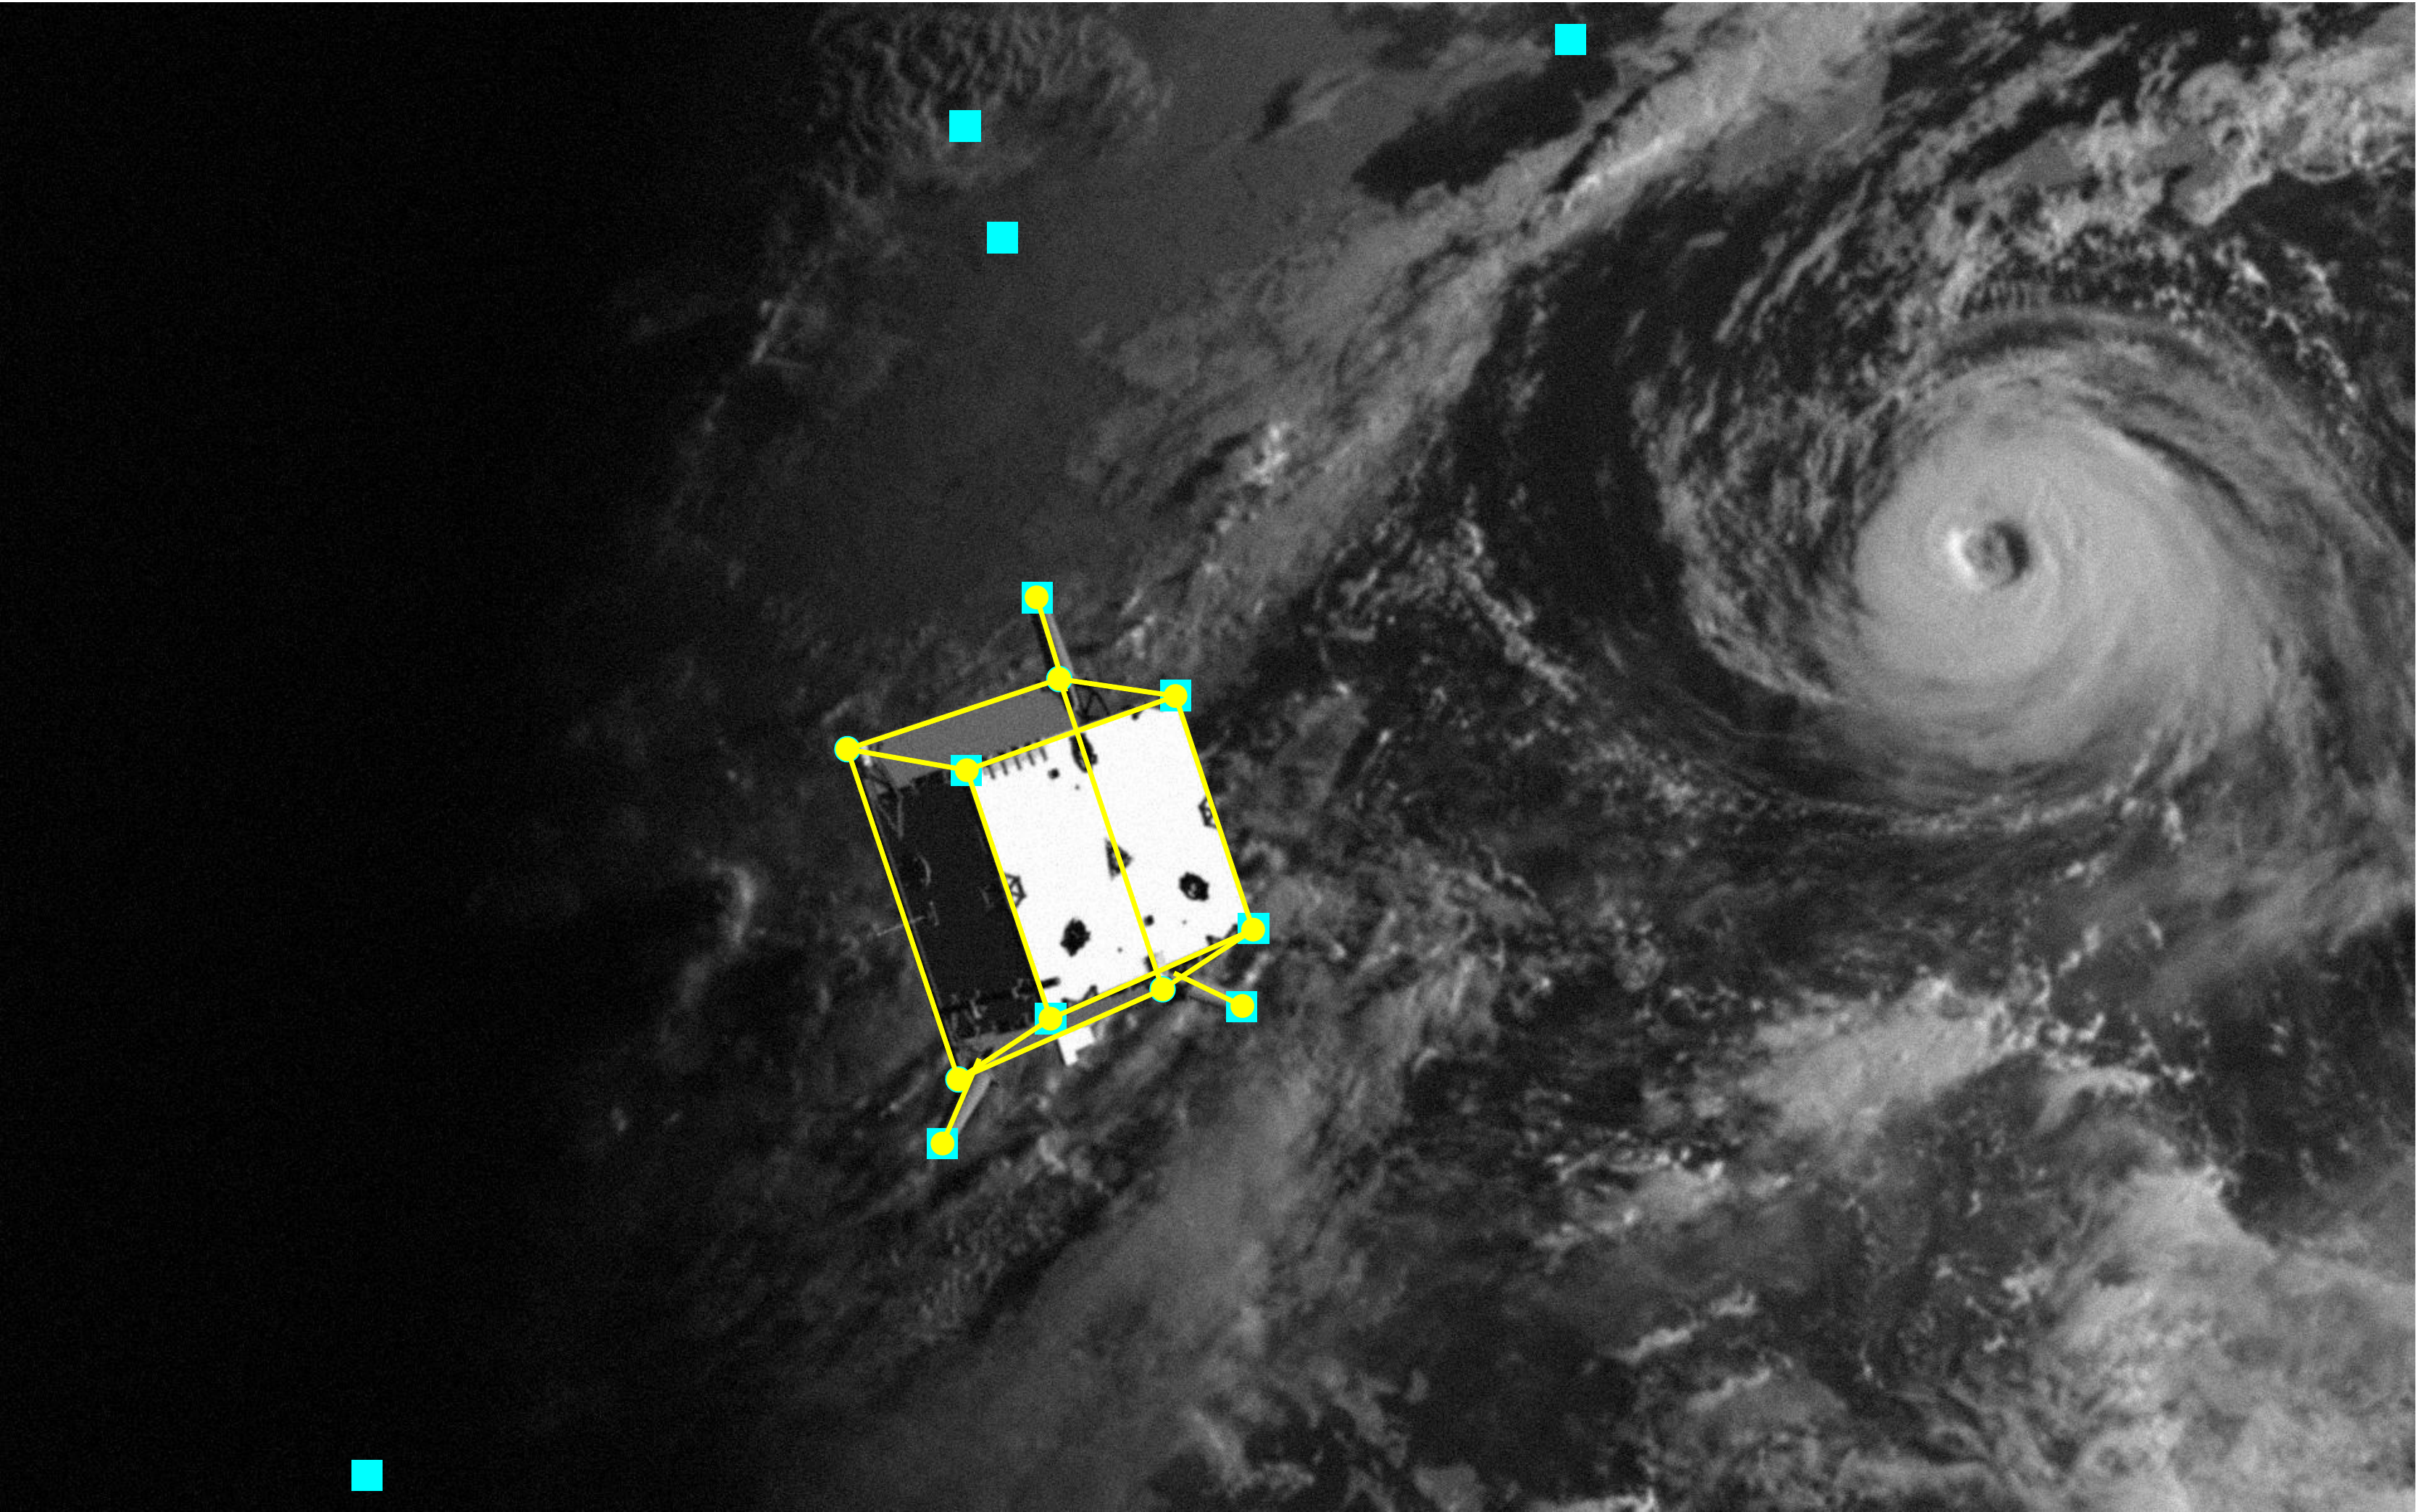}\\
			 $\MR$ error: $0.07^{\circ}$, $\vt$ error: $0.02$ \\ 
			 $\subopt=3.6\ee{-7}$, time: $132$ [s]
			\end{minipage}
		&  
			\begin{minipage}{\mpwfour}%
			\centering%
			\includegraphics[width=\columnwidth]{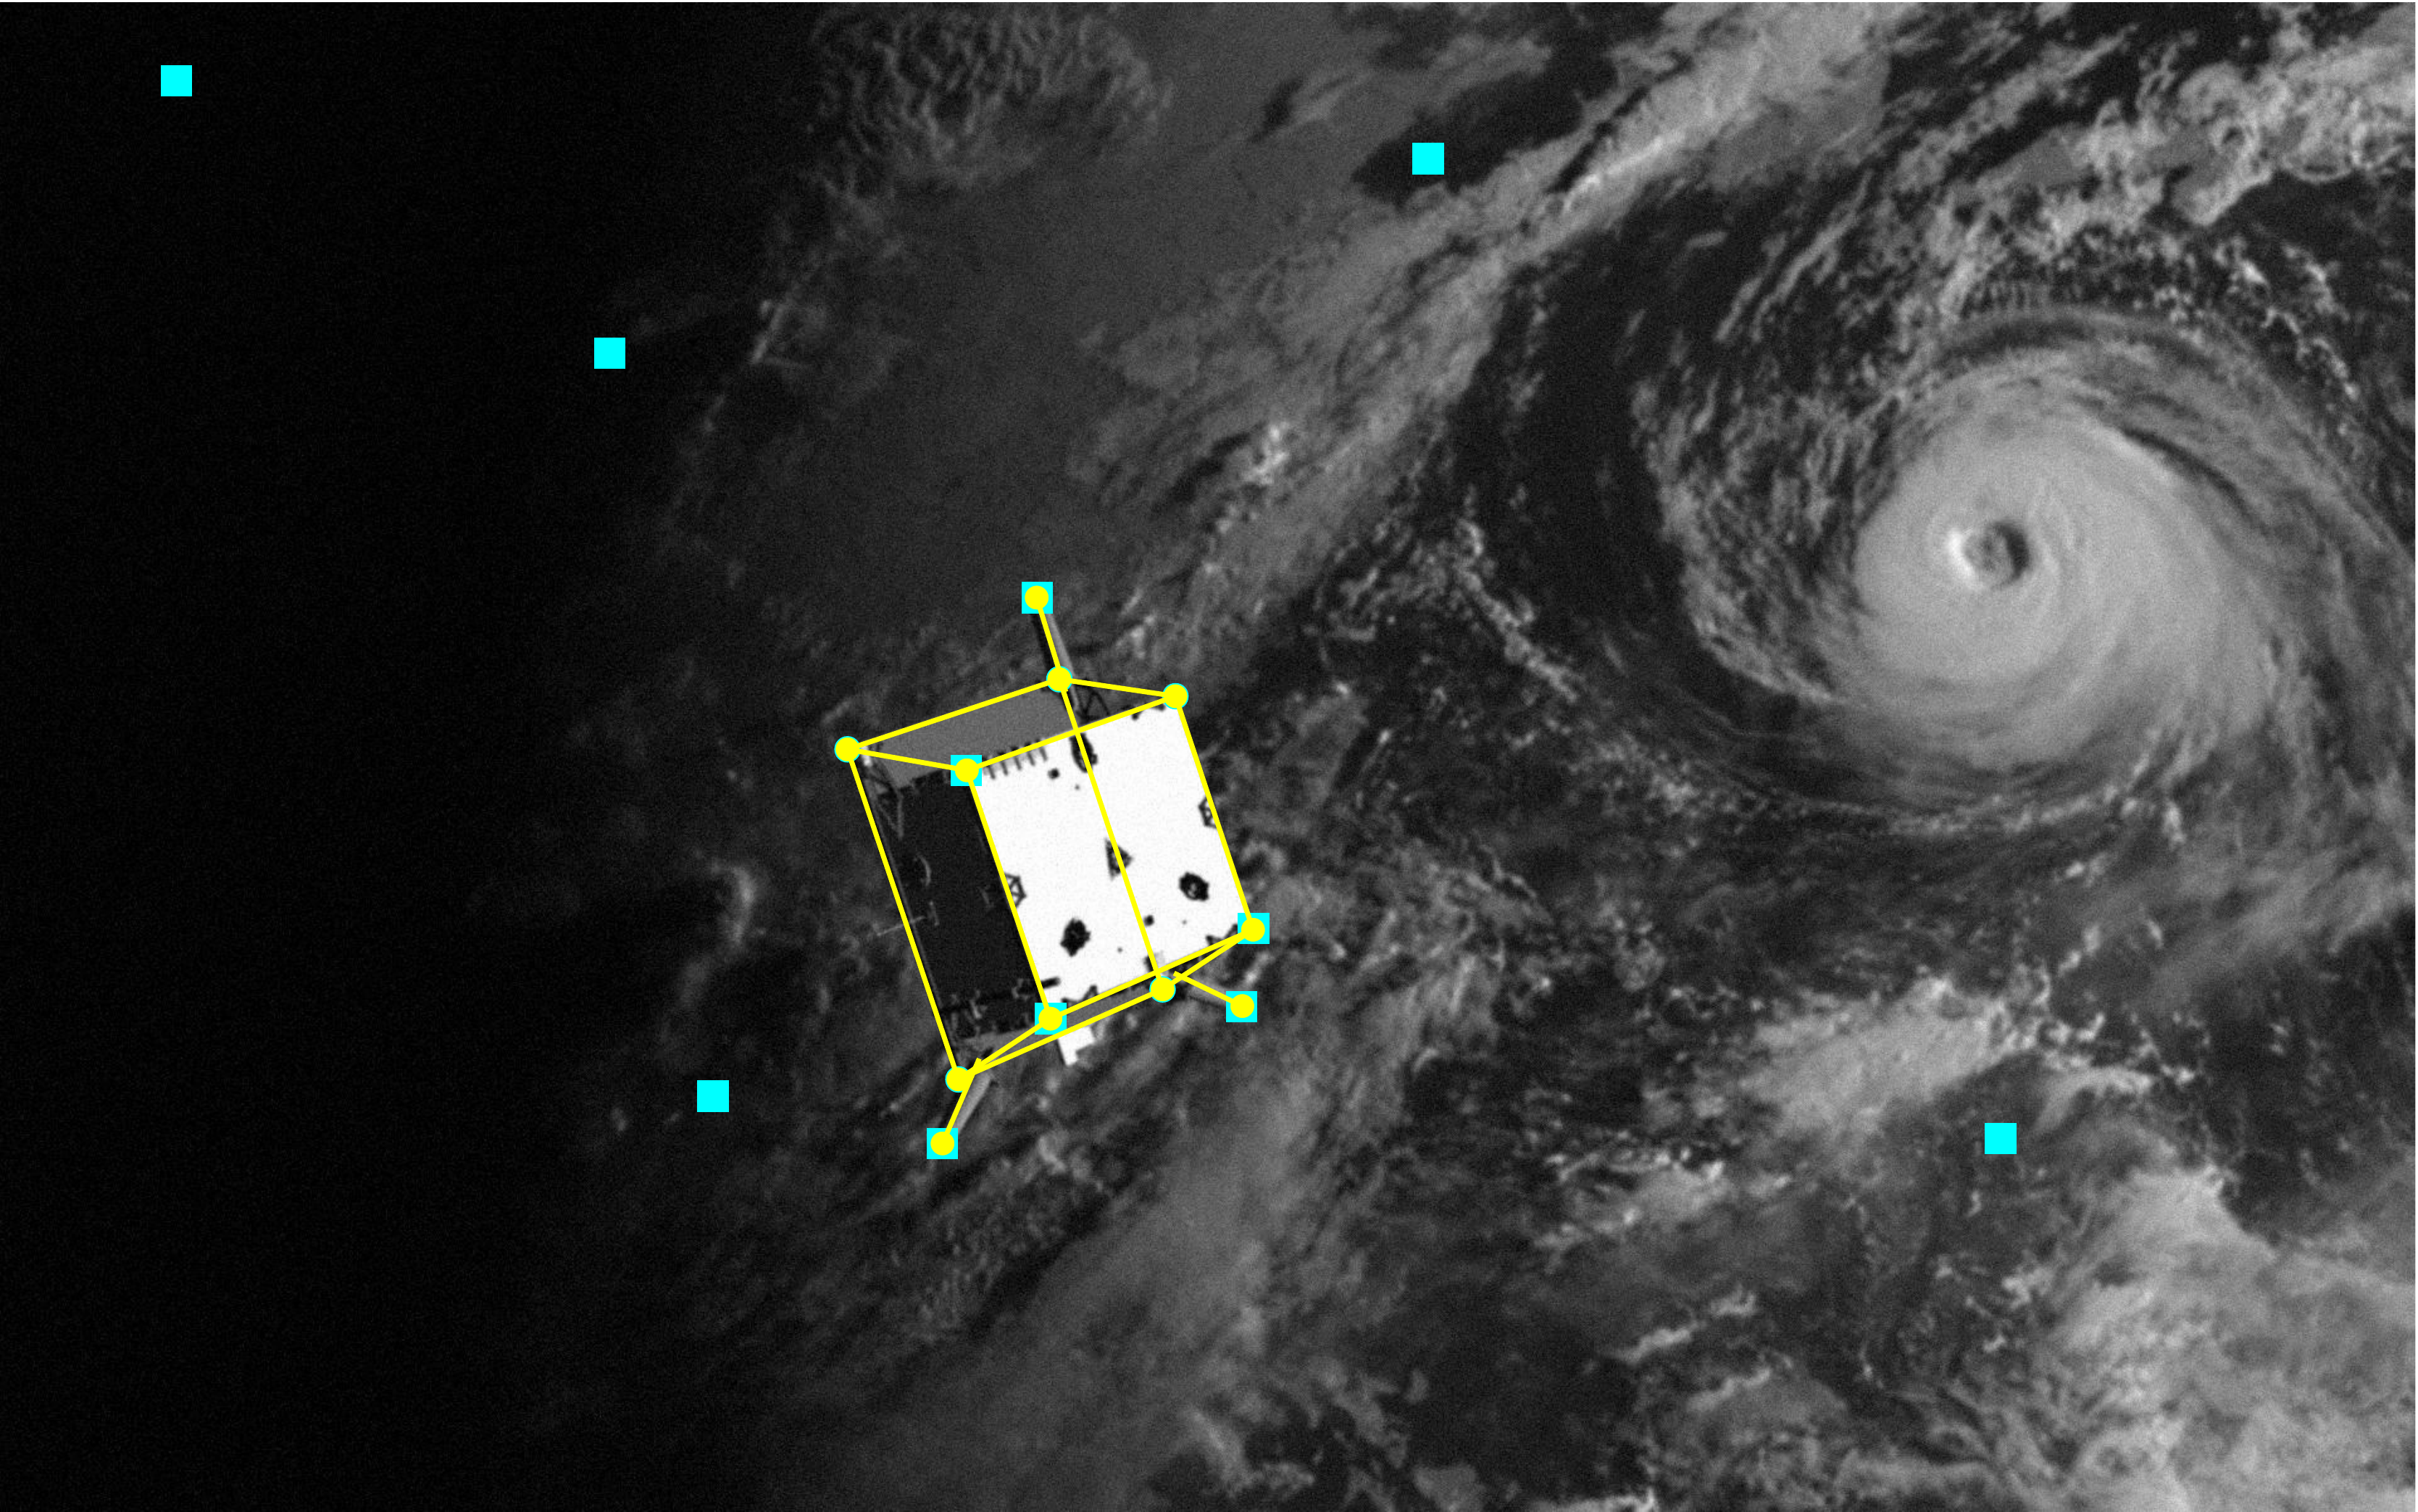}\\
			 $\MR$ error: $0.06^{\circ}$, $\vt$ error: $0.02$ \\ 
			 $\subopt=1.3\ee{-7}$, time: $95$ [s]
			\end{minipage} \vspace{1mm}
		\\

		%%%%%%%%%%%%%%%%%%%%%%%%%%%%%%%%%%%%%%%%%%%%%%%%%%%%%%%%%%%%%%%%%%%%%%%%%%%%%%%%%%%%%%%%%%%%%%%%%%%%%%%%%
			\begin{minipage}{\mpwfour}%
			\centering%
			\includegraphics[width=\columnwidth]{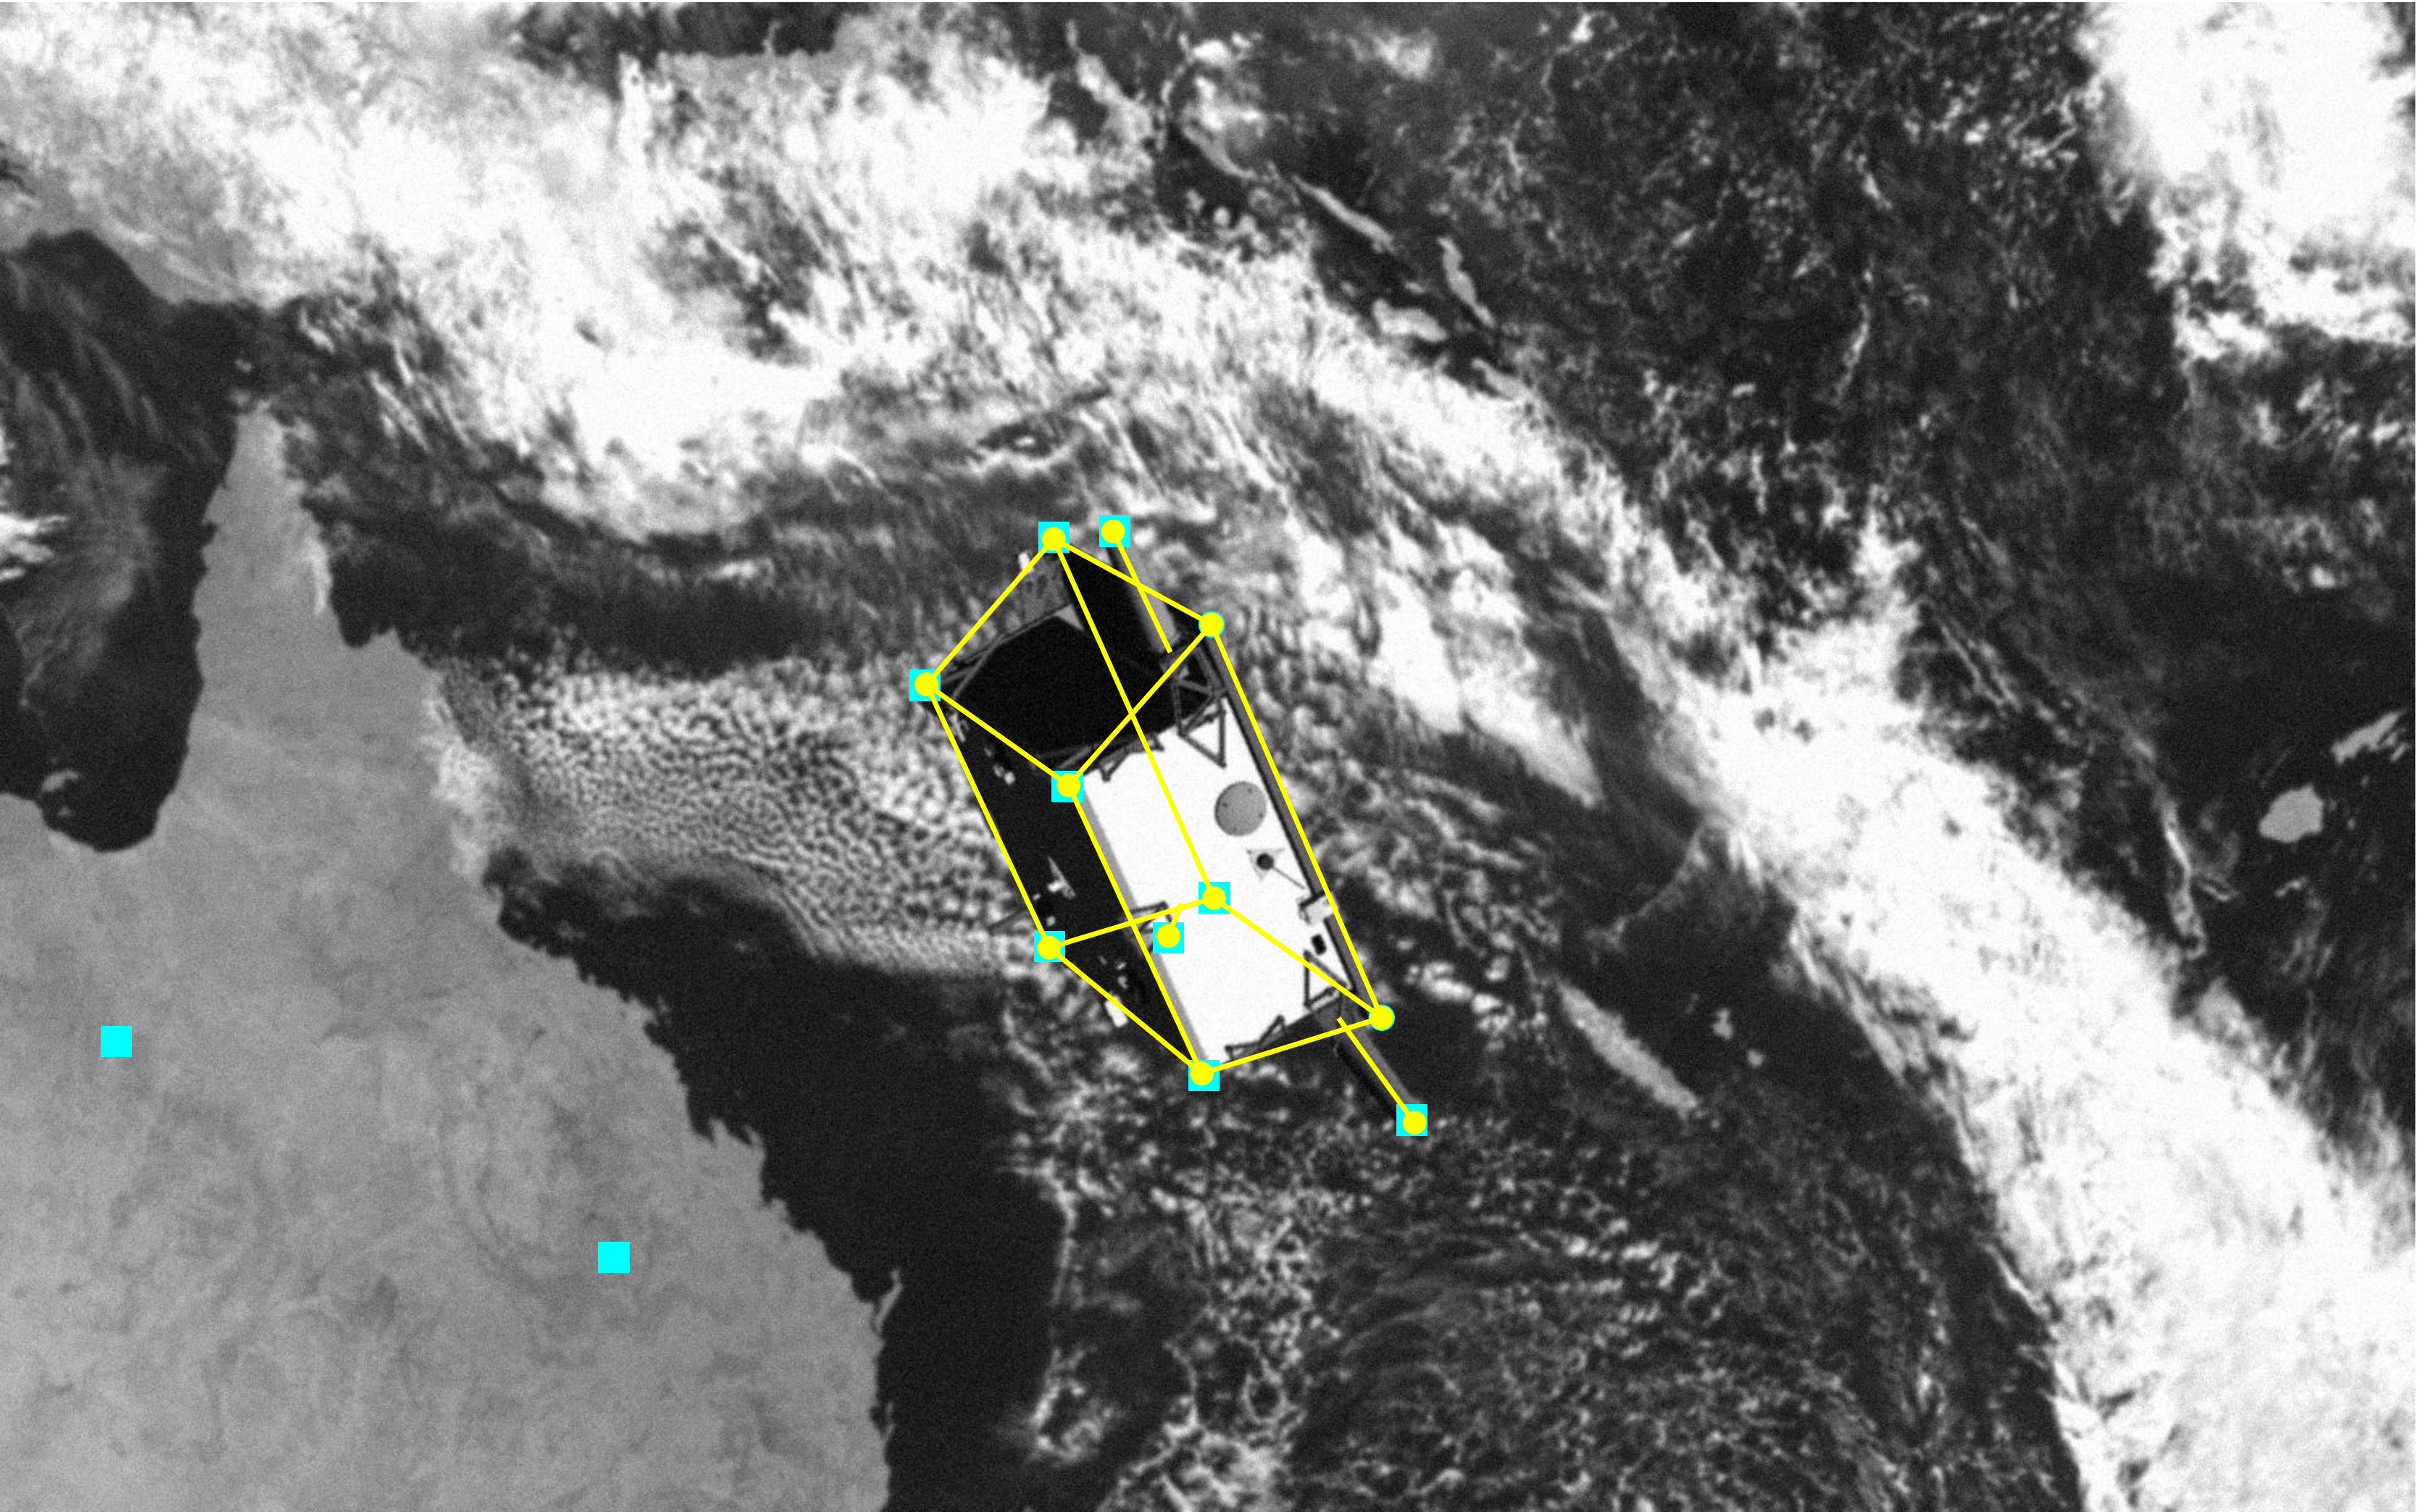}\\
			 $\MR$ error: $0.28^{\circ}$, $\vt$ error: $0.02$ \\ 
			 $\subopt=3.9\ee{-8}$, time: $46$ [s]
			\end{minipage}
		&  
			\begin{minipage}{\mpwfour}%
			\centering%
			\includegraphics[width=\columnwidth]{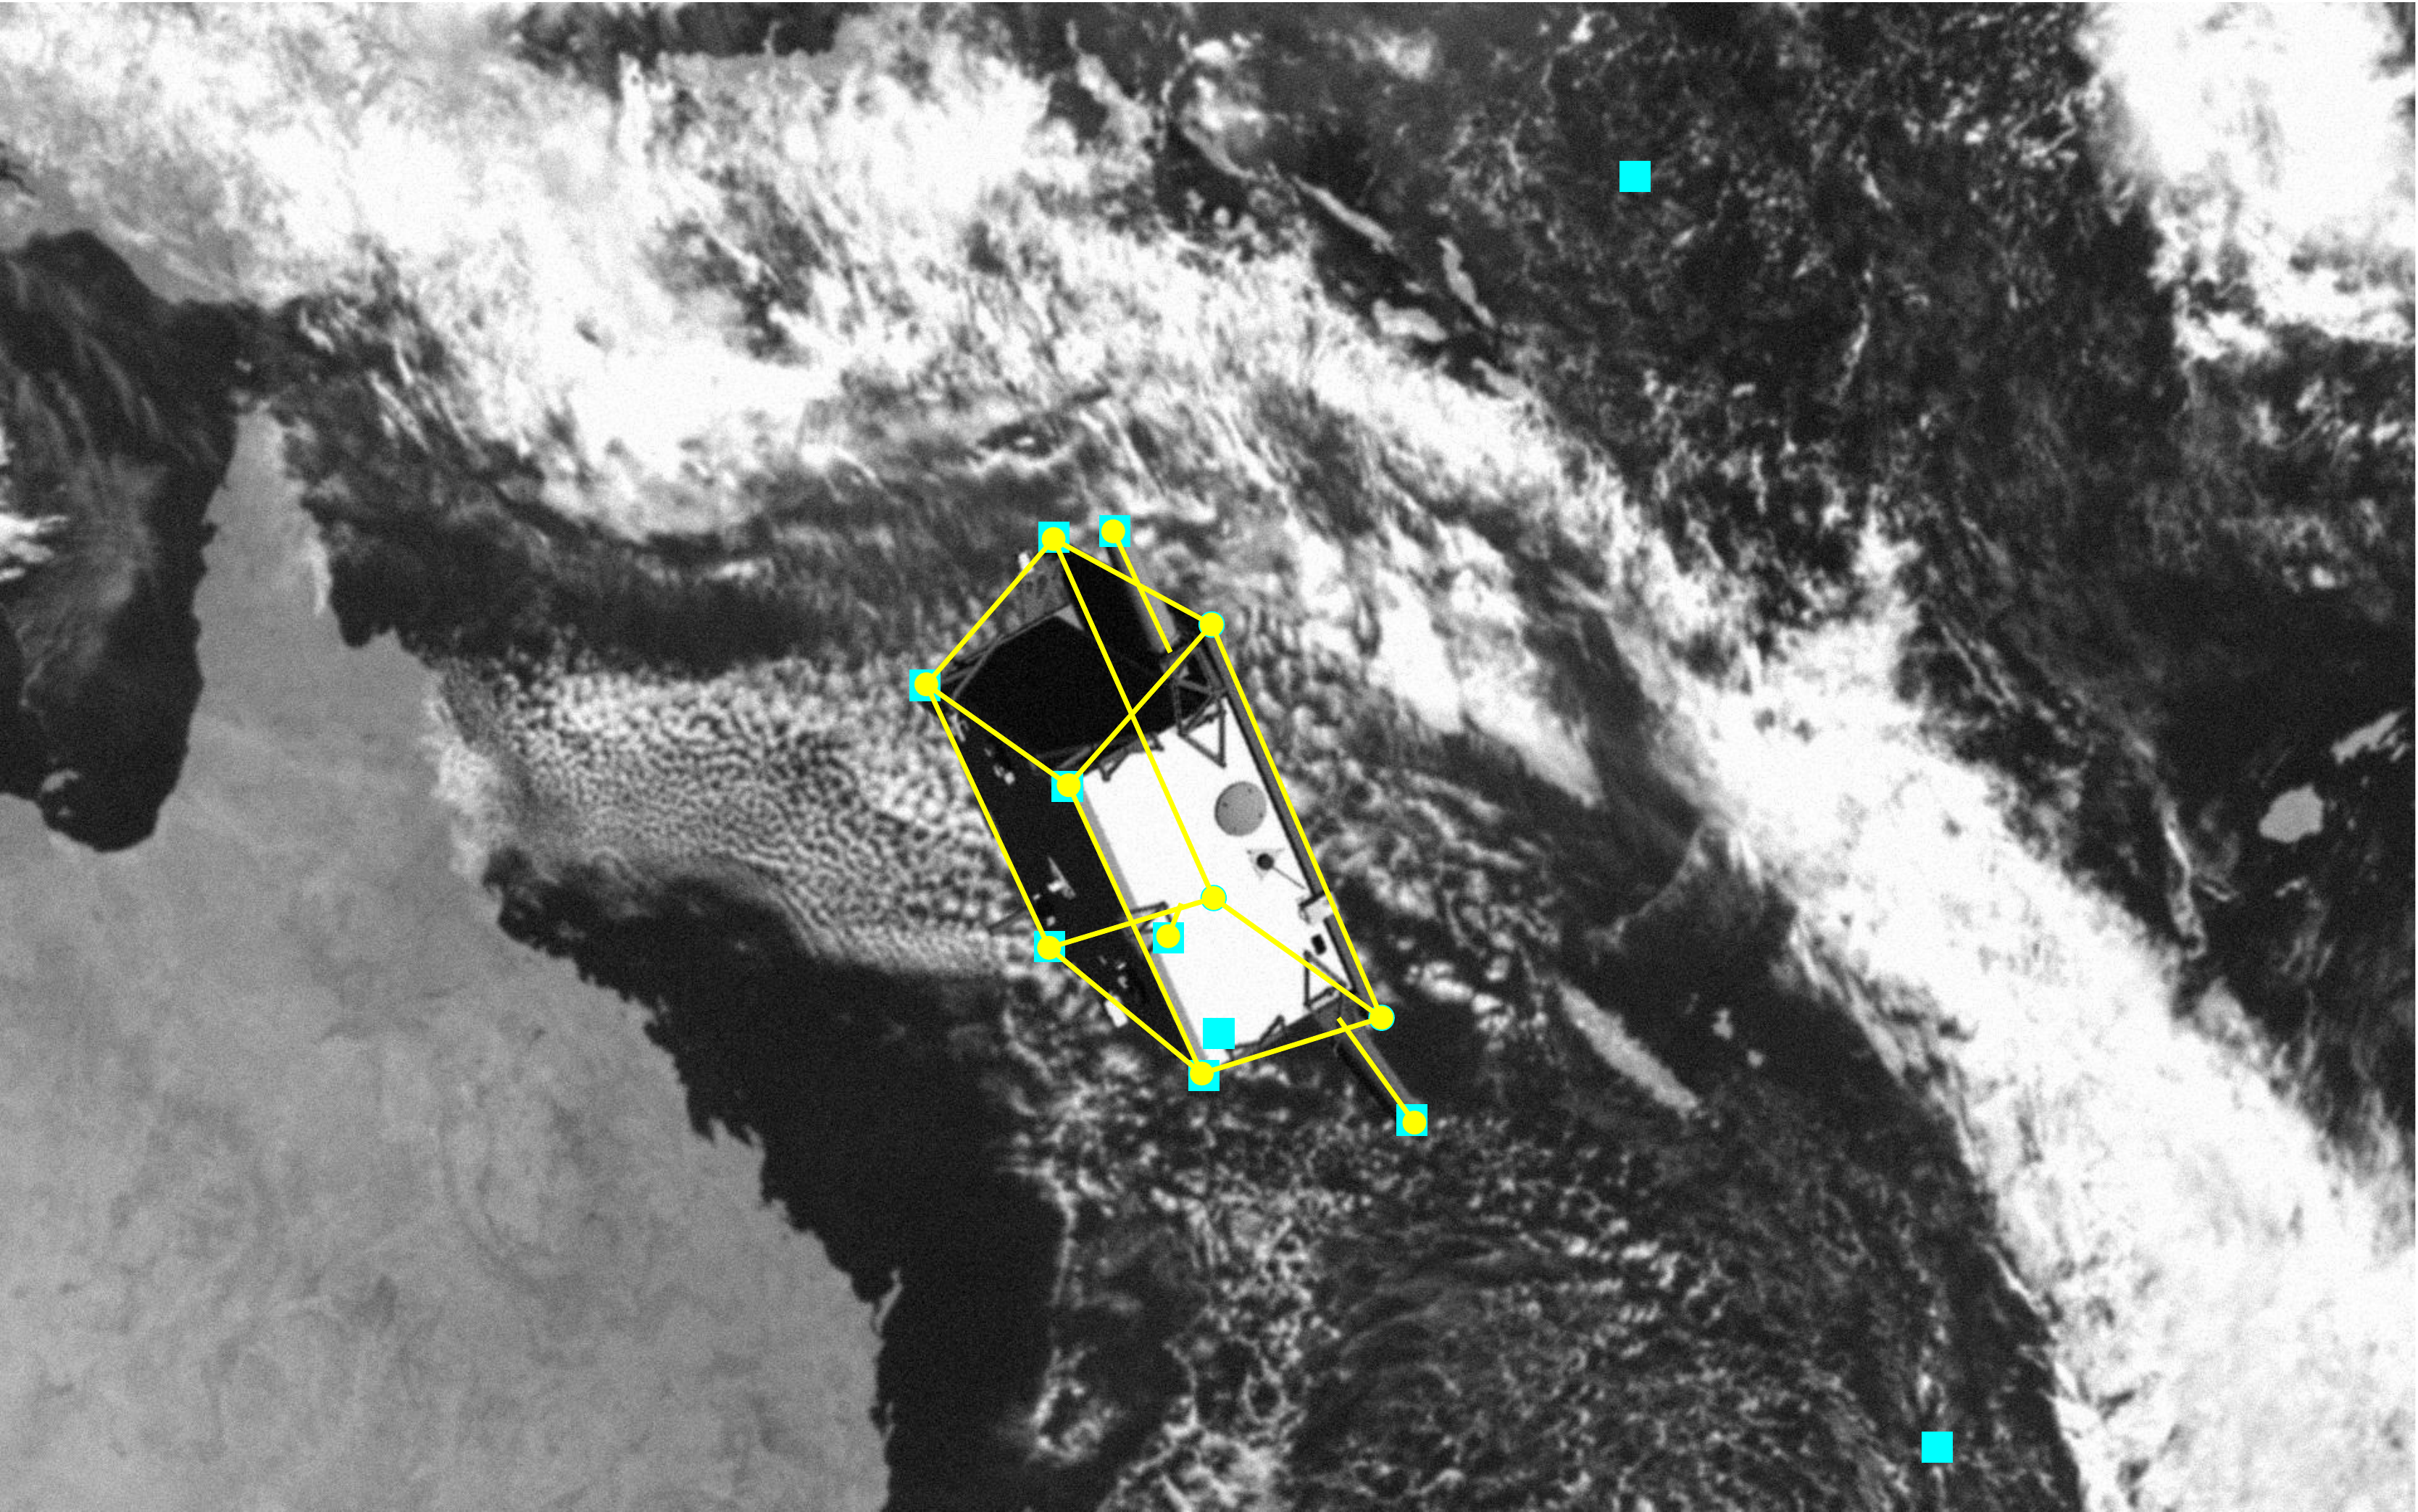}\\
			 $\MR$ error: $0.30^{\circ}$, $\vt$ error: $0.02$ \\ 
			 $\subopt=5.1\ee{-8}$, time: $47$ [s]
			\end{minipage}
		&  
			\begin{minipage}{\mpwfour}%
			\centering%
			\includegraphics[width=\columnwidth]{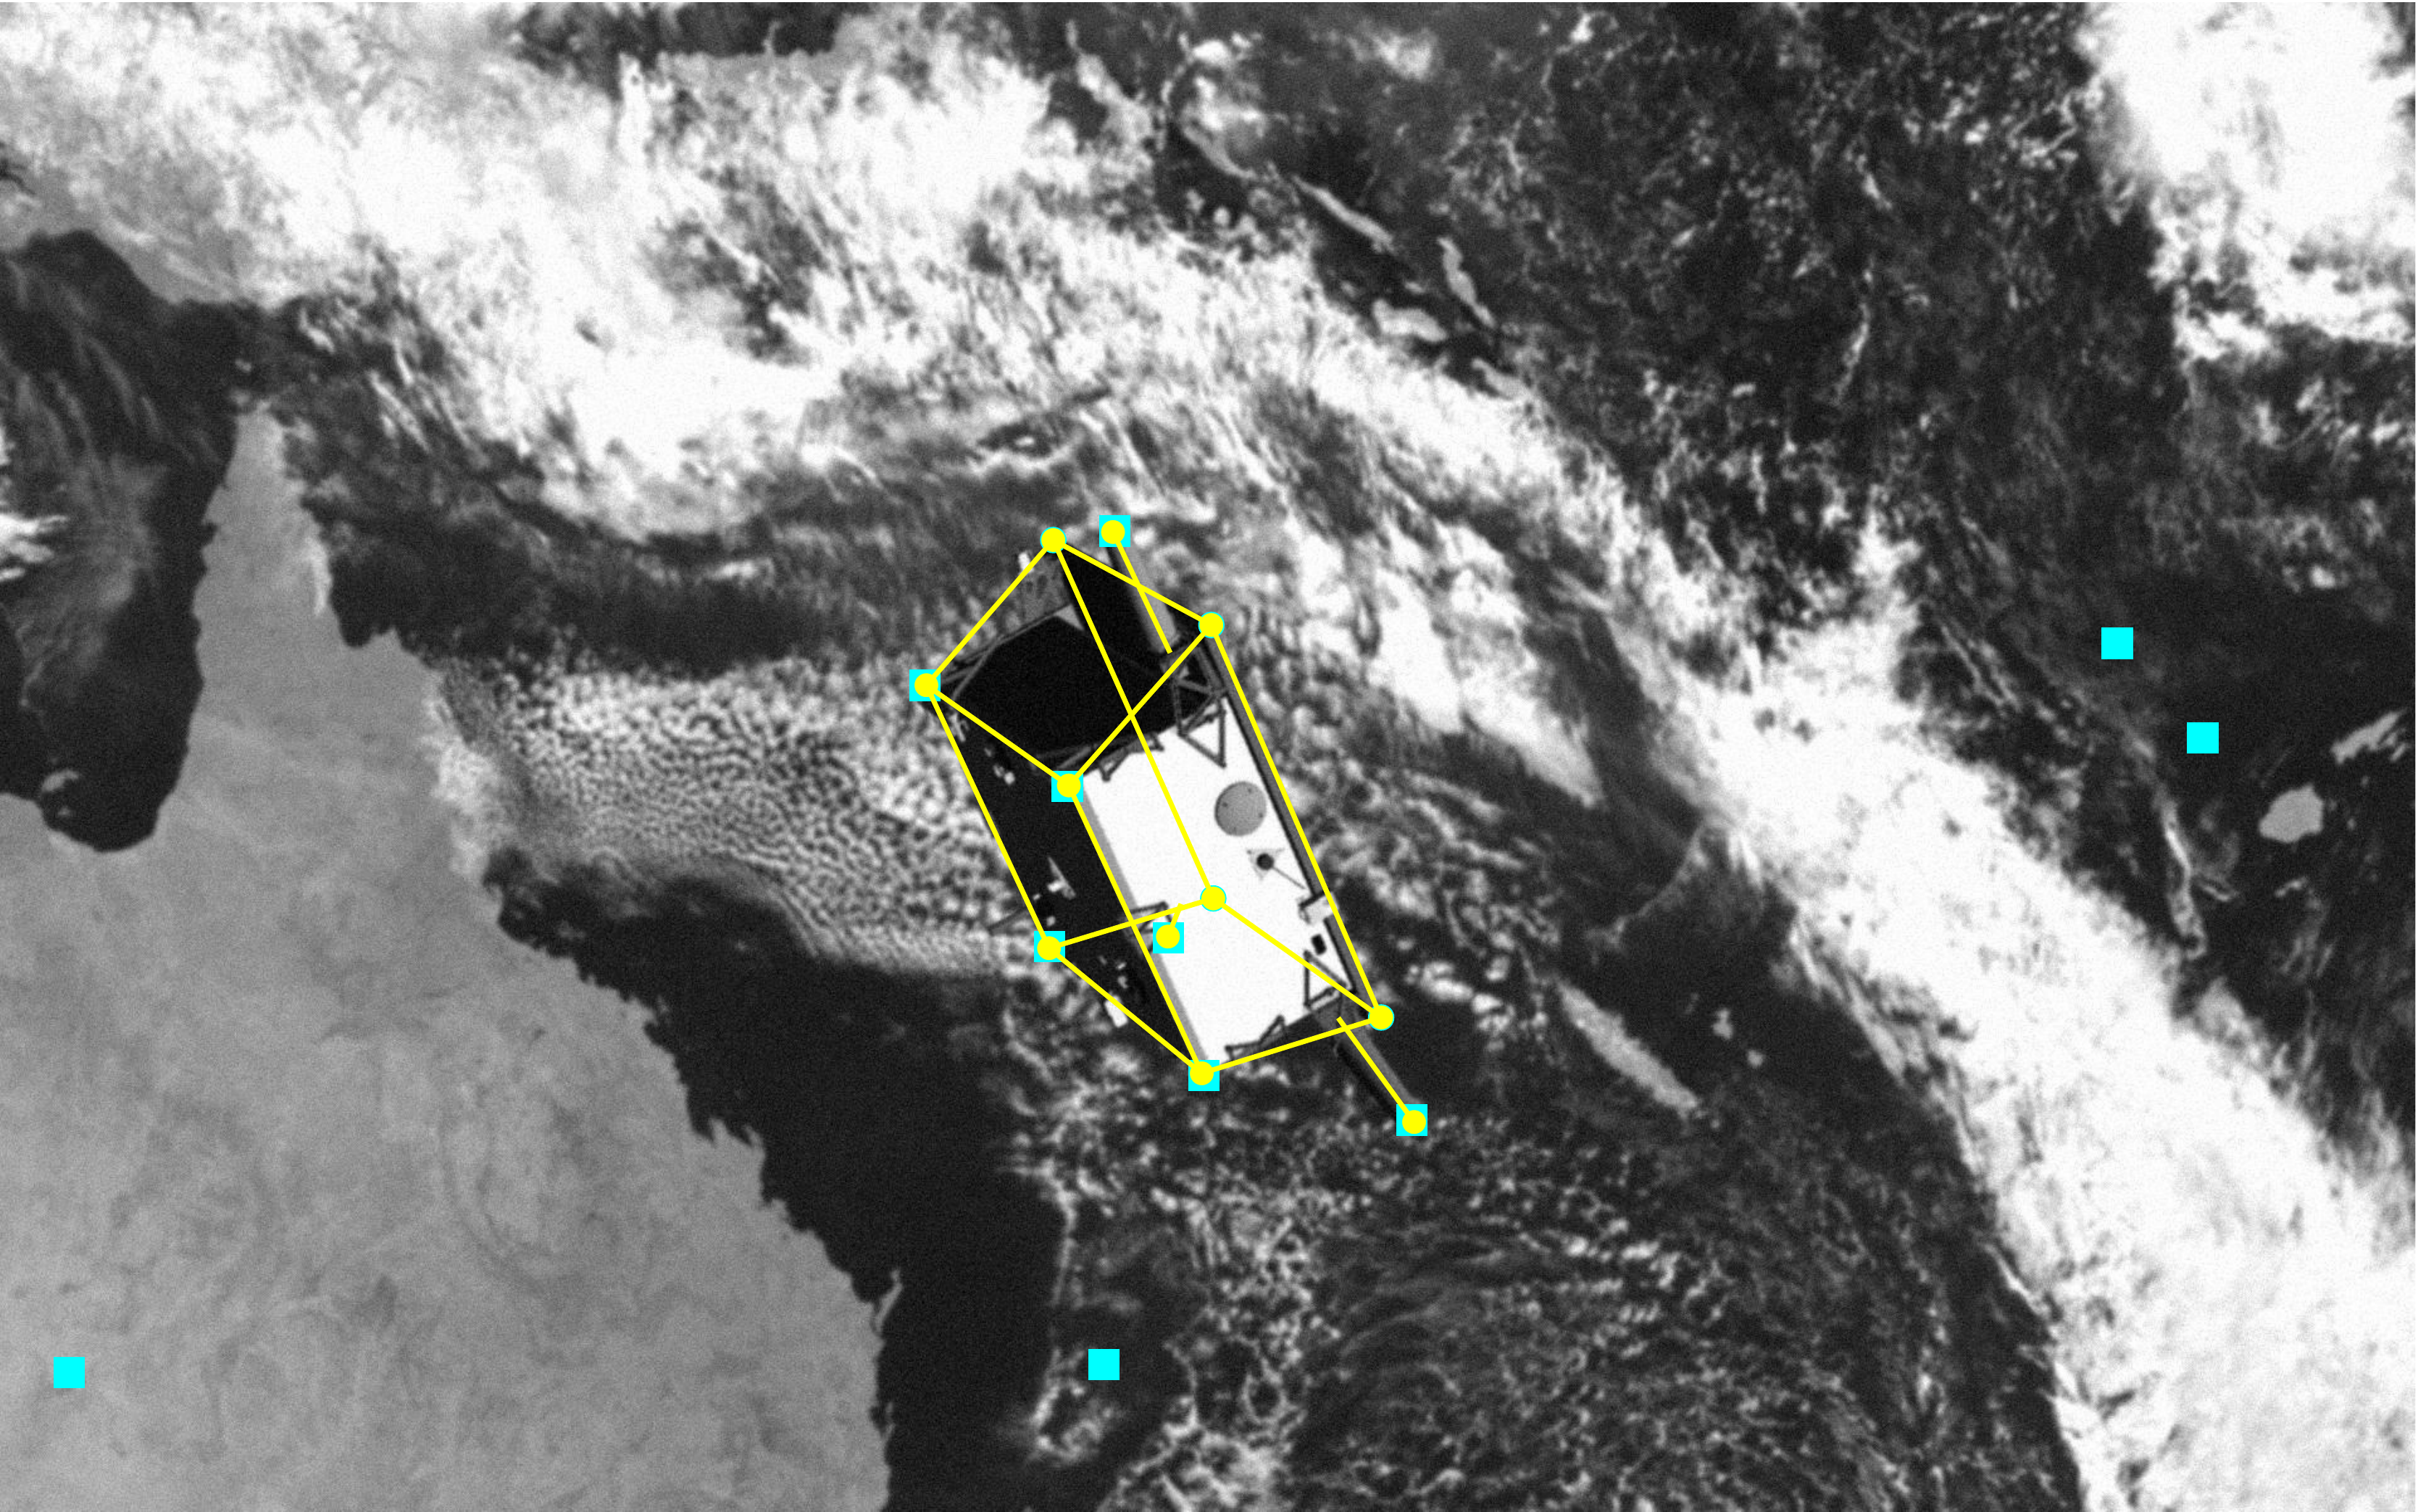}\\
			 $\MR$ error: $0.37^{\circ}$, $\vt$ error: $0.04$ \\ 
			 $\subopt=8.0\ee{-8}$, time: $93$ [s]
			\end{minipage}
		&  
			\begin{minipage}{\mpwfour}%
			\centering%
			\includegraphics[width=\columnwidth]{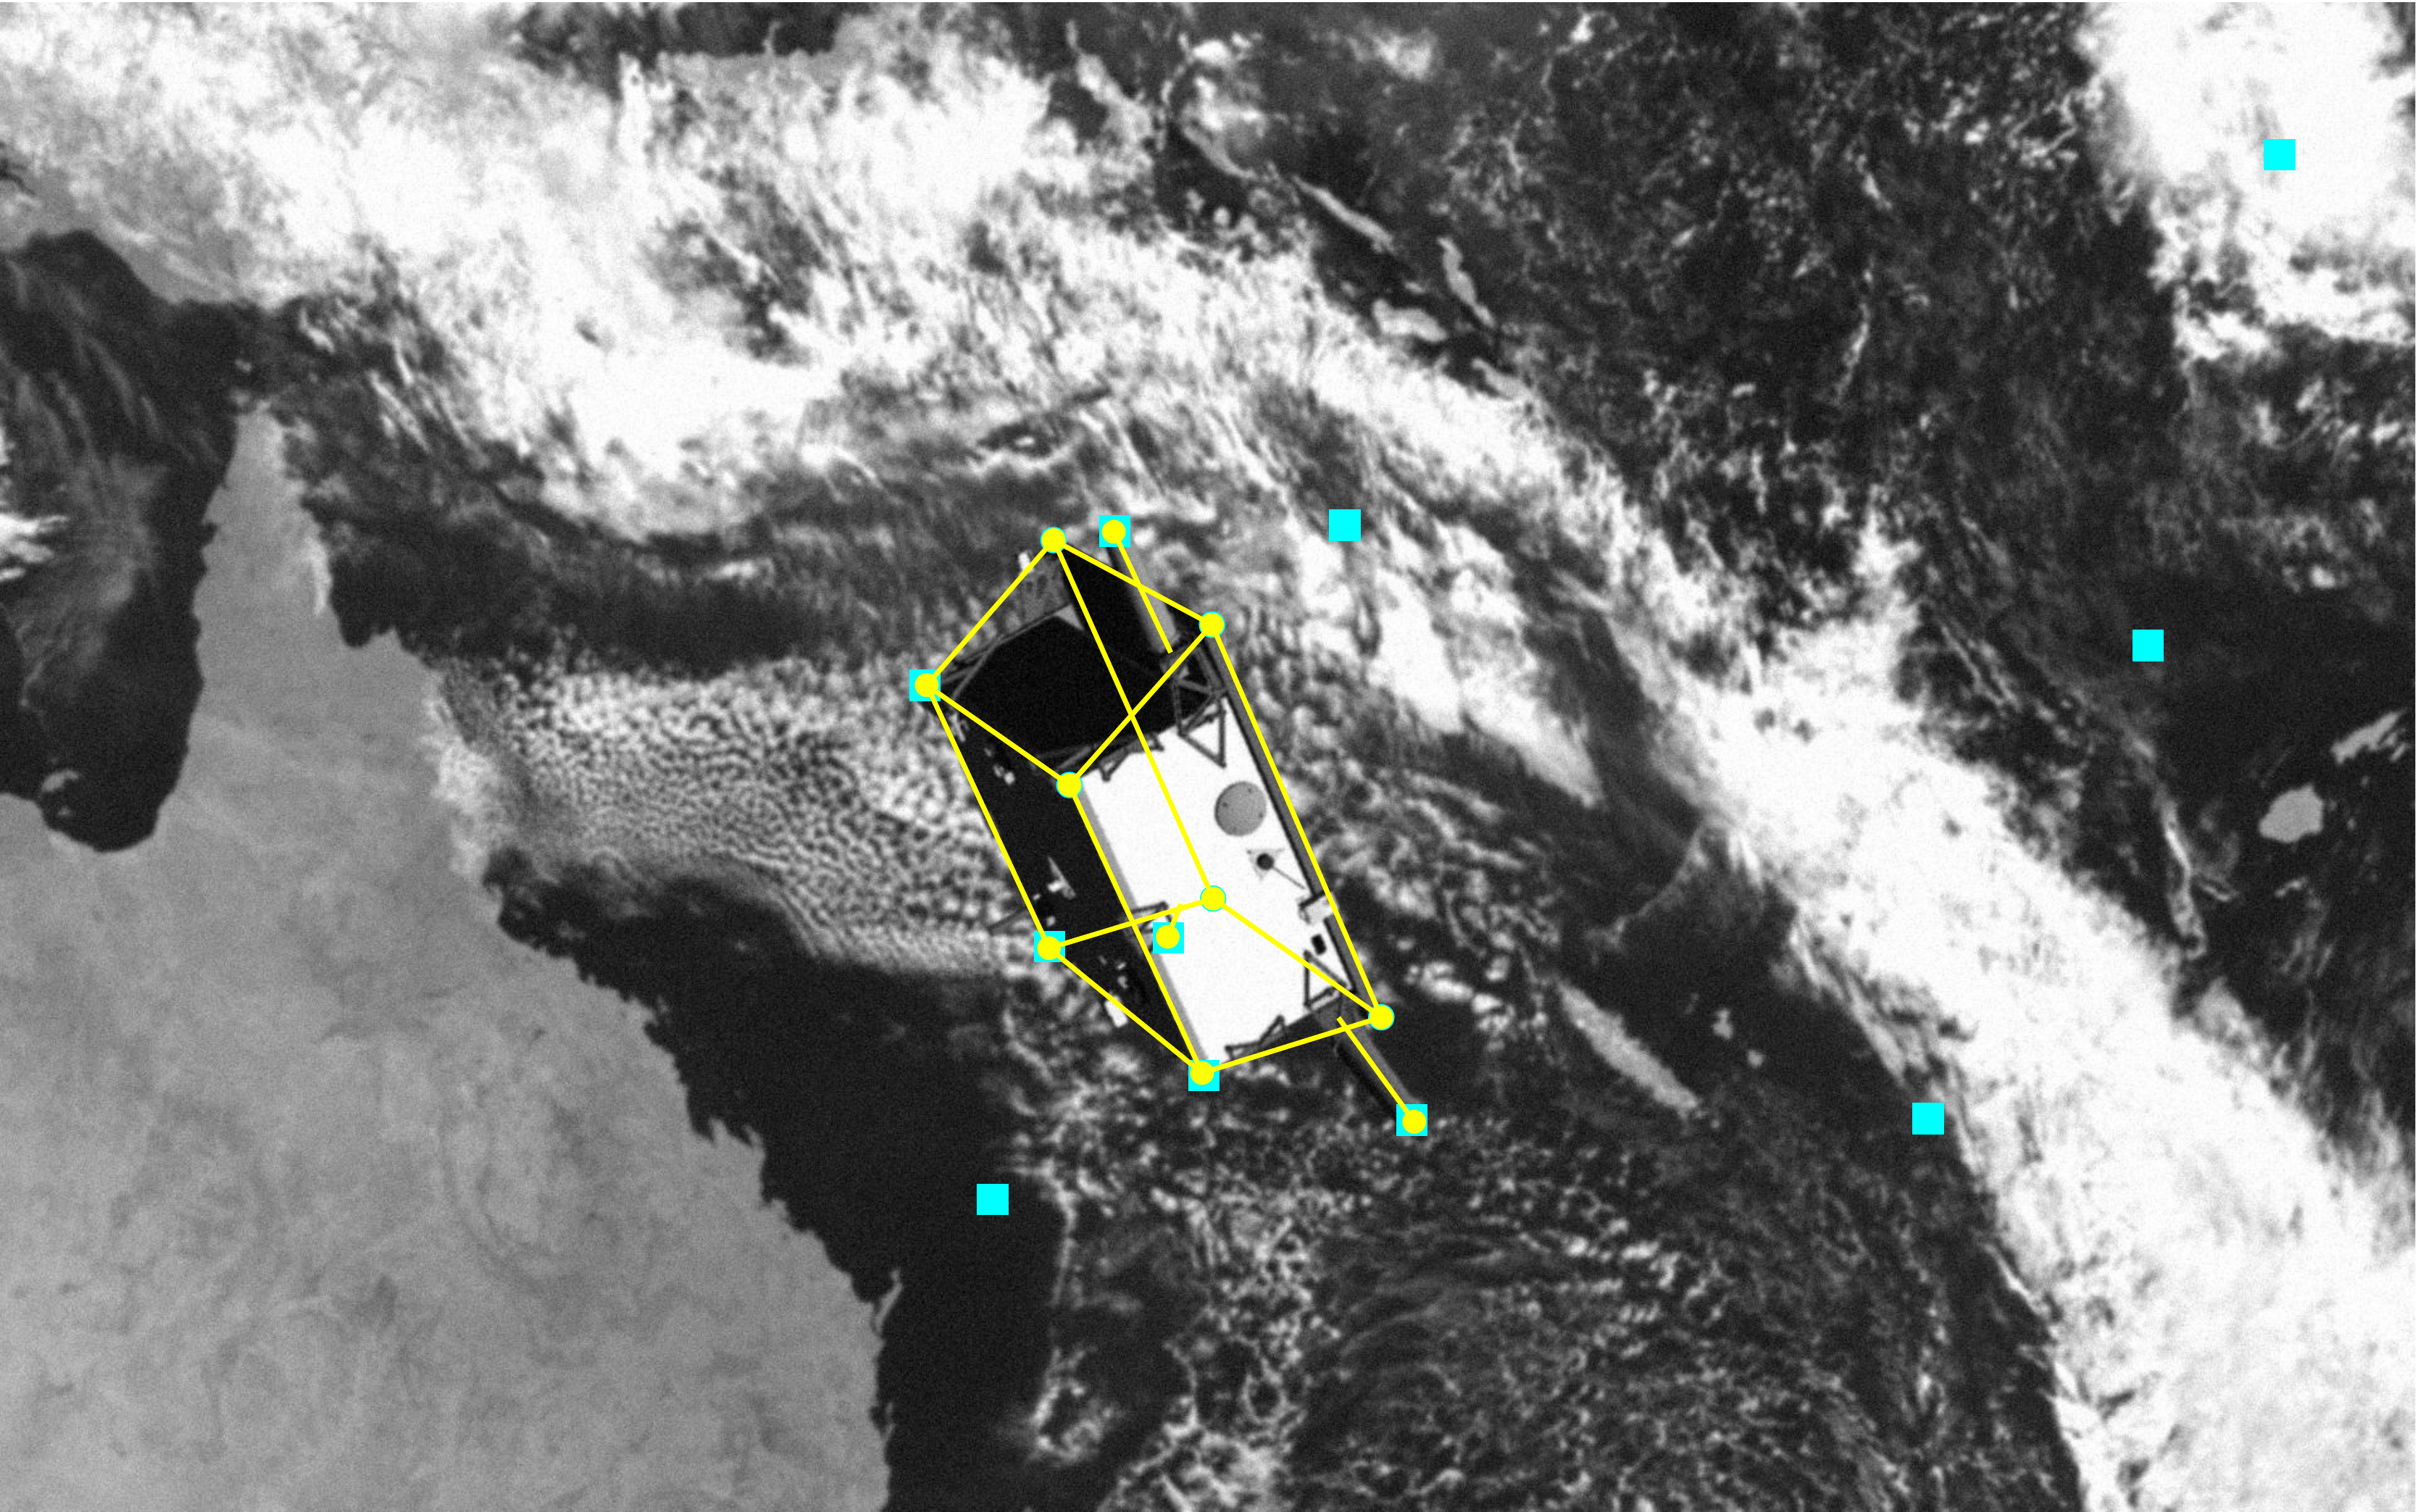}\\
			 $\MR$ error: $0.43^{\circ}$, $\vt$ error: $0.04$ \\ 
			 $\subopt=1.6\ee{-6}$, time: $155$ [s]
			\end{minipage} \vspace{1mm}
		\\

		%%%%%%%%%%%%%%%%%%%%%%%%%%%%%%%%%%%%%%%%%%%%%%%%%%%%%%%%%%%%%%%%%%%%%%%%%%%%%%%%%%%%%%%%%%%%%%%%%%%%%%%%%
			\begin{minipage}{\mpwfour}%
			\centering%
			\includegraphics[width=\columnwidth]{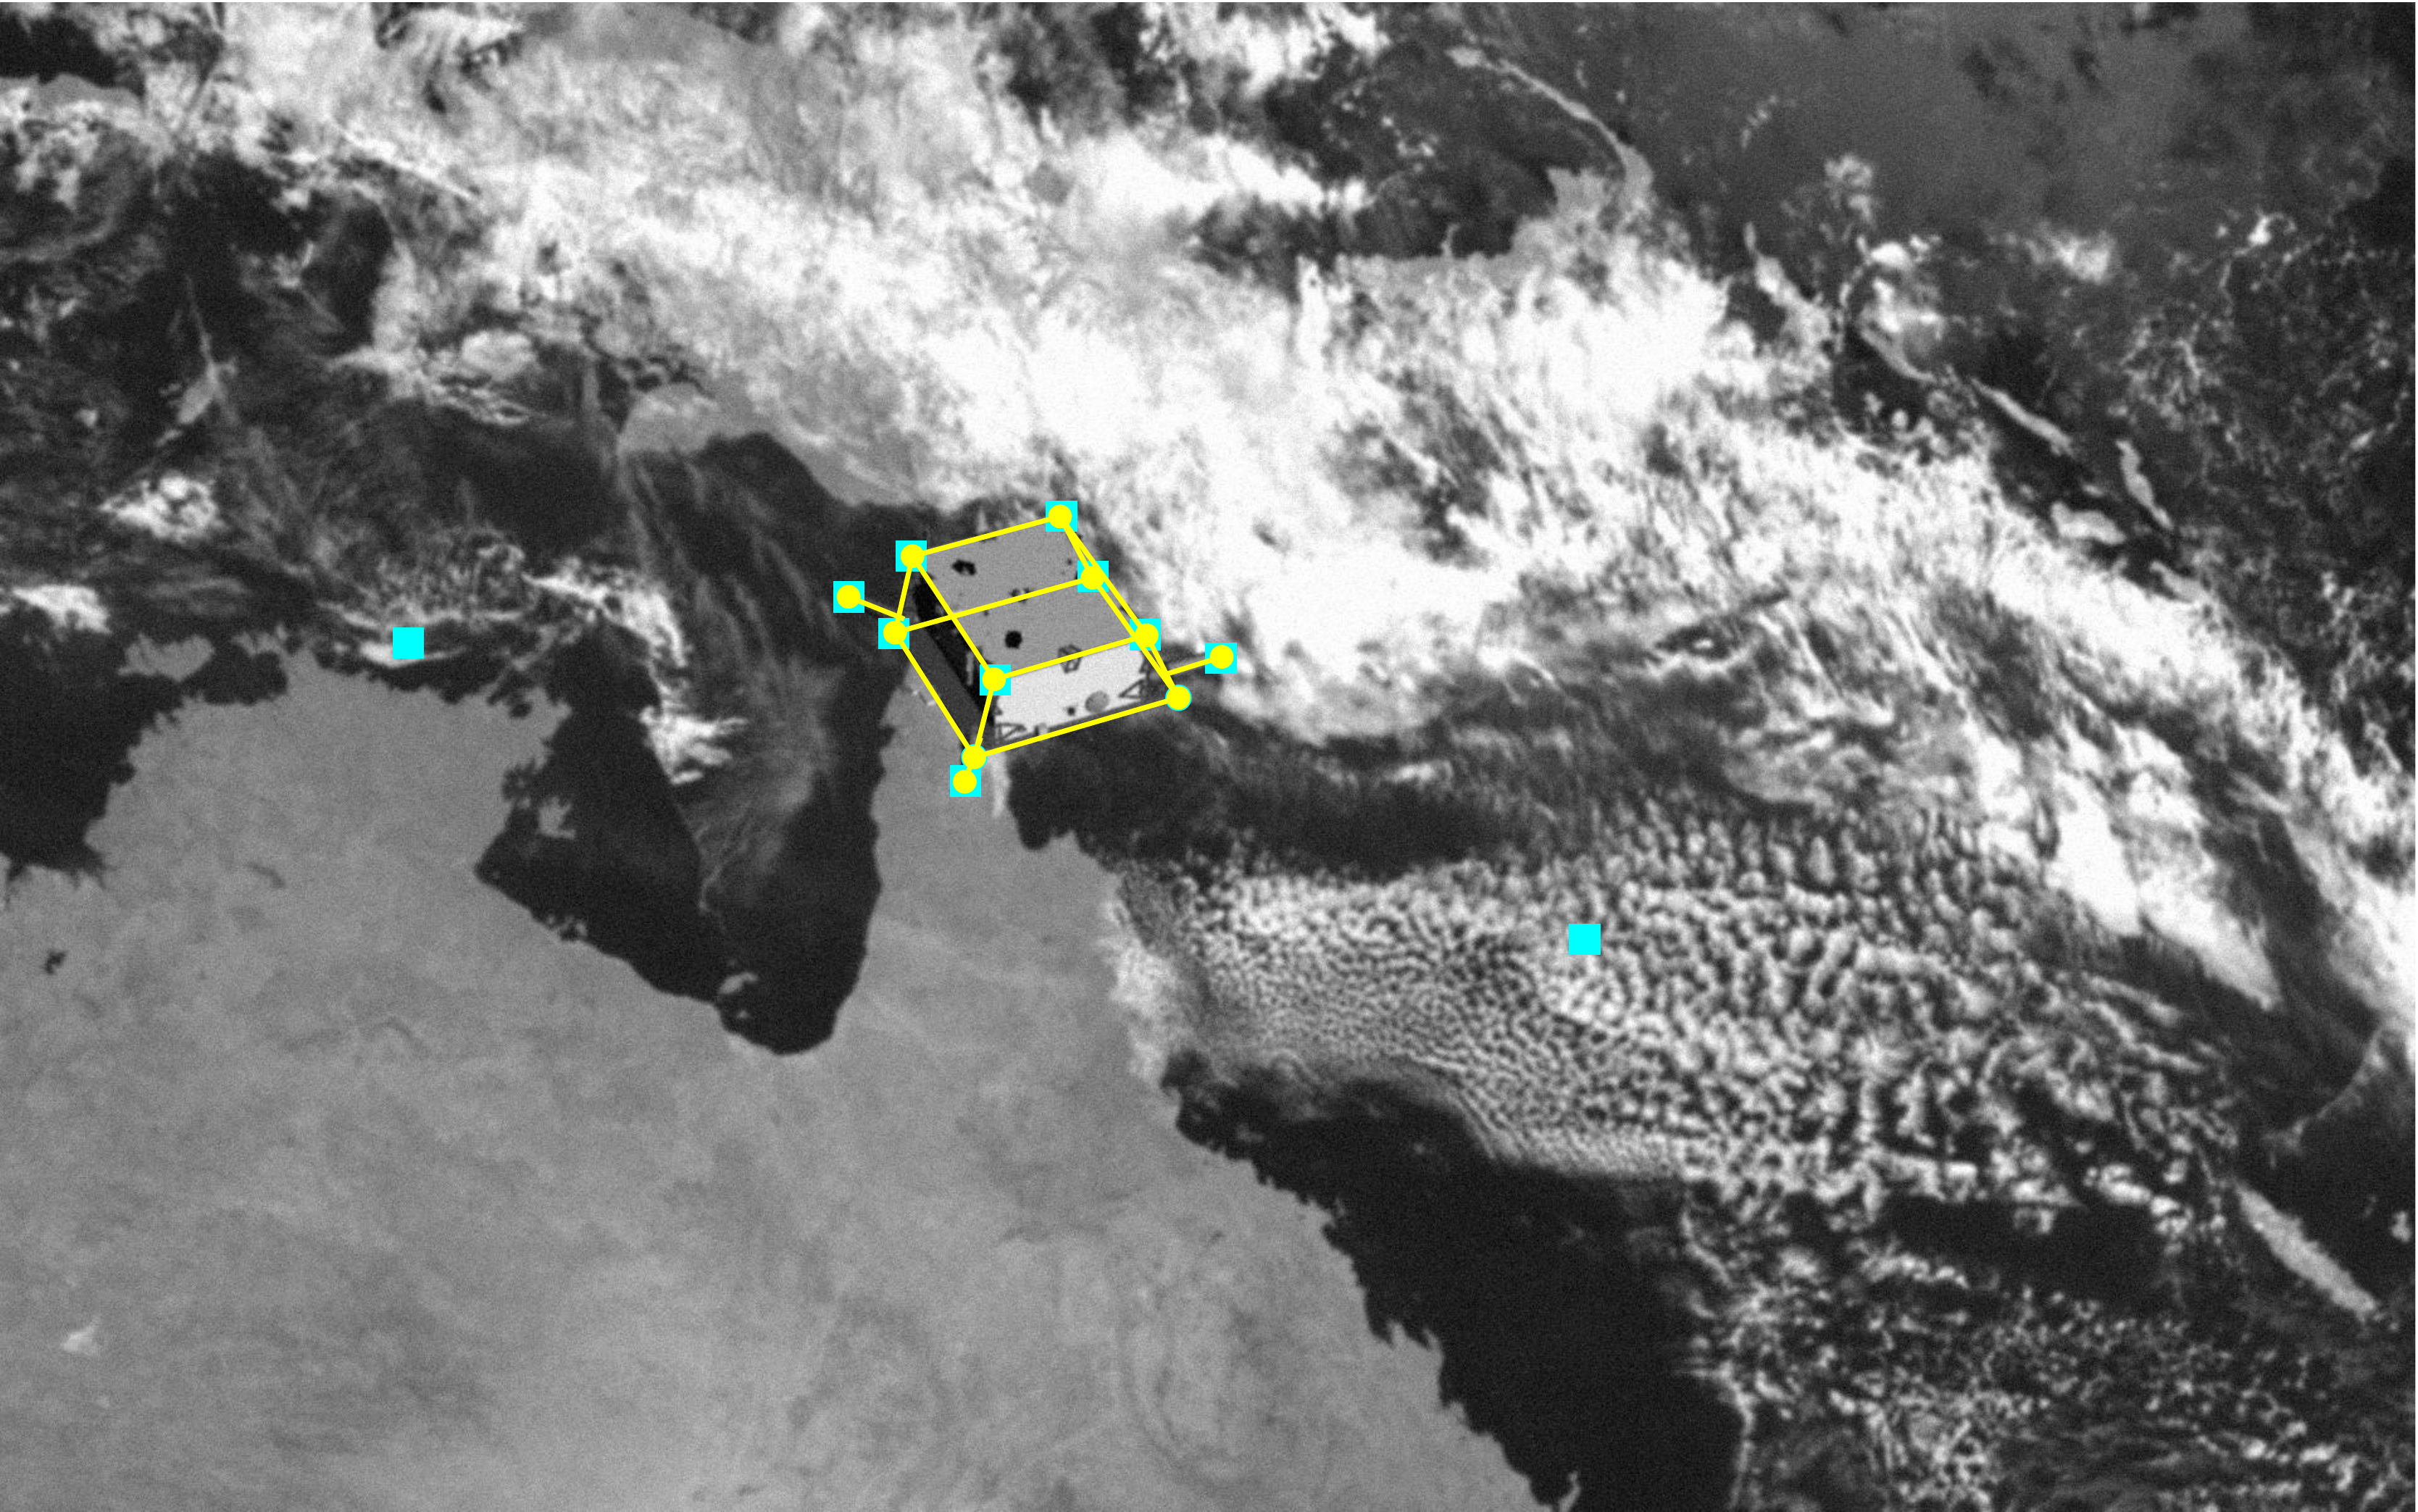}\\
			 $\MR$ error: $0.64^{\circ}$, $\vt$ error: $0.06$ \\ 
			 $\subopt=1.7\ee{-7}$, time: $52$ [s]
			\end{minipage}
		&  
			\begin{minipage}{\mpwfour}%
			\centering%
			\includegraphics[width=\columnwidth]{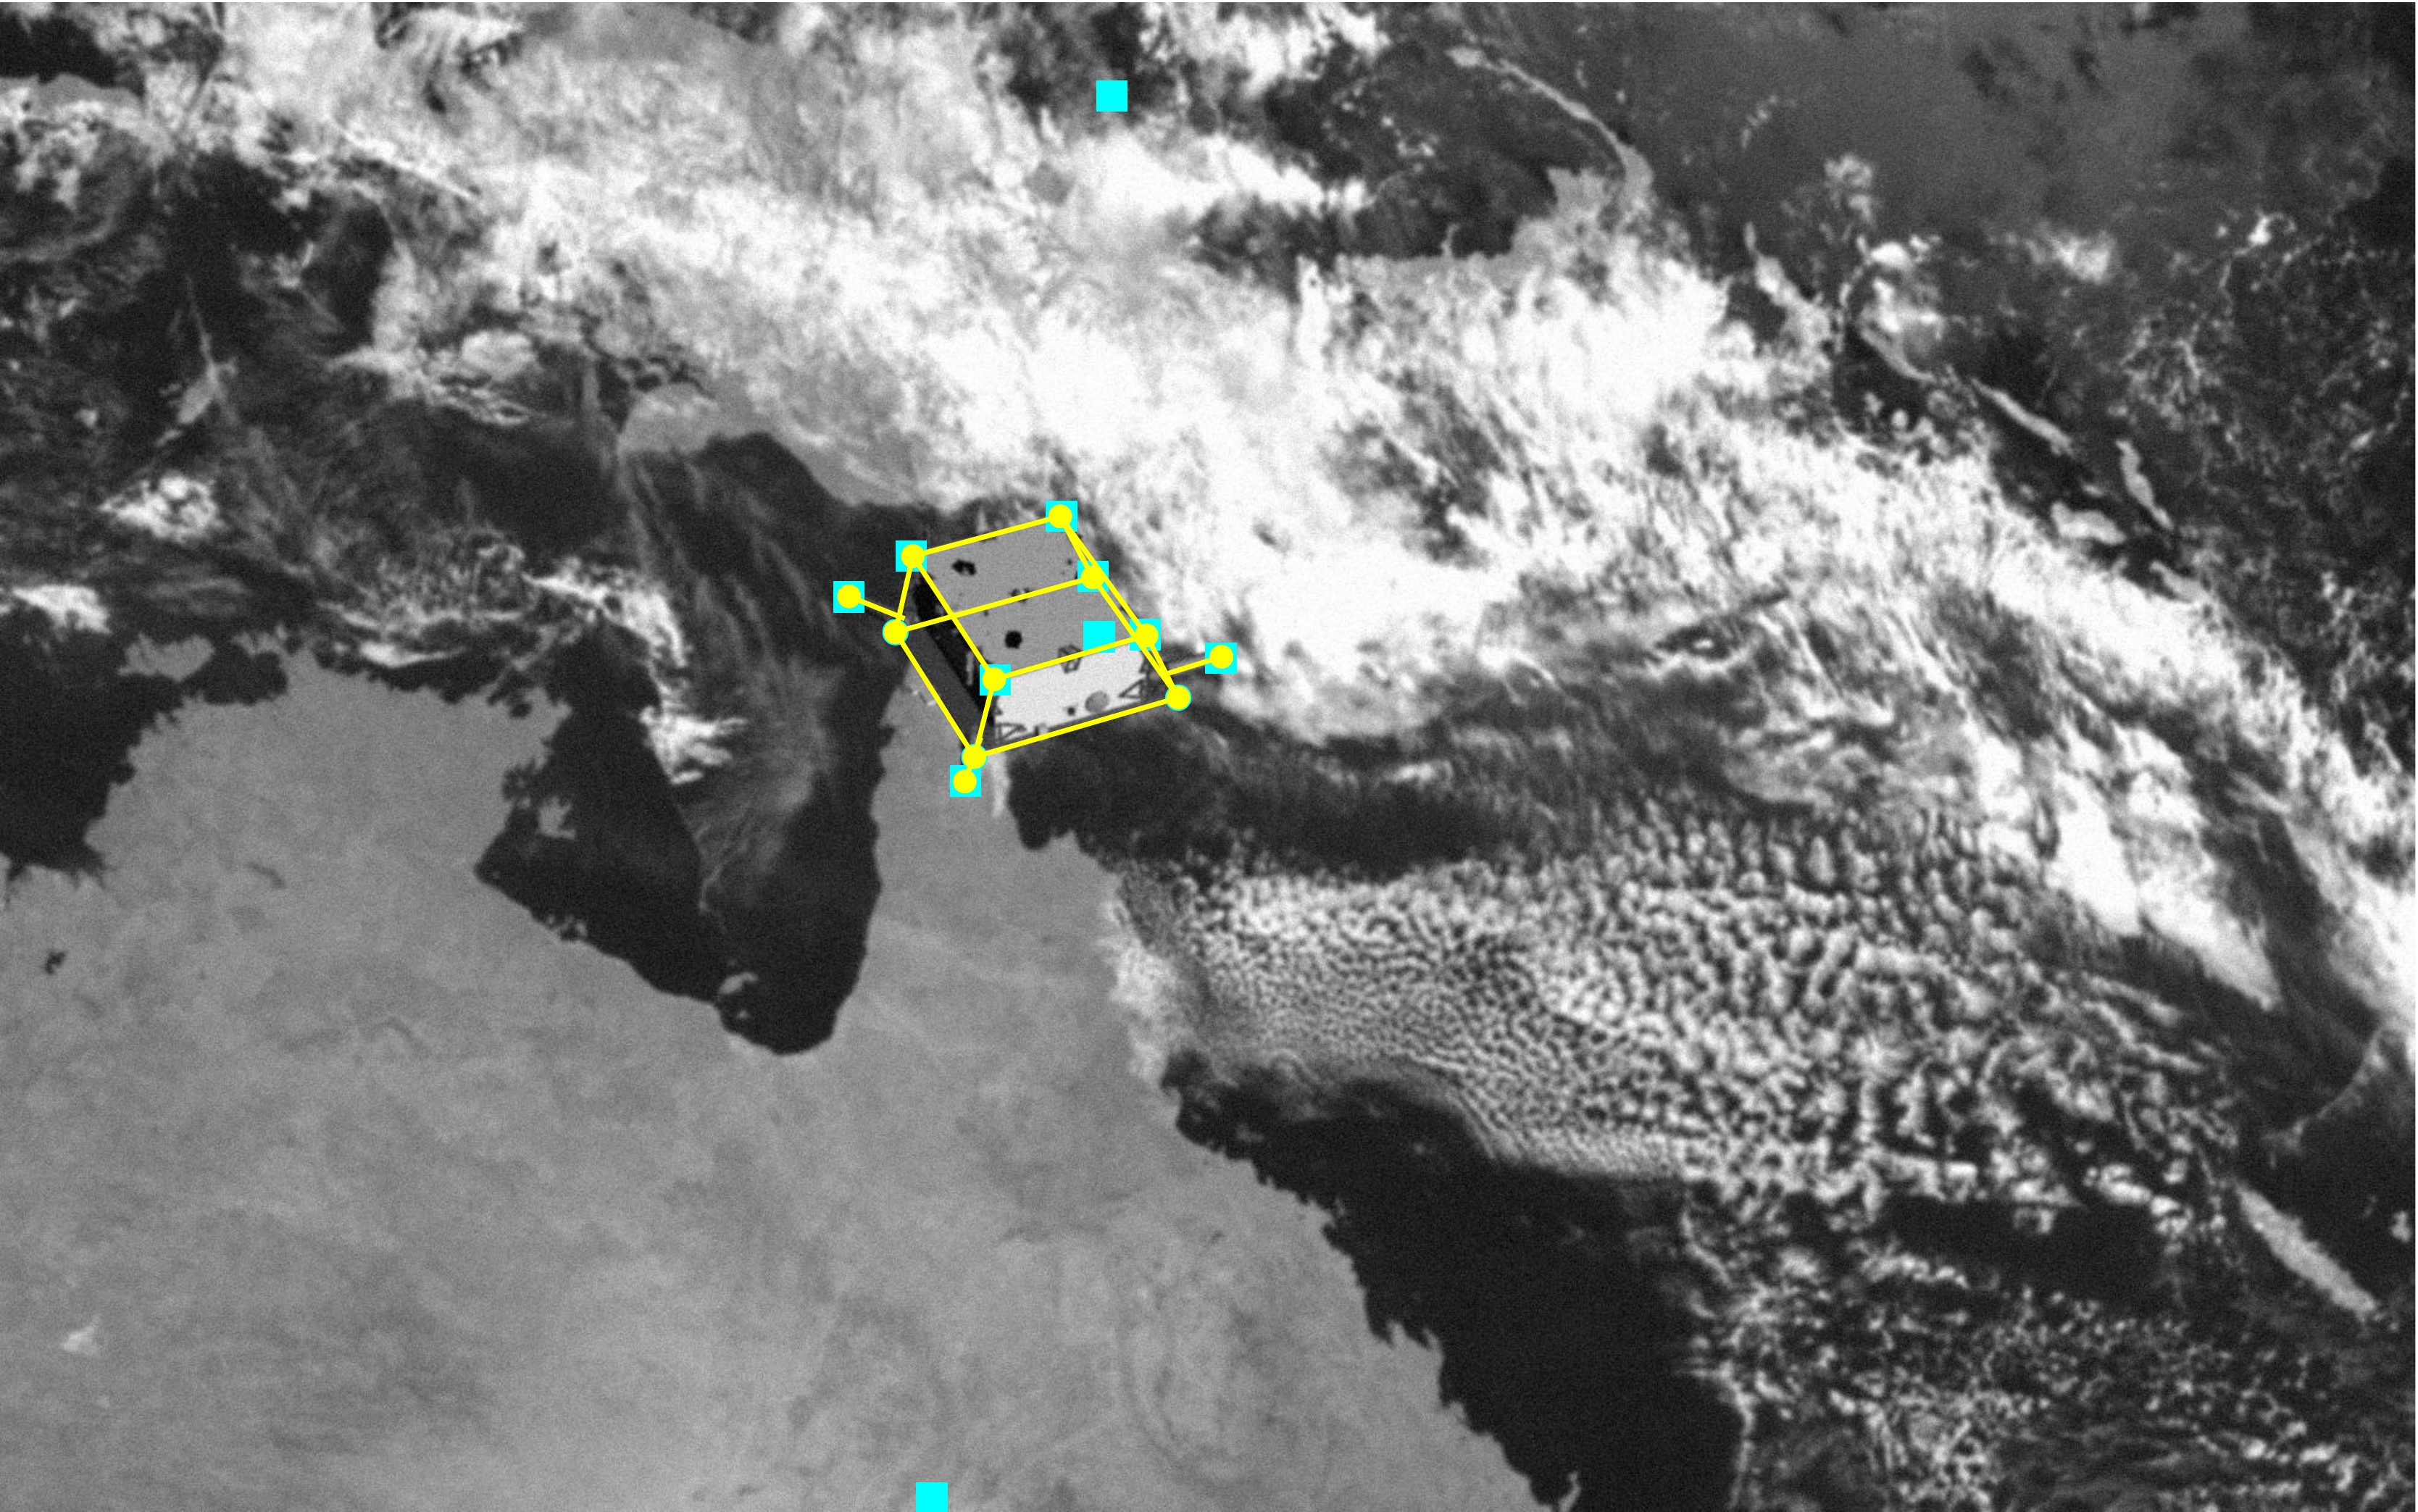}\\
			 $\MR$ error: $0.68^{\circ}$, $\vt$ error: $0.04$ \\ 
			 $\subopt=8.7\ee{-8}$, time: $47$ [s]
			\end{minipage}
		&  
			\begin{minipage}{\mpwfour}%
			\centering%
			\includegraphics[width=\columnwidth]{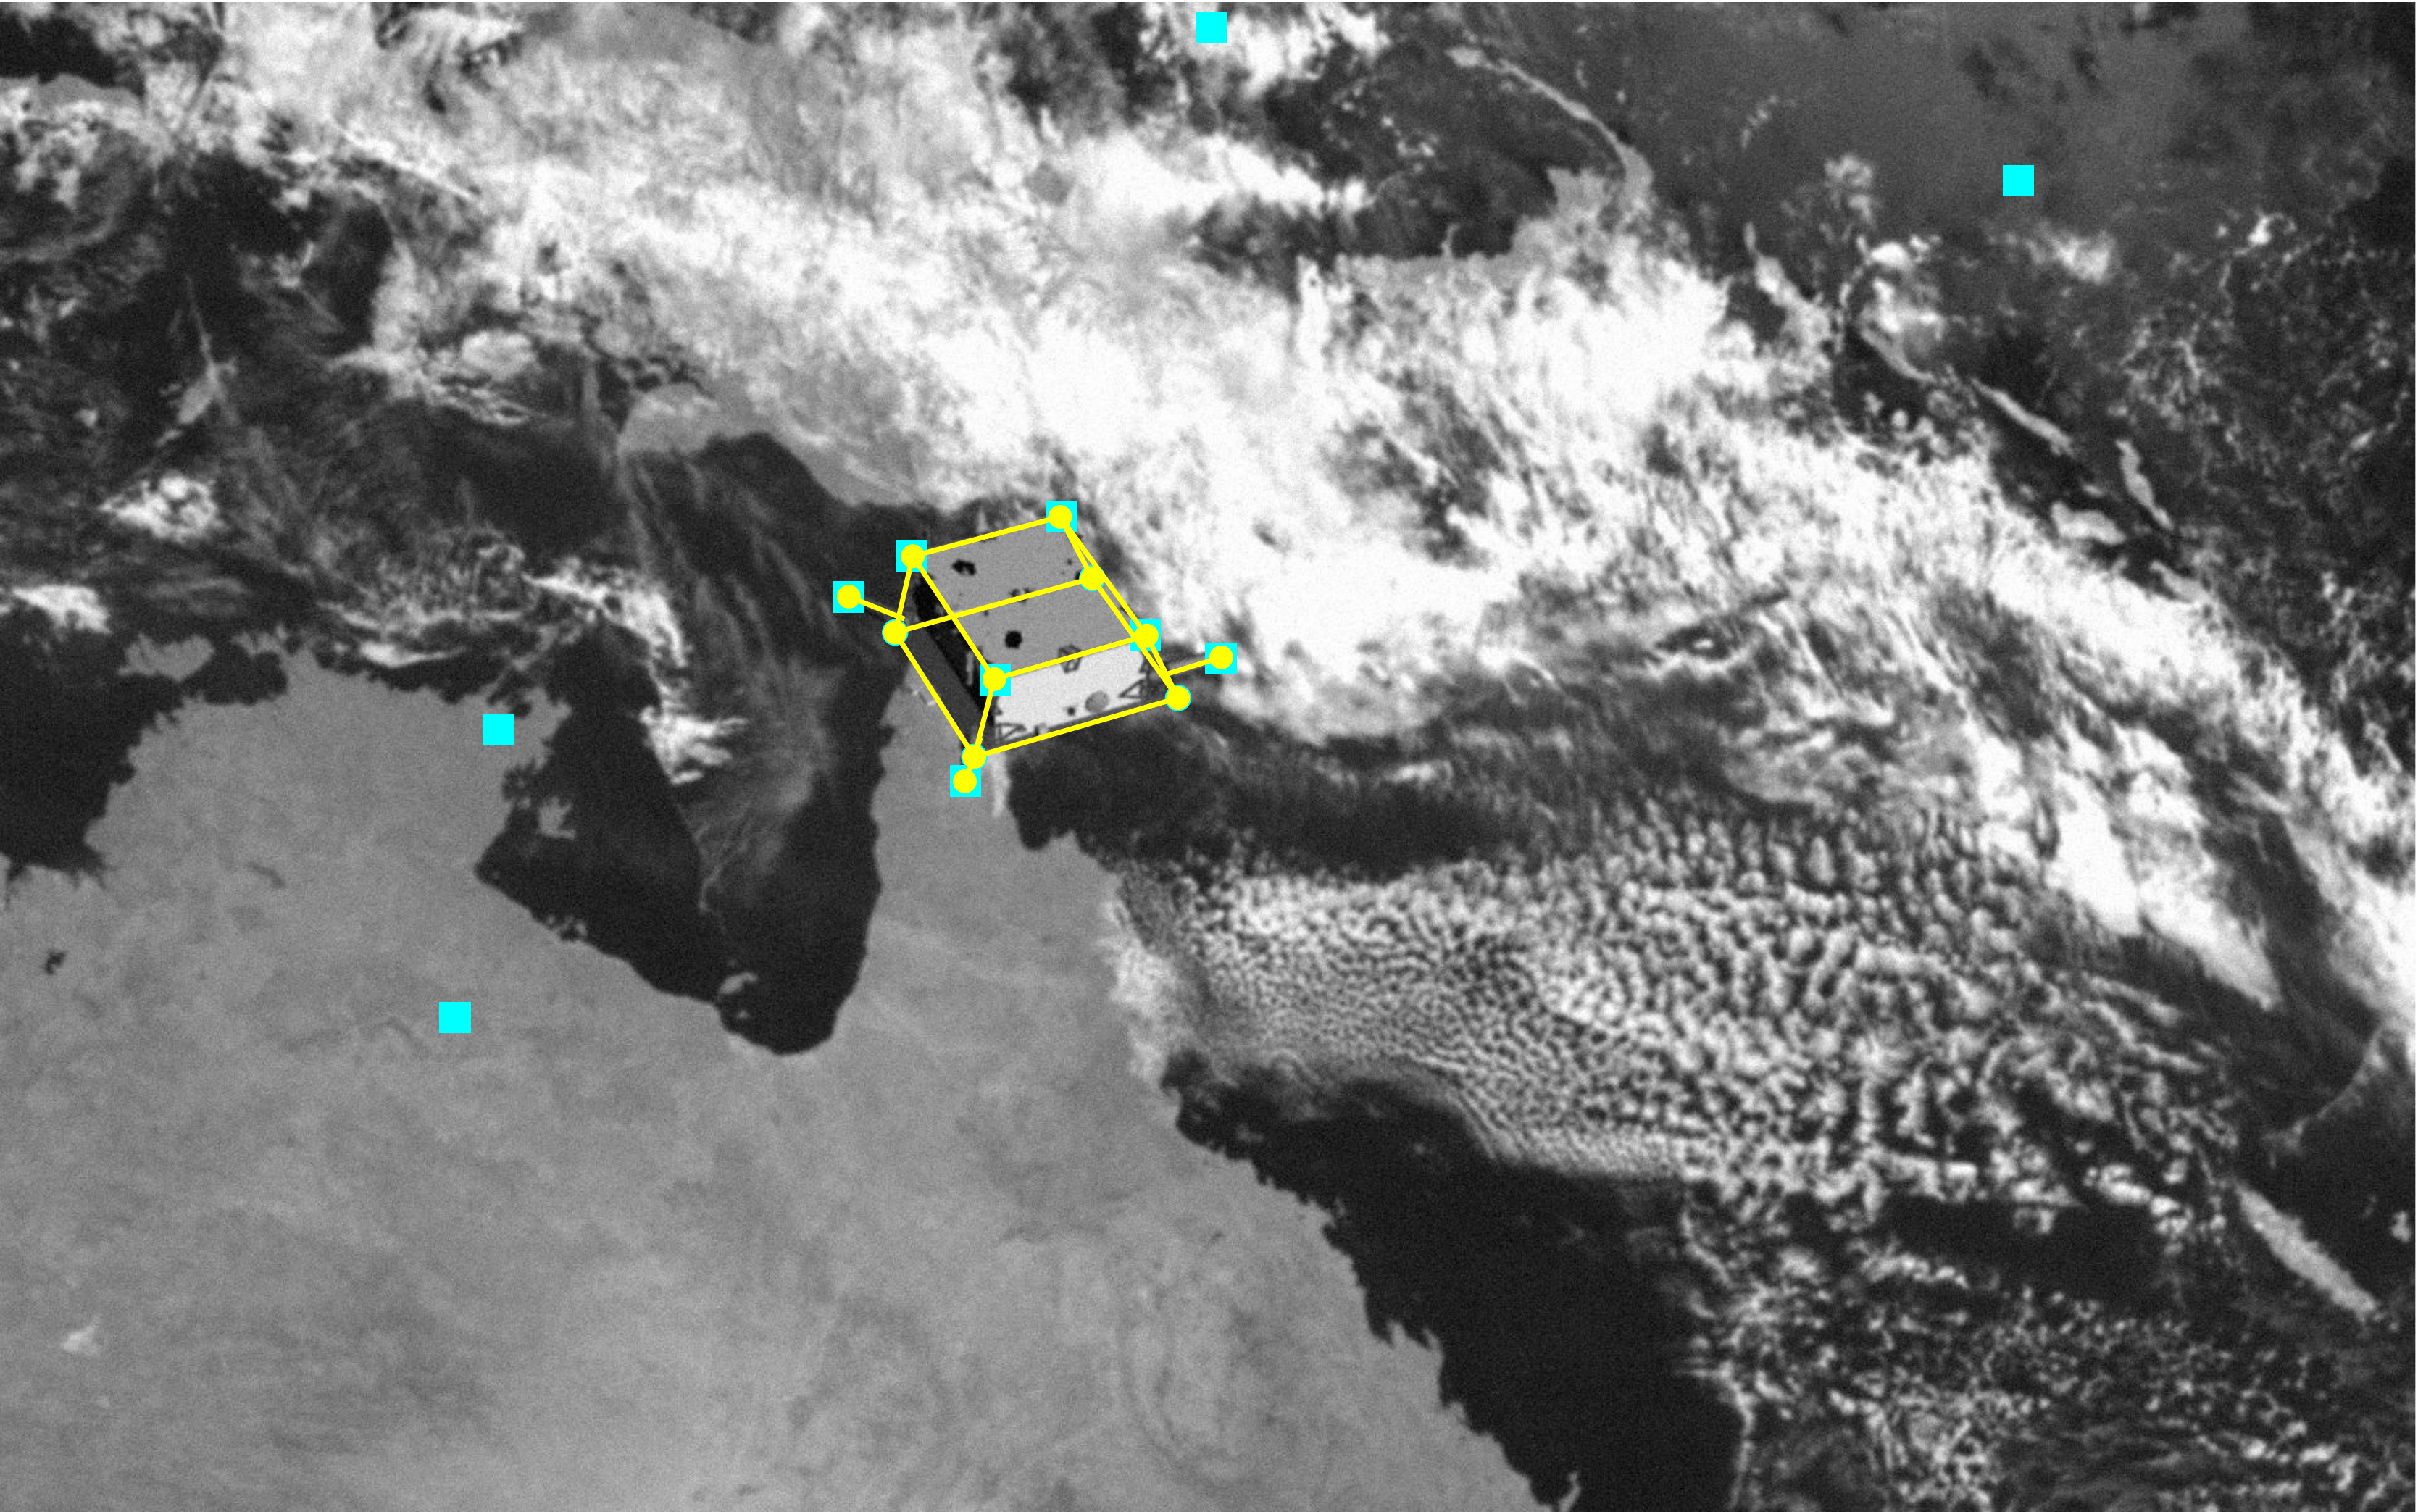}\\
			 $\MR$ error: $0.55^{\circ}$, $\vt$ error: $0.04$ \\ 
			 $\subopt=3.5\ee{-8}$, time: $127$ [s]
			\end{minipage}
		&  
			\begin{minipage}{\mpwfour}%
			\centering%
			\includegraphics[width=\columnwidth]{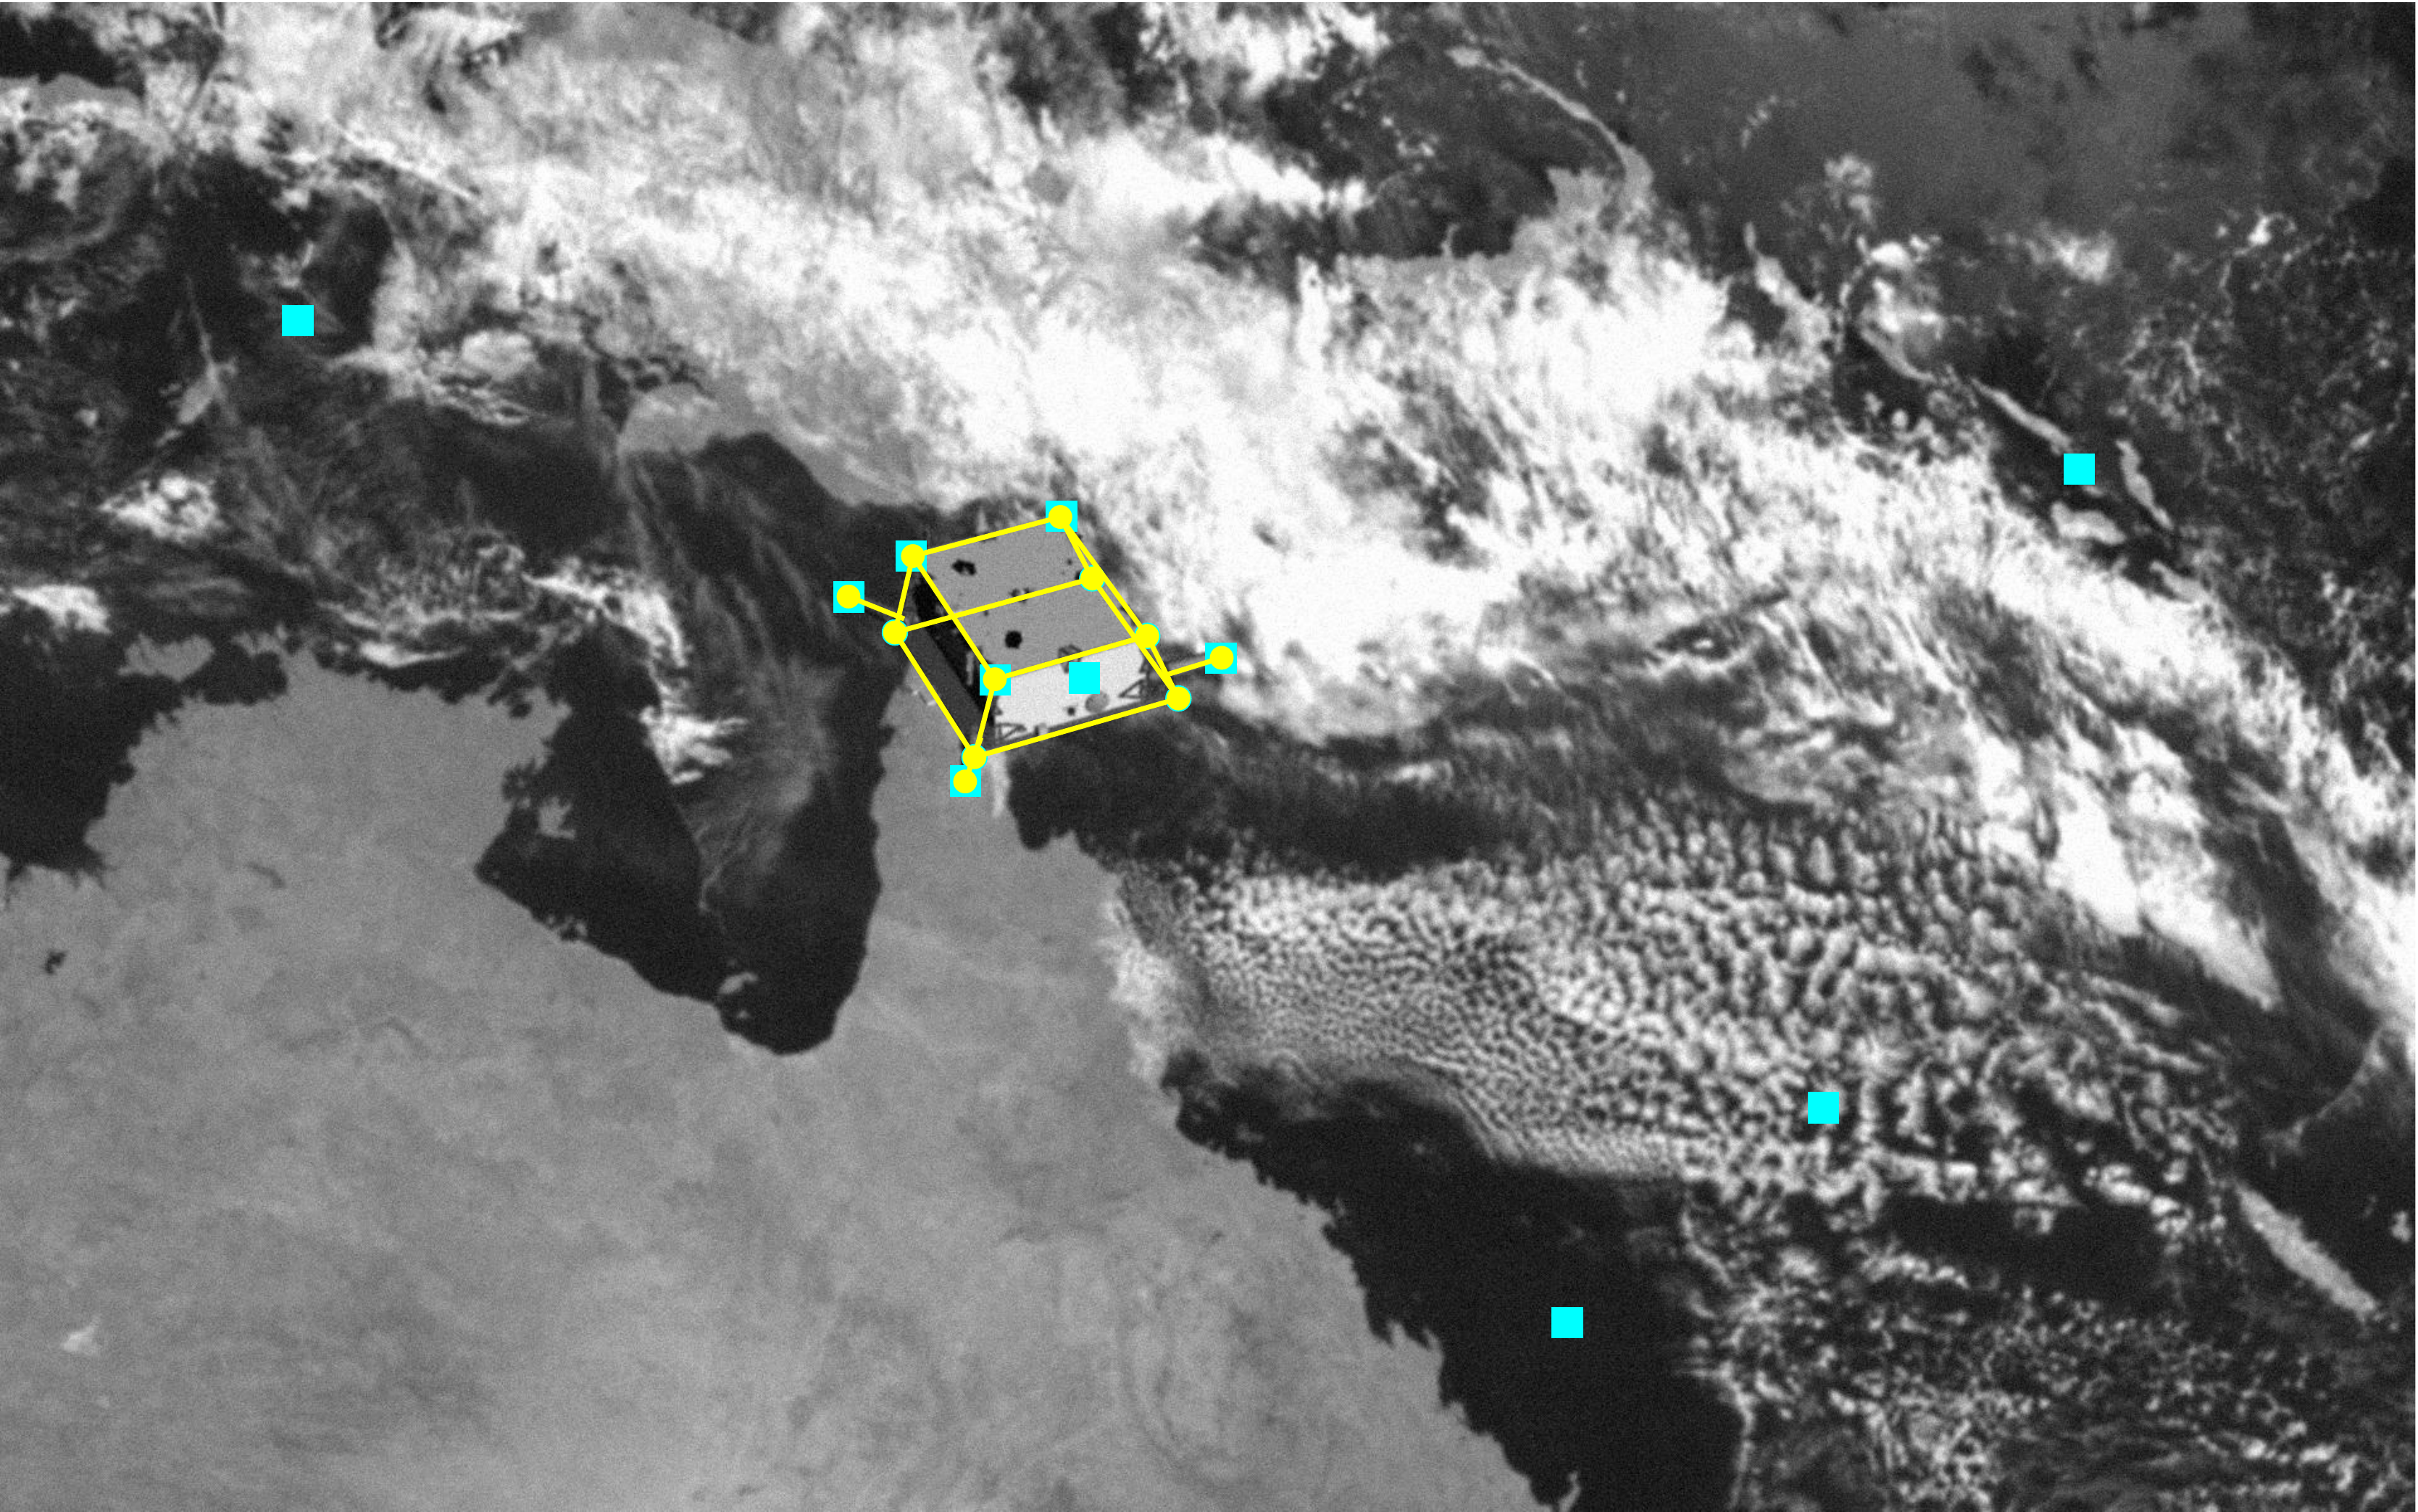}\\
			 $\MR$ error: $0.45^{\circ}$, $\vt$ error: $0.06$ \\ 
			 $\subopt=4.3\ee{-8}$, time: $64$ [s]
			\end{minipage} \vspace{1mm}
		\\

		%%%%%%%%%%%%%%%%%%%%%%%%%%%%%%%%%%%%%%%%%%%%%%%%%%%%%%%%%%%%%%%%%%%%%%%%%%%%%%%%%%%%%%%%%%%%%%%%%%%%%%%%%
			\begin{minipage}{\mpwfour}%
			\centering%
			\includegraphics[width=\columnwidth]{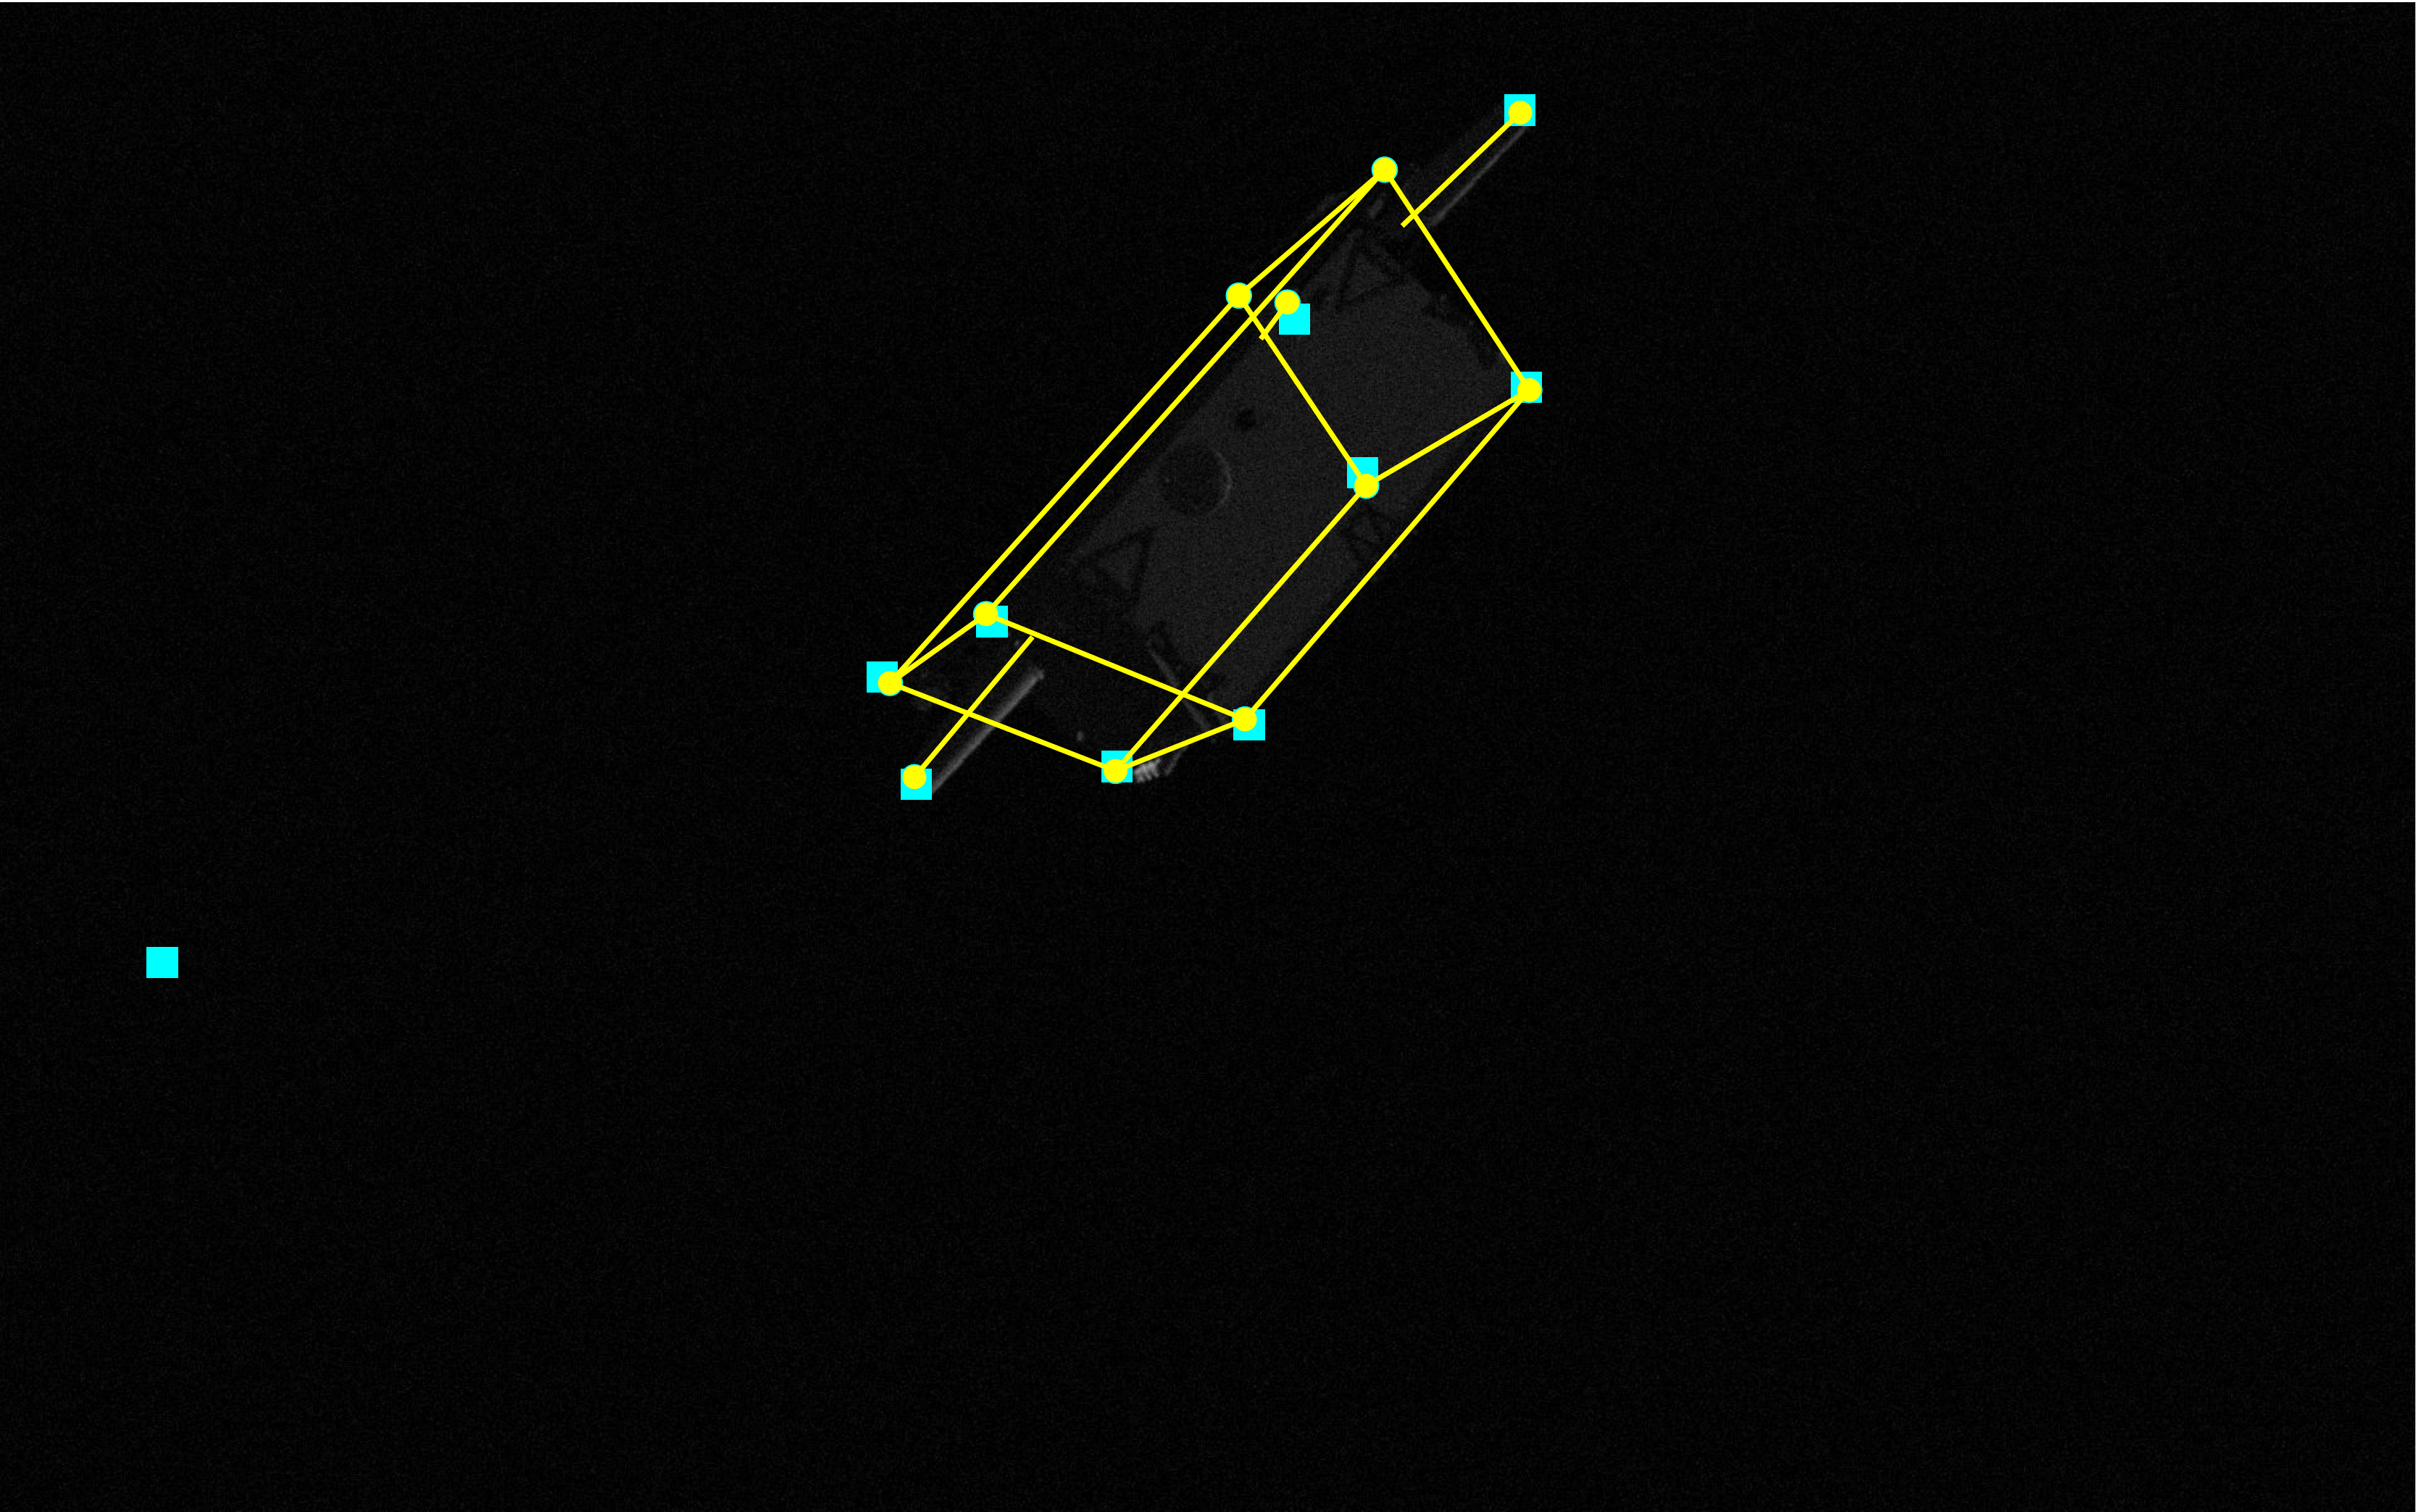}\\
			 $\MR$ error: $1.70^{\circ}$, $\vt$ error: $0.02$ \\ 
			 $\subopt=1.8\ee{-8}$, time: $47$ [s]
			\end{minipage}
		&  
			\begin{minipage}{\mpwfour}%
			\centering%
			\includegraphics[width=\columnwidth]{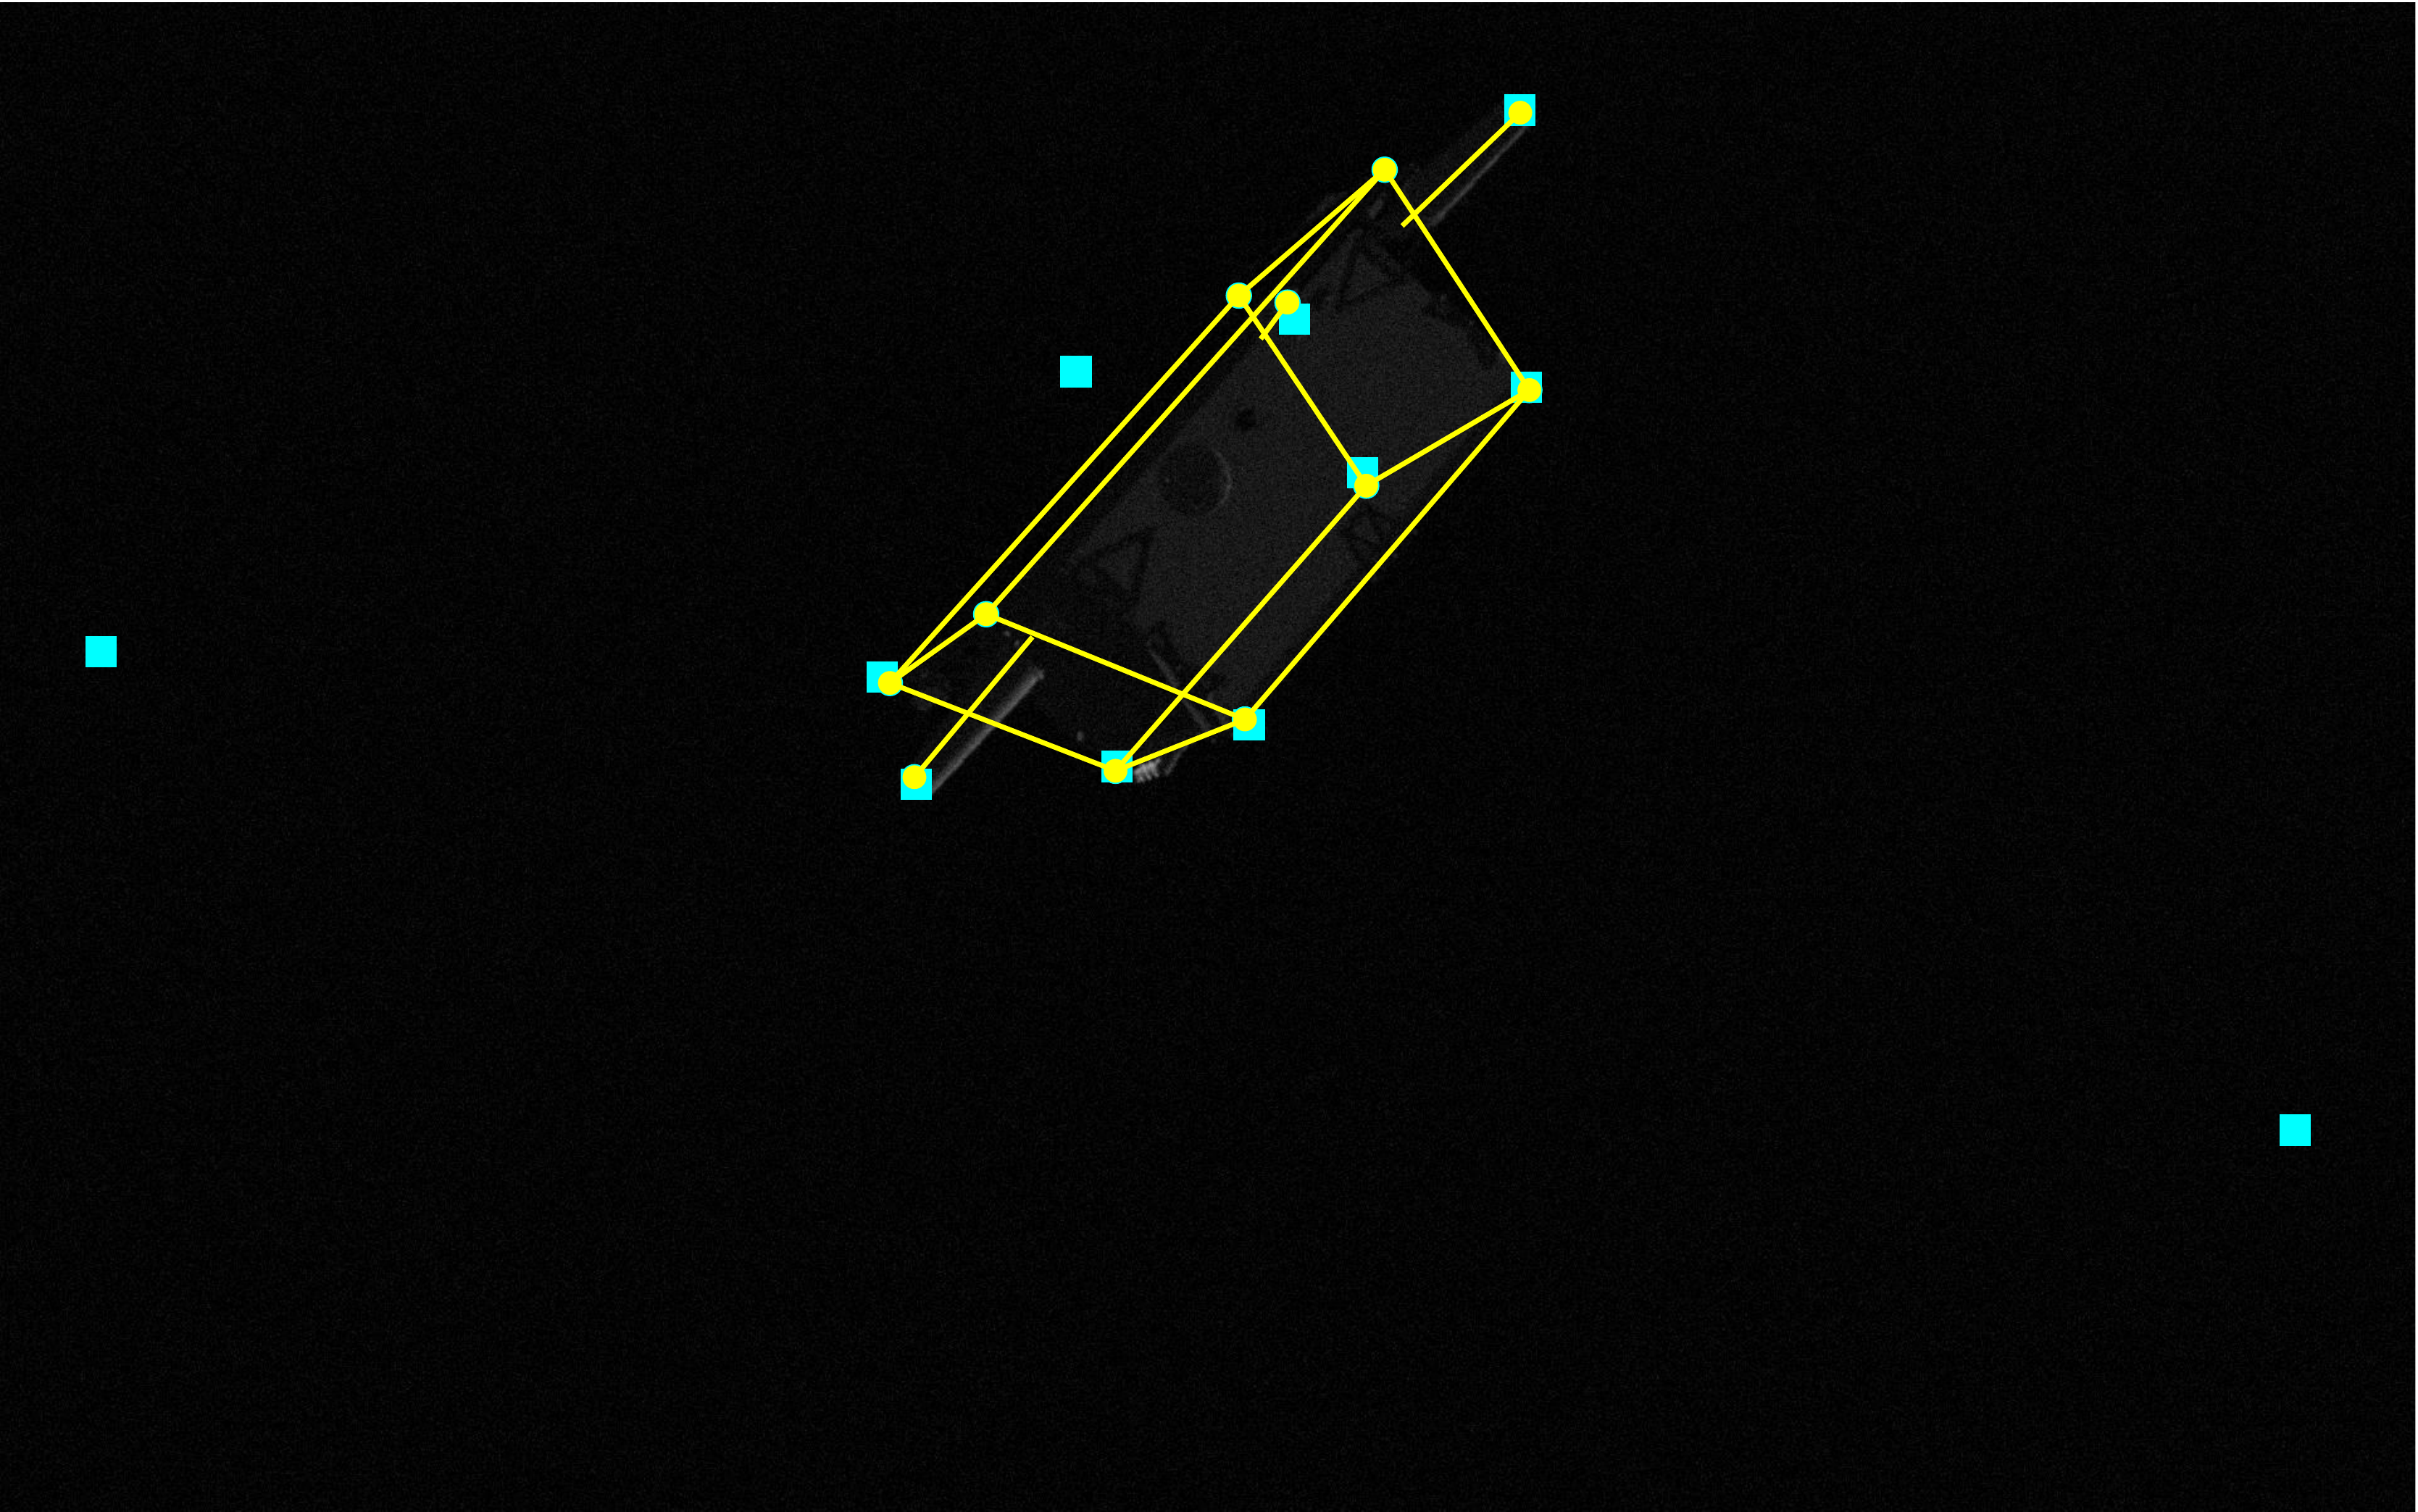}\\
			 $\MR$ error: $1.70^{\circ}$, $\vt$ error: $0.02$ \\ 
			 $\subopt=6.0\ee{-8}$, time: $48$ [s]
			\end{minipage}
		&  
			\begin{minipage}{\mpwfour}%
			\centering%
			\includegraphics[width=\columnwidth]{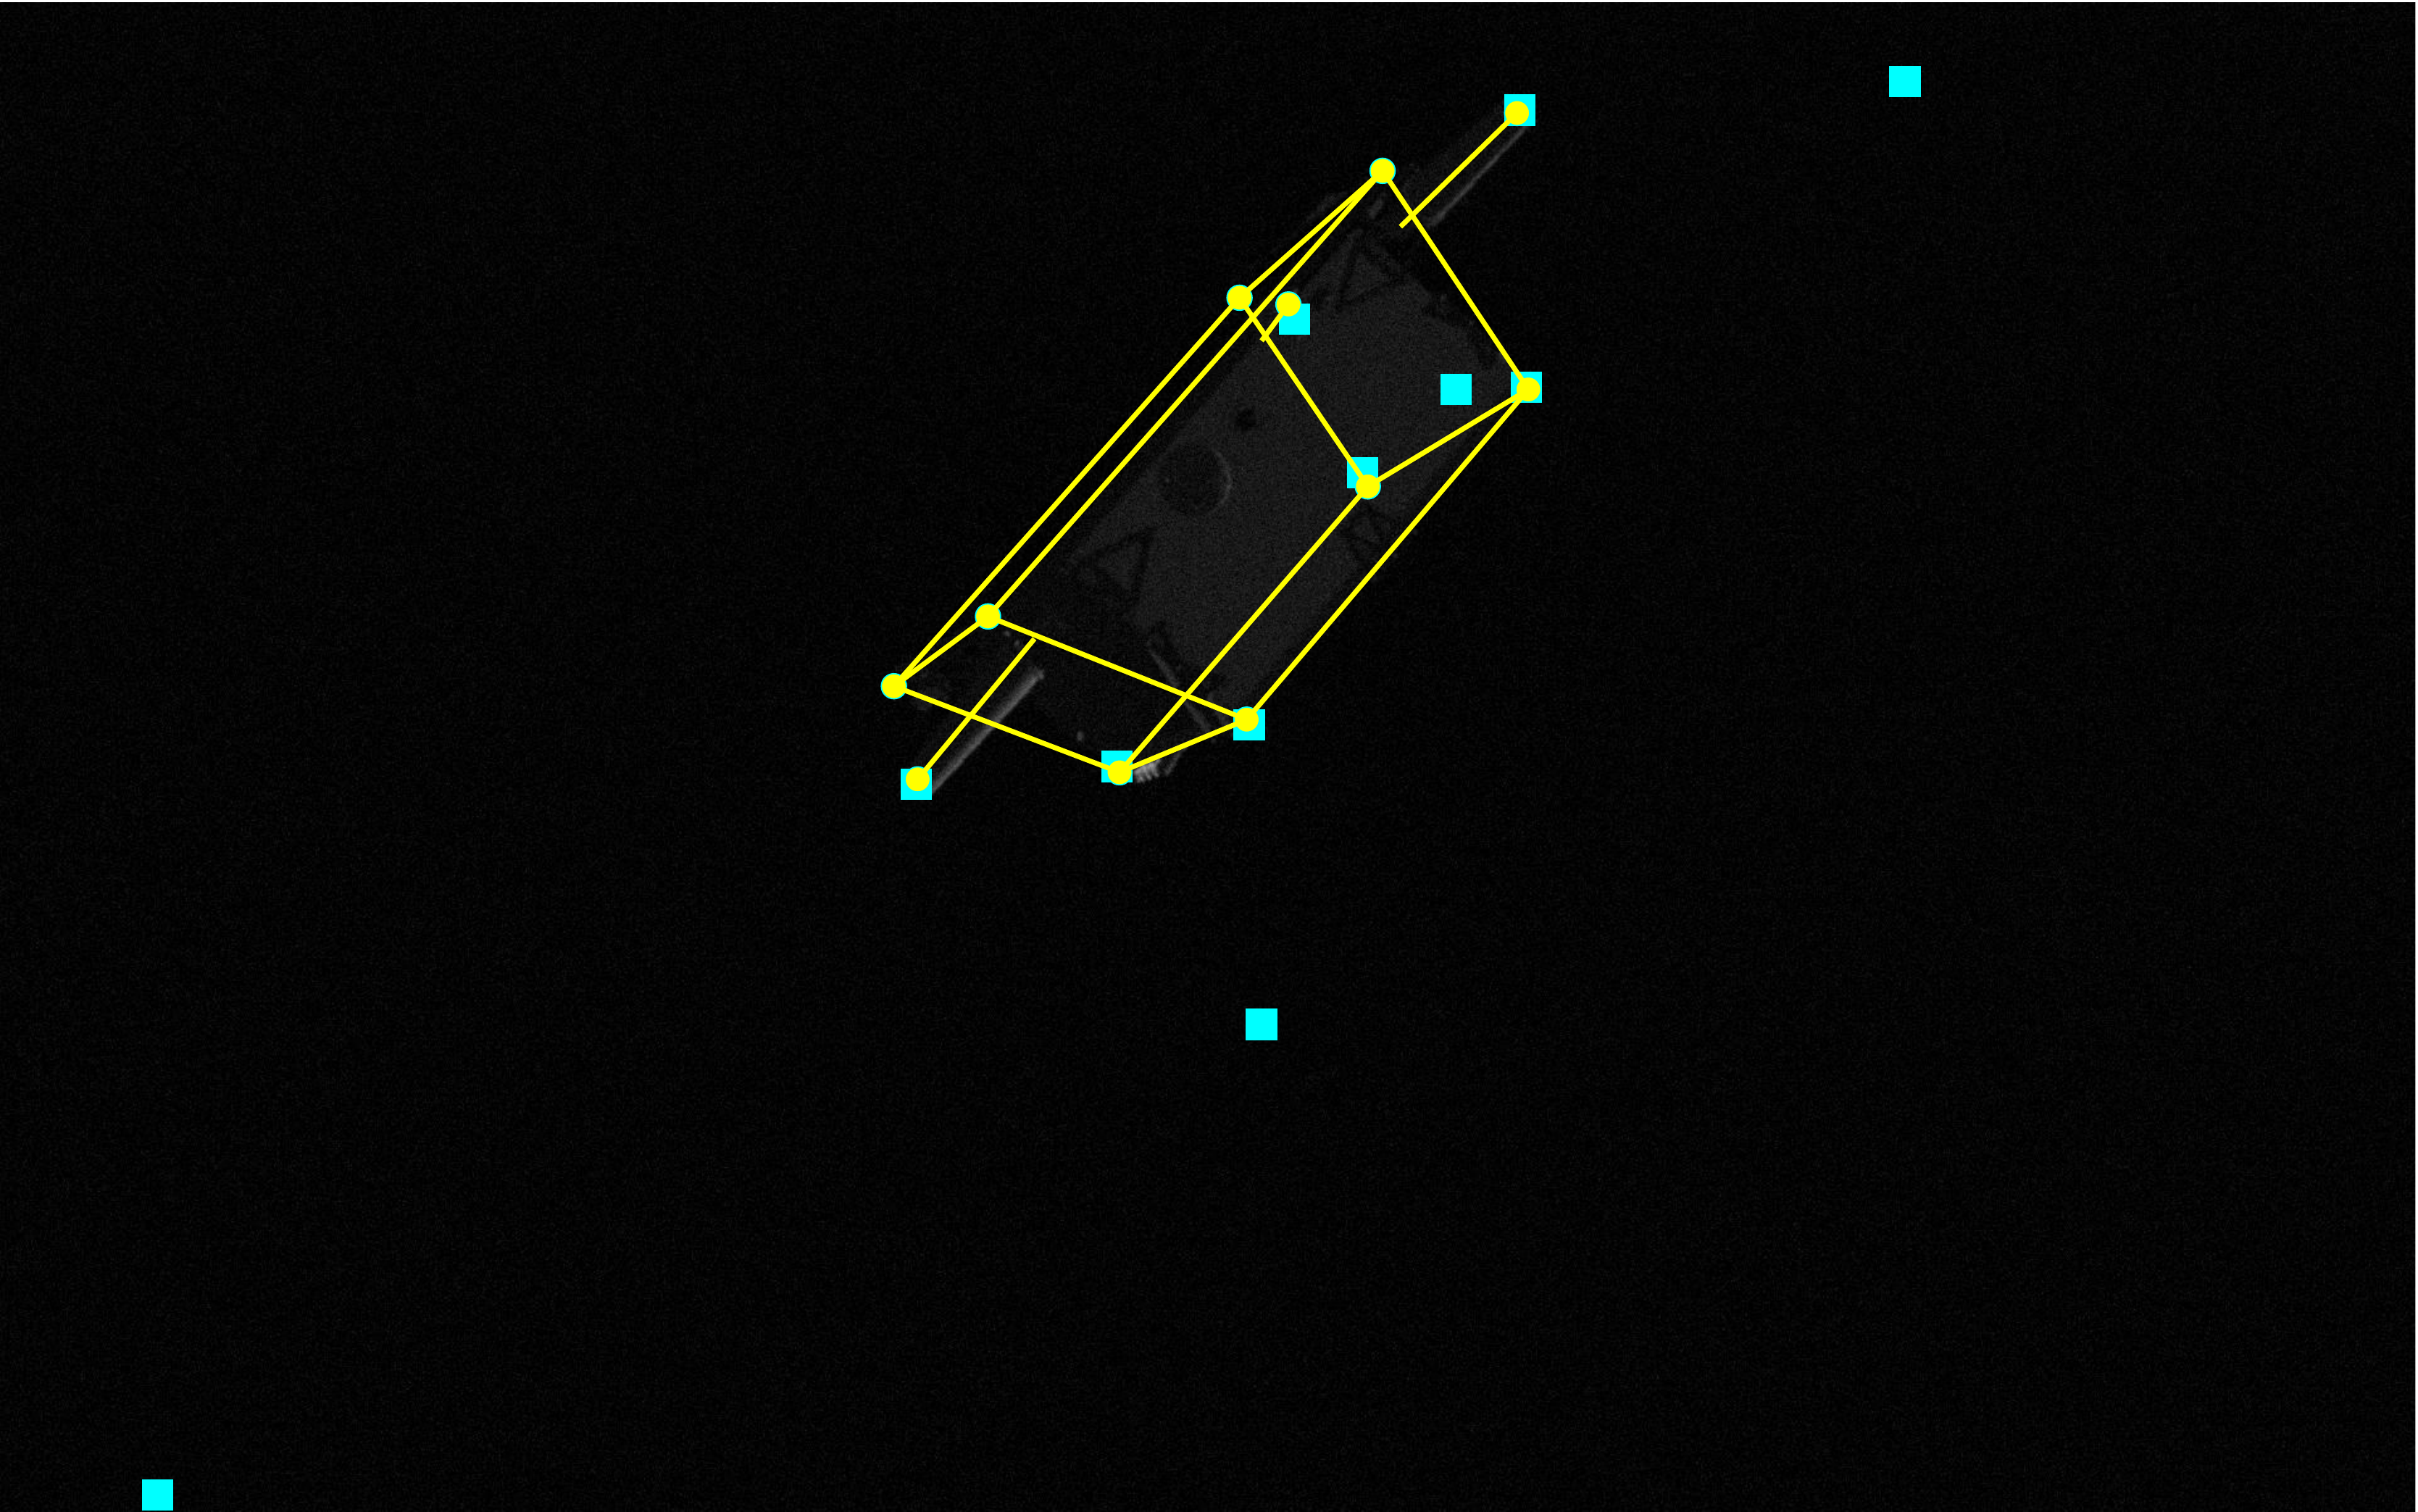}\\
			 $\MR$ error: $1.74^{\circ}$, $\vt$ error: $0.04$ \\ 
			 $\subopt=6.8\ee{-8}$, time: $48$ [s]
			\end{minipage}
		&  
			\begin{minipage}{\mpwfour}%
			\centering%
			\includegraphics[width=\columnwidth]{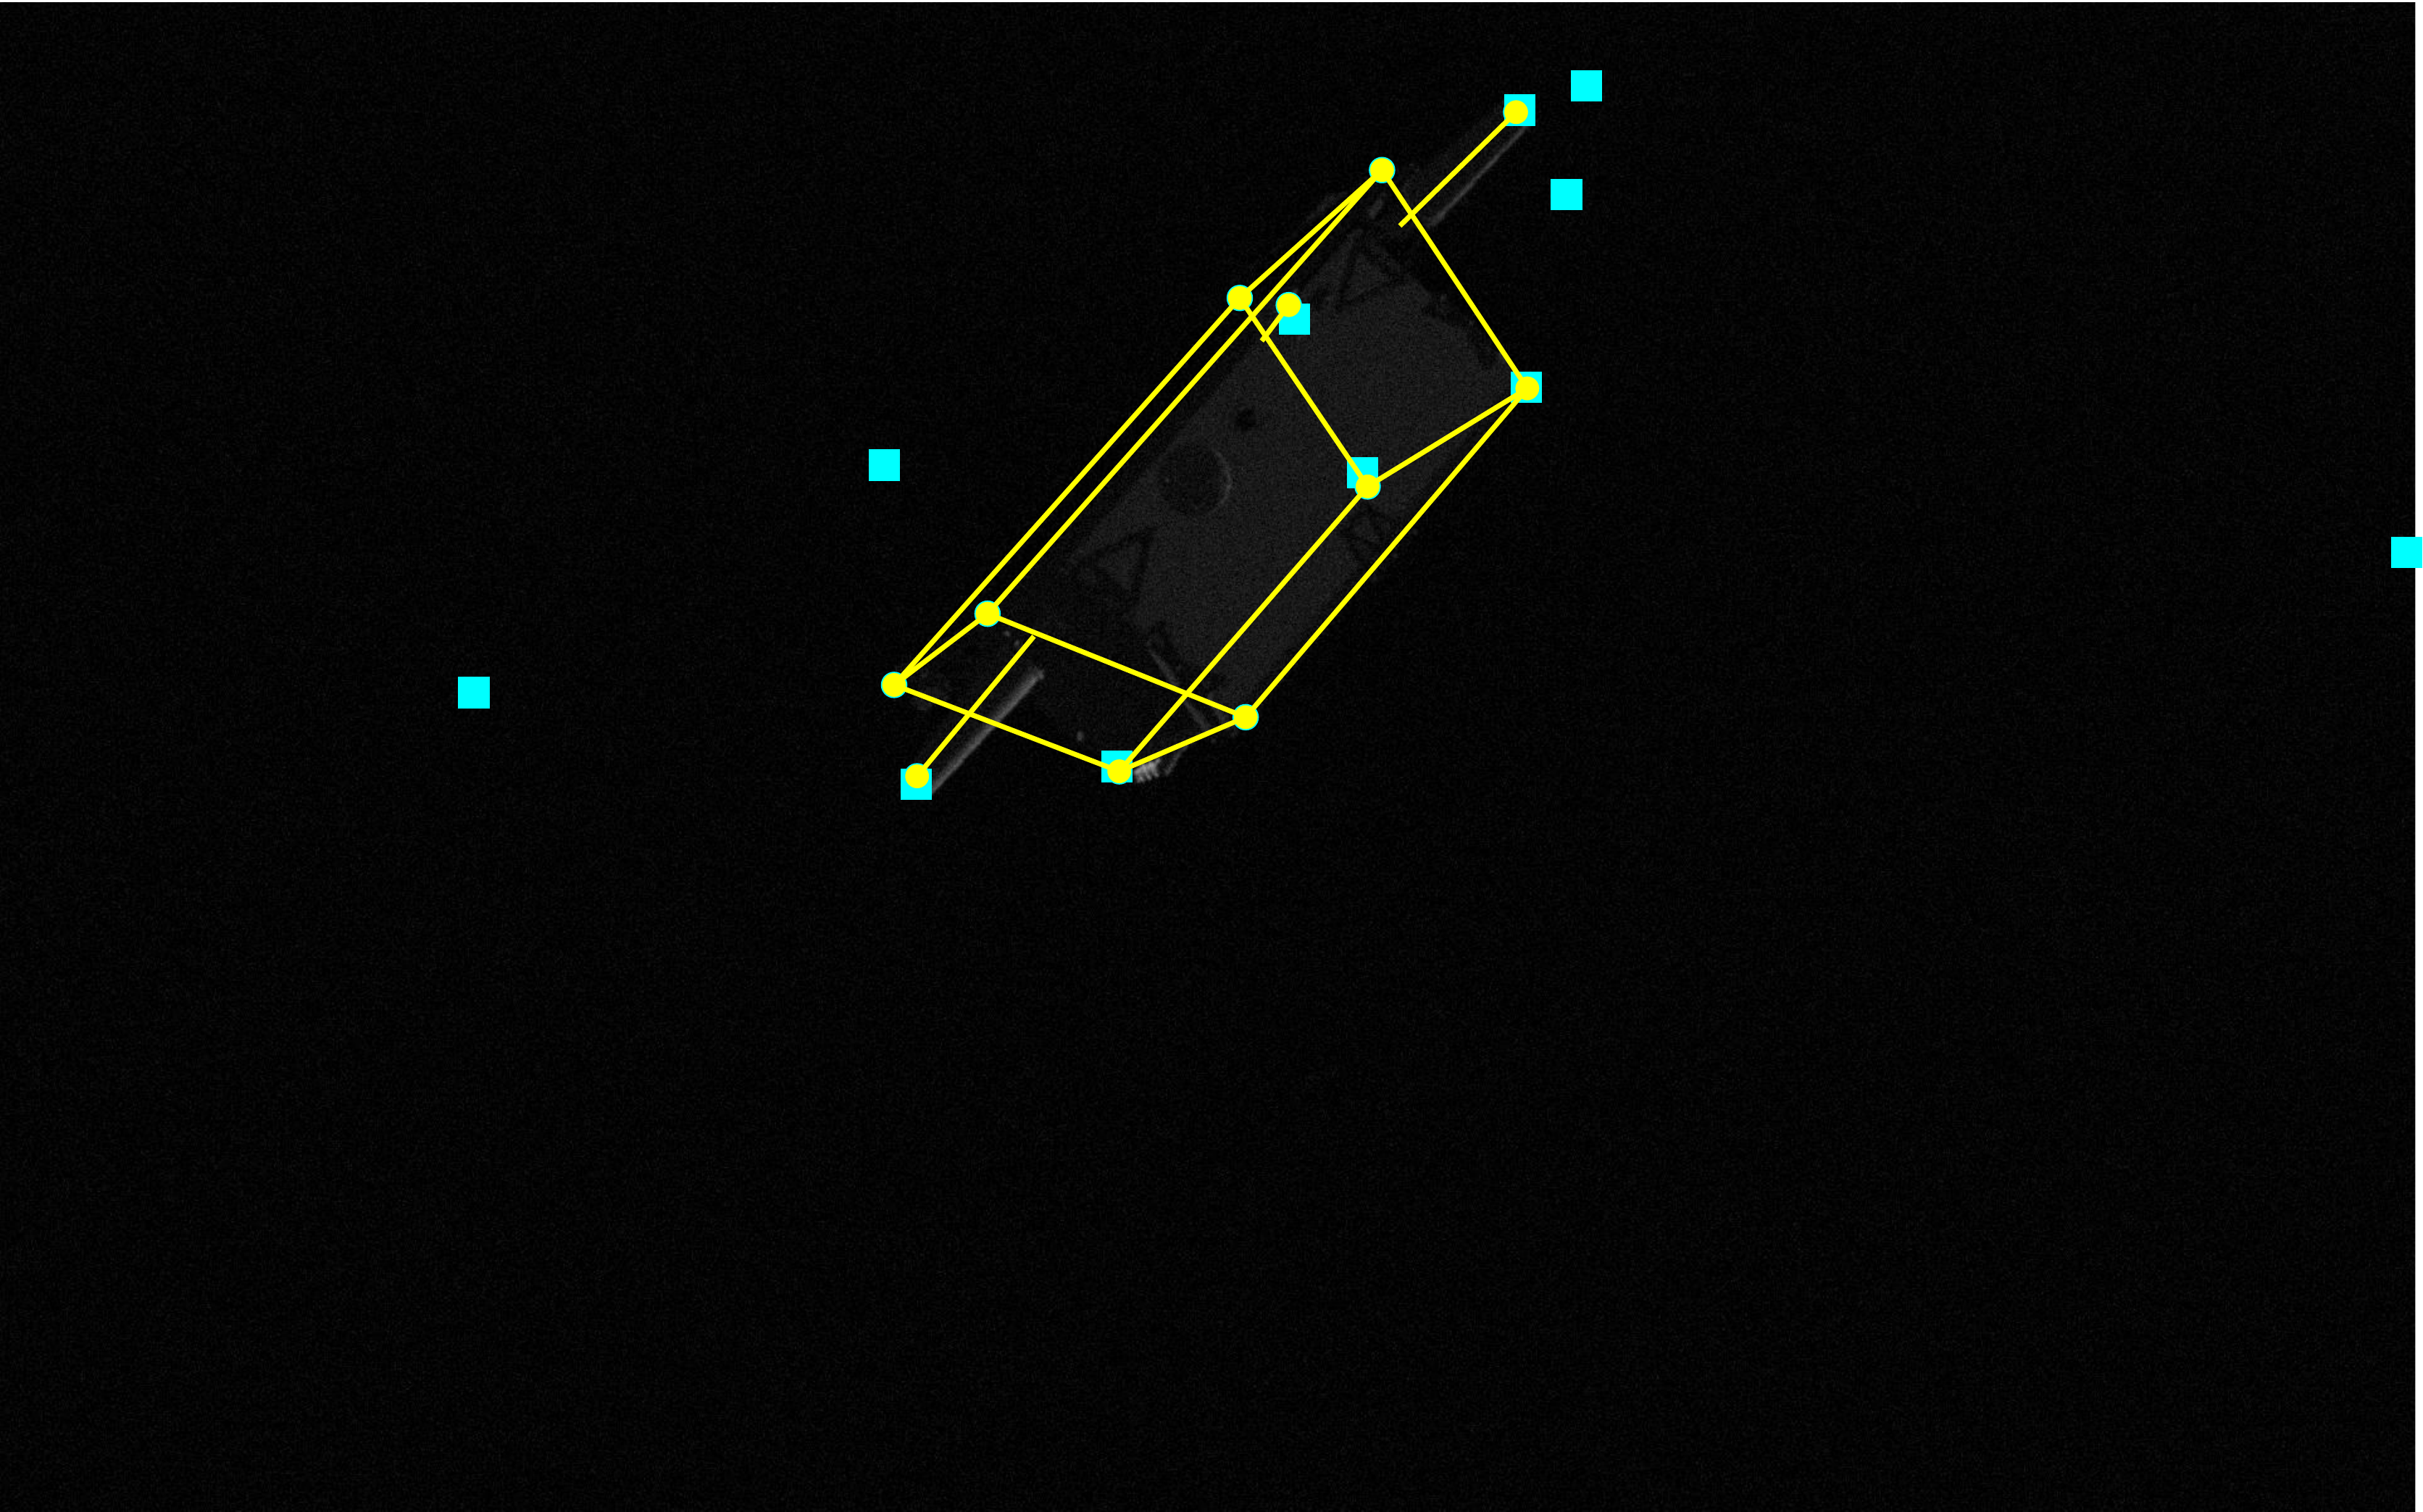}\\
			 $\MR$ error: $1.90^{\circ}$, $\vt$ error: $0.05$ \\ 
			 $\subopt=4.6\ee{-5}$, time: $159$ [s]
			\end{minipage} \vspace{1mm}
		\\

		%%%%%%%%%%%%%%%%%%%%%%%%%%%%%%%%%%%%%%%%%%%%%%%%%%%%%%%%%%%%%%%%%%%%%%%%%%%%%%%%%%%%%%%%%%%%%%%%%%%%%%%%%
			\begin{minipage}{\mpwfour}%
			\centering%
			\includegraphics[width=\columnwidth]{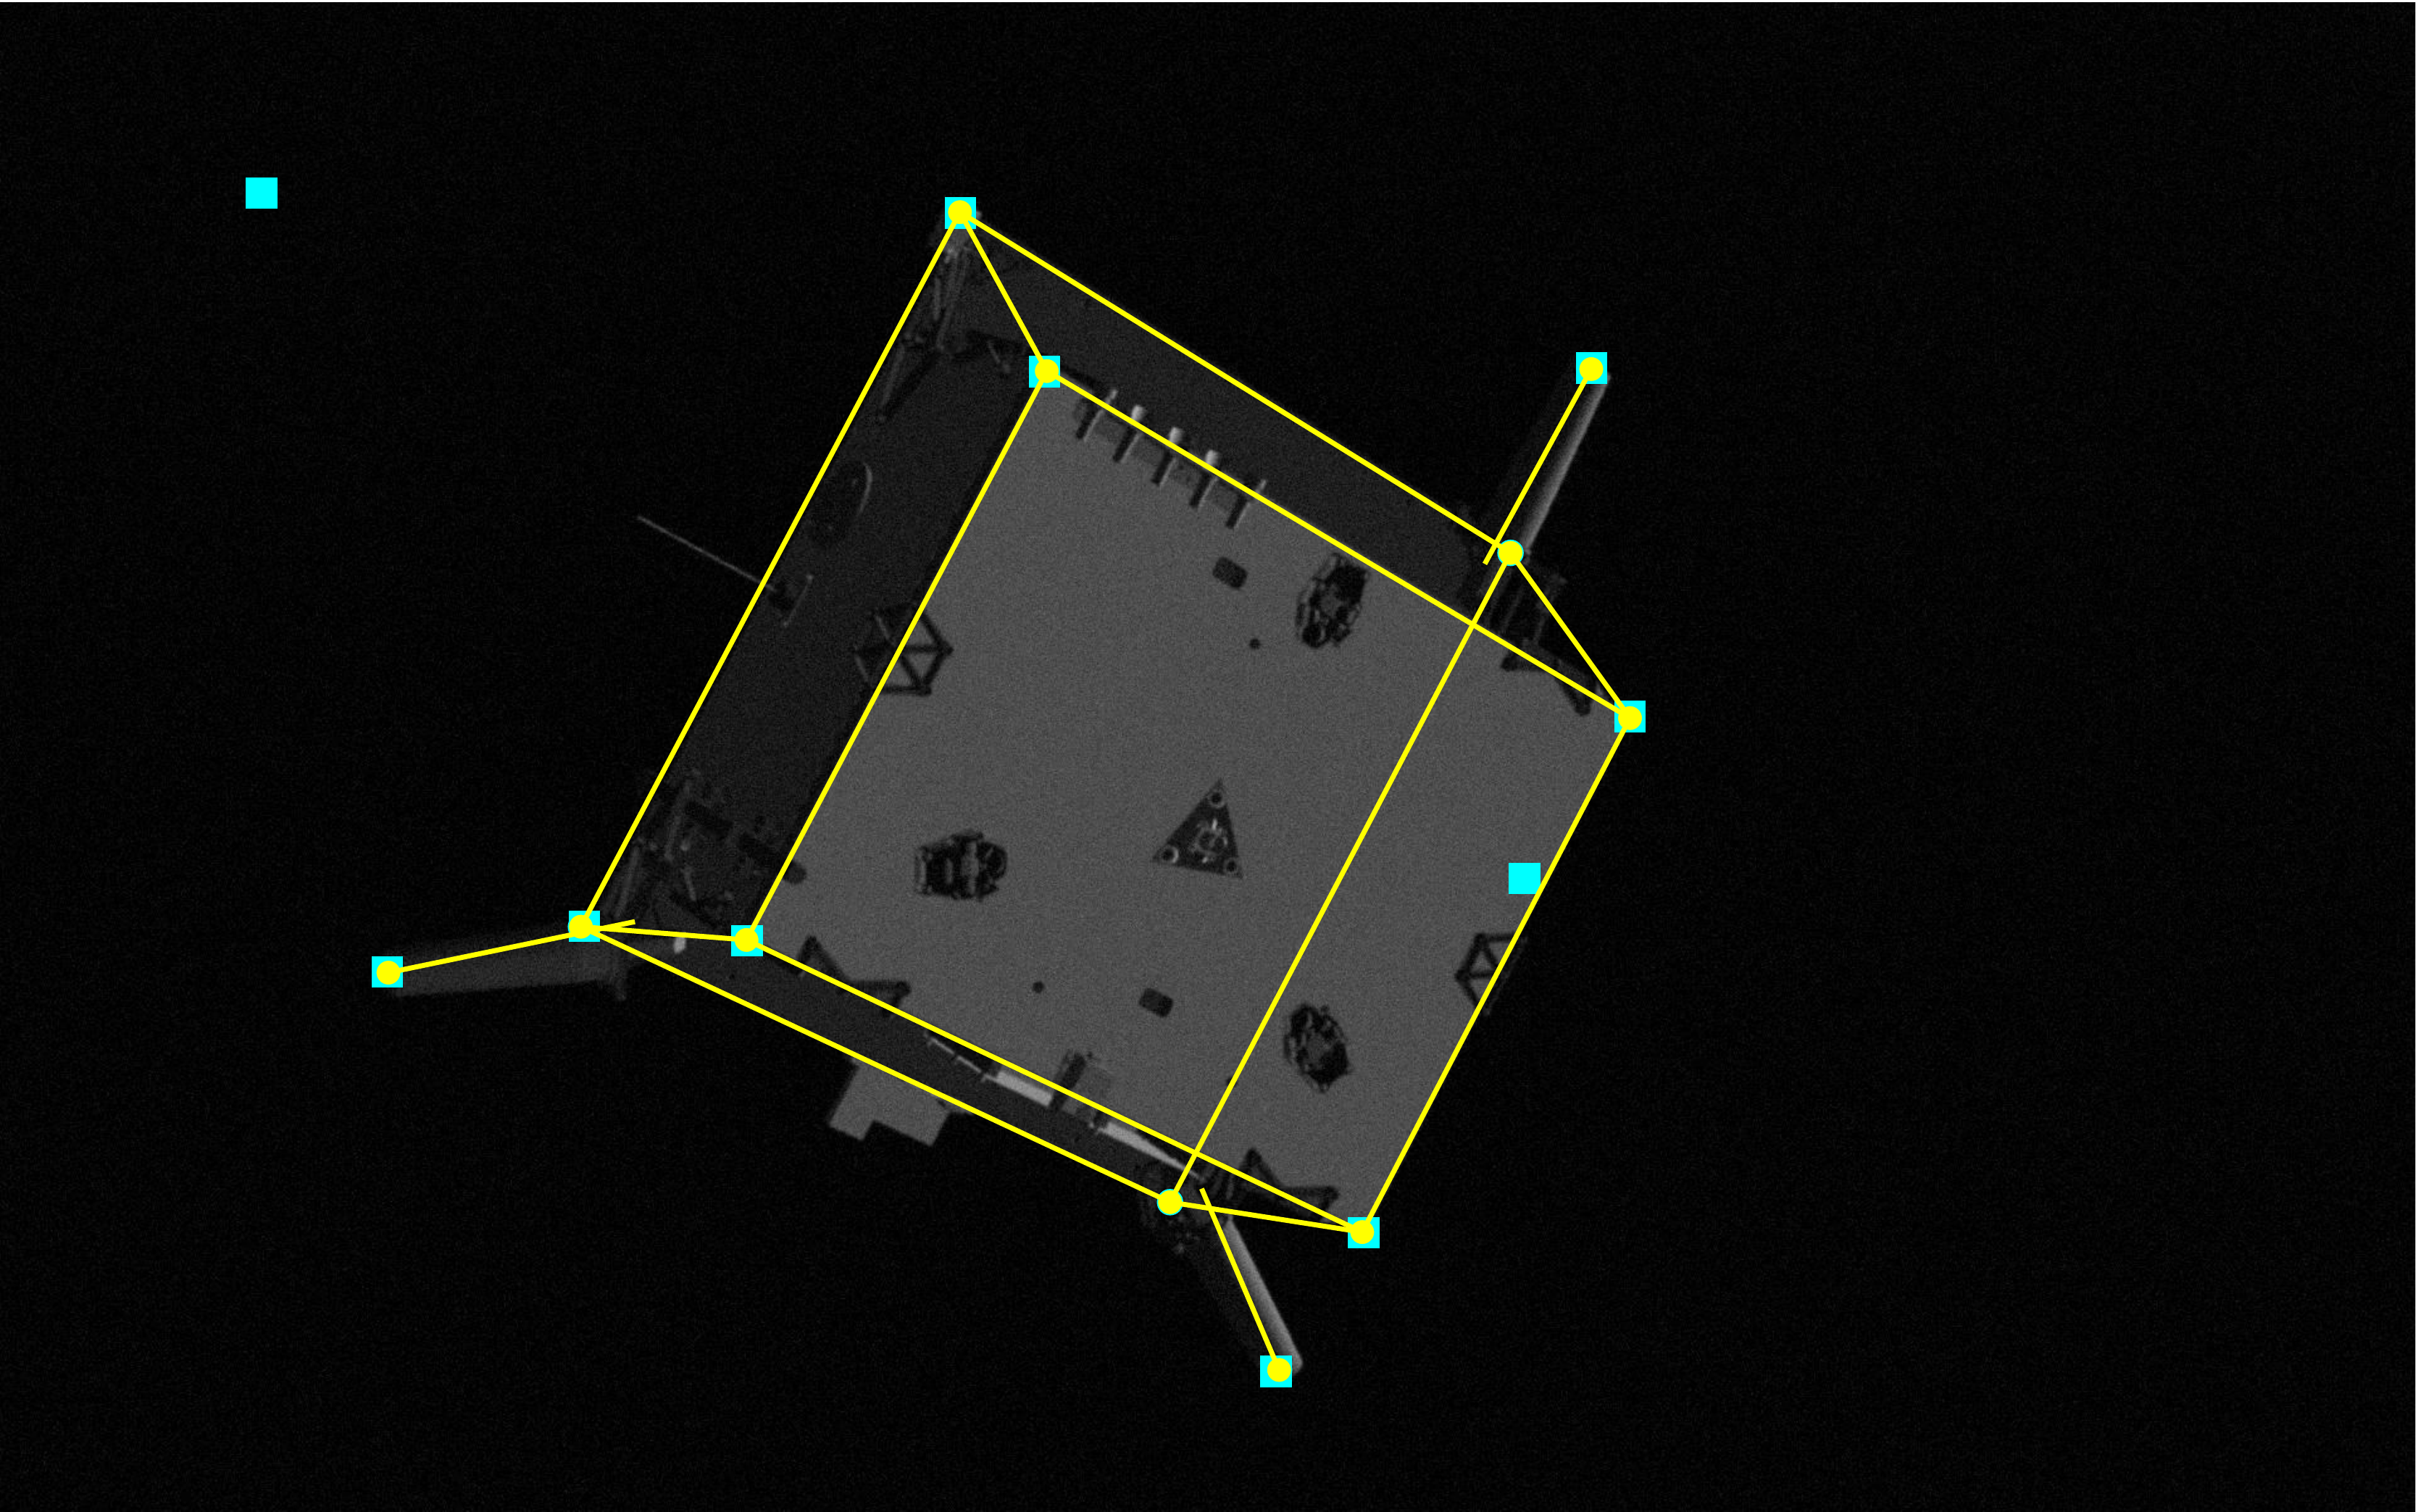}\\
			 $\MR$ error: $0.21^{\circ}$, $\vt$ error: $0.003$ \\ 
			 $\subopt=5.7\ee{-10}$, time: $44$ [s]
			\end{minipage}
		&  
			\begin{minipage}{\mpwfour}%
			\centering%
			\includegraphics[width=\columnwidth]{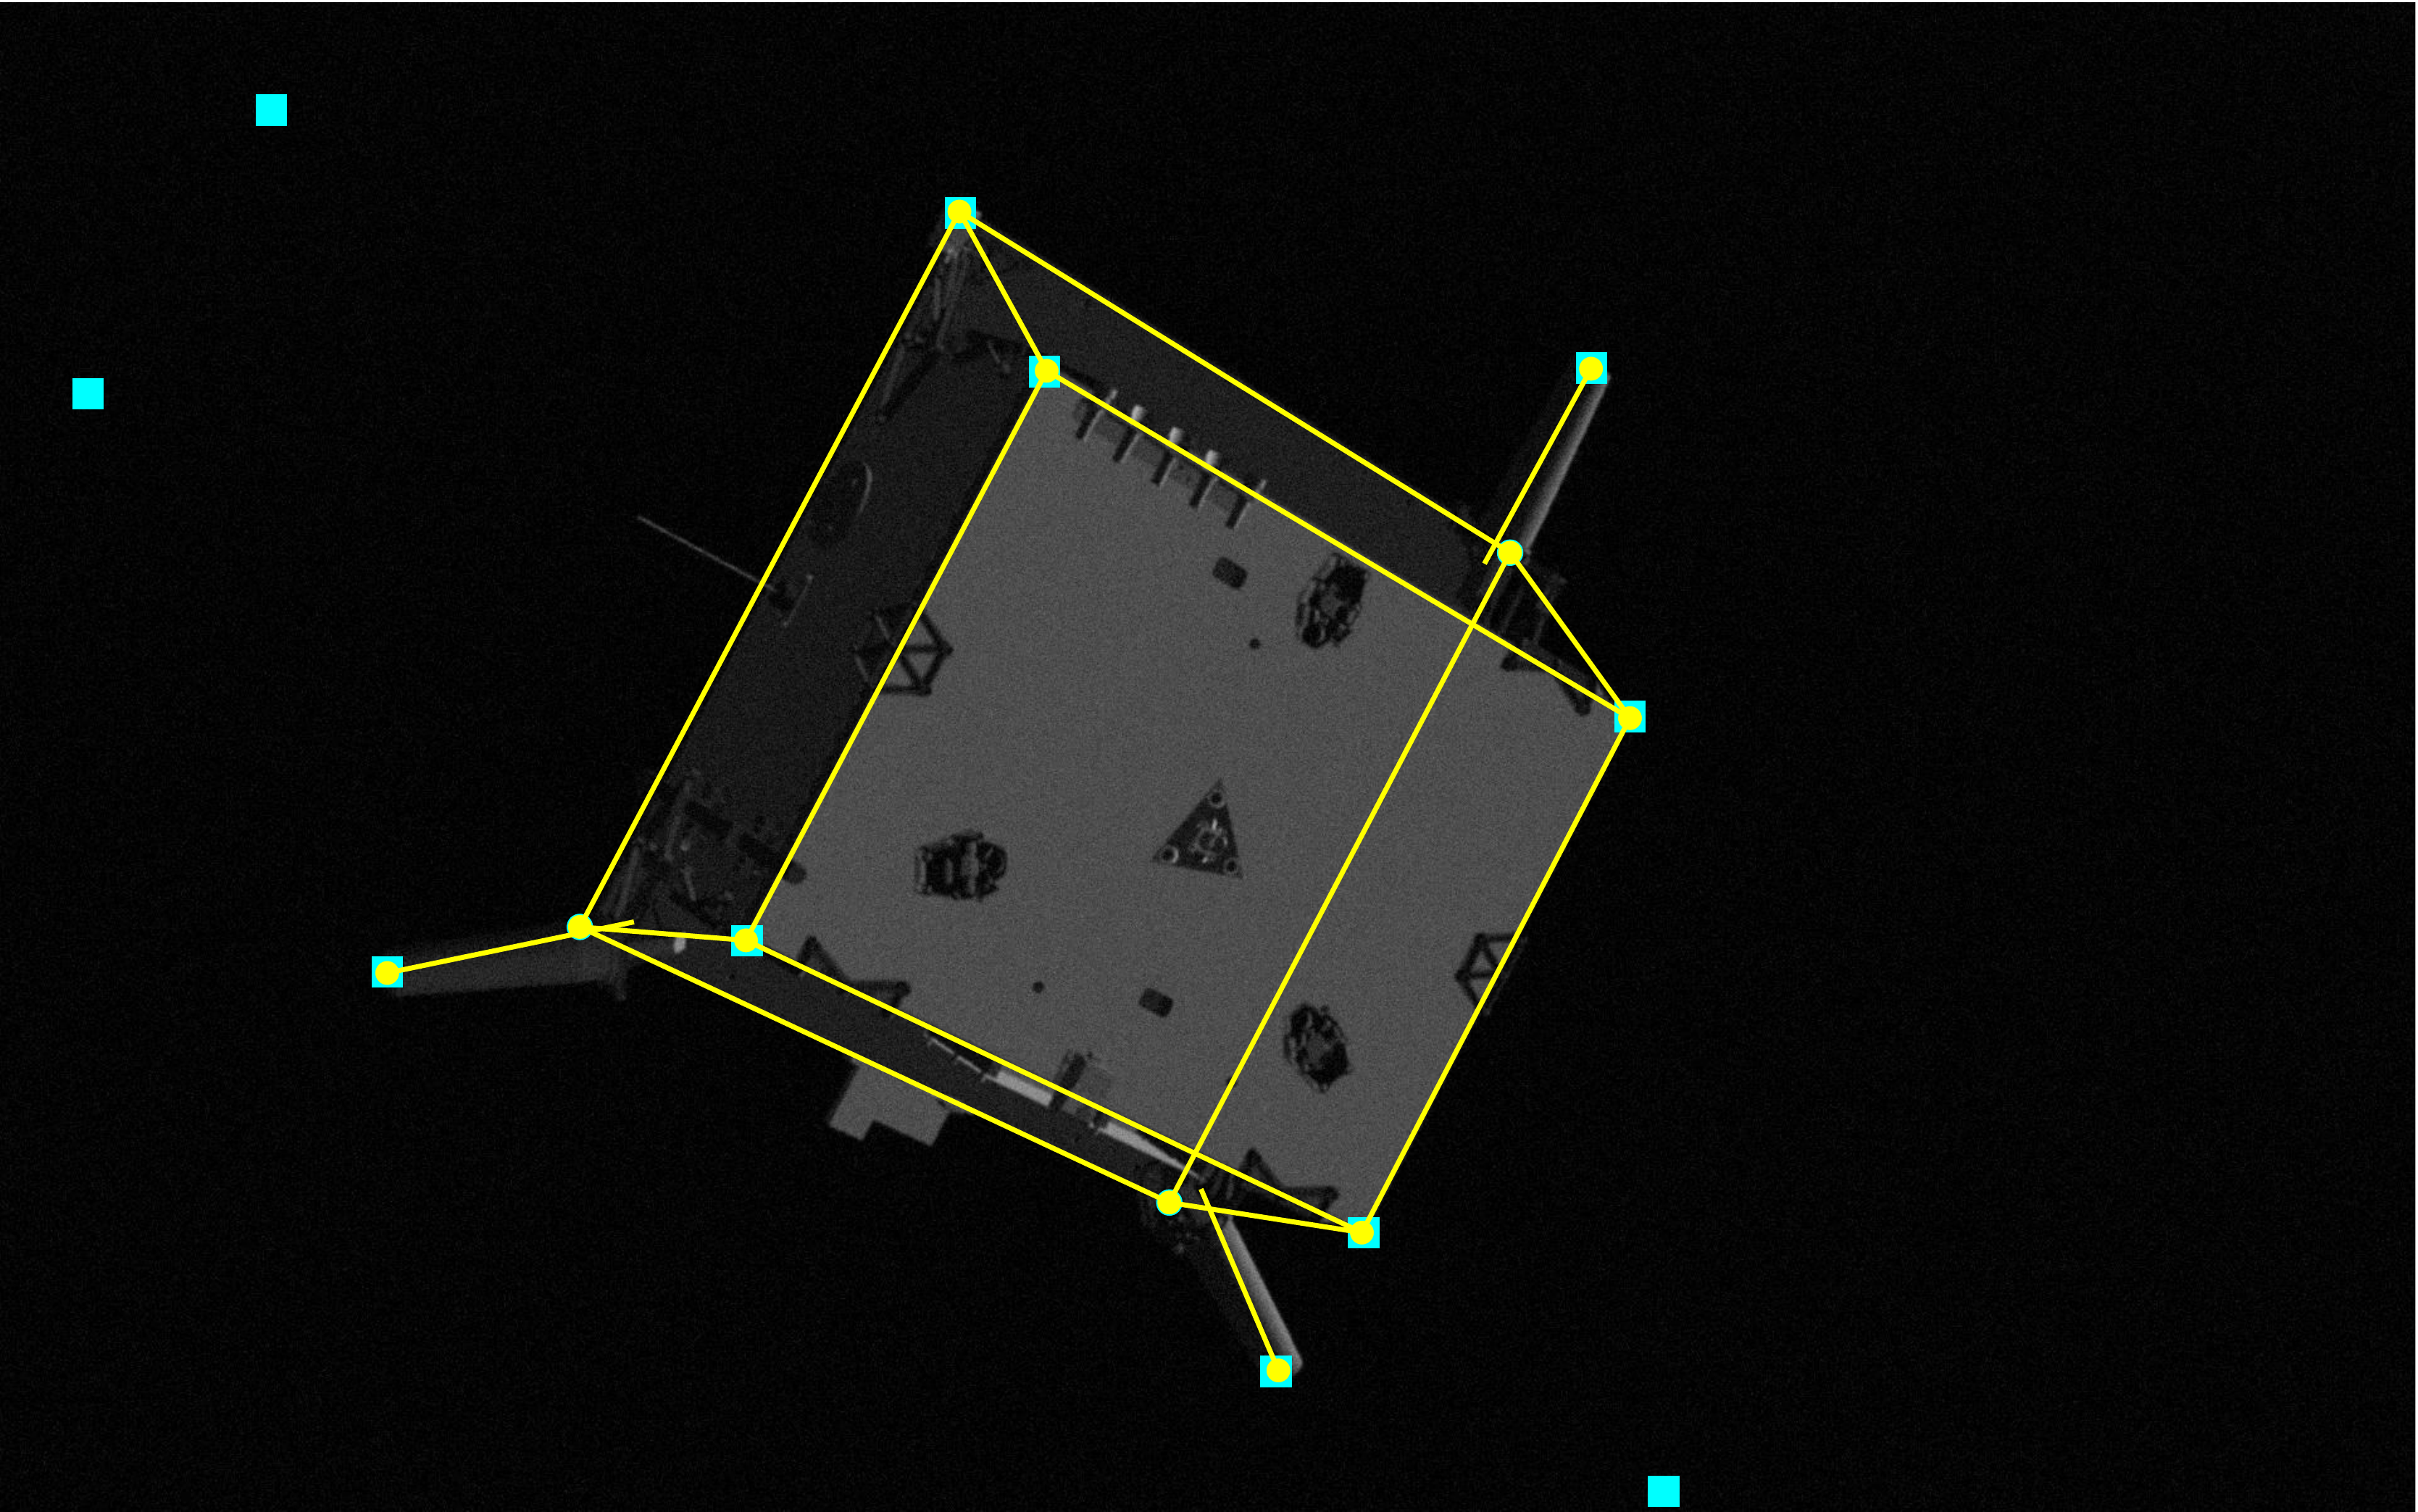}\\
			 $\MR$ error: $0.28^{\circ}$, $\vt$ error: $0.006$ \\ 
			 $\subopt=4.6\ee{-8}$, time: $47$ [s]
			\end{minipage}
		&  
			\begin{minipage}{\mpwfour}%
			\centering%
			\includegraphics[width=\columnwidth]{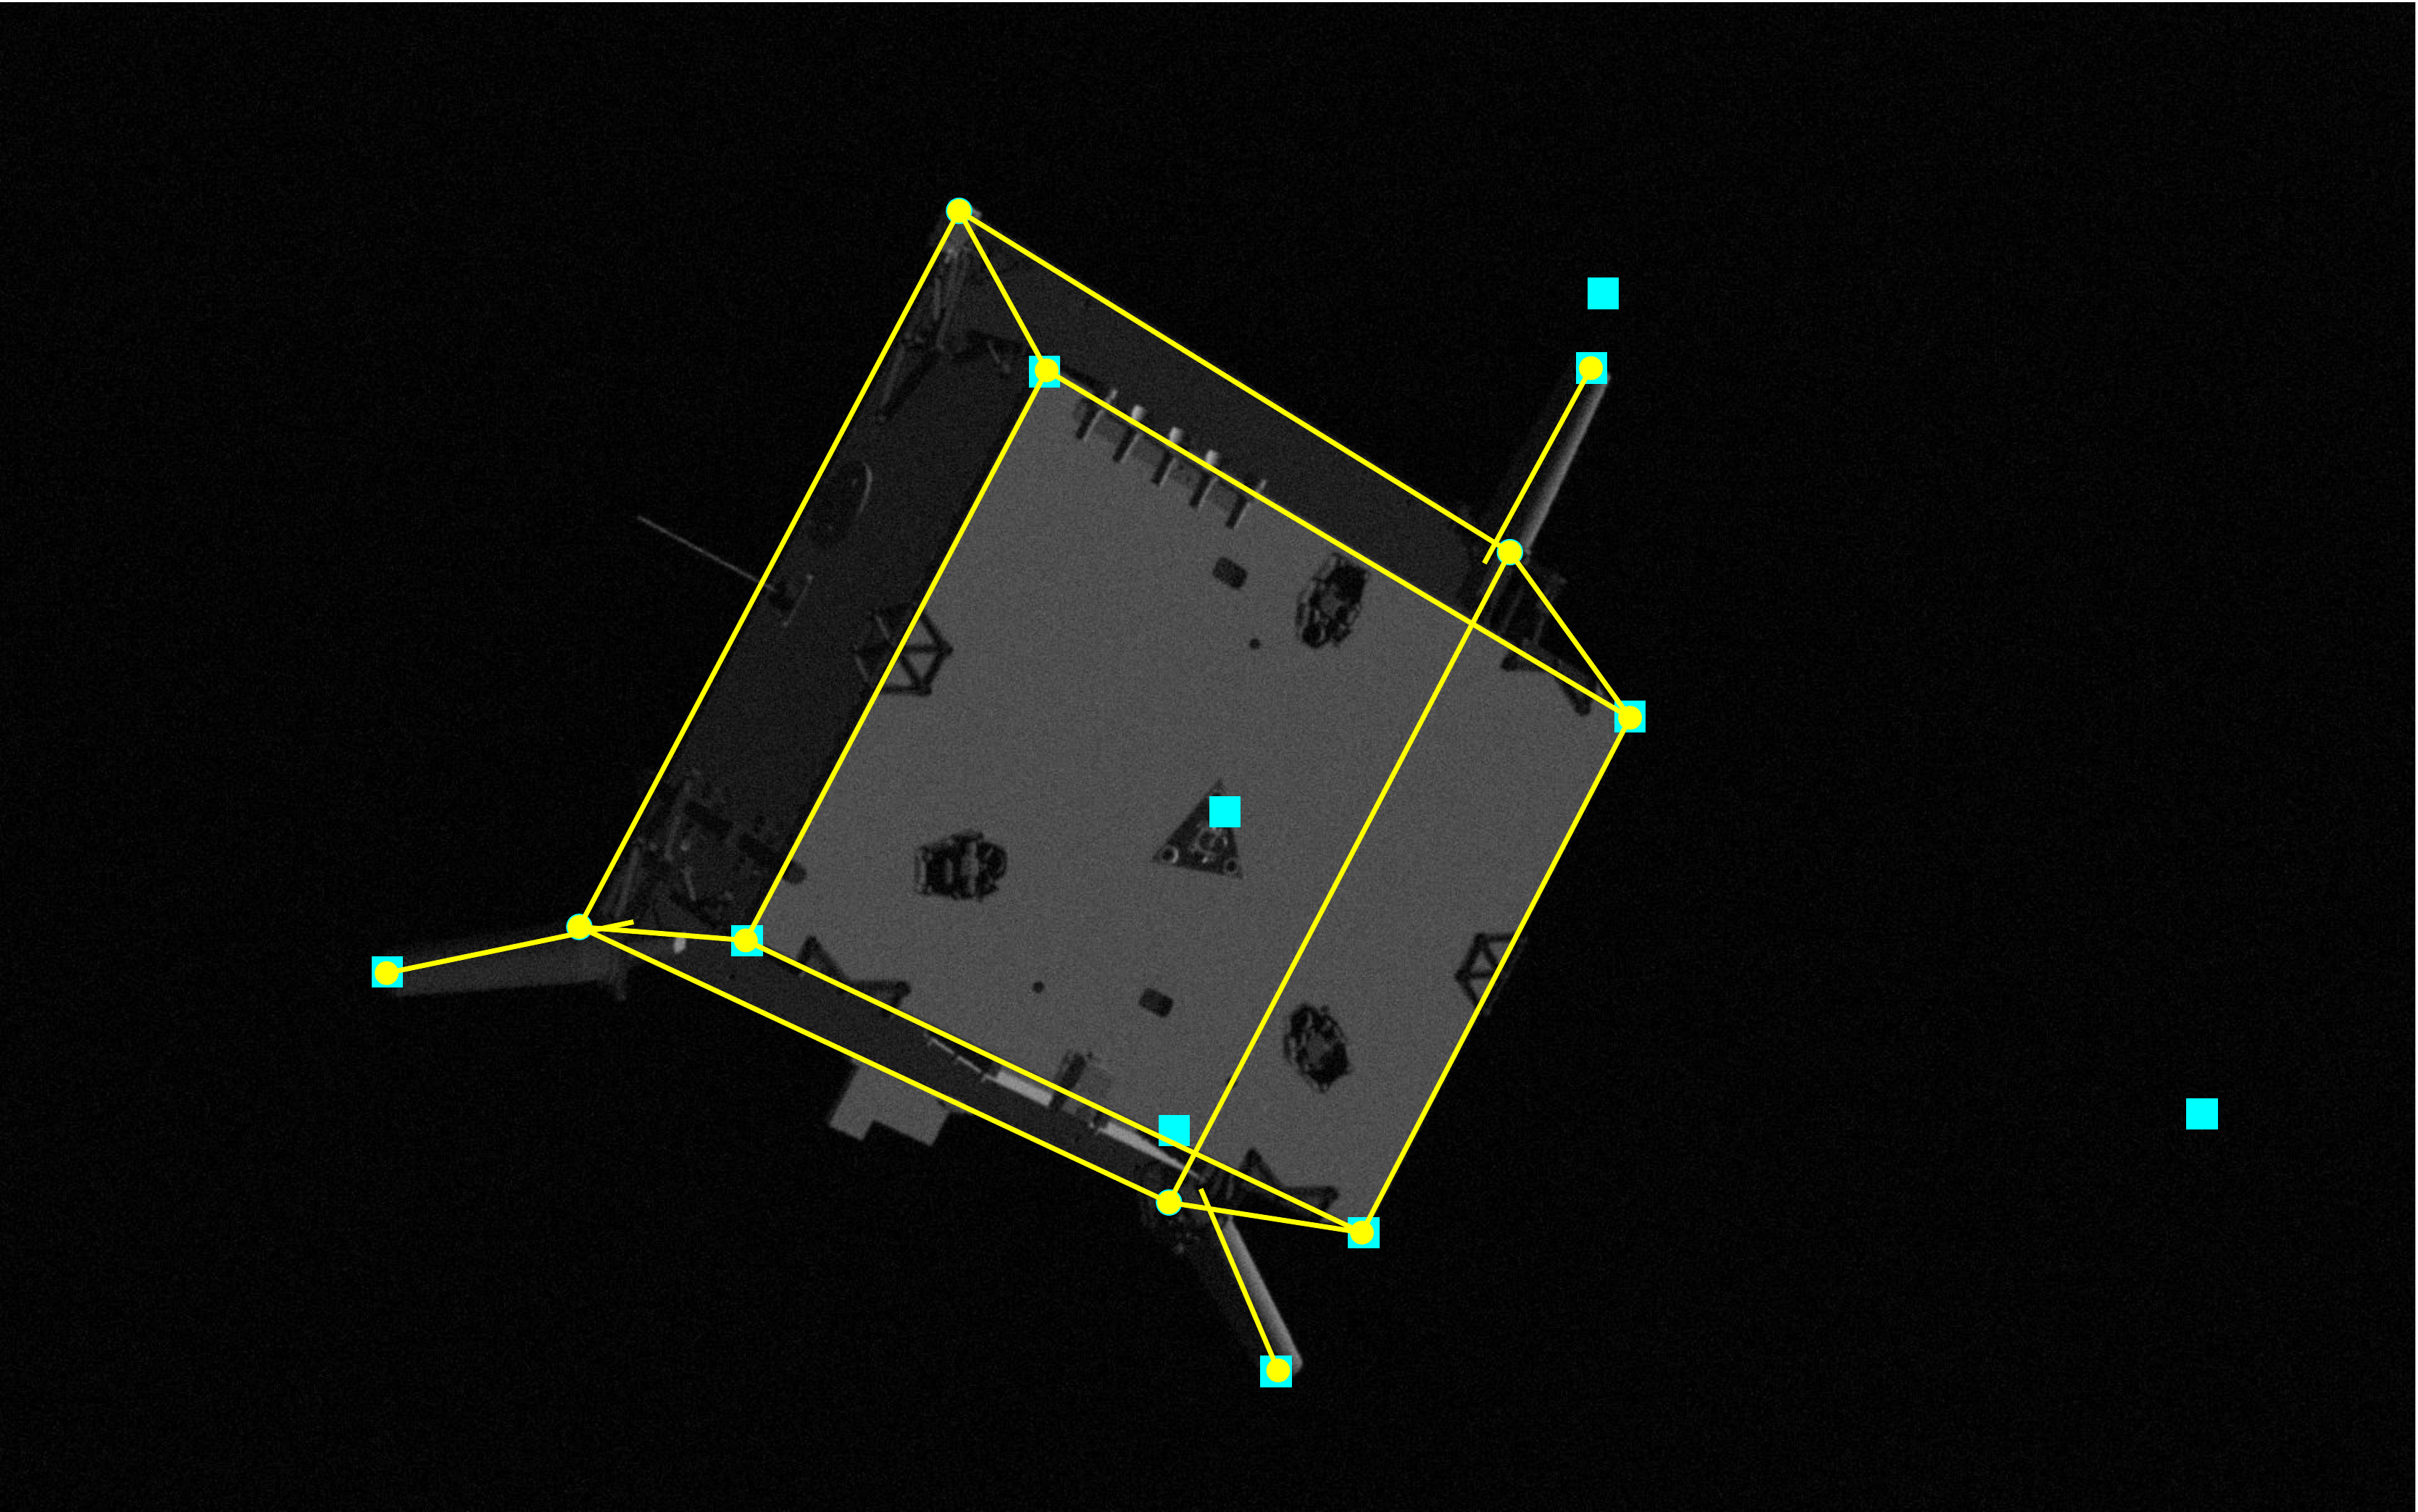}\\
			 $\MR$ error: $0.32^{\circ}$, $\vt$ error: $0.008$ \\ 
			 $\subopt=4.6\ee{-8}$, time: $49$ [s]
			\end{minipage}
		&  
			\begin{minipage}{\mpwfour}%
			\centering%
			\includegraphics[width=\columnwidth]{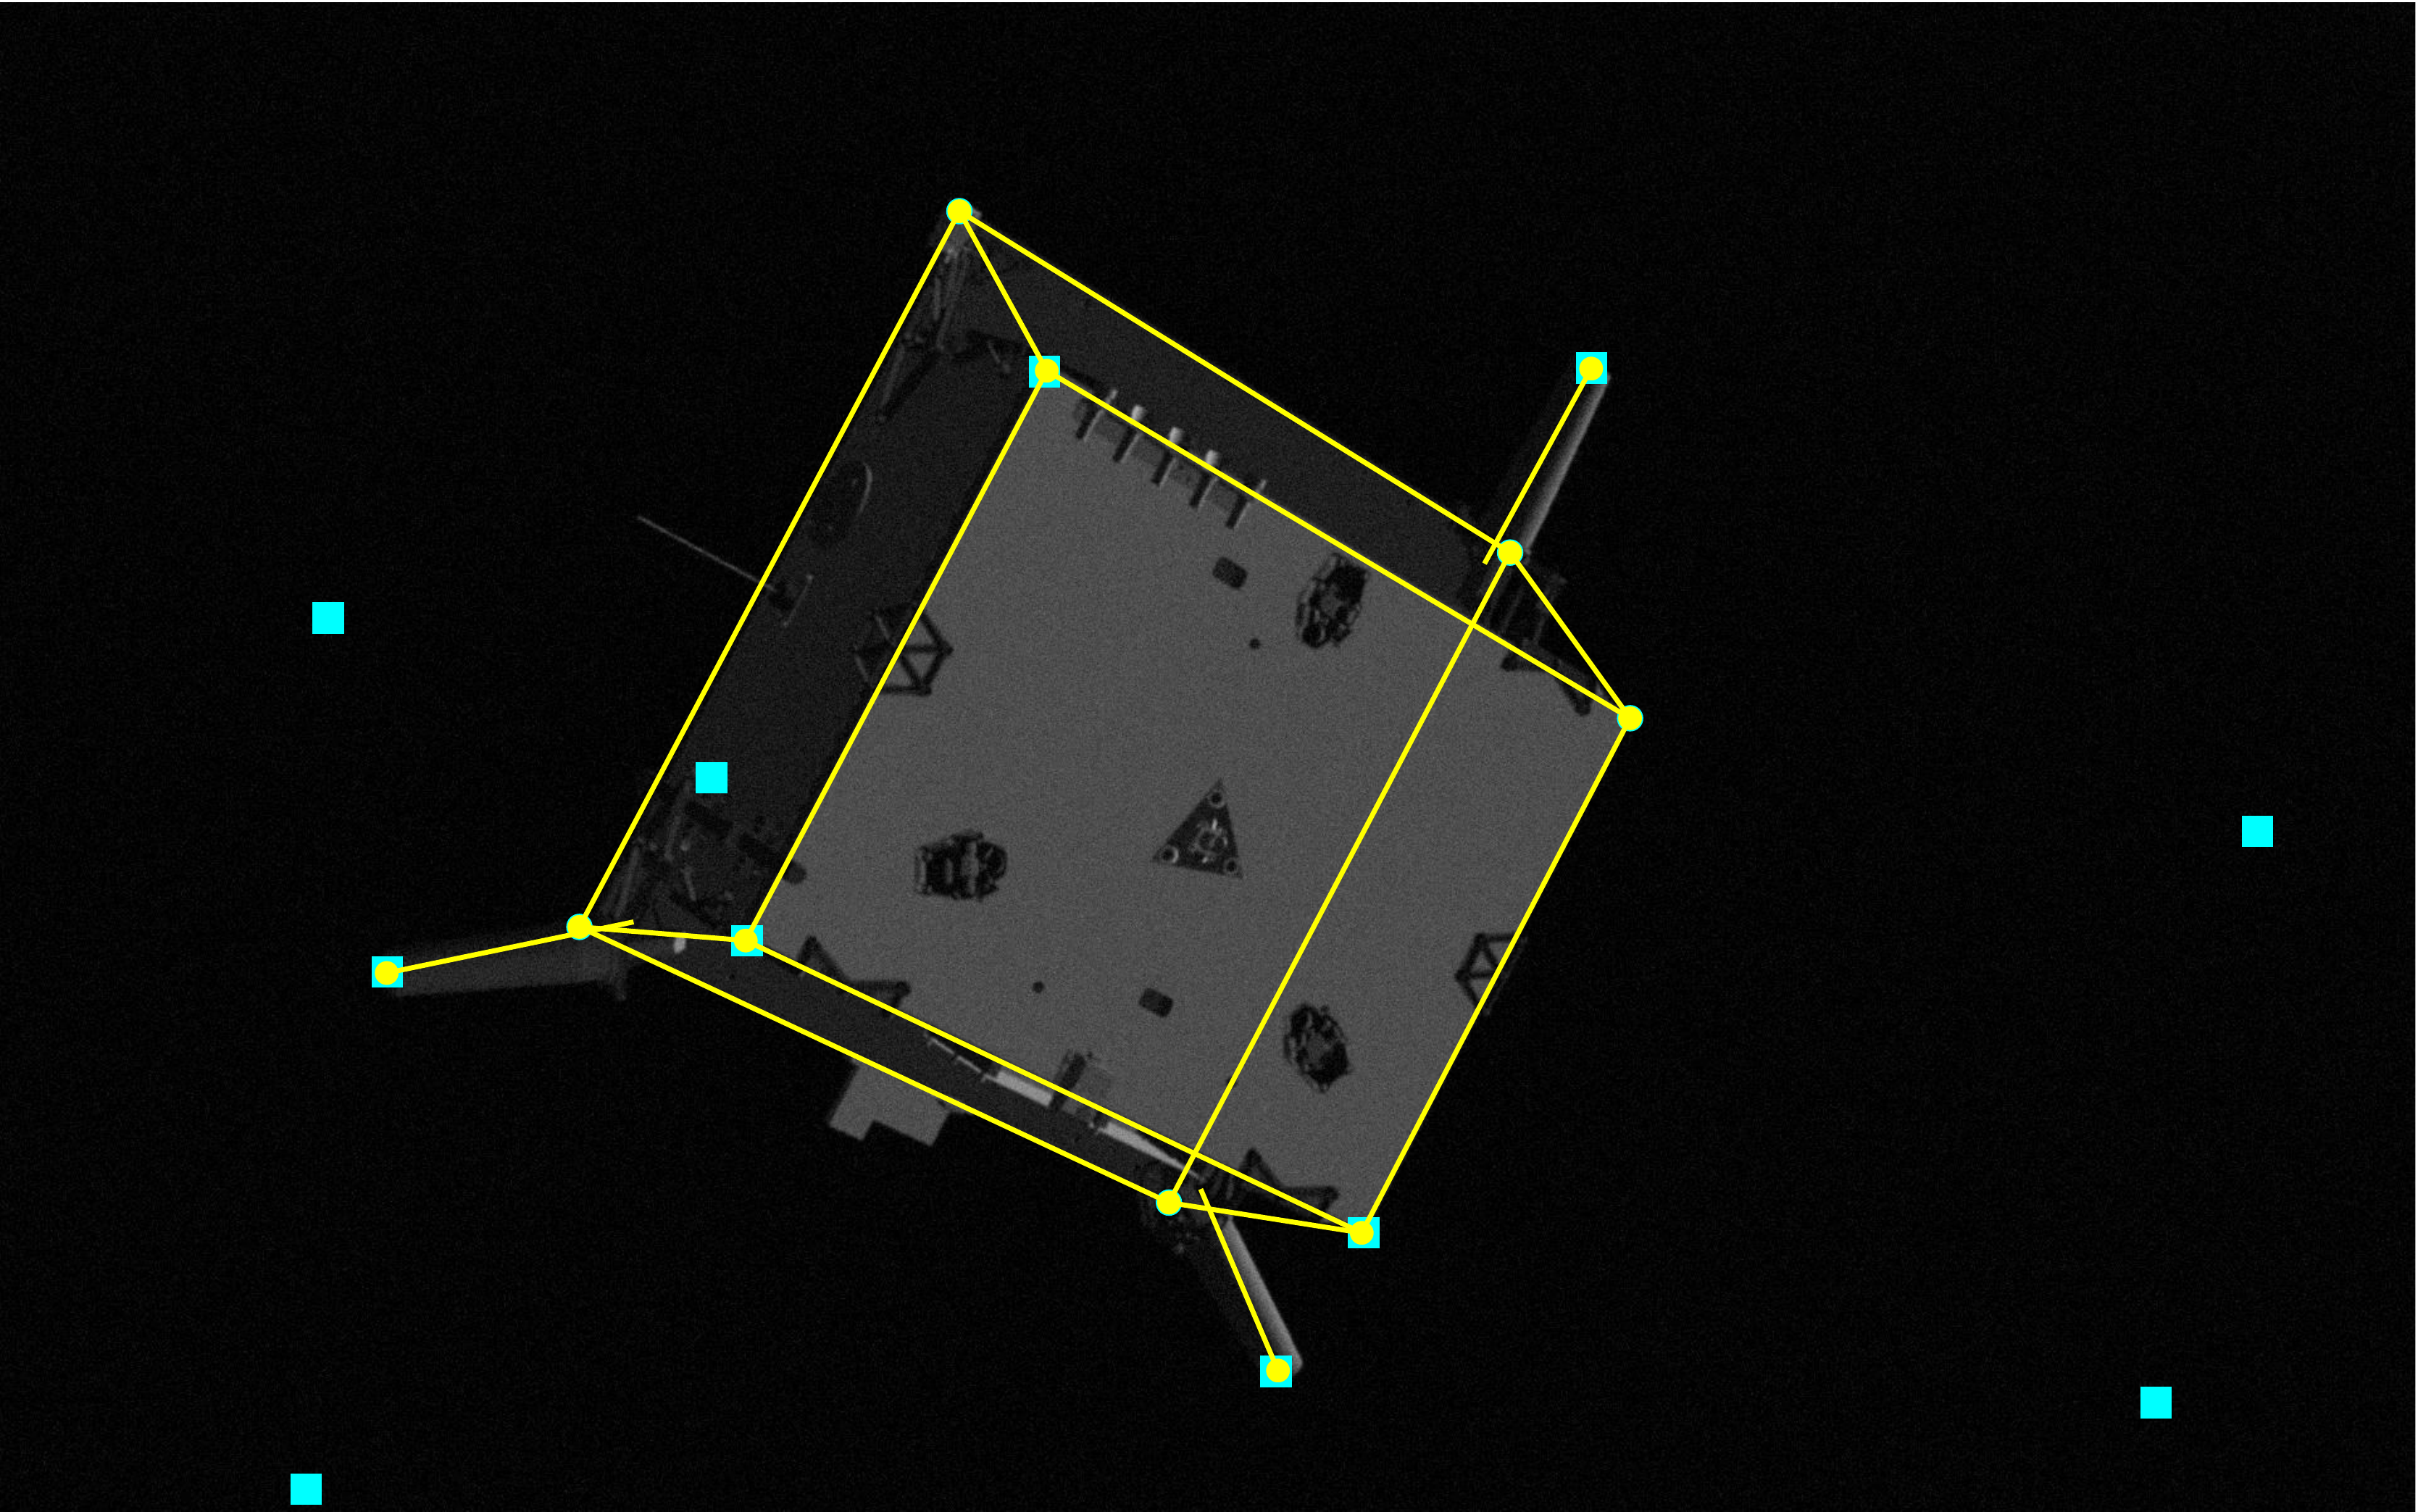}\\
			 $\MR$ error: $0.32^{\circ}$, $\vt$ error: $0.008$ \\ 
			 $\subopt=1.8\ee{-6}$, time: $131$ [s]
			\end{minipage} \vspace{1mm}
		
	\end{tabular}
	\end{minipage}
	\caption{Extra satellite pose estimation results on {\speed}.
	\label{fig:supp-speed-results}} 
	\vspace{-4mm} 
	\end{center}
\end{figure*}
